# Supplementary material for: Developing hybrid mechanistic and data-driven personalized prediction models for platelet dynamics
Source: arXiv:2505.21204 source file (2025-05-27)

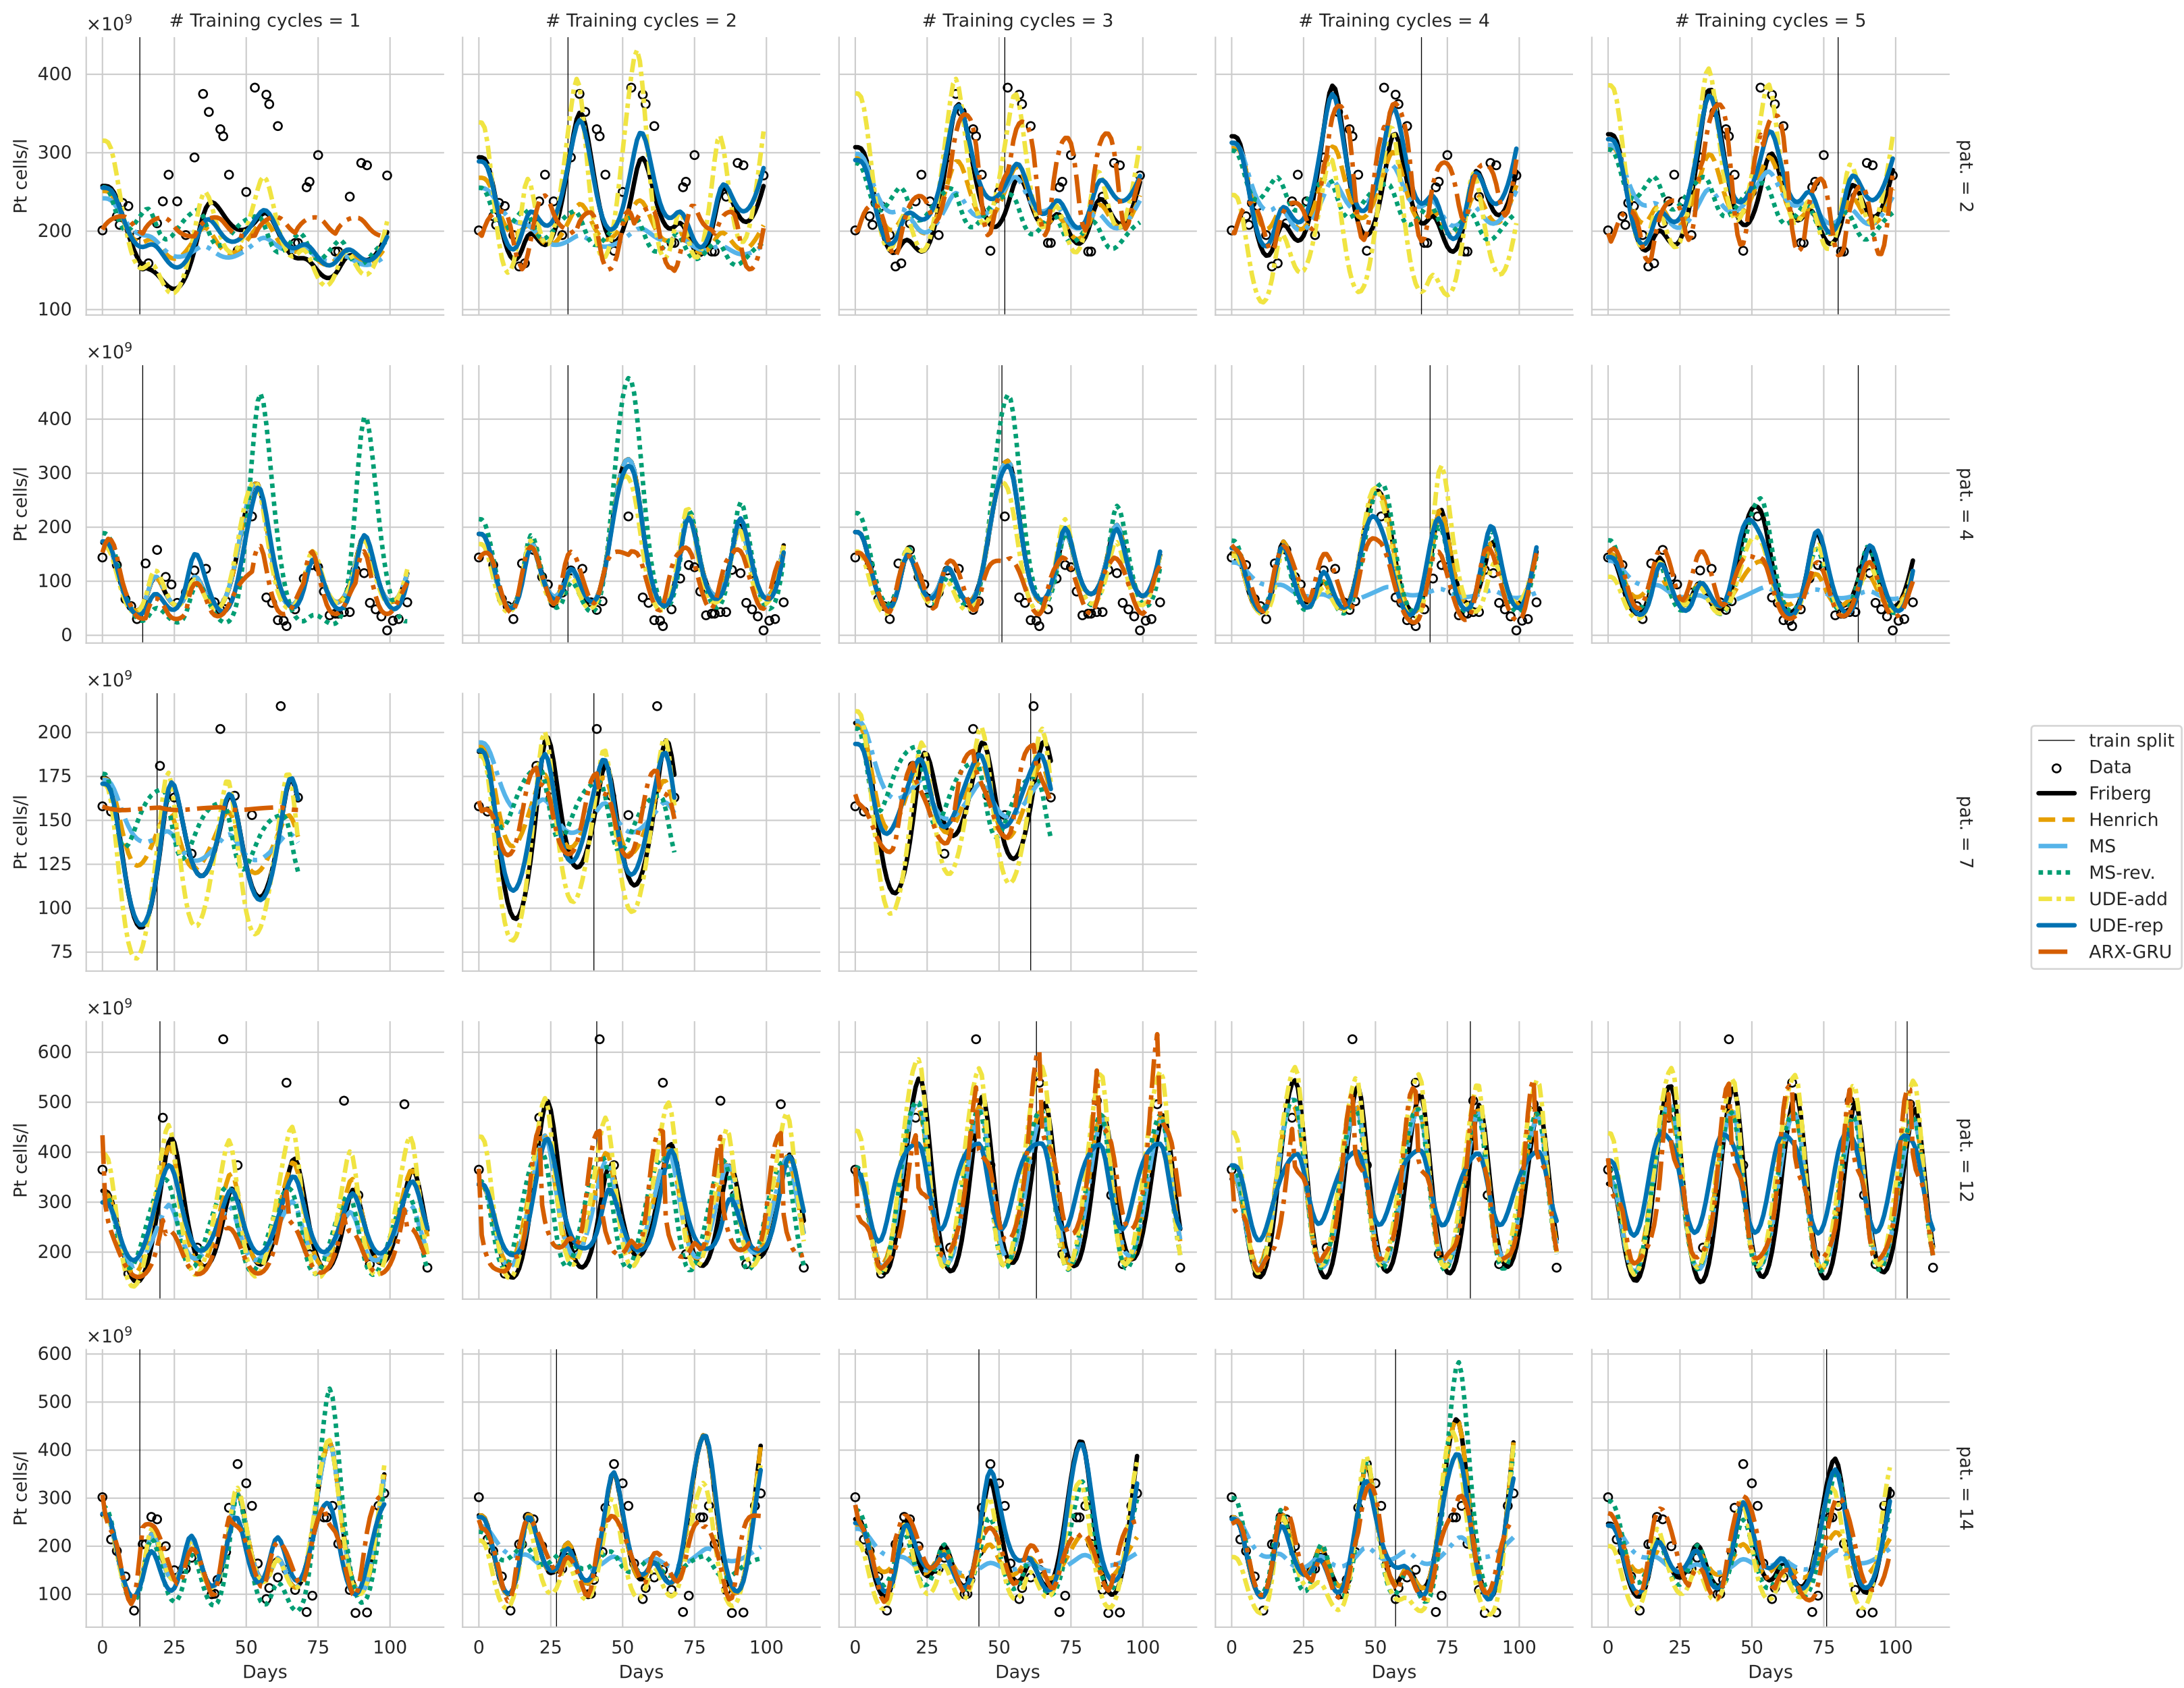

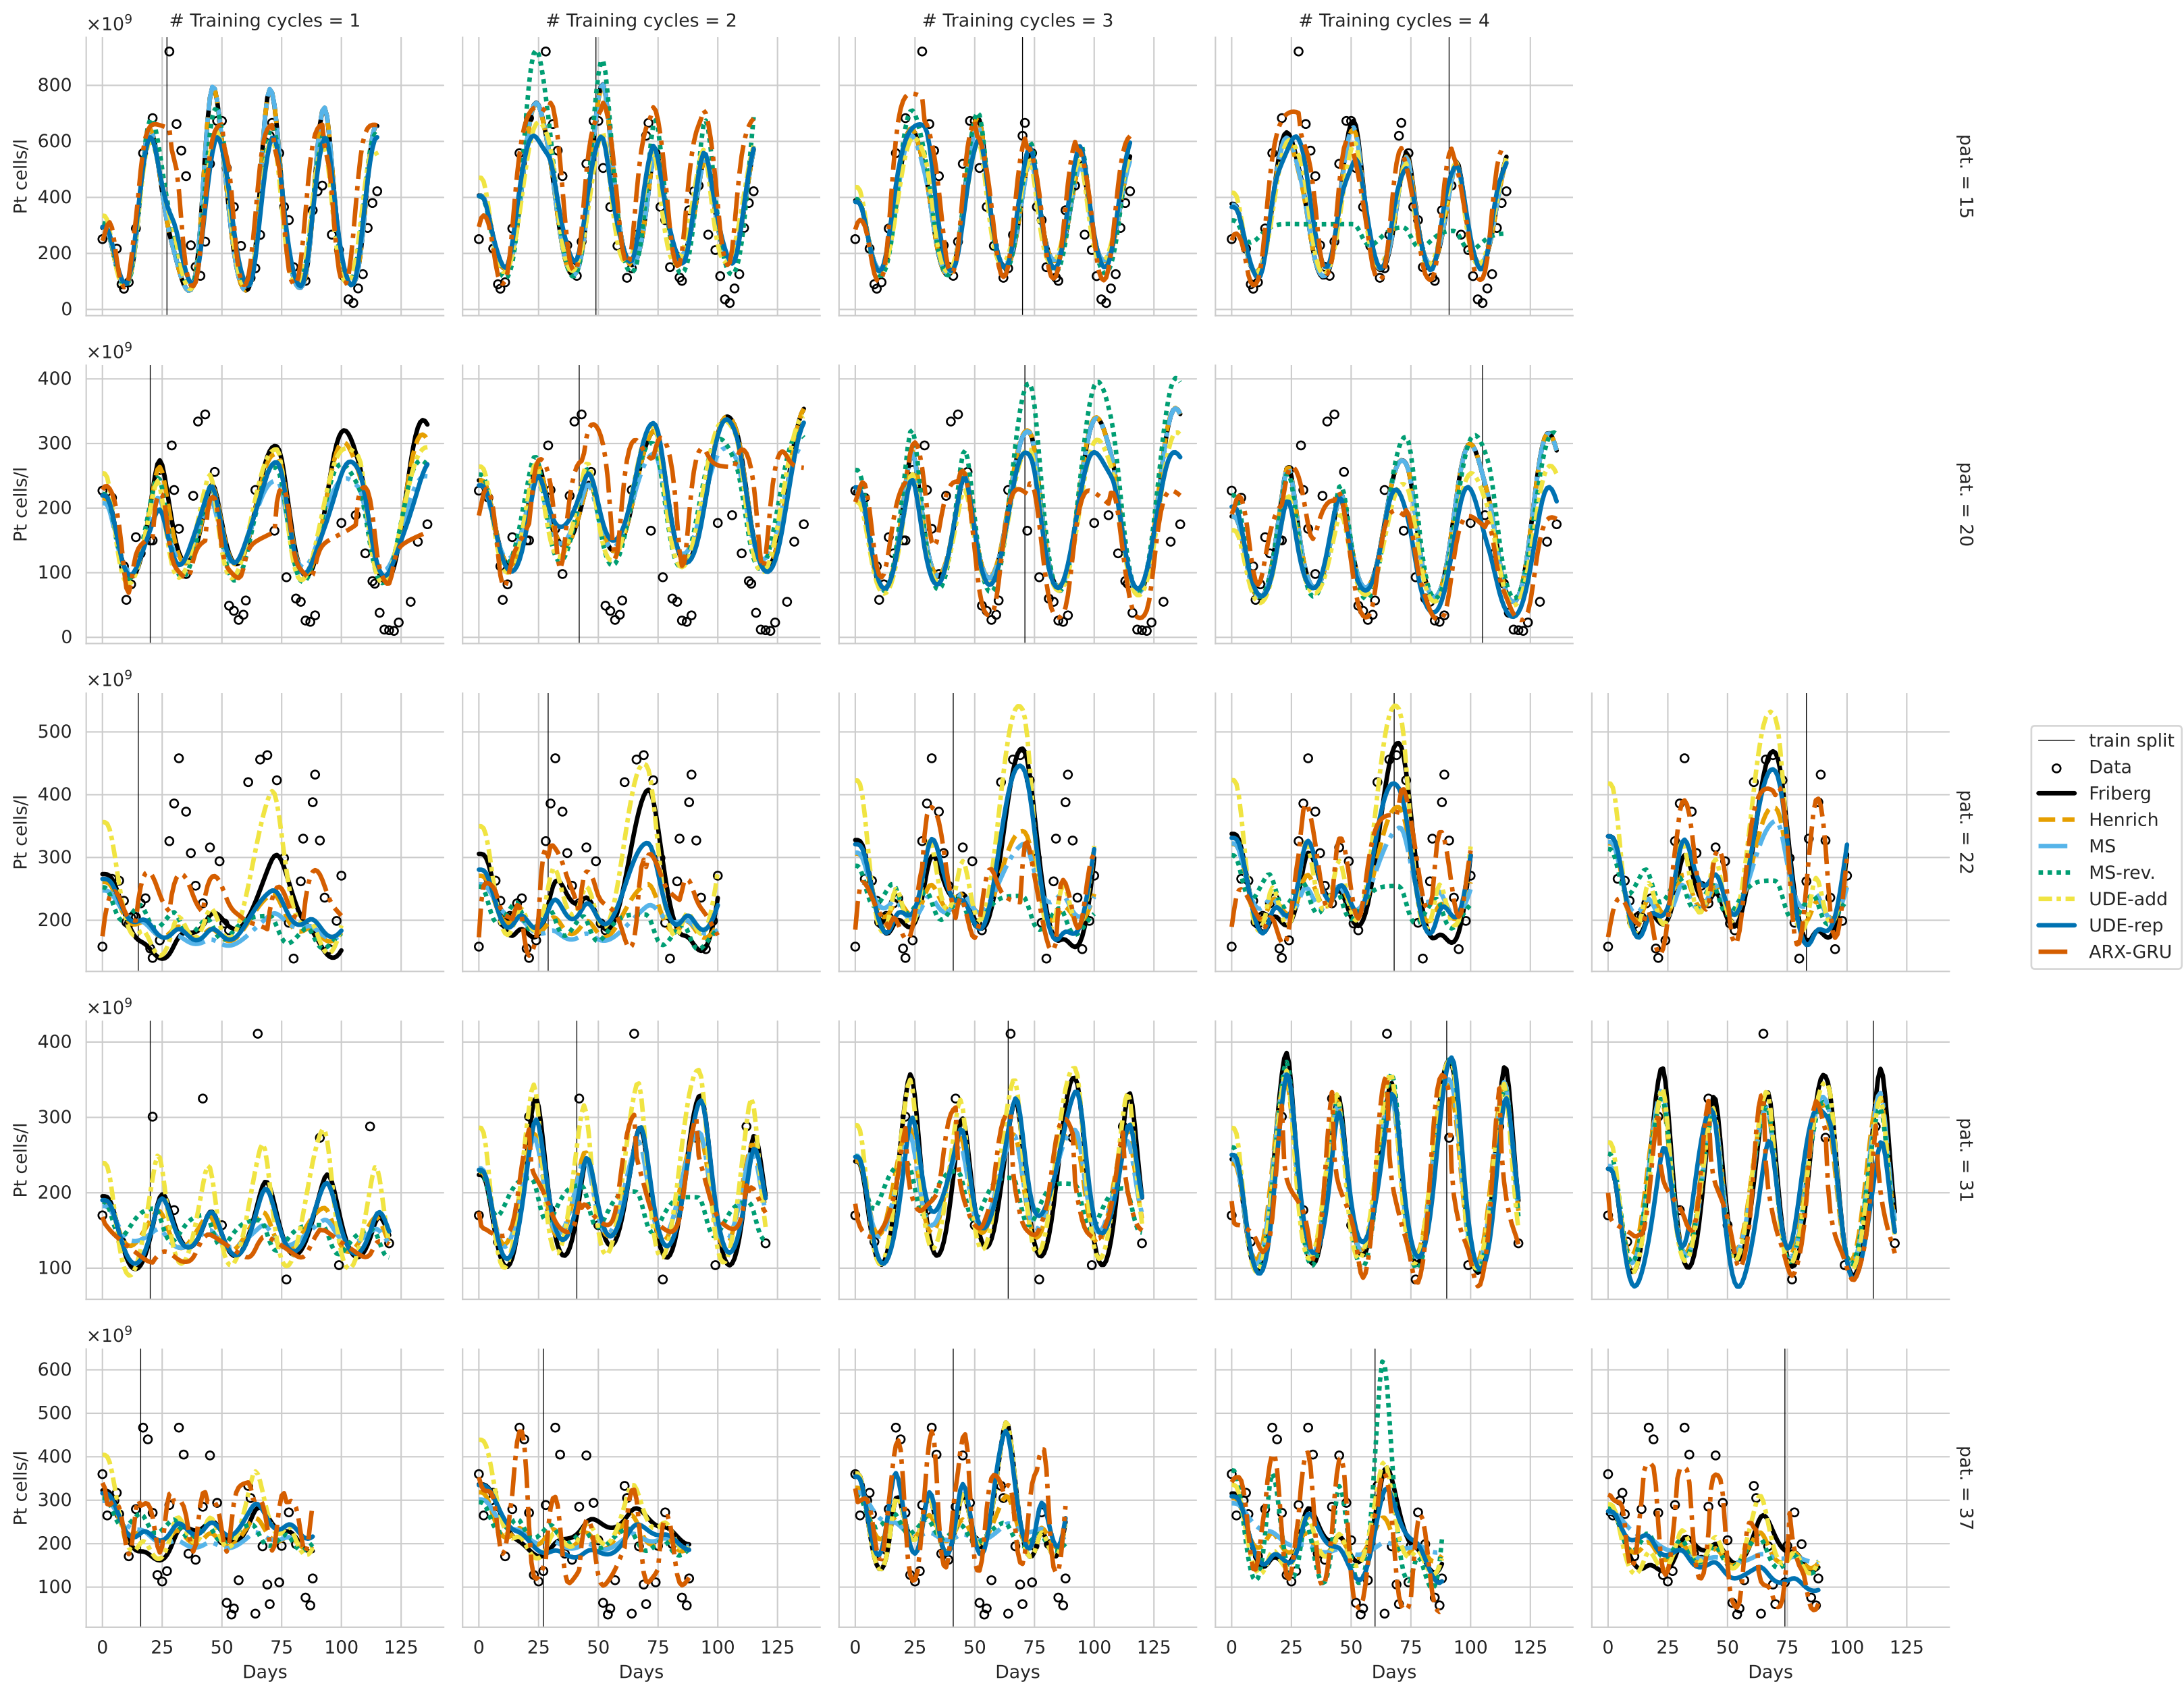



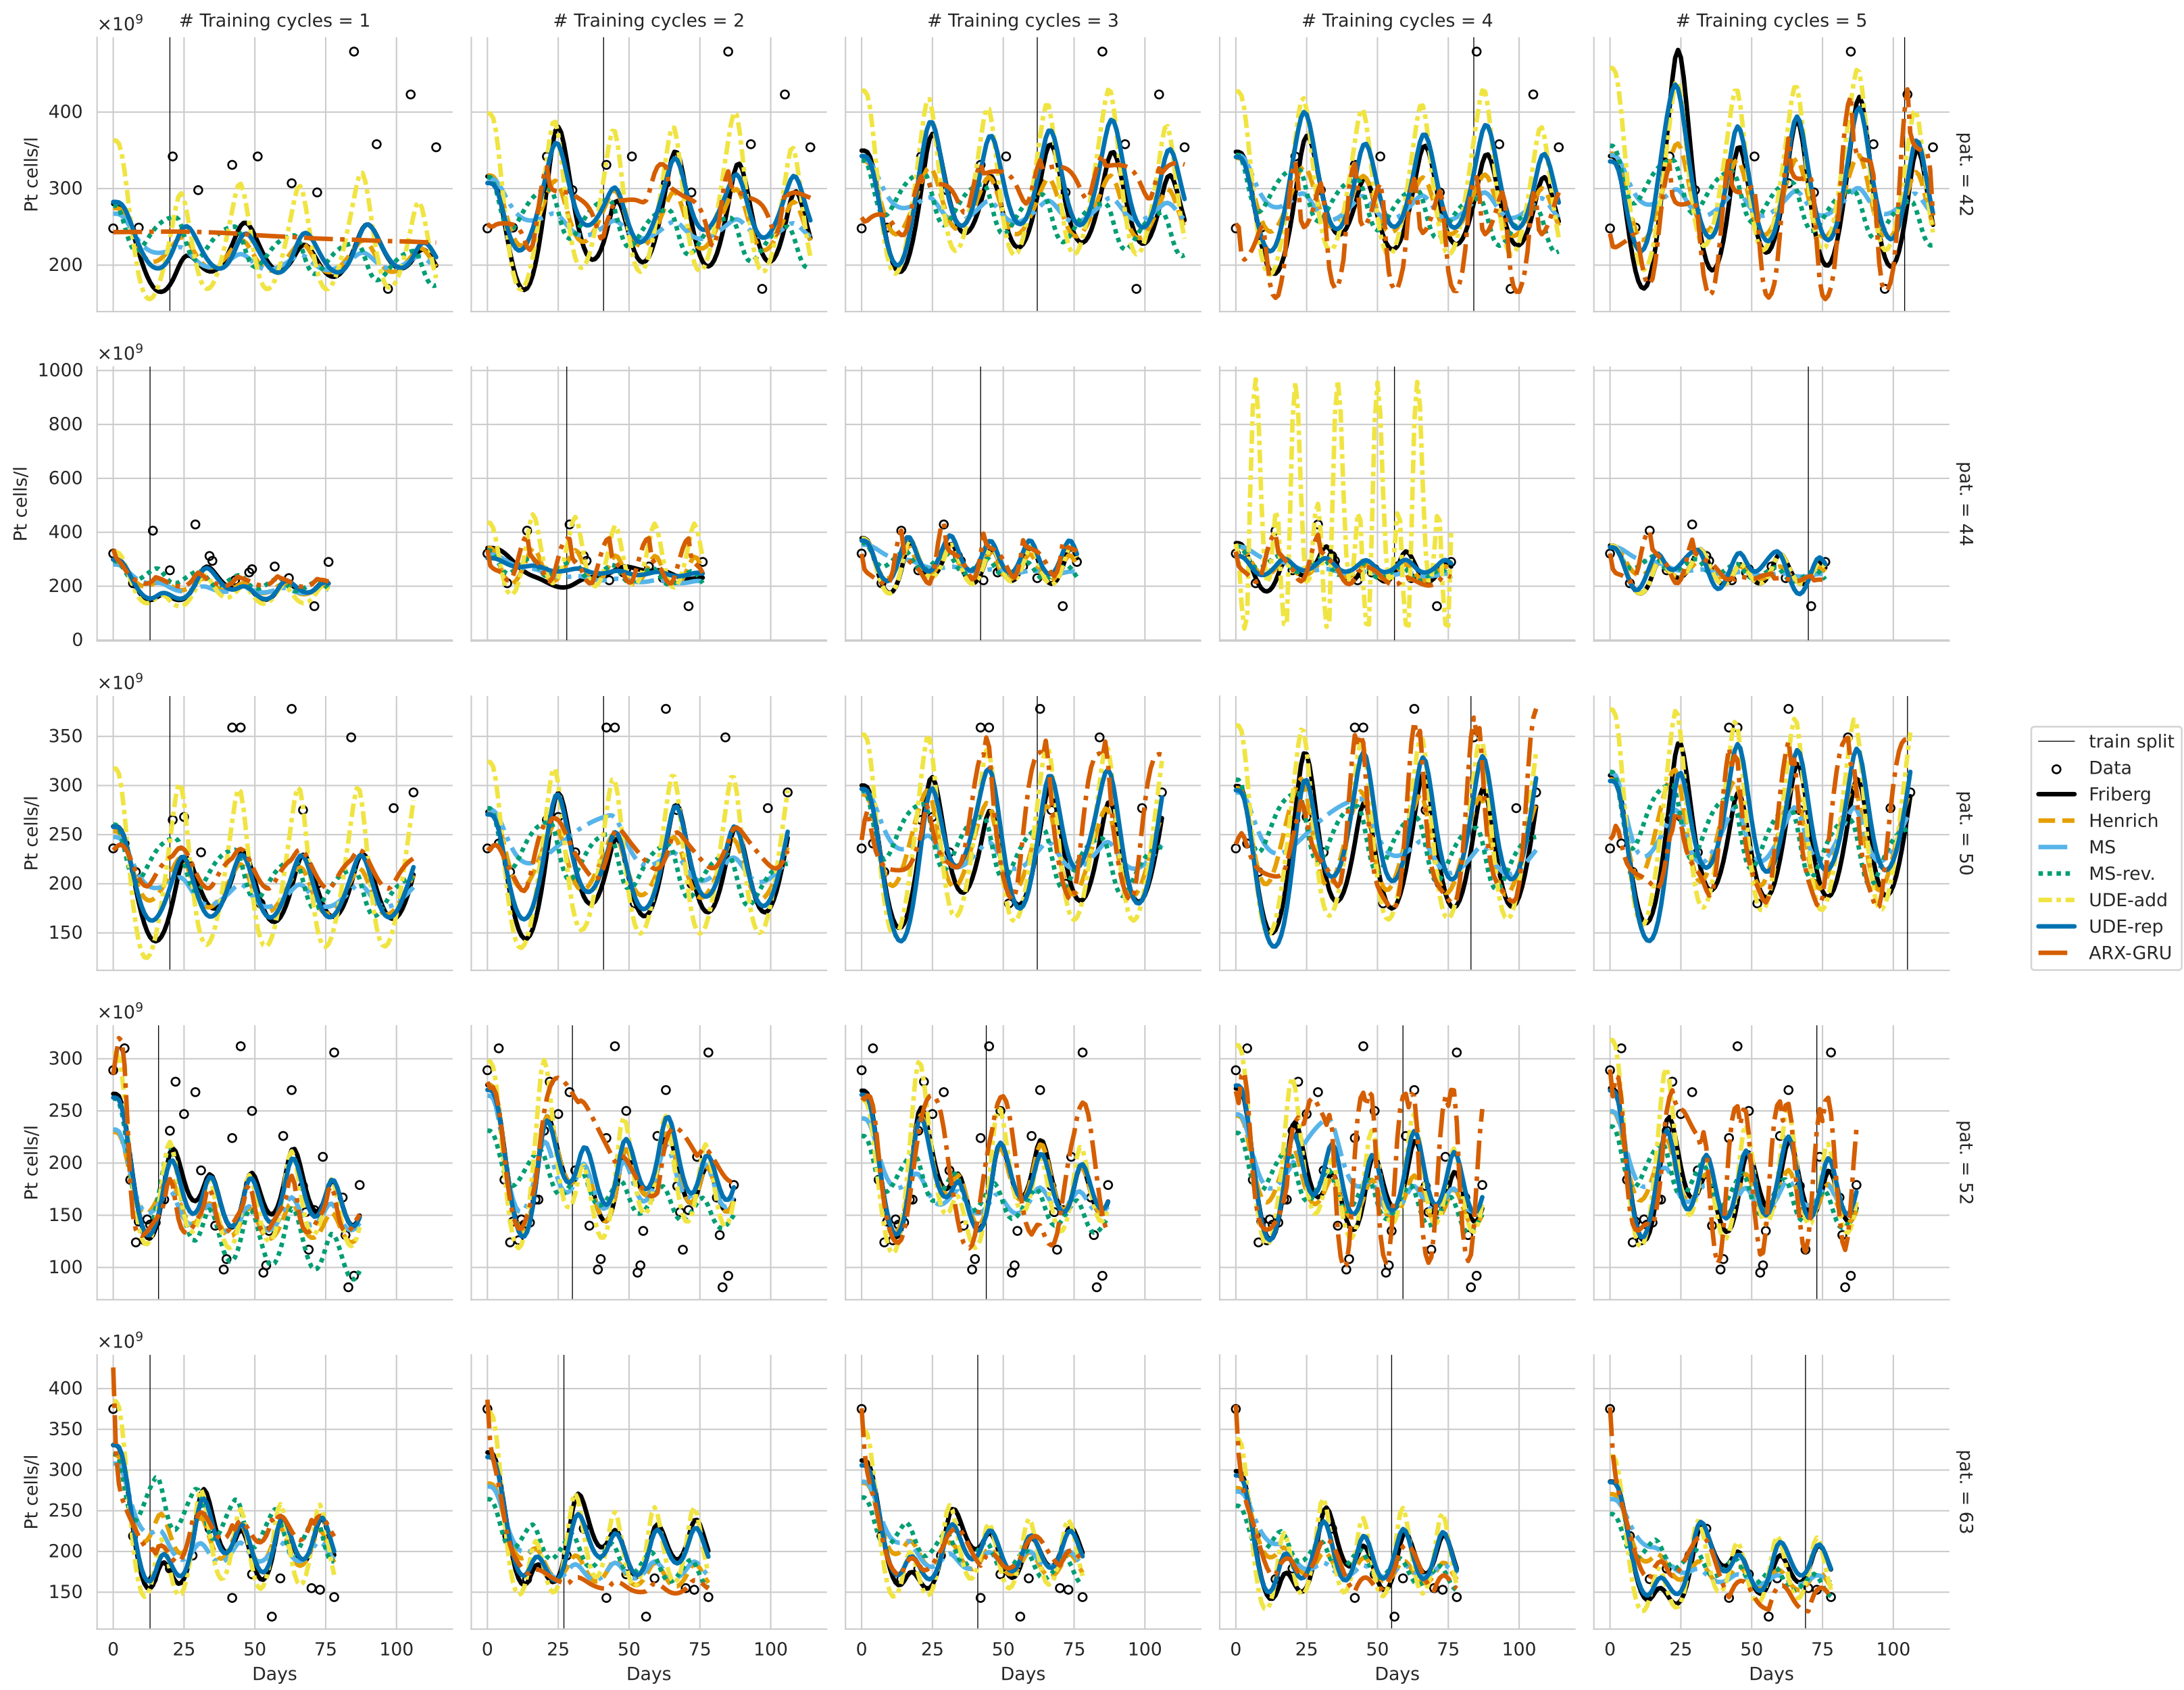

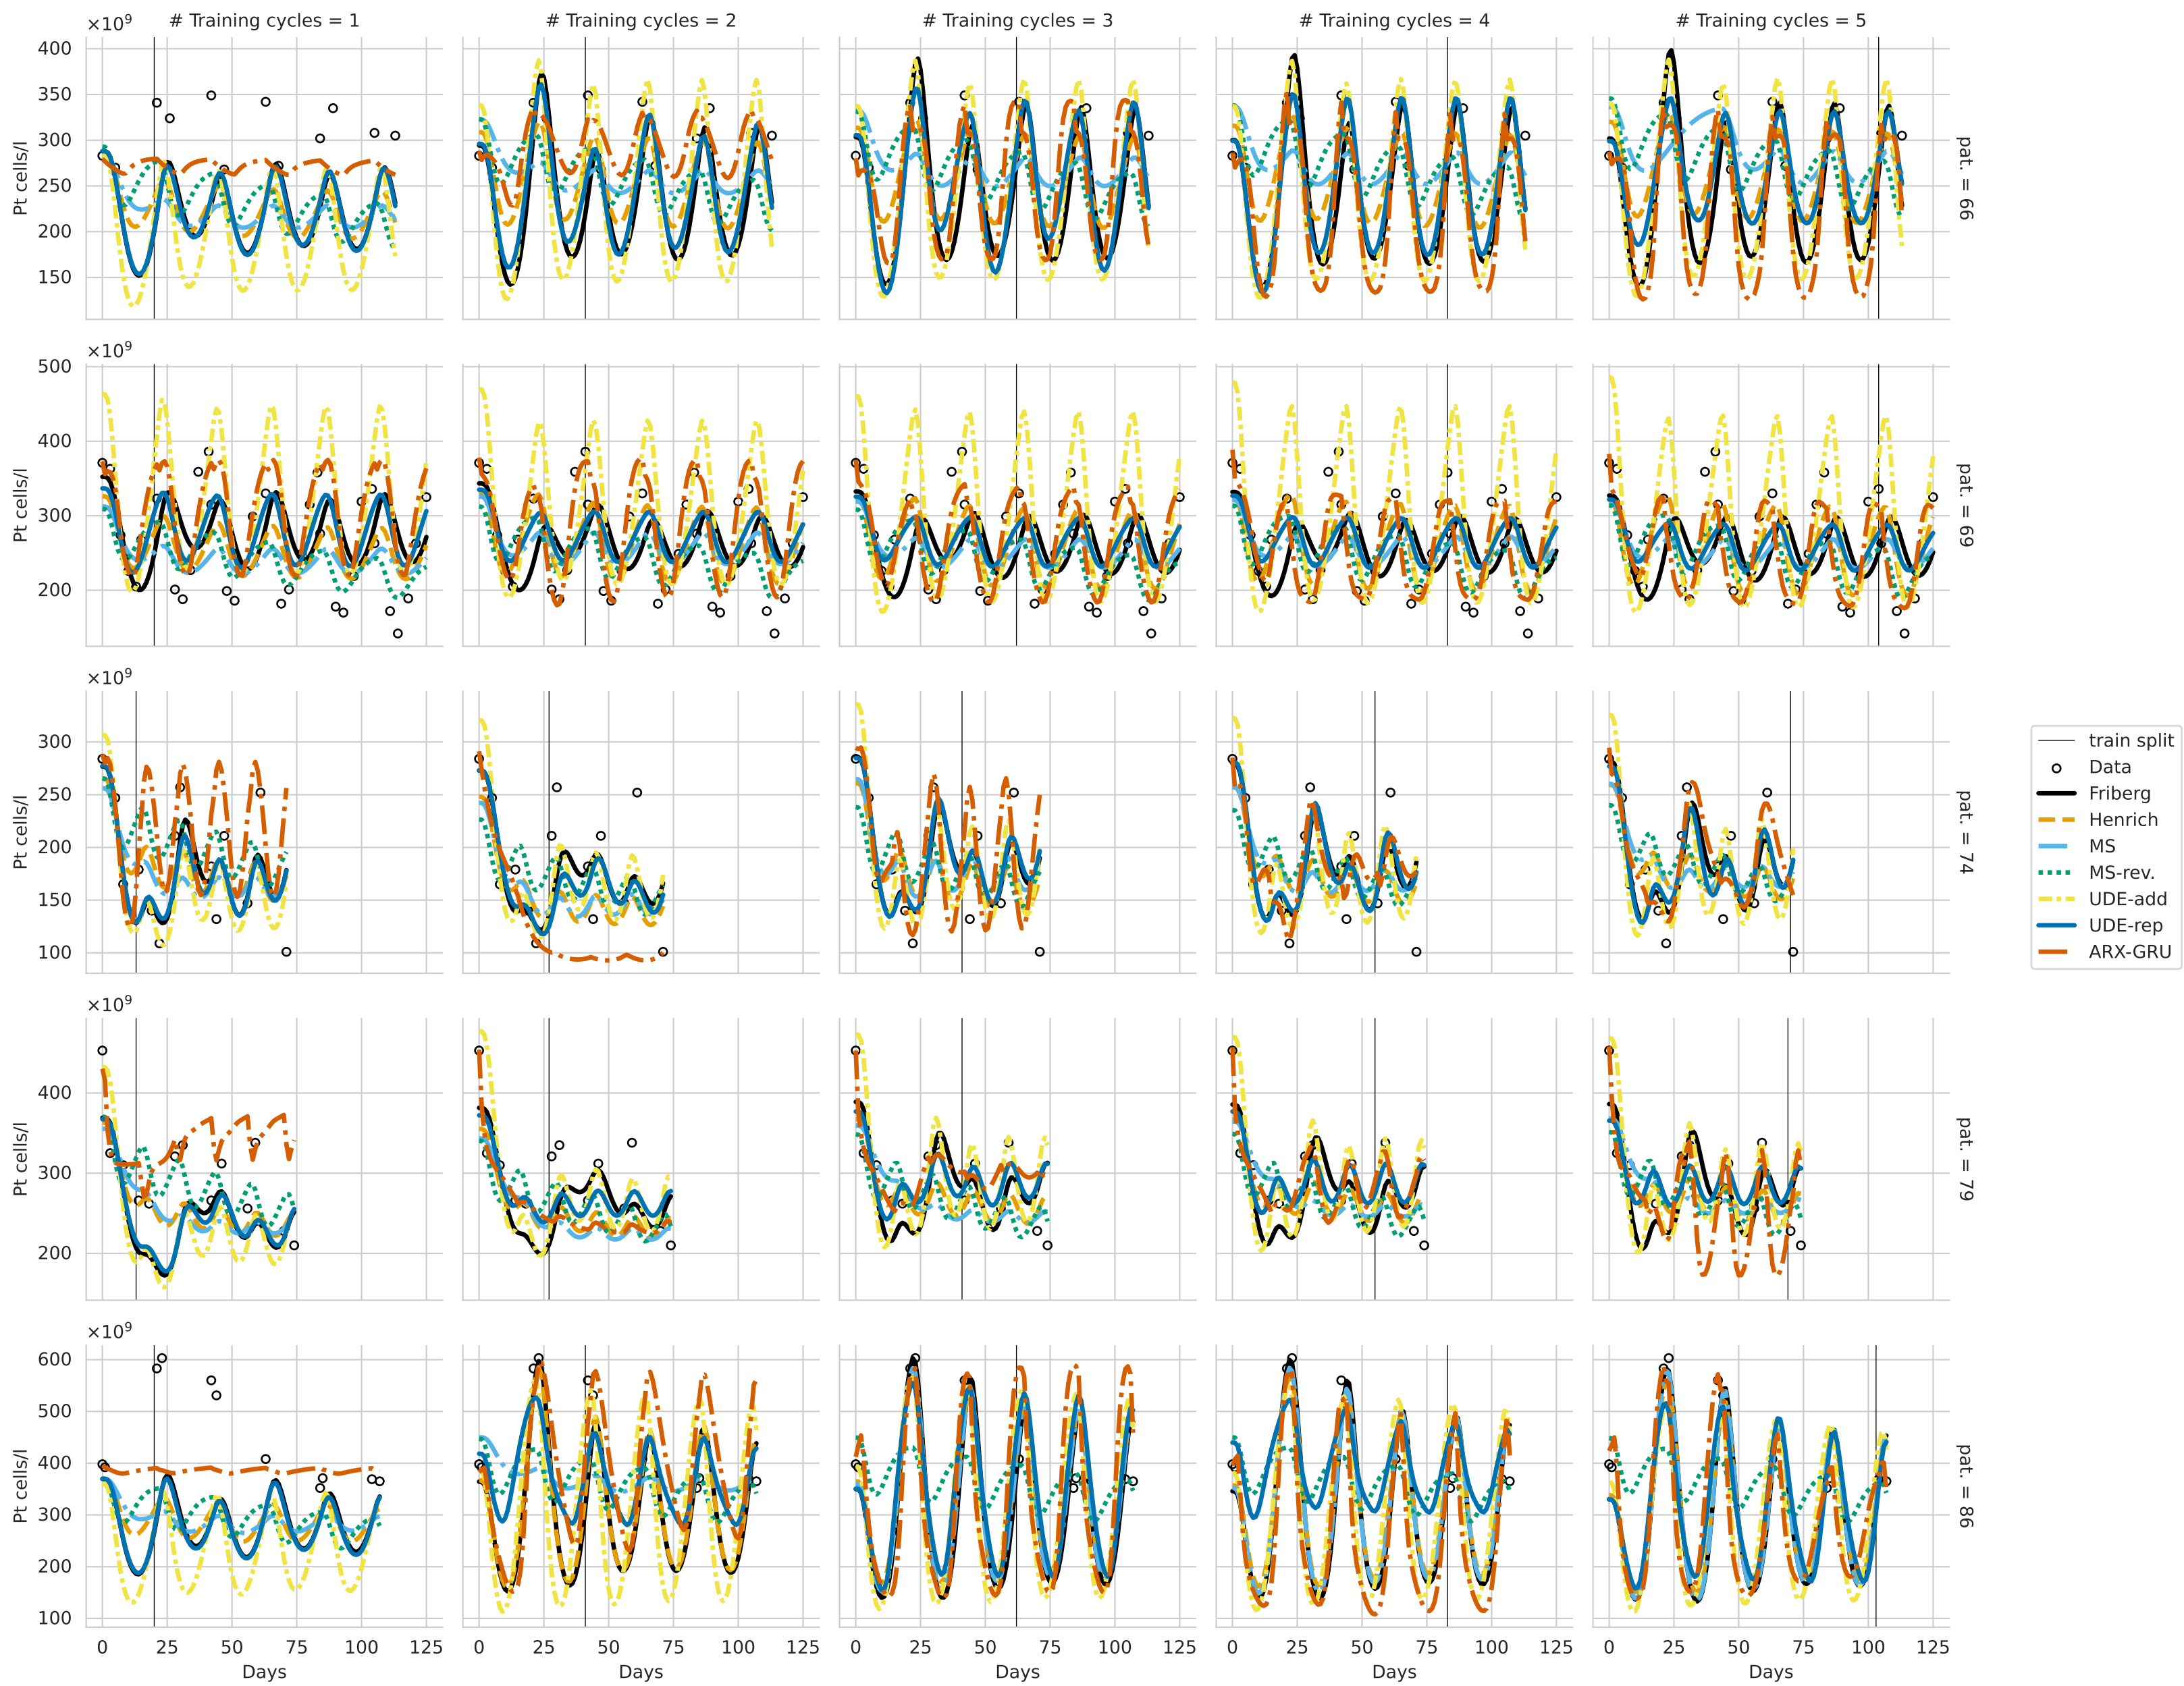



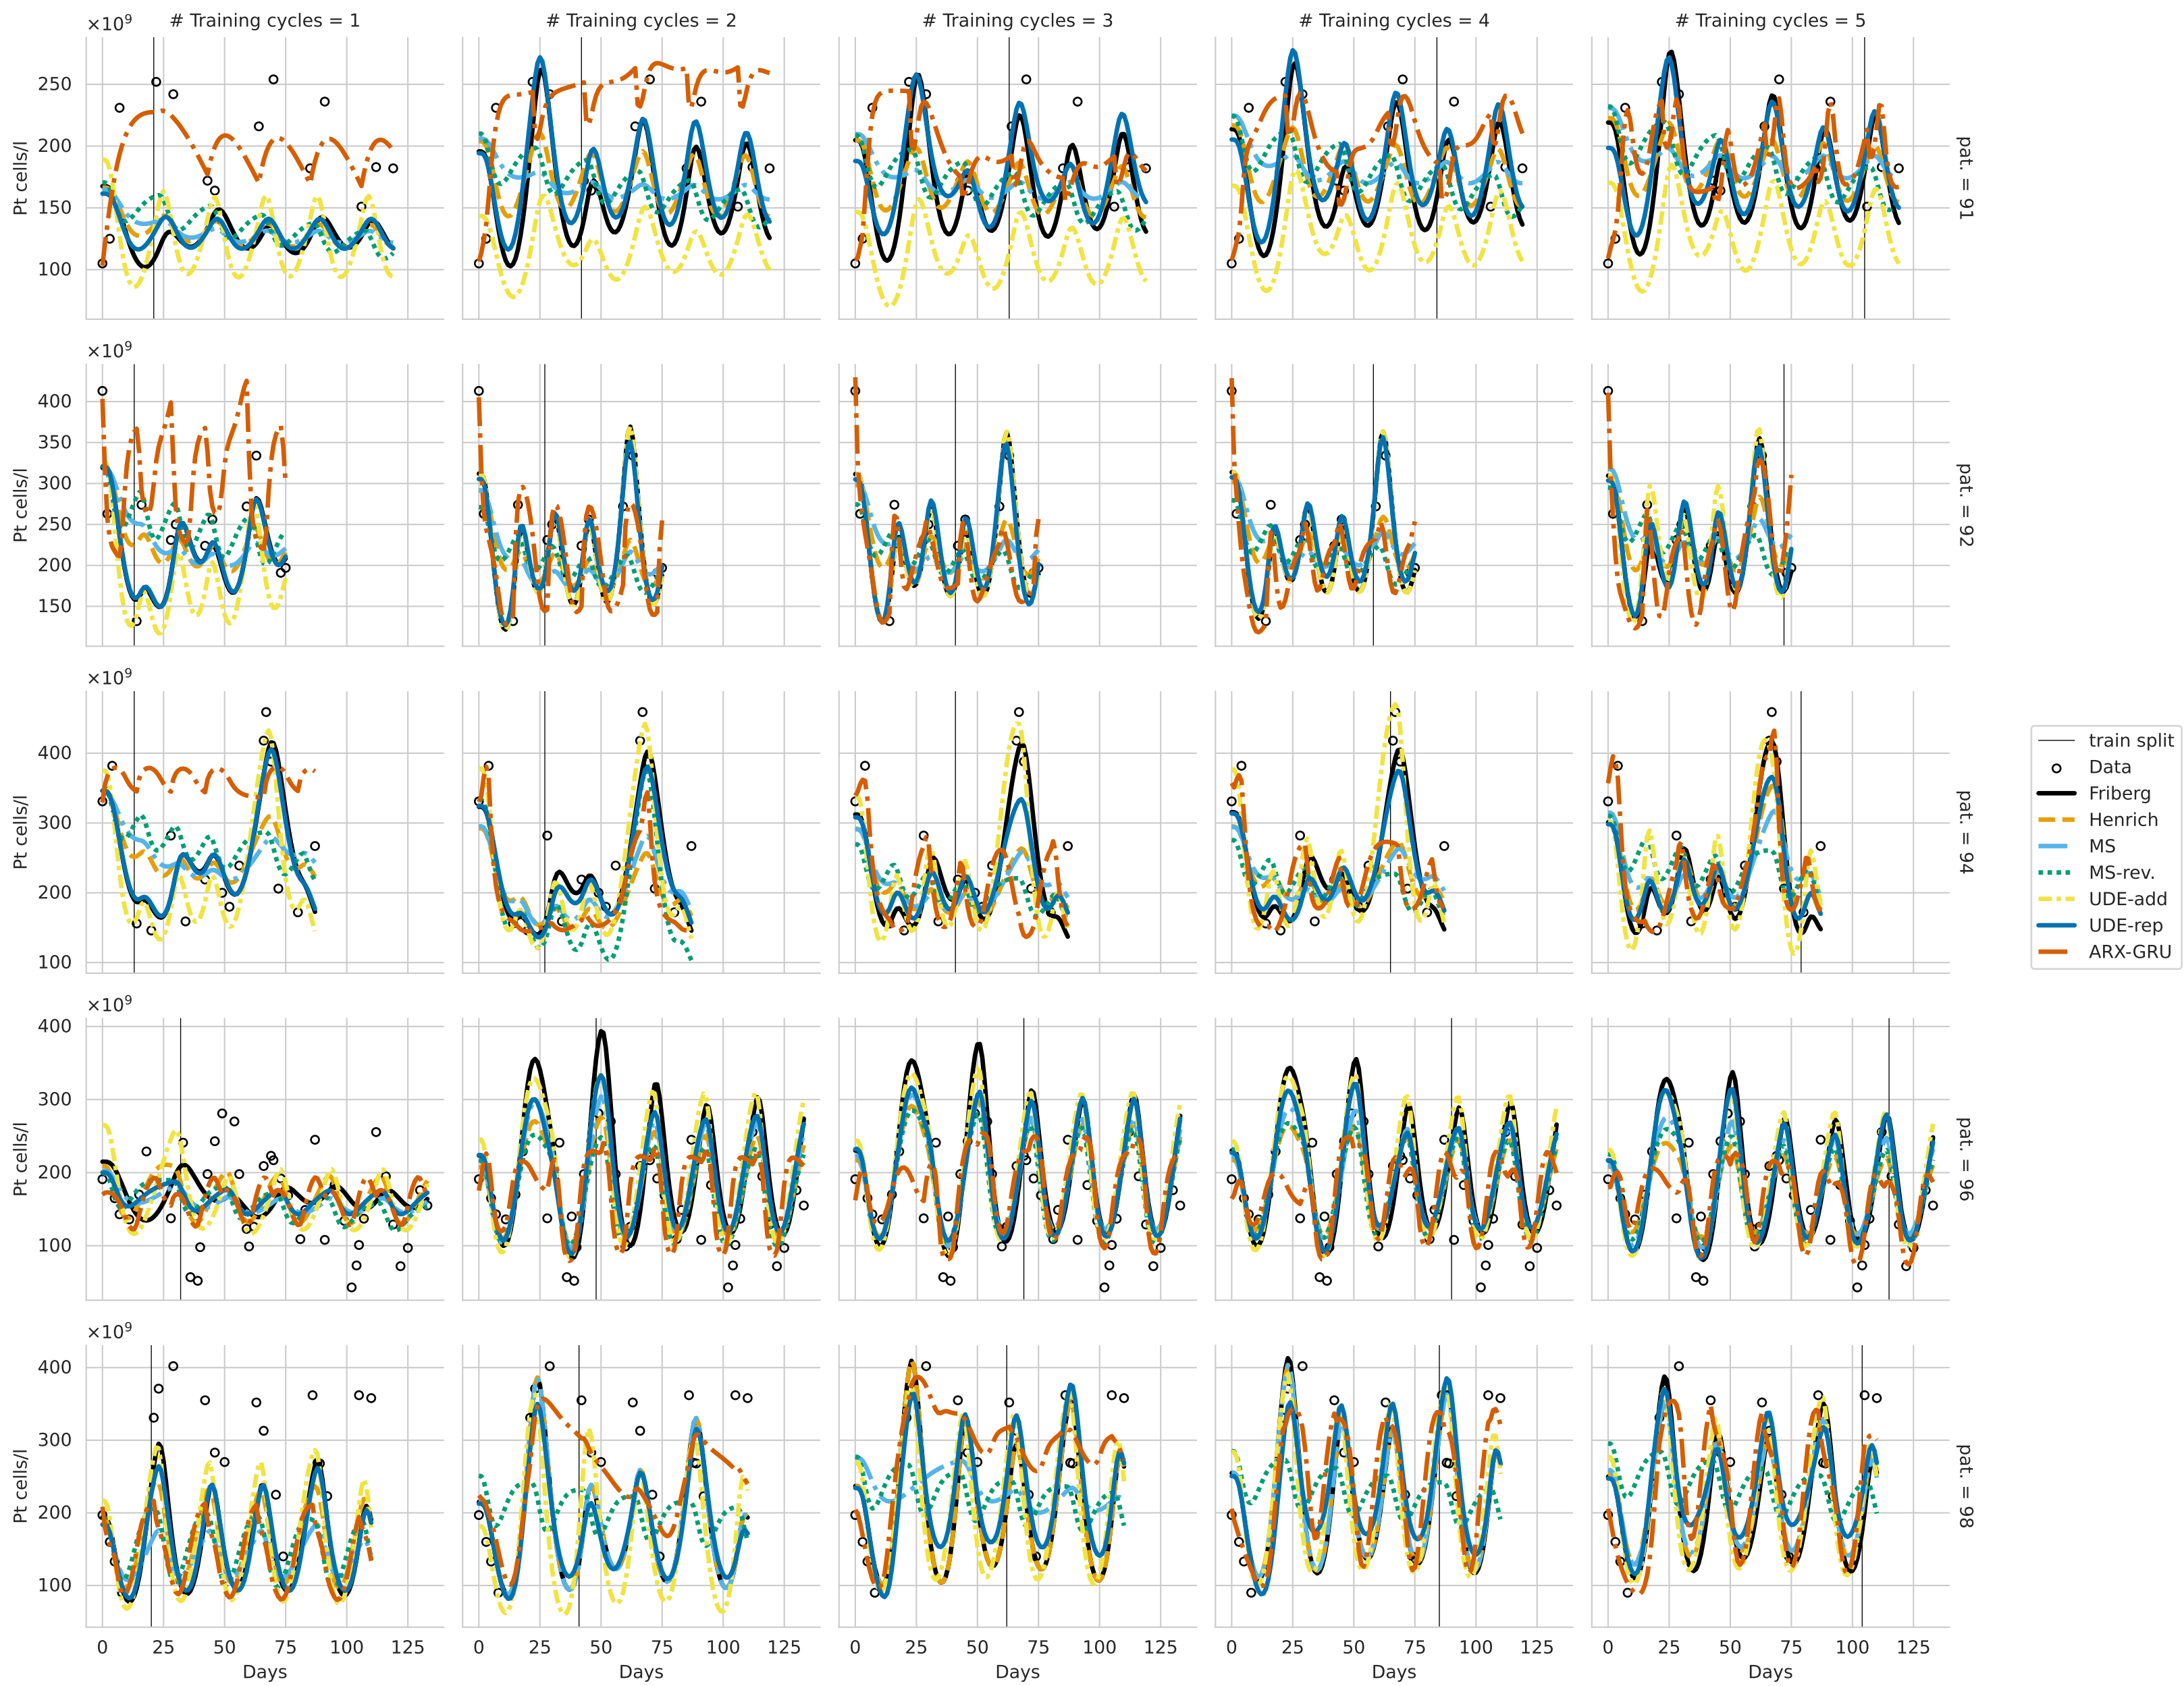

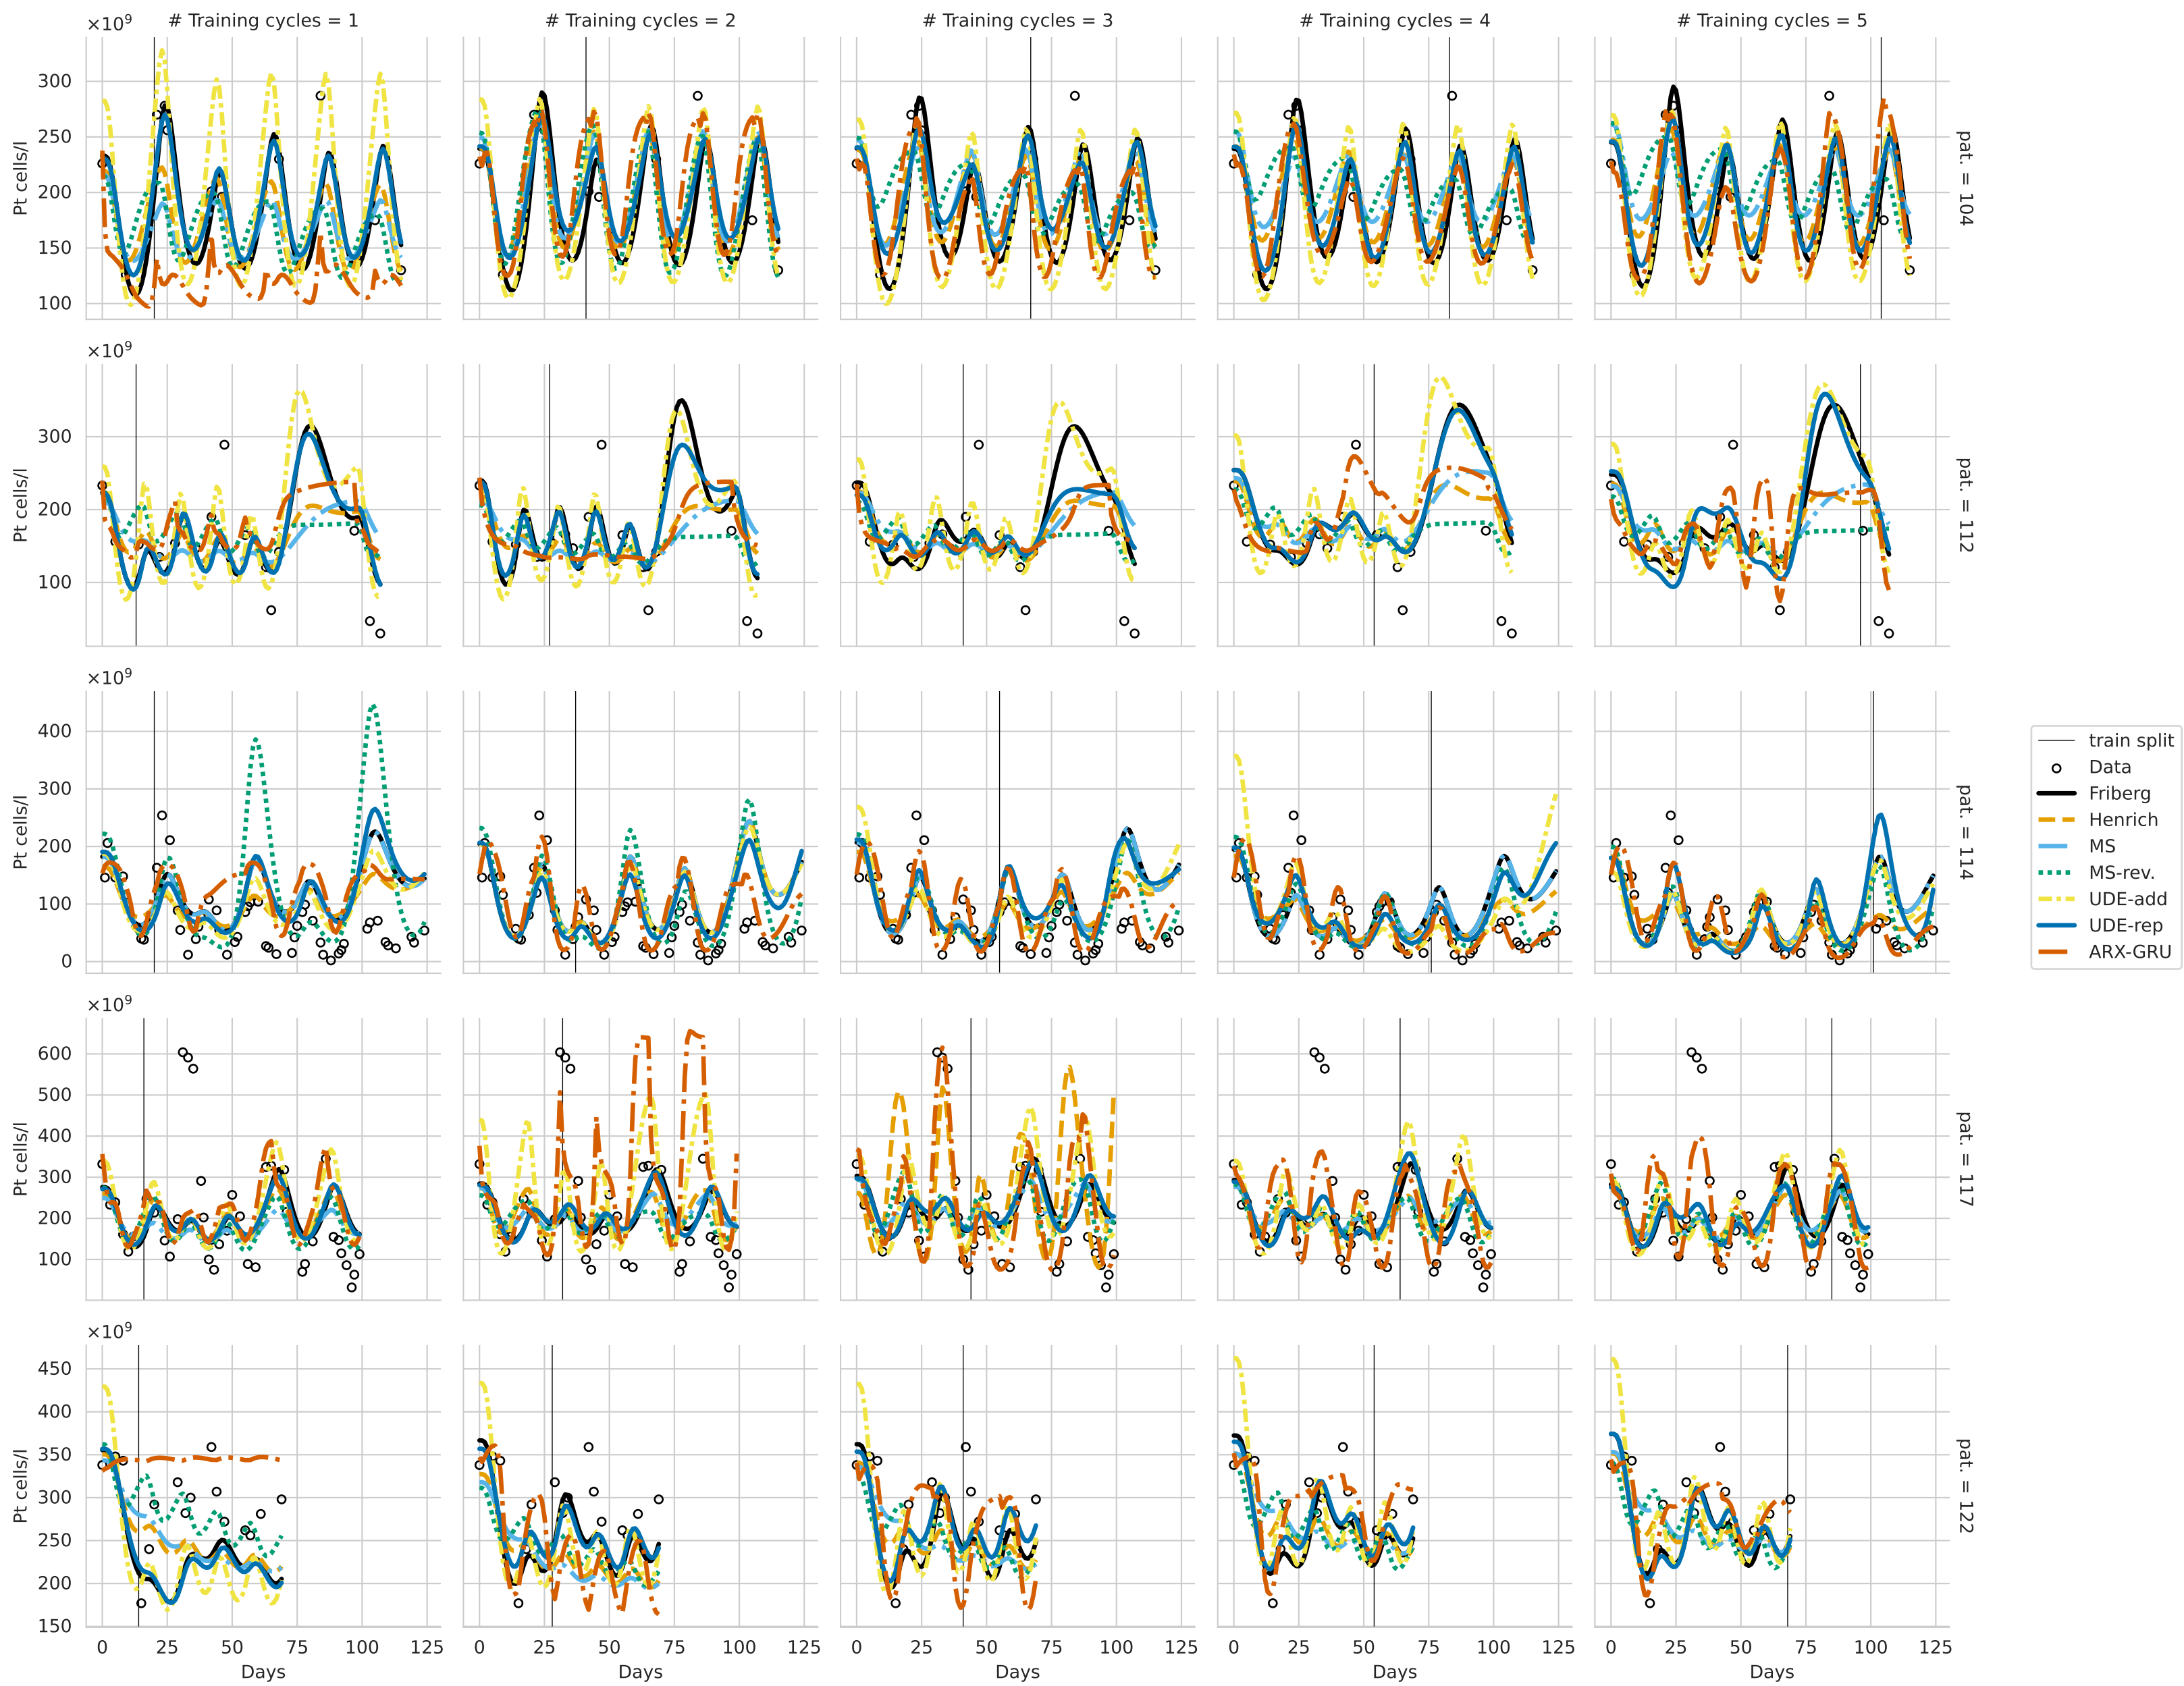



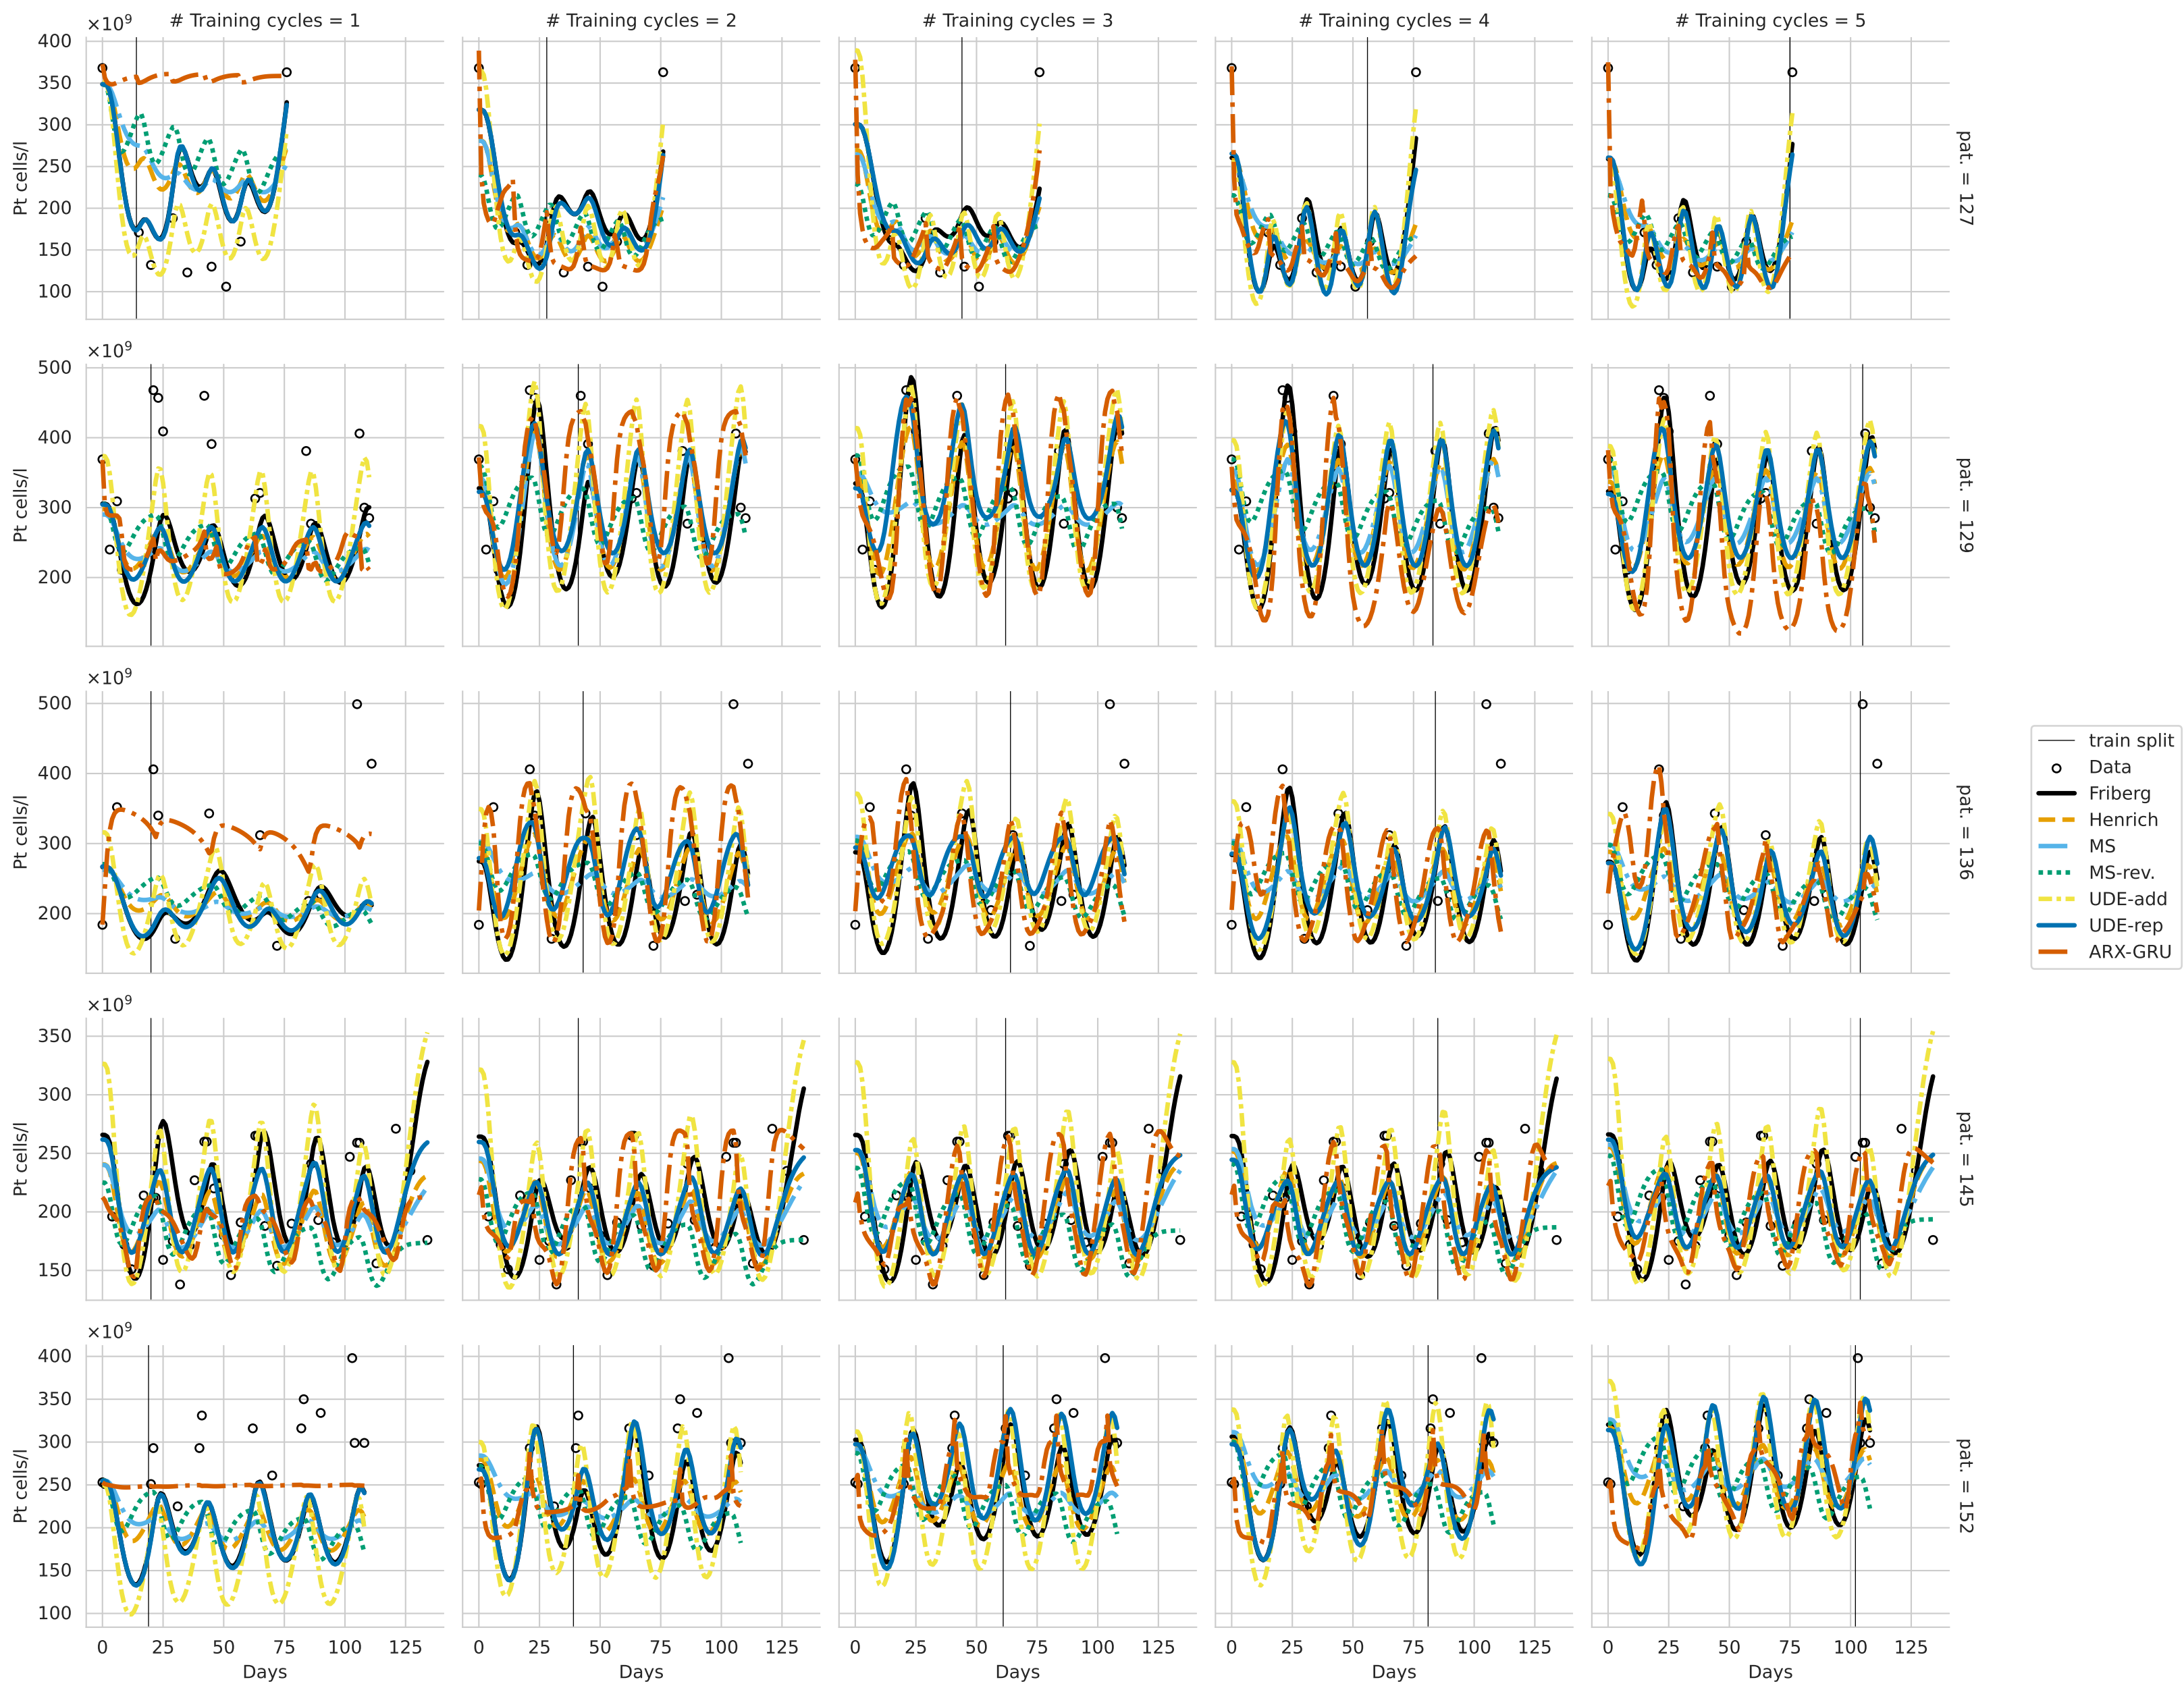

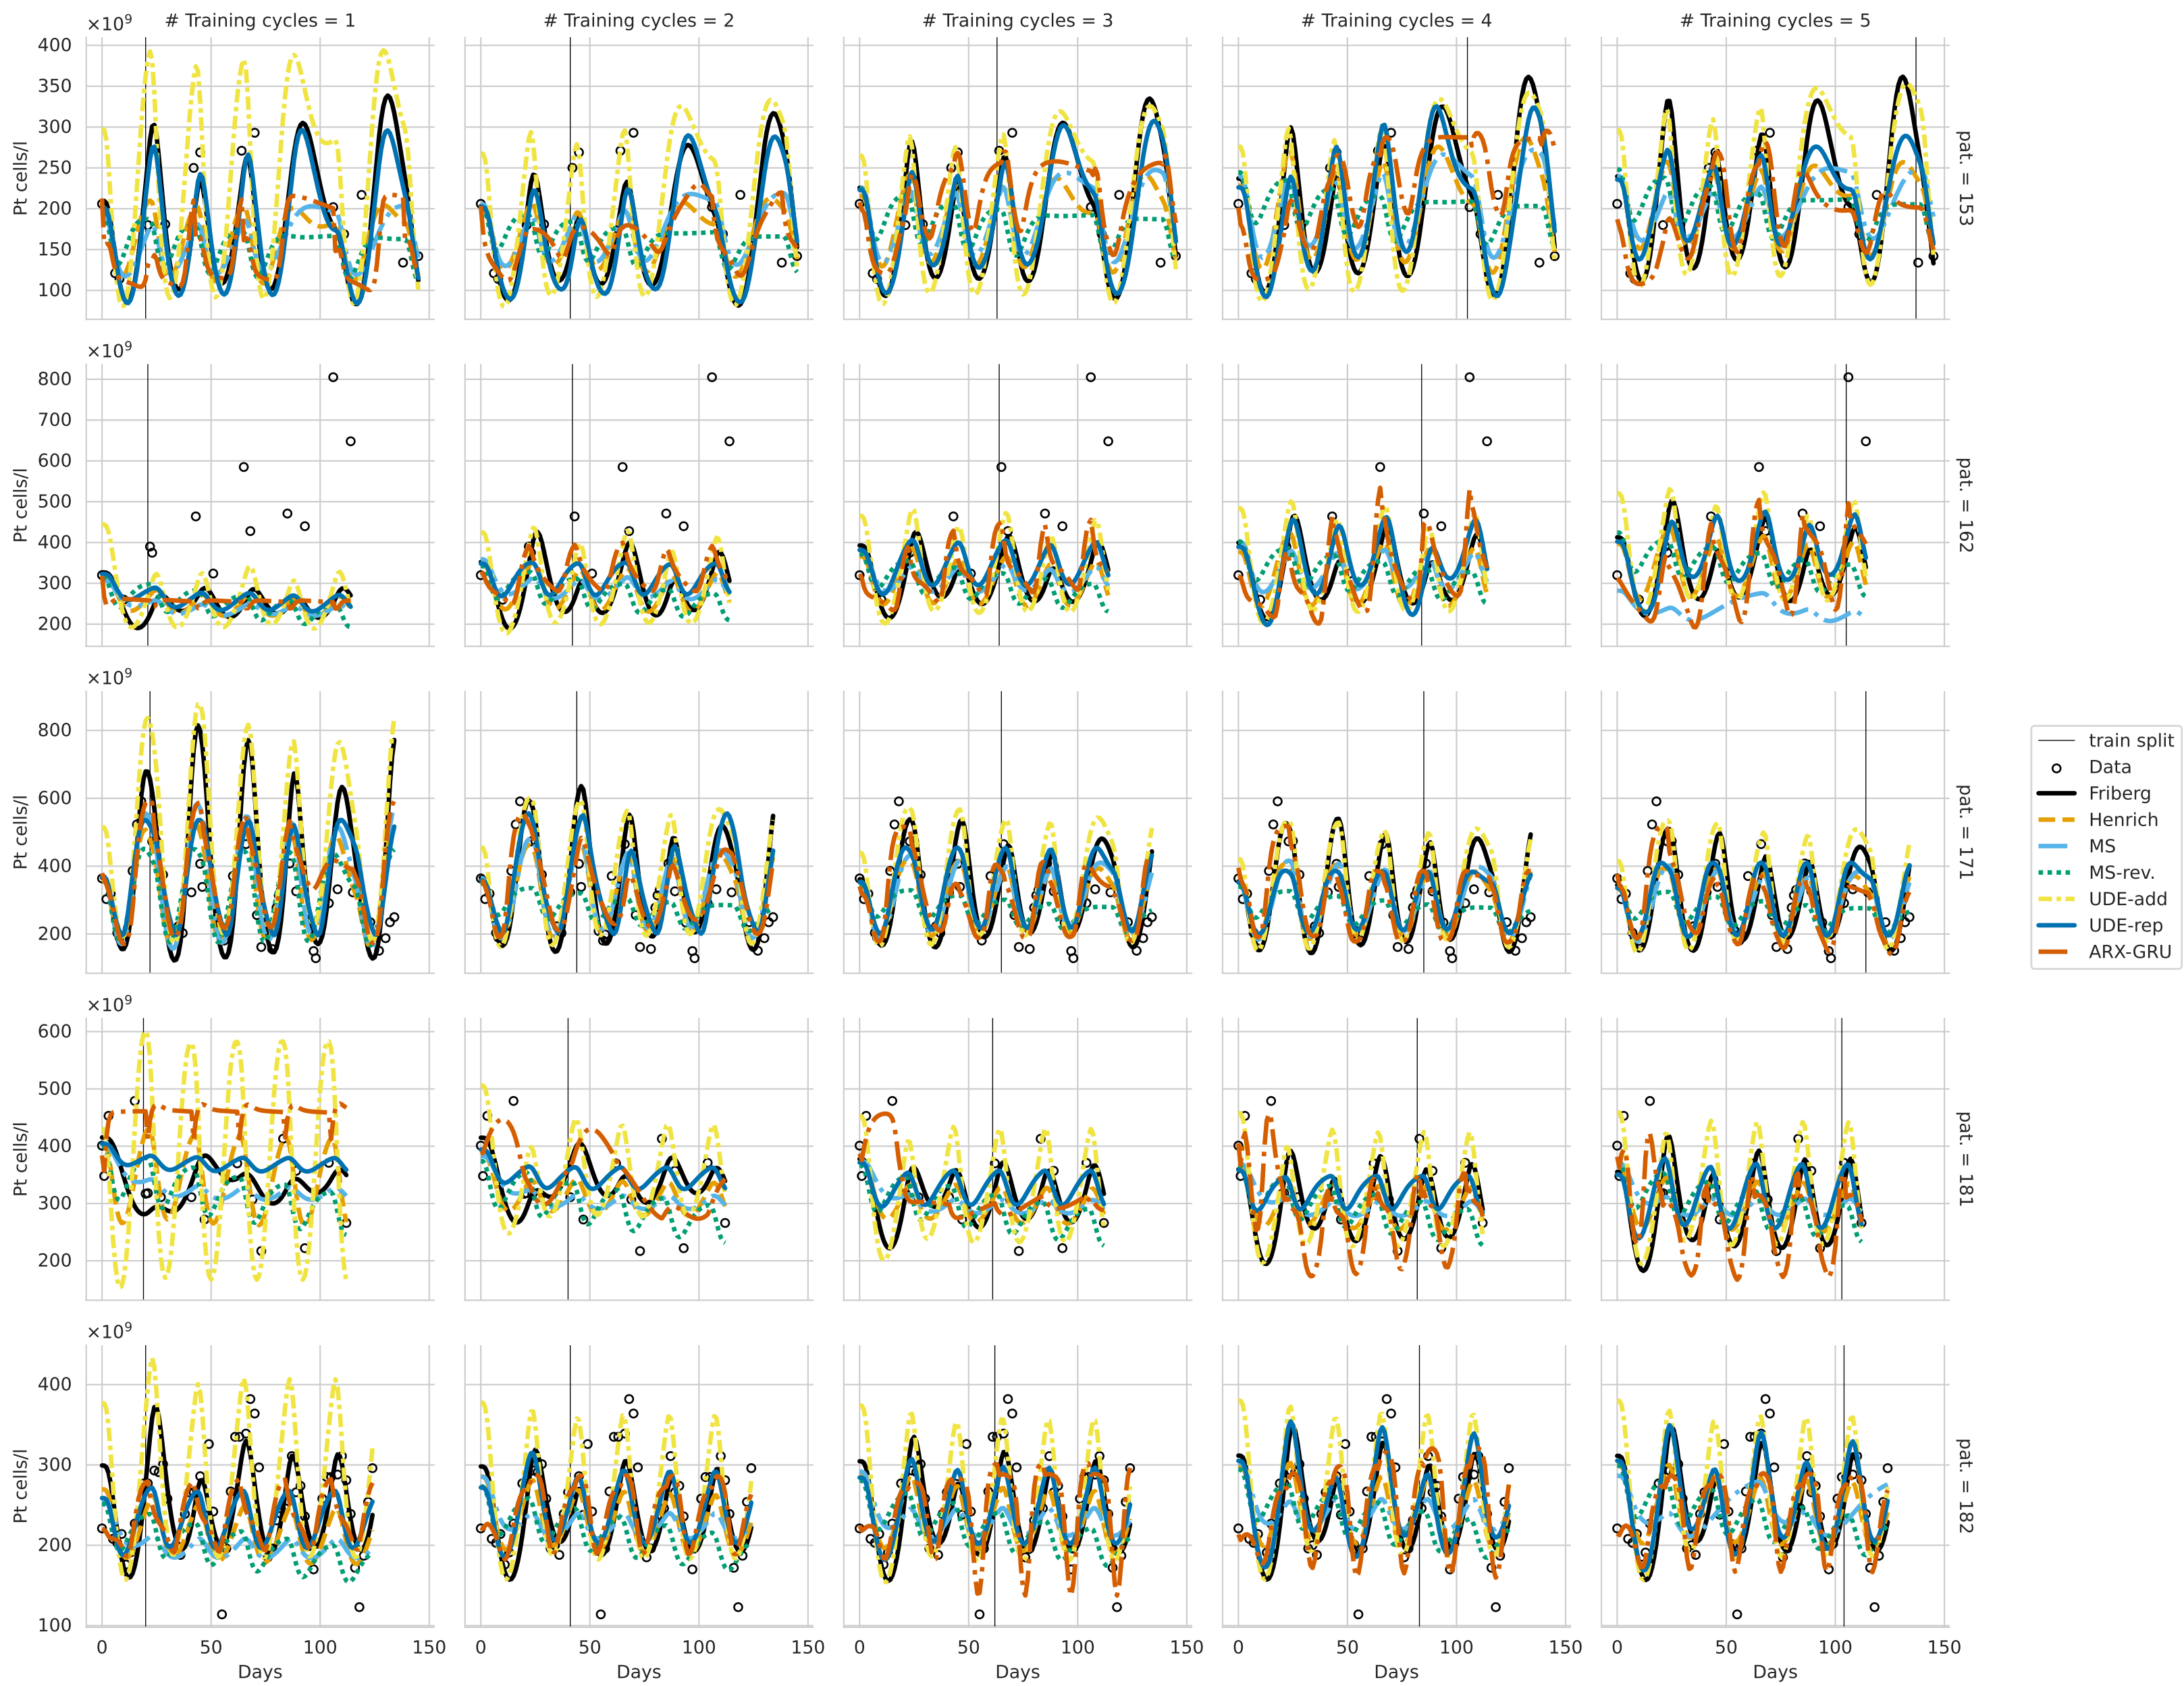



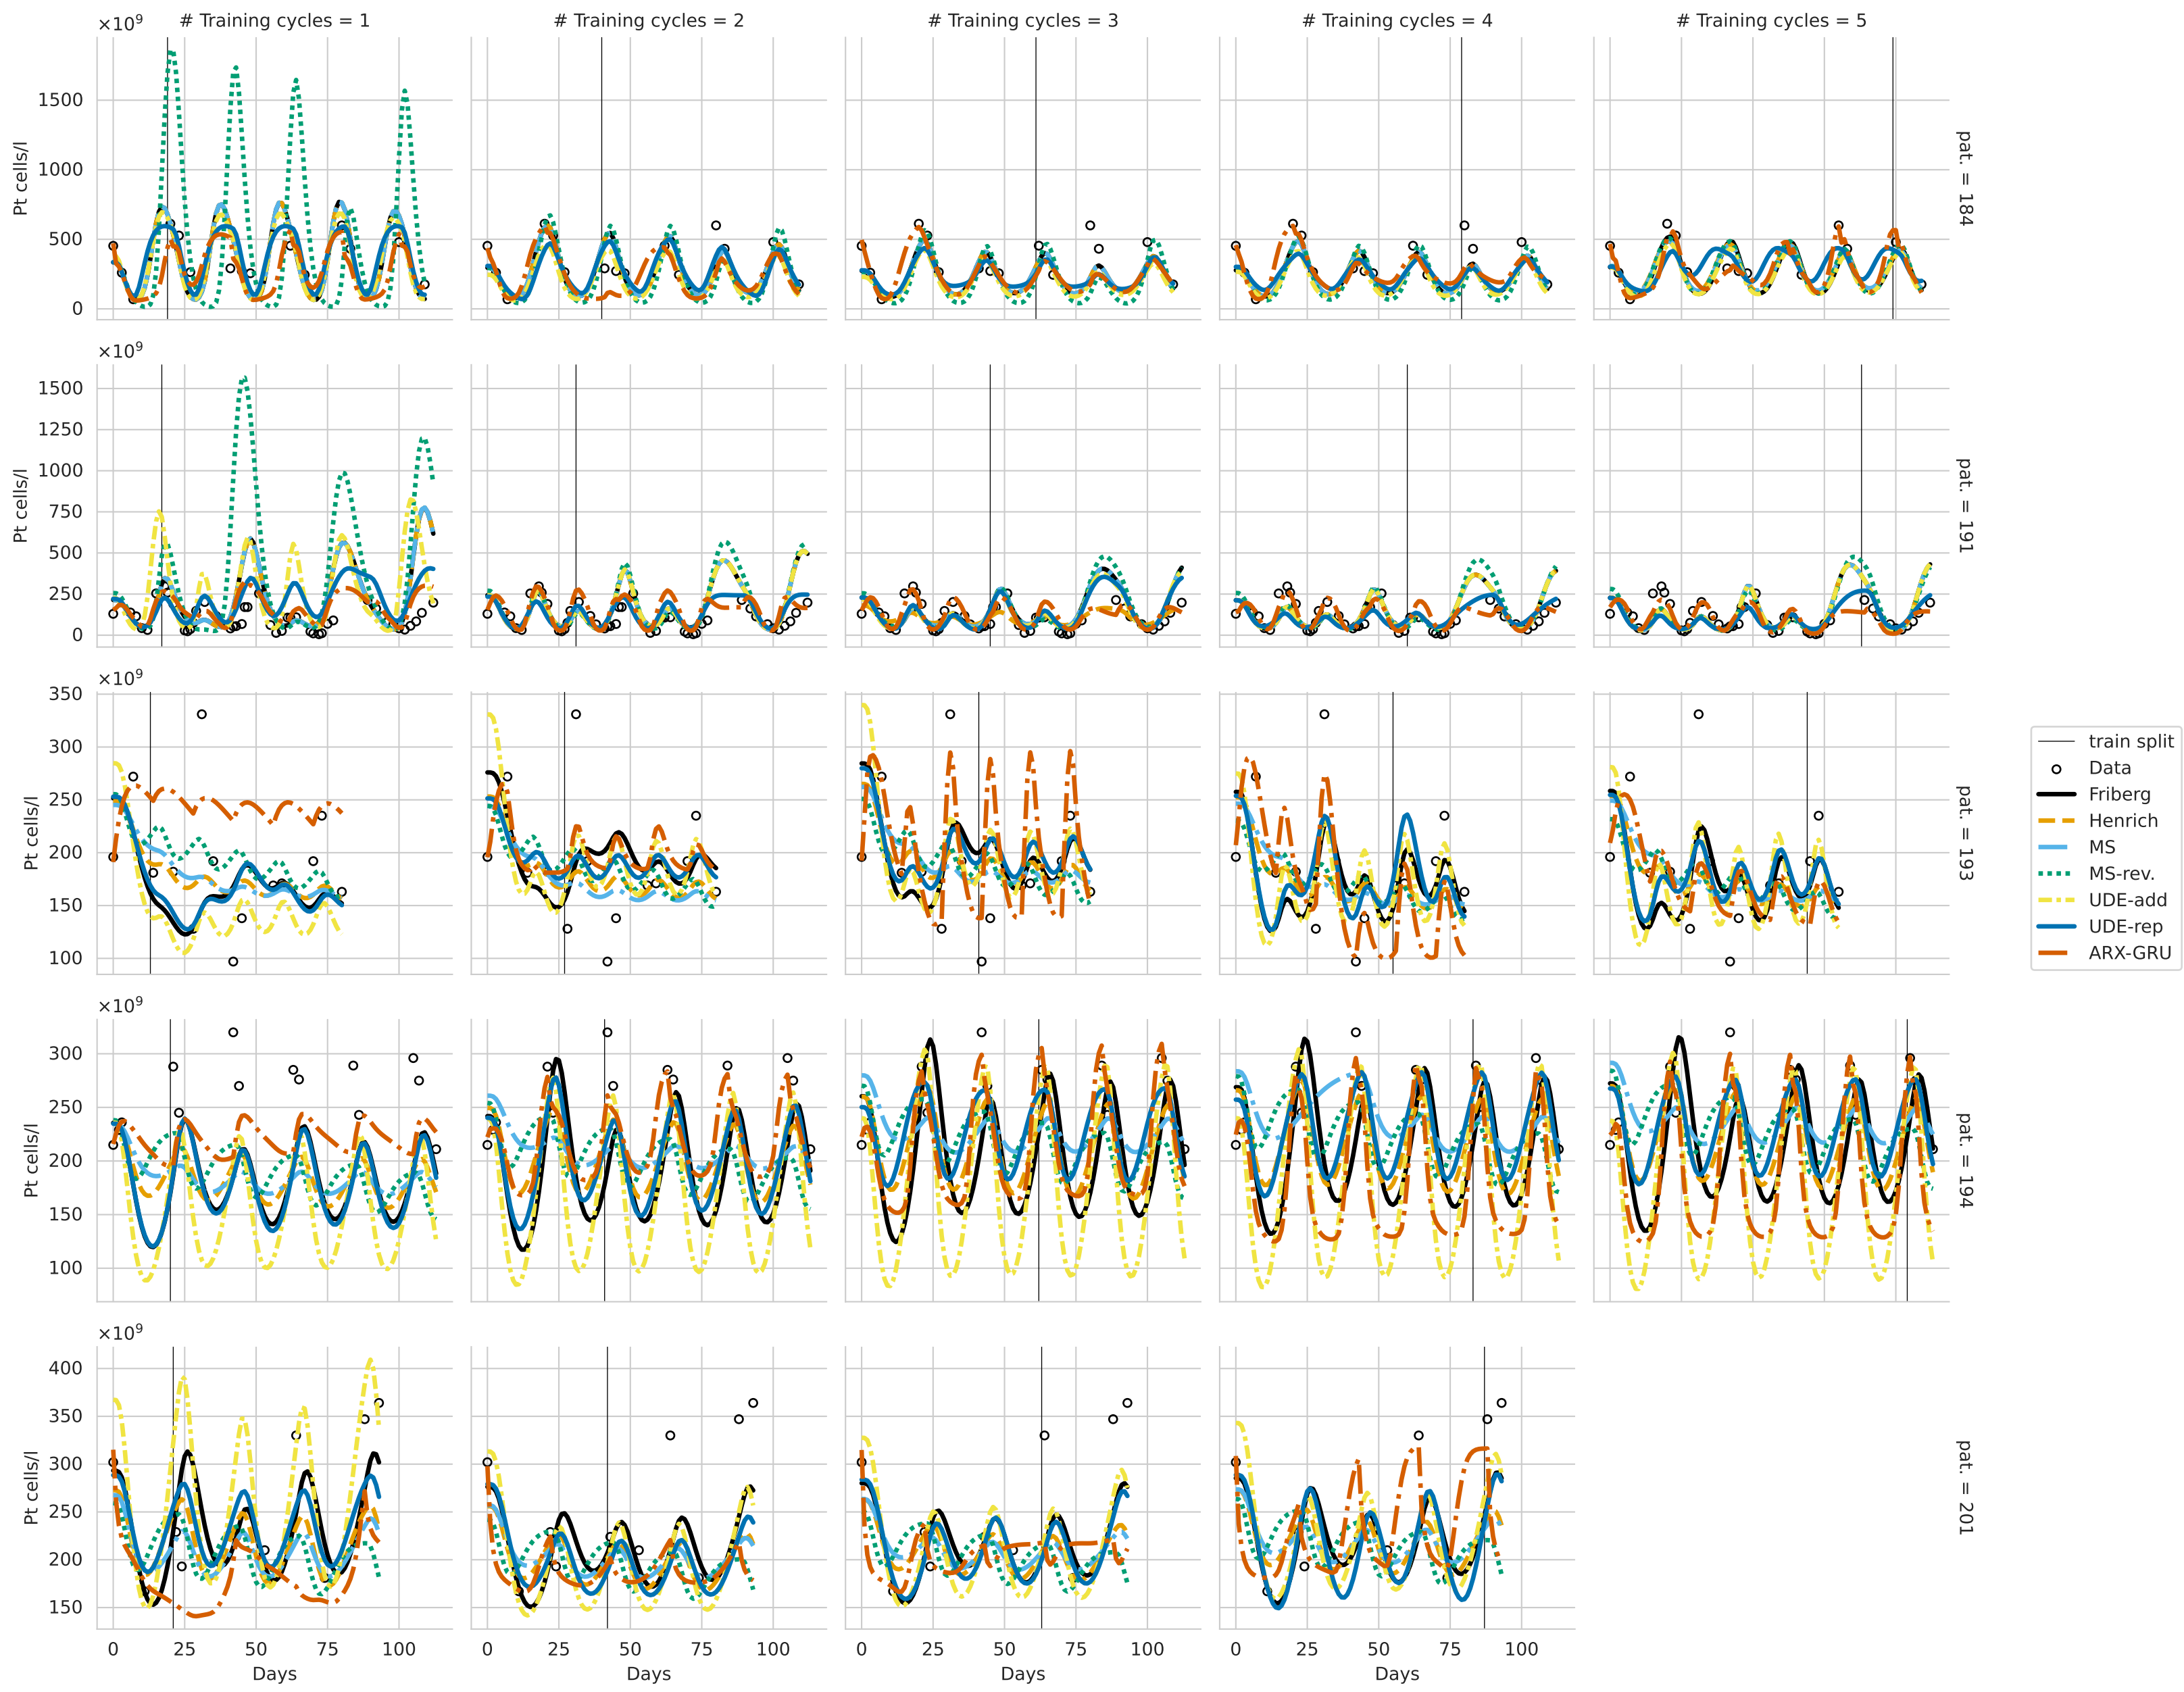

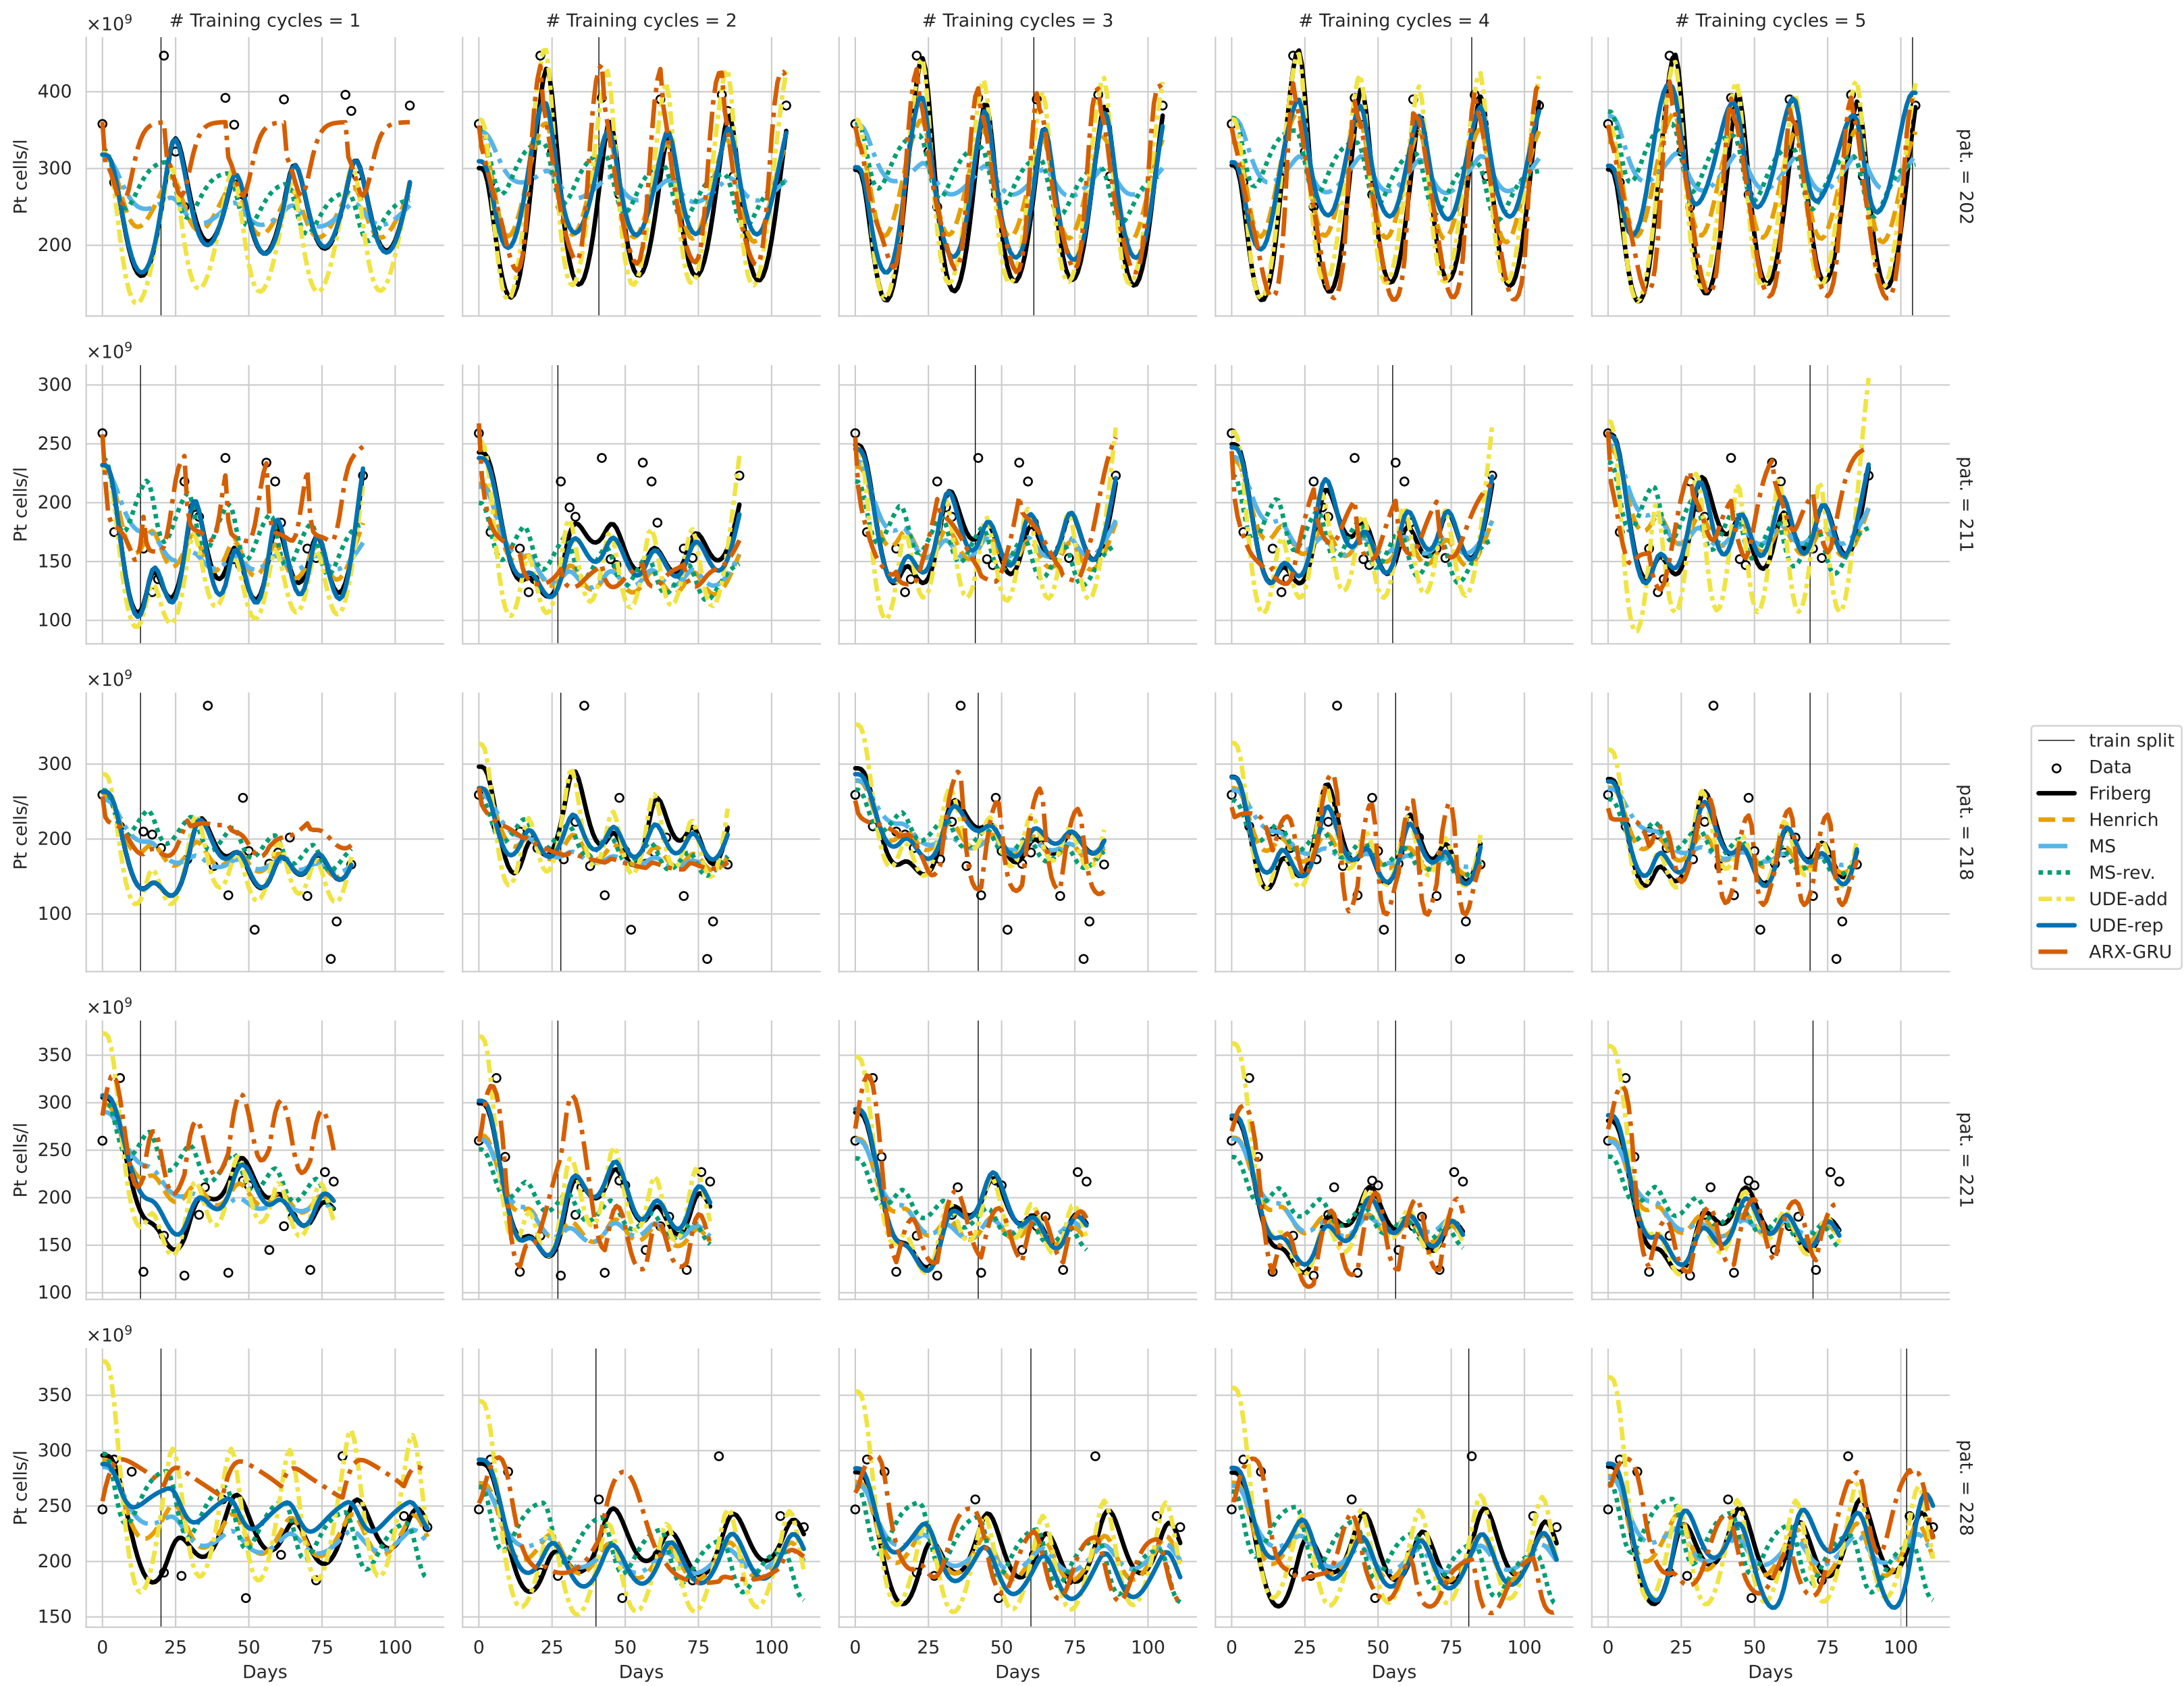



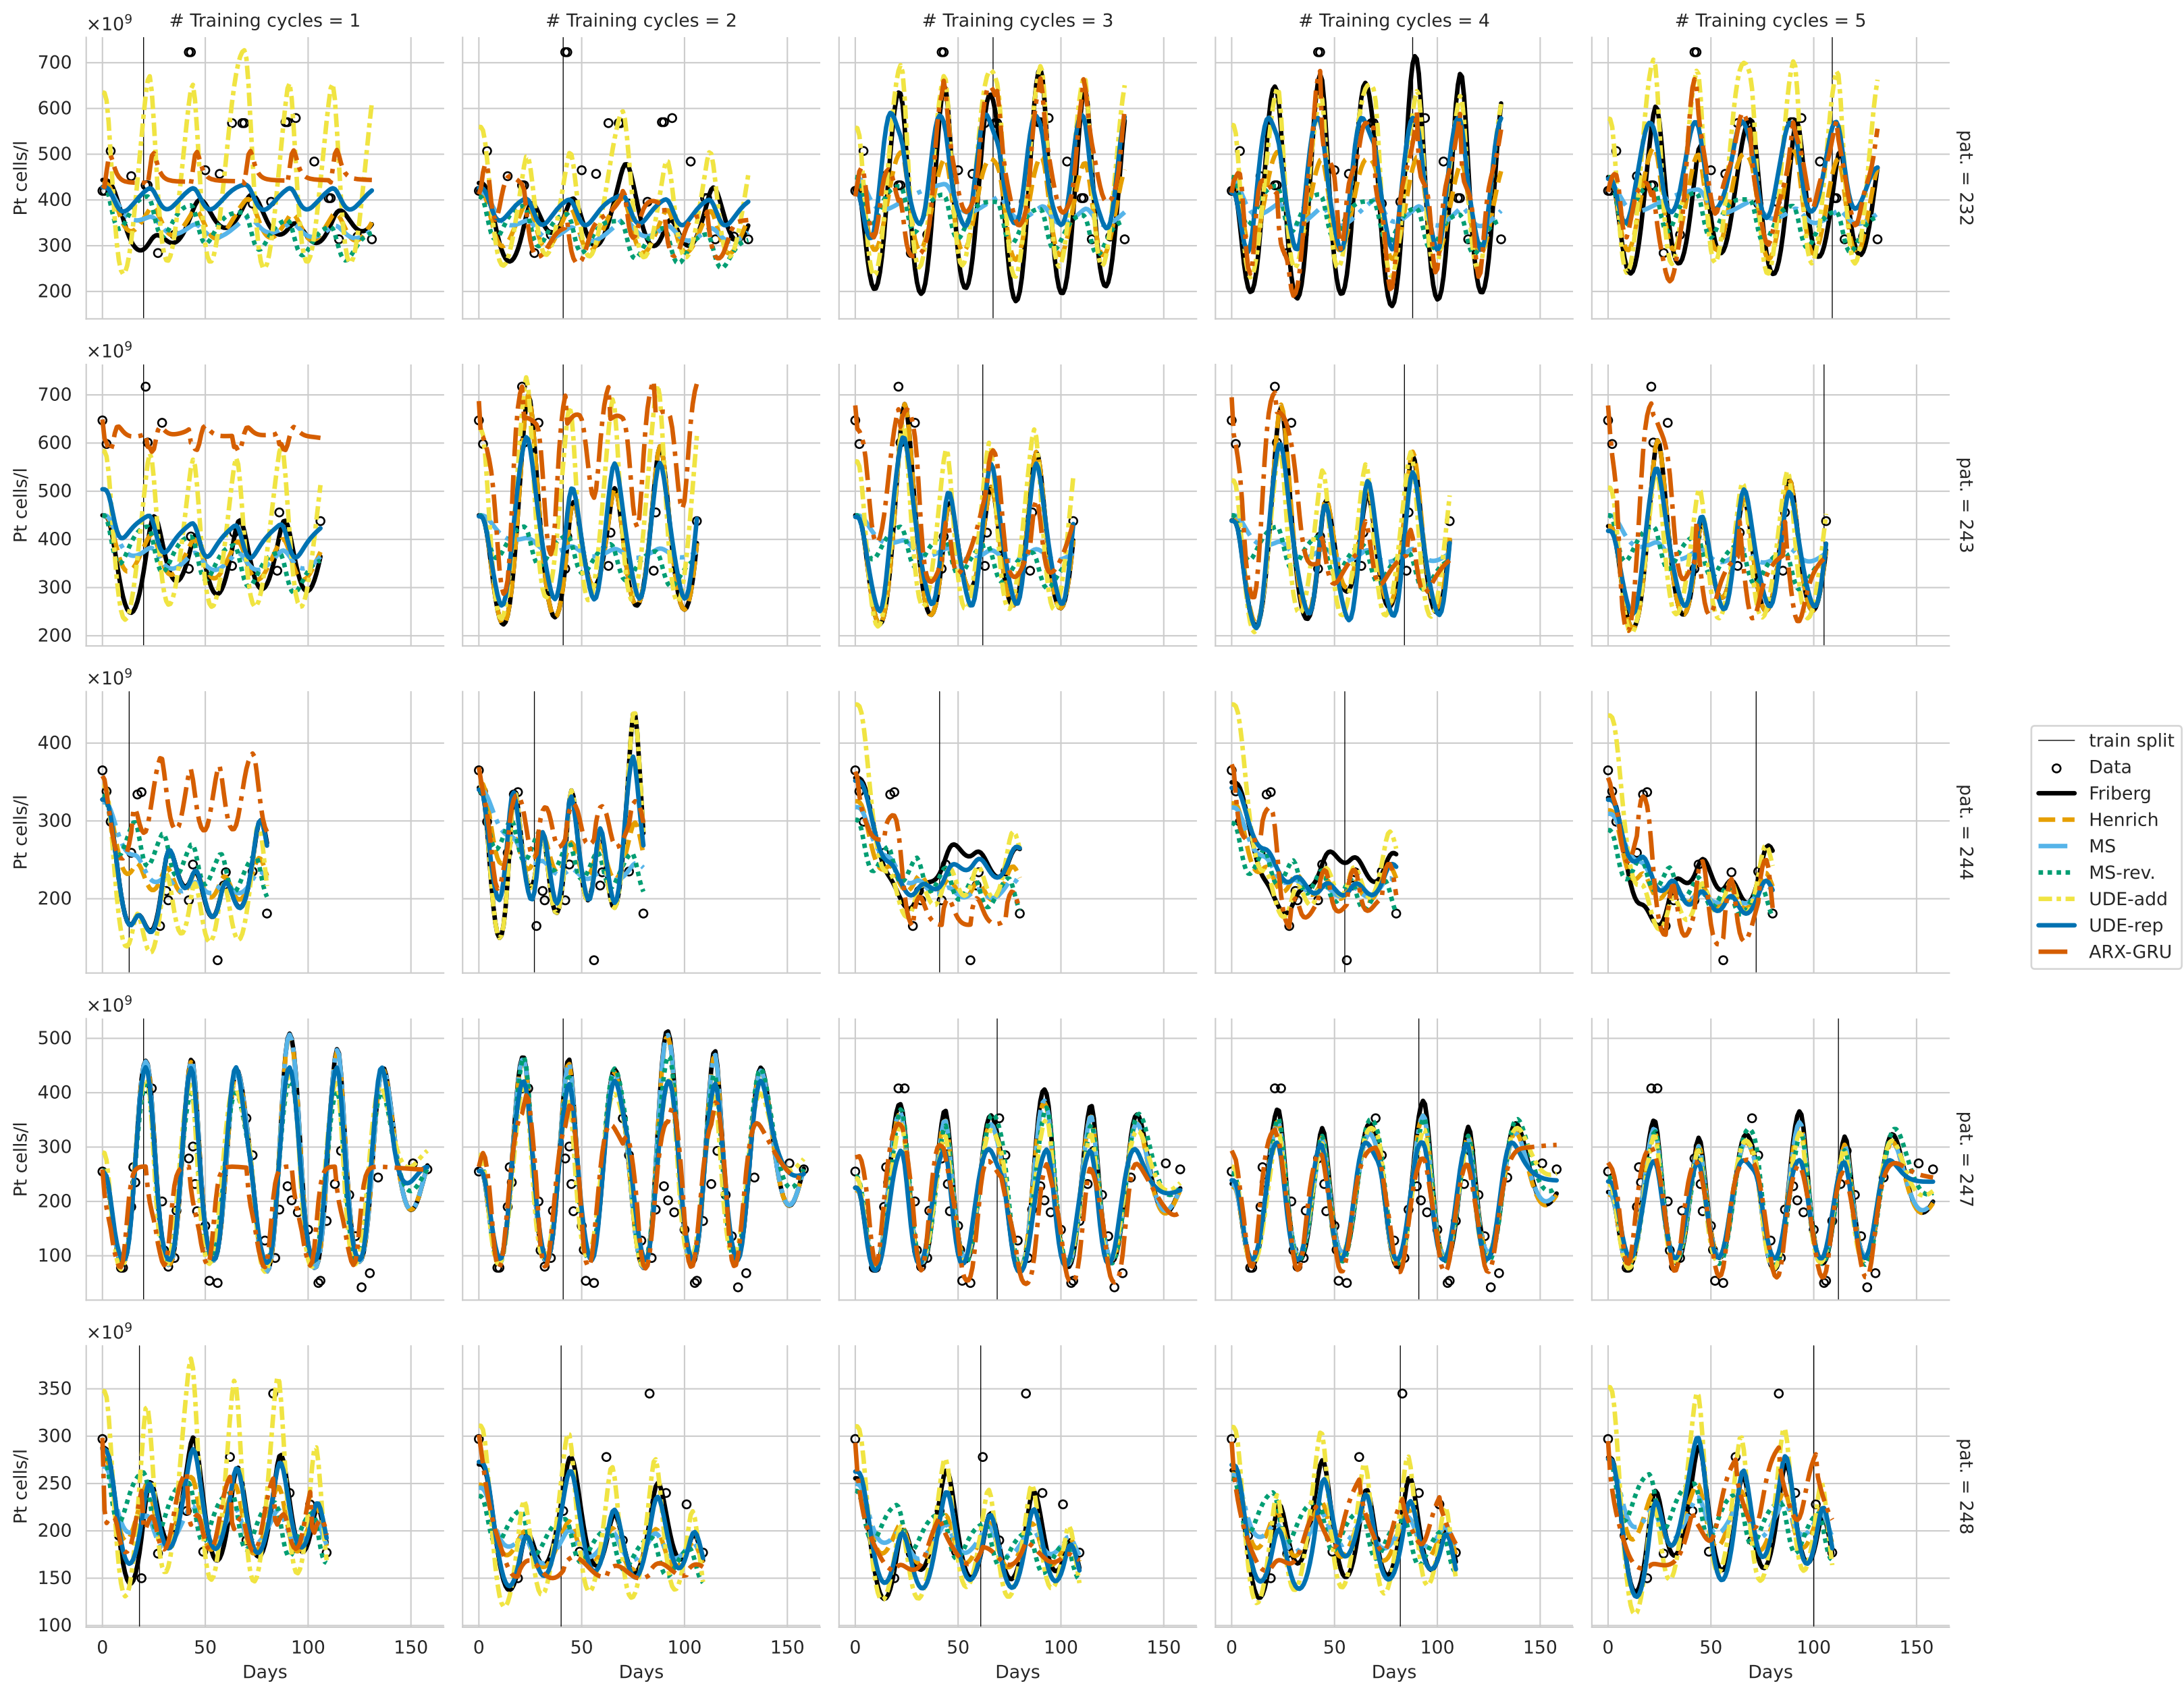

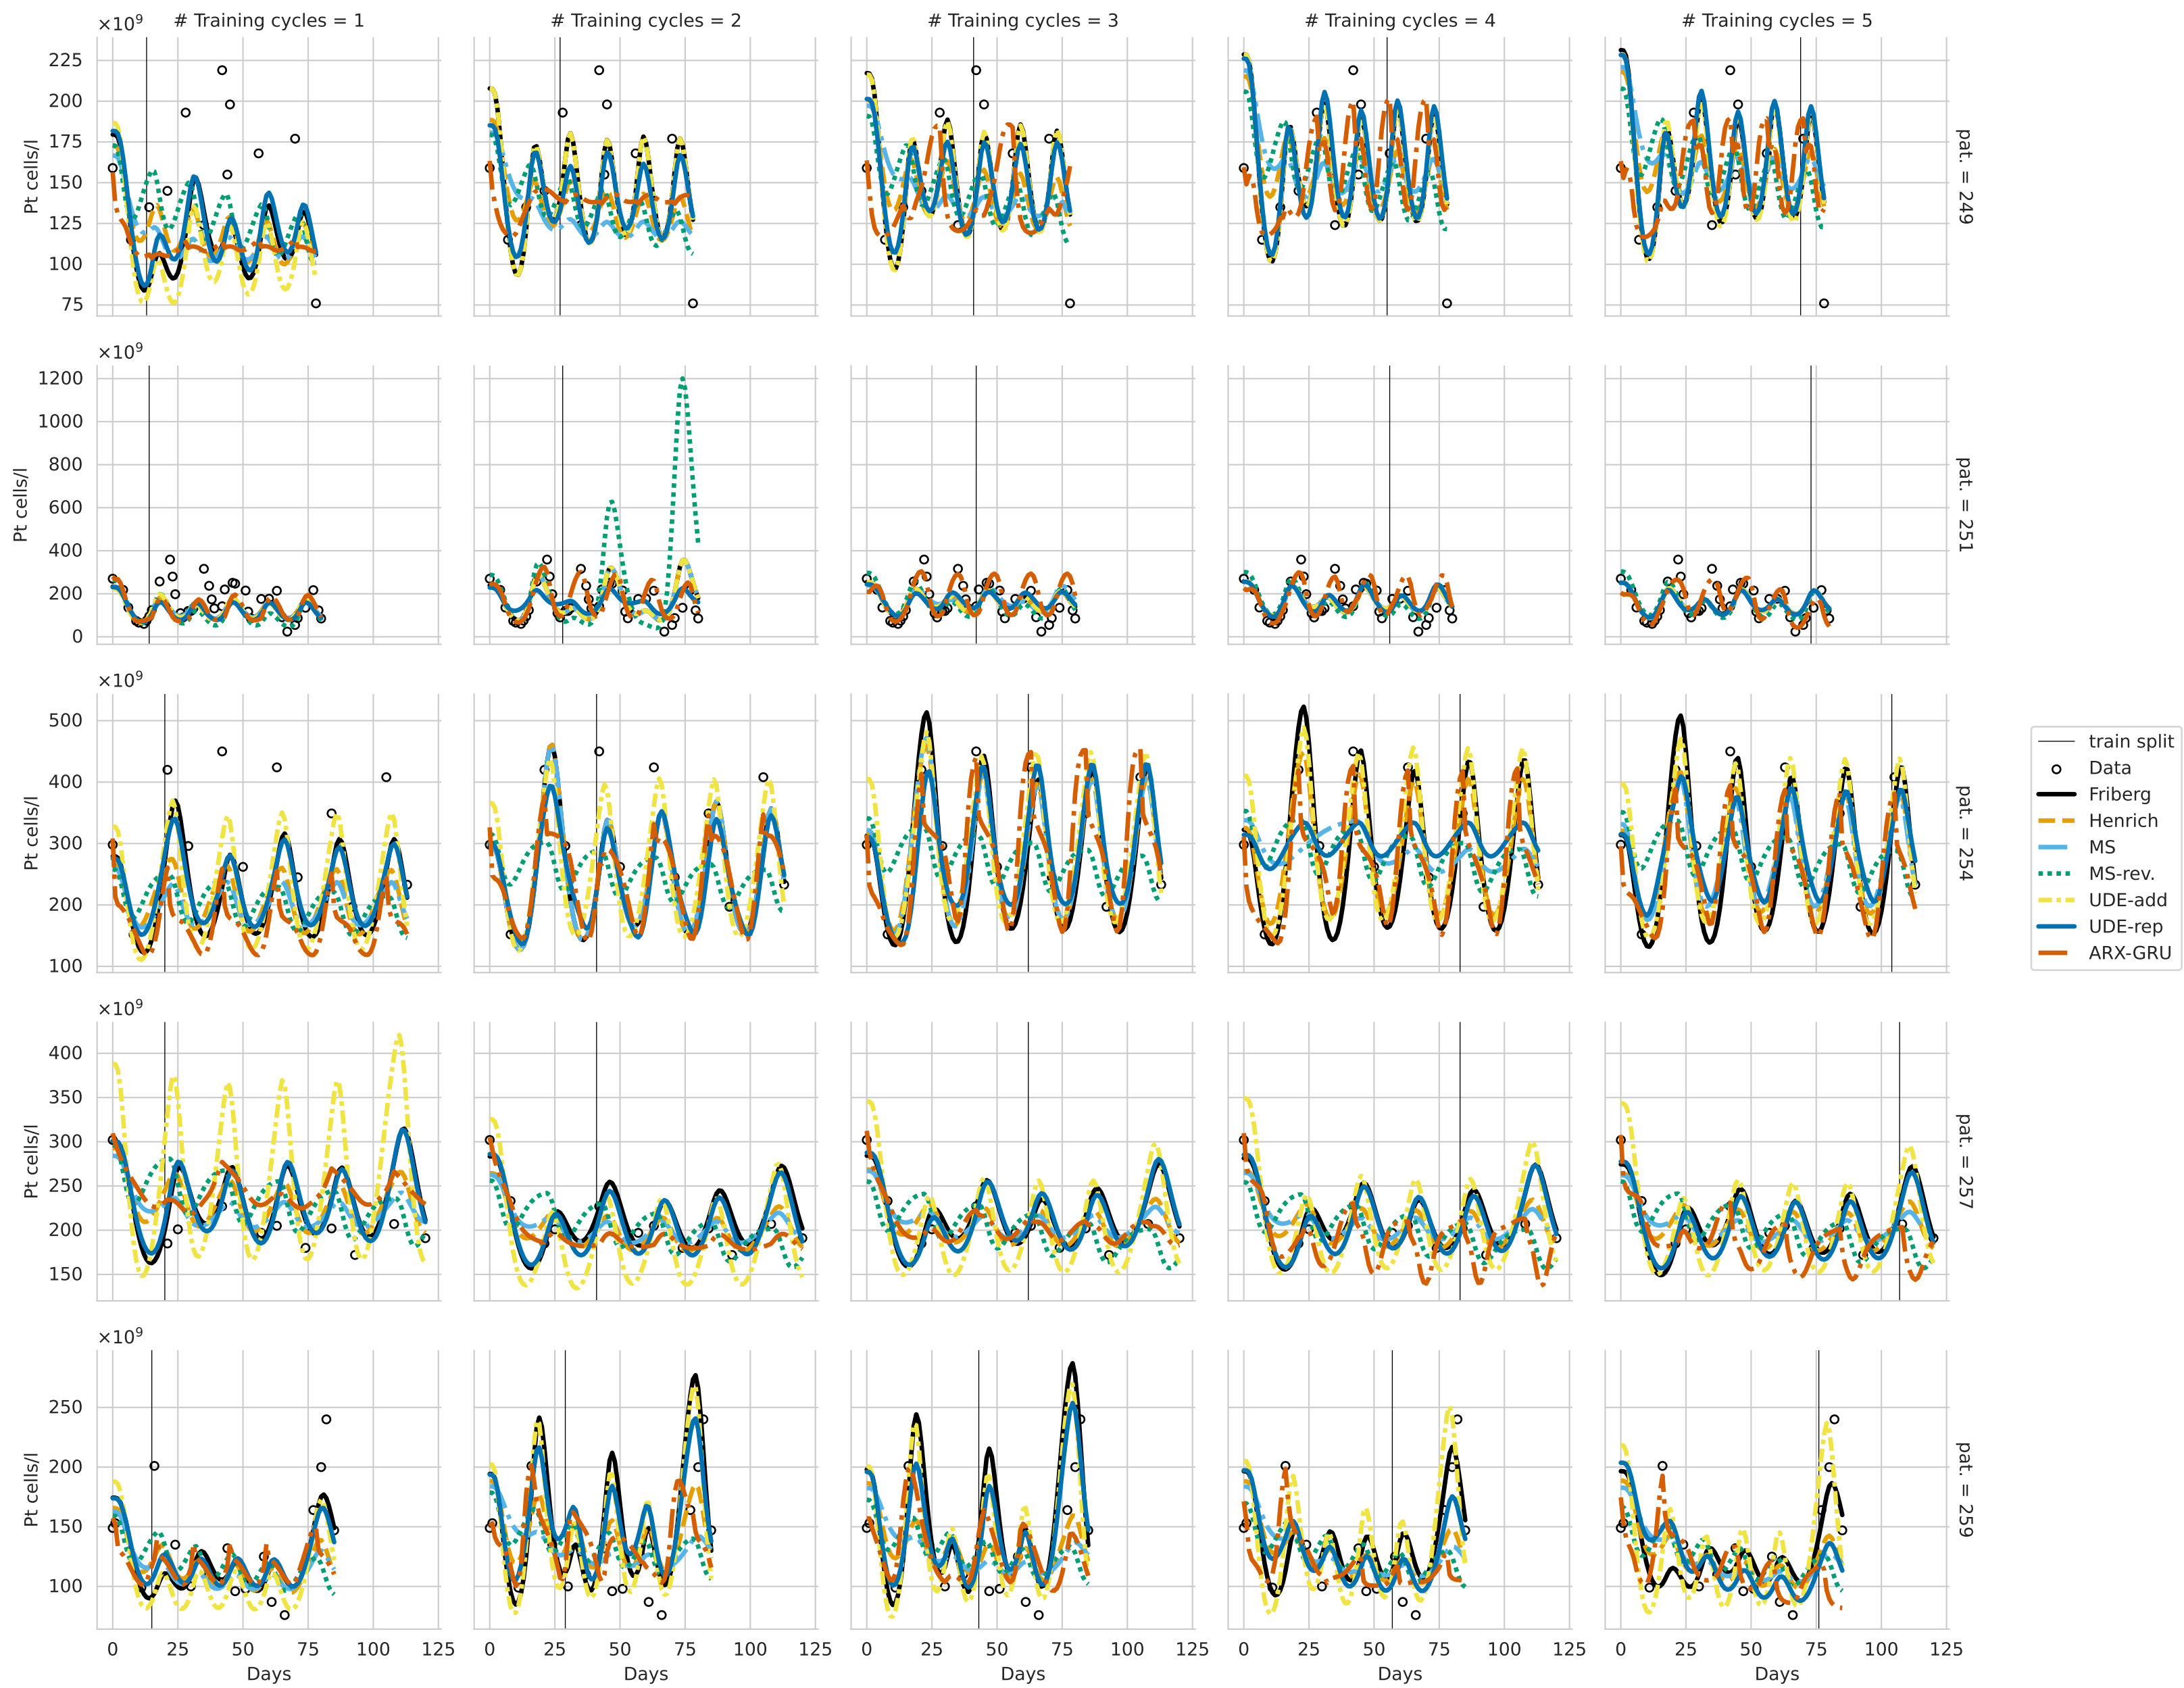



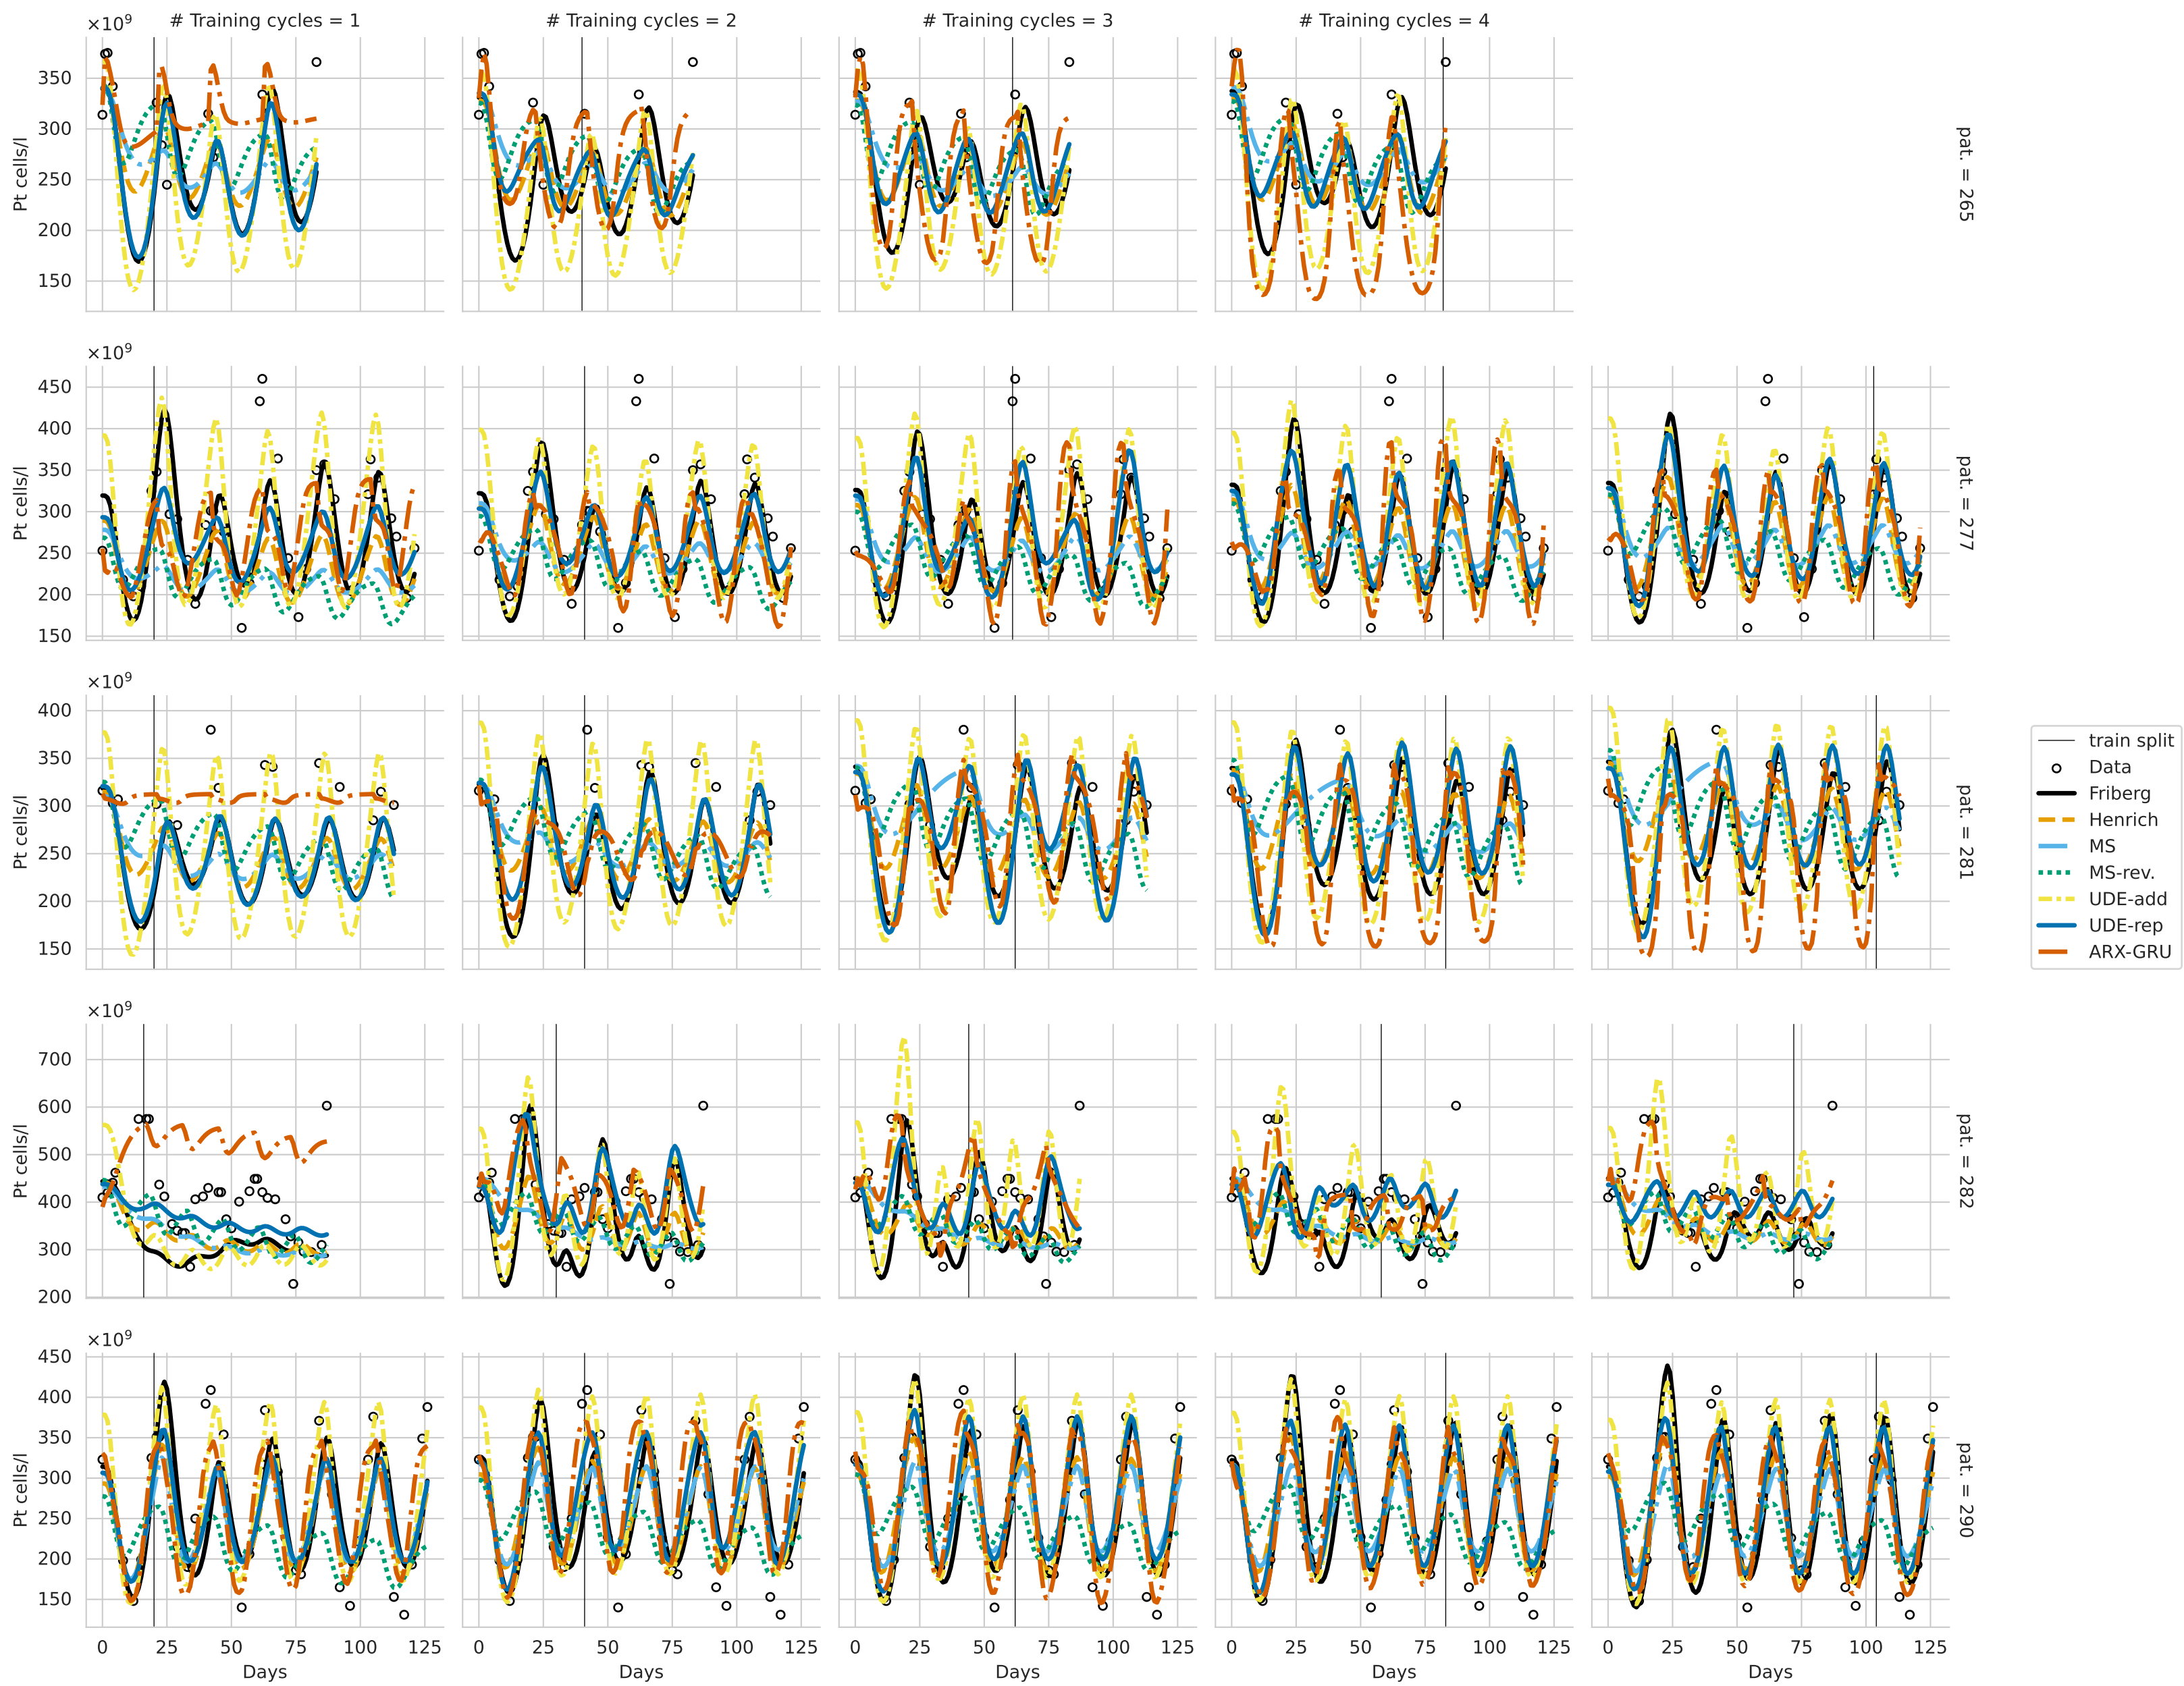

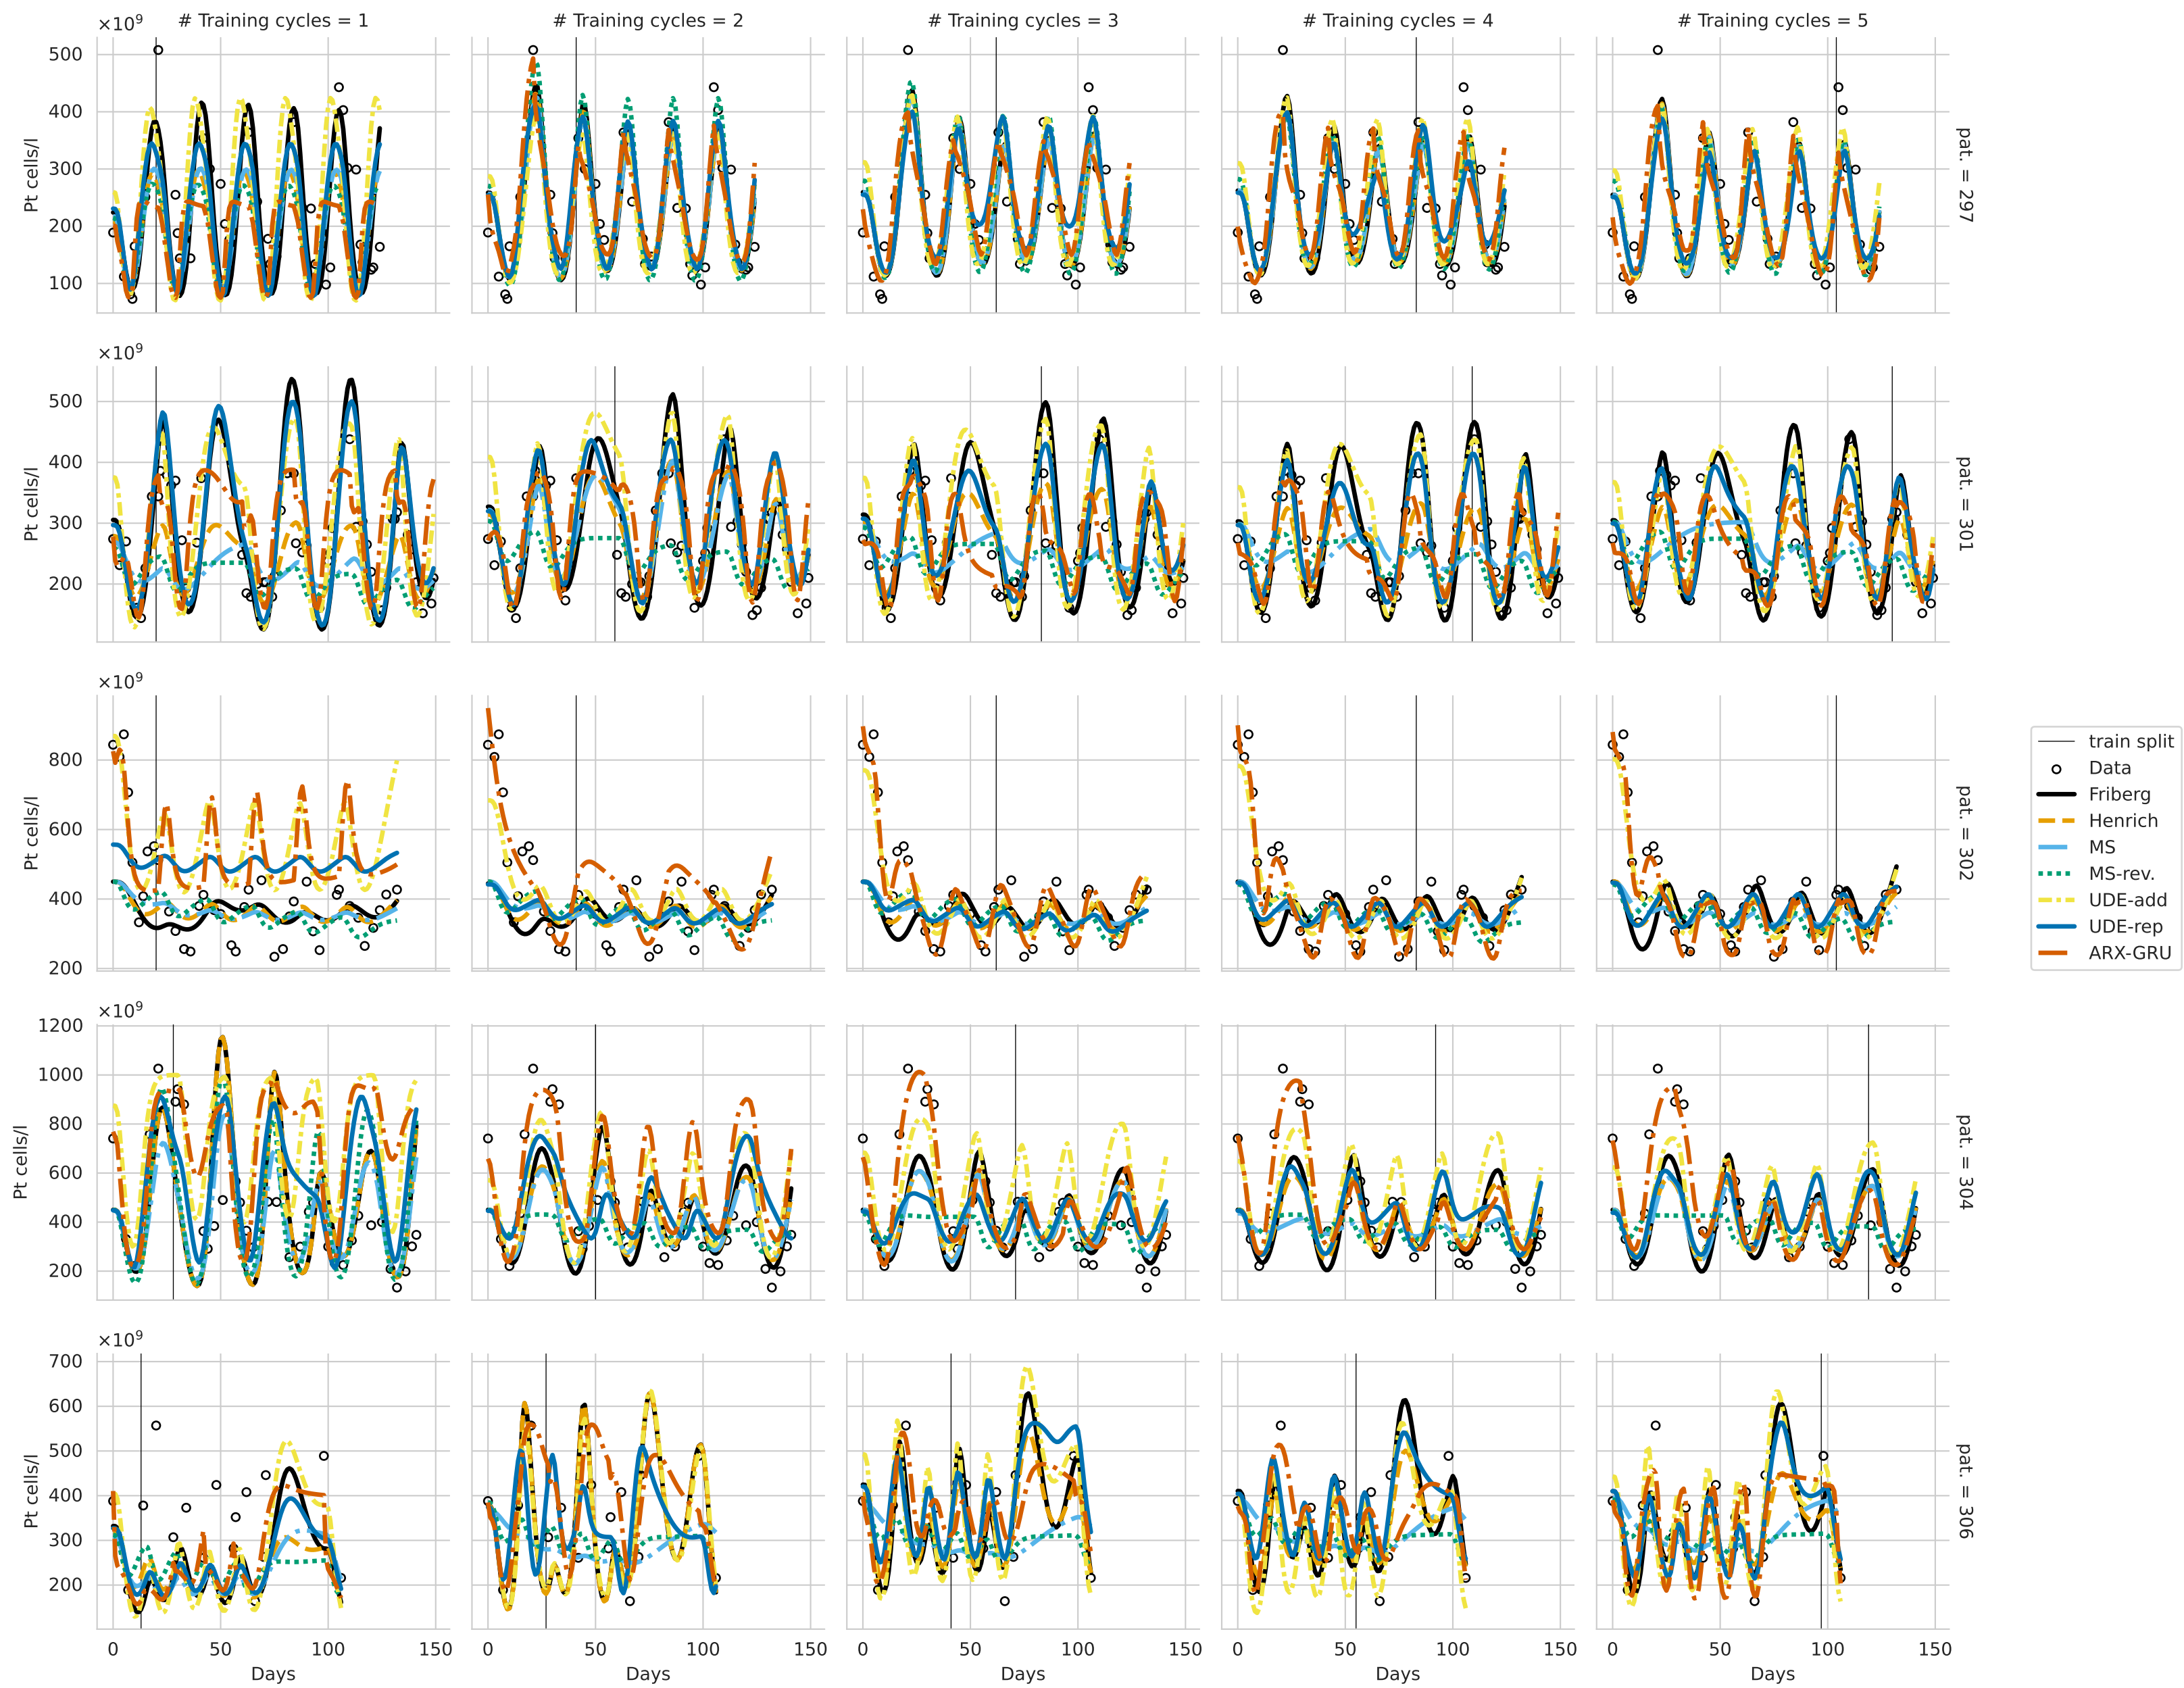



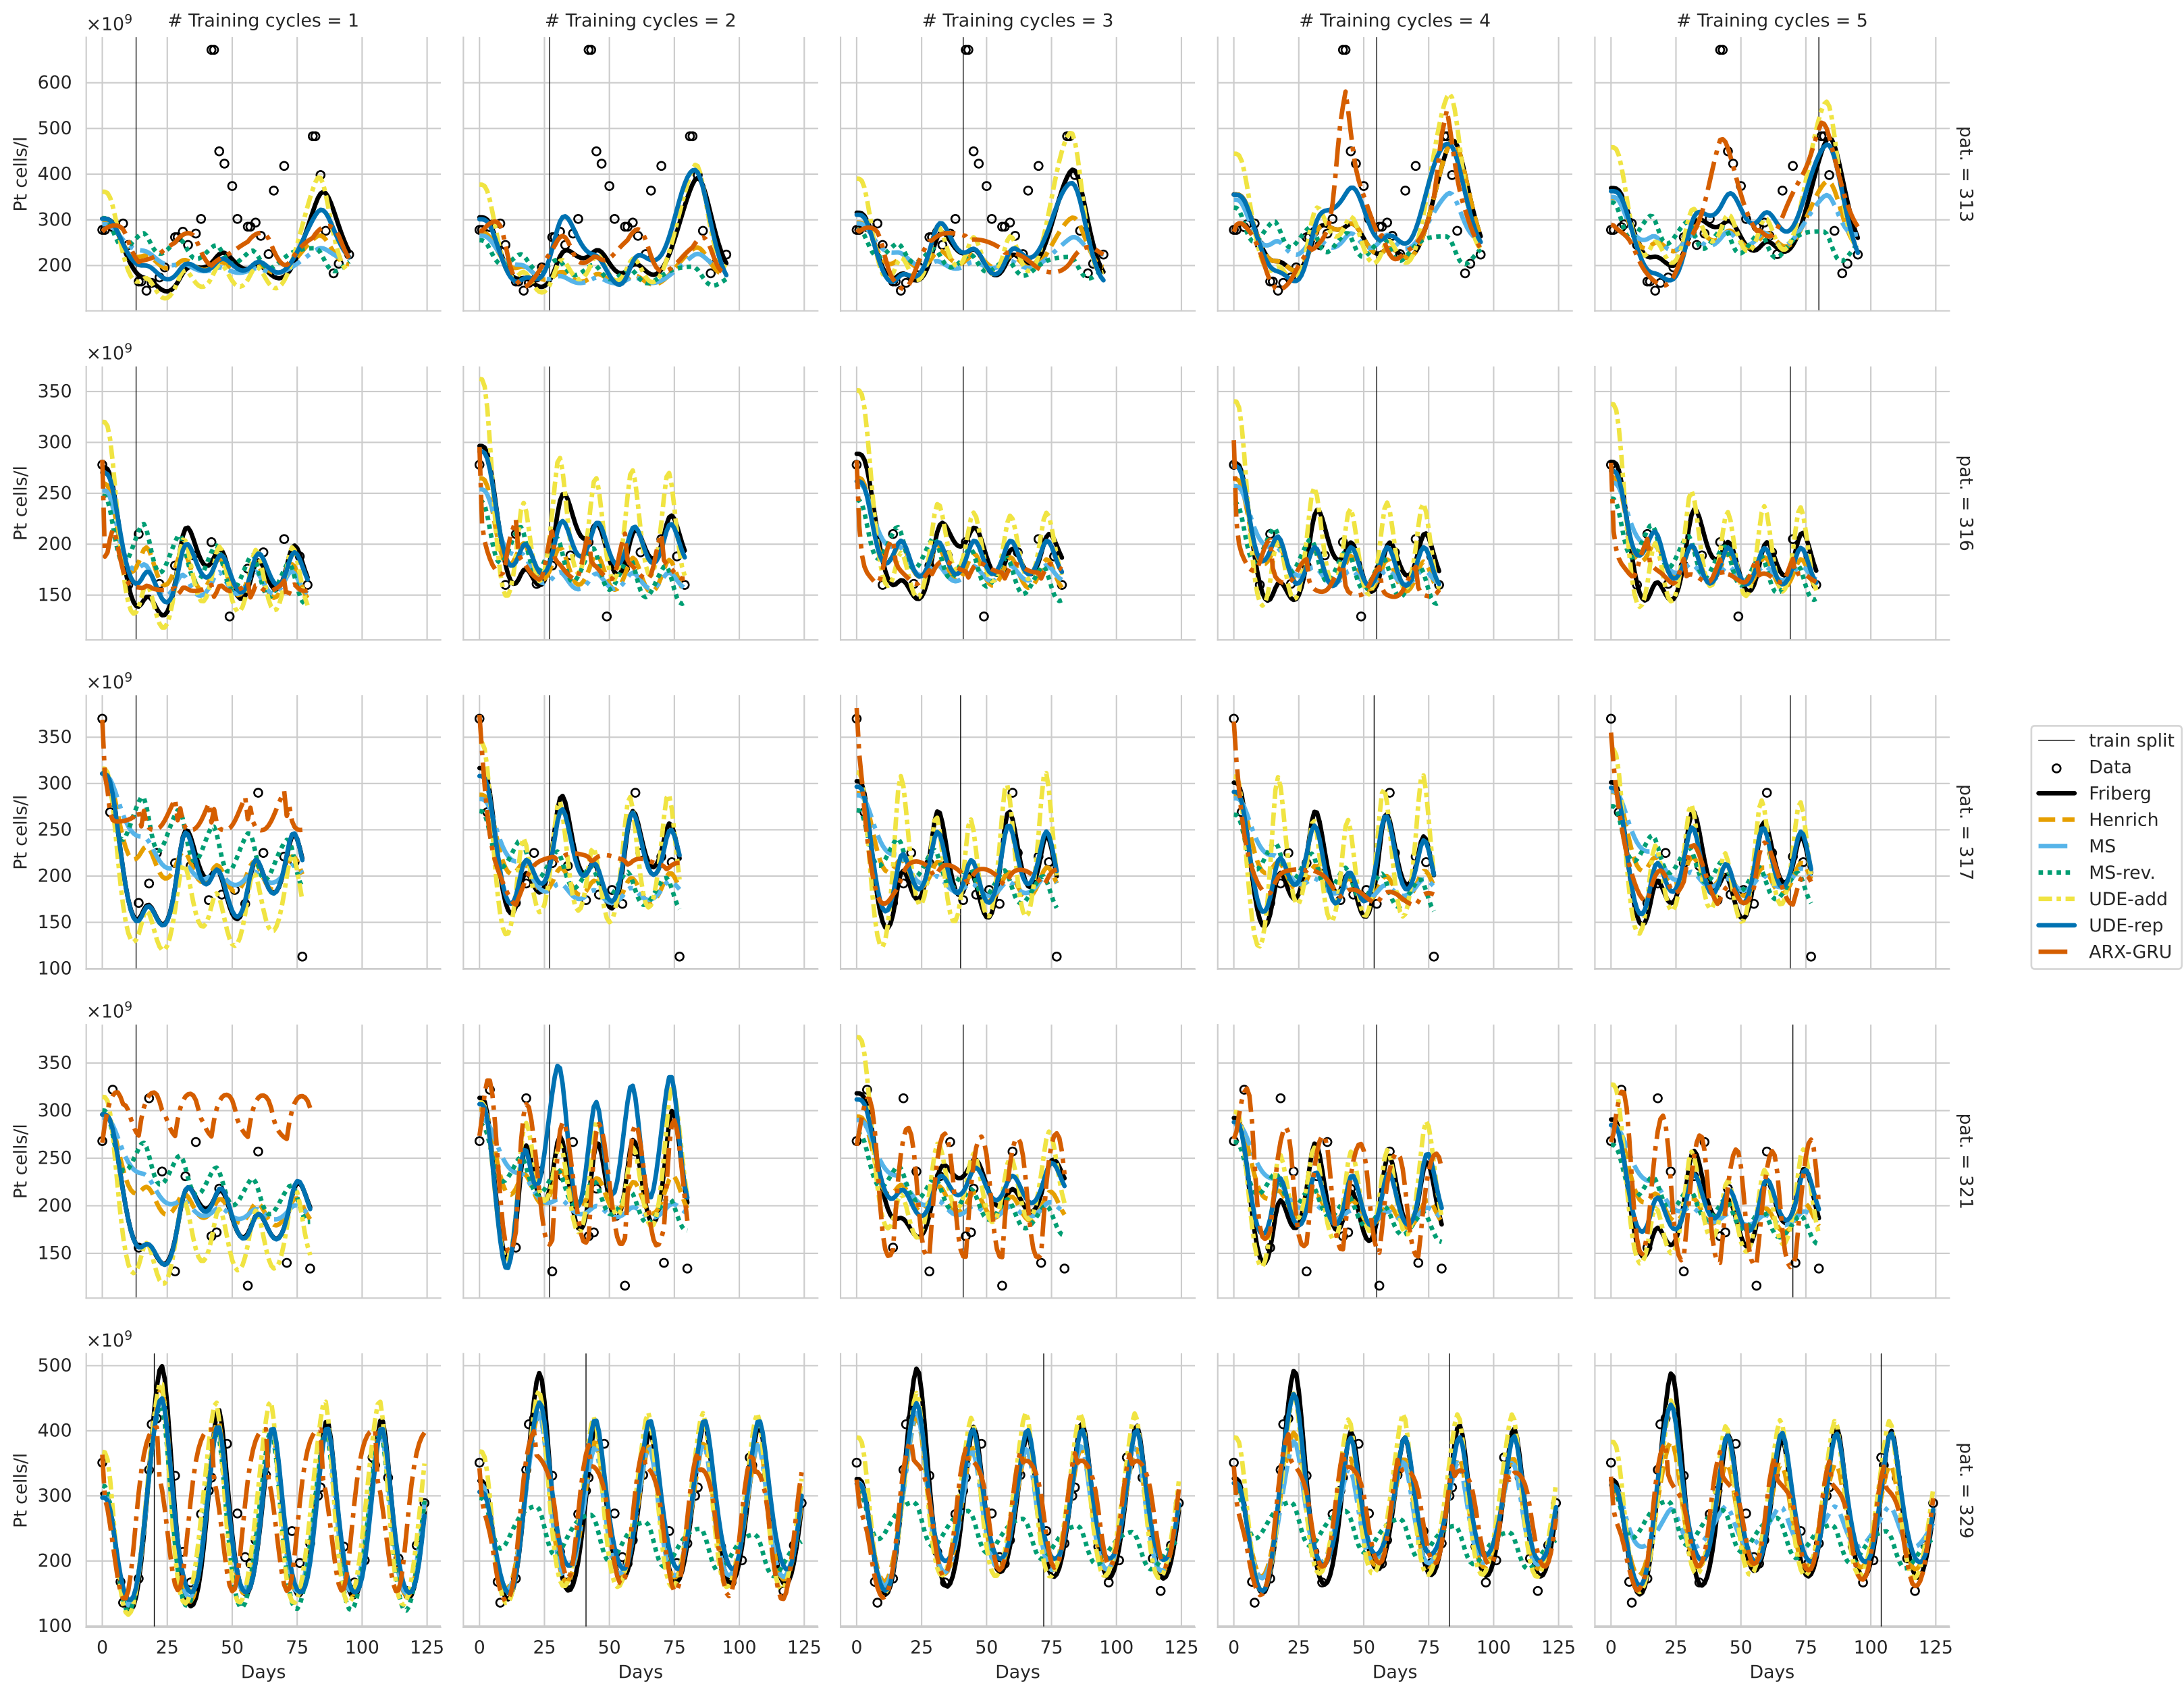

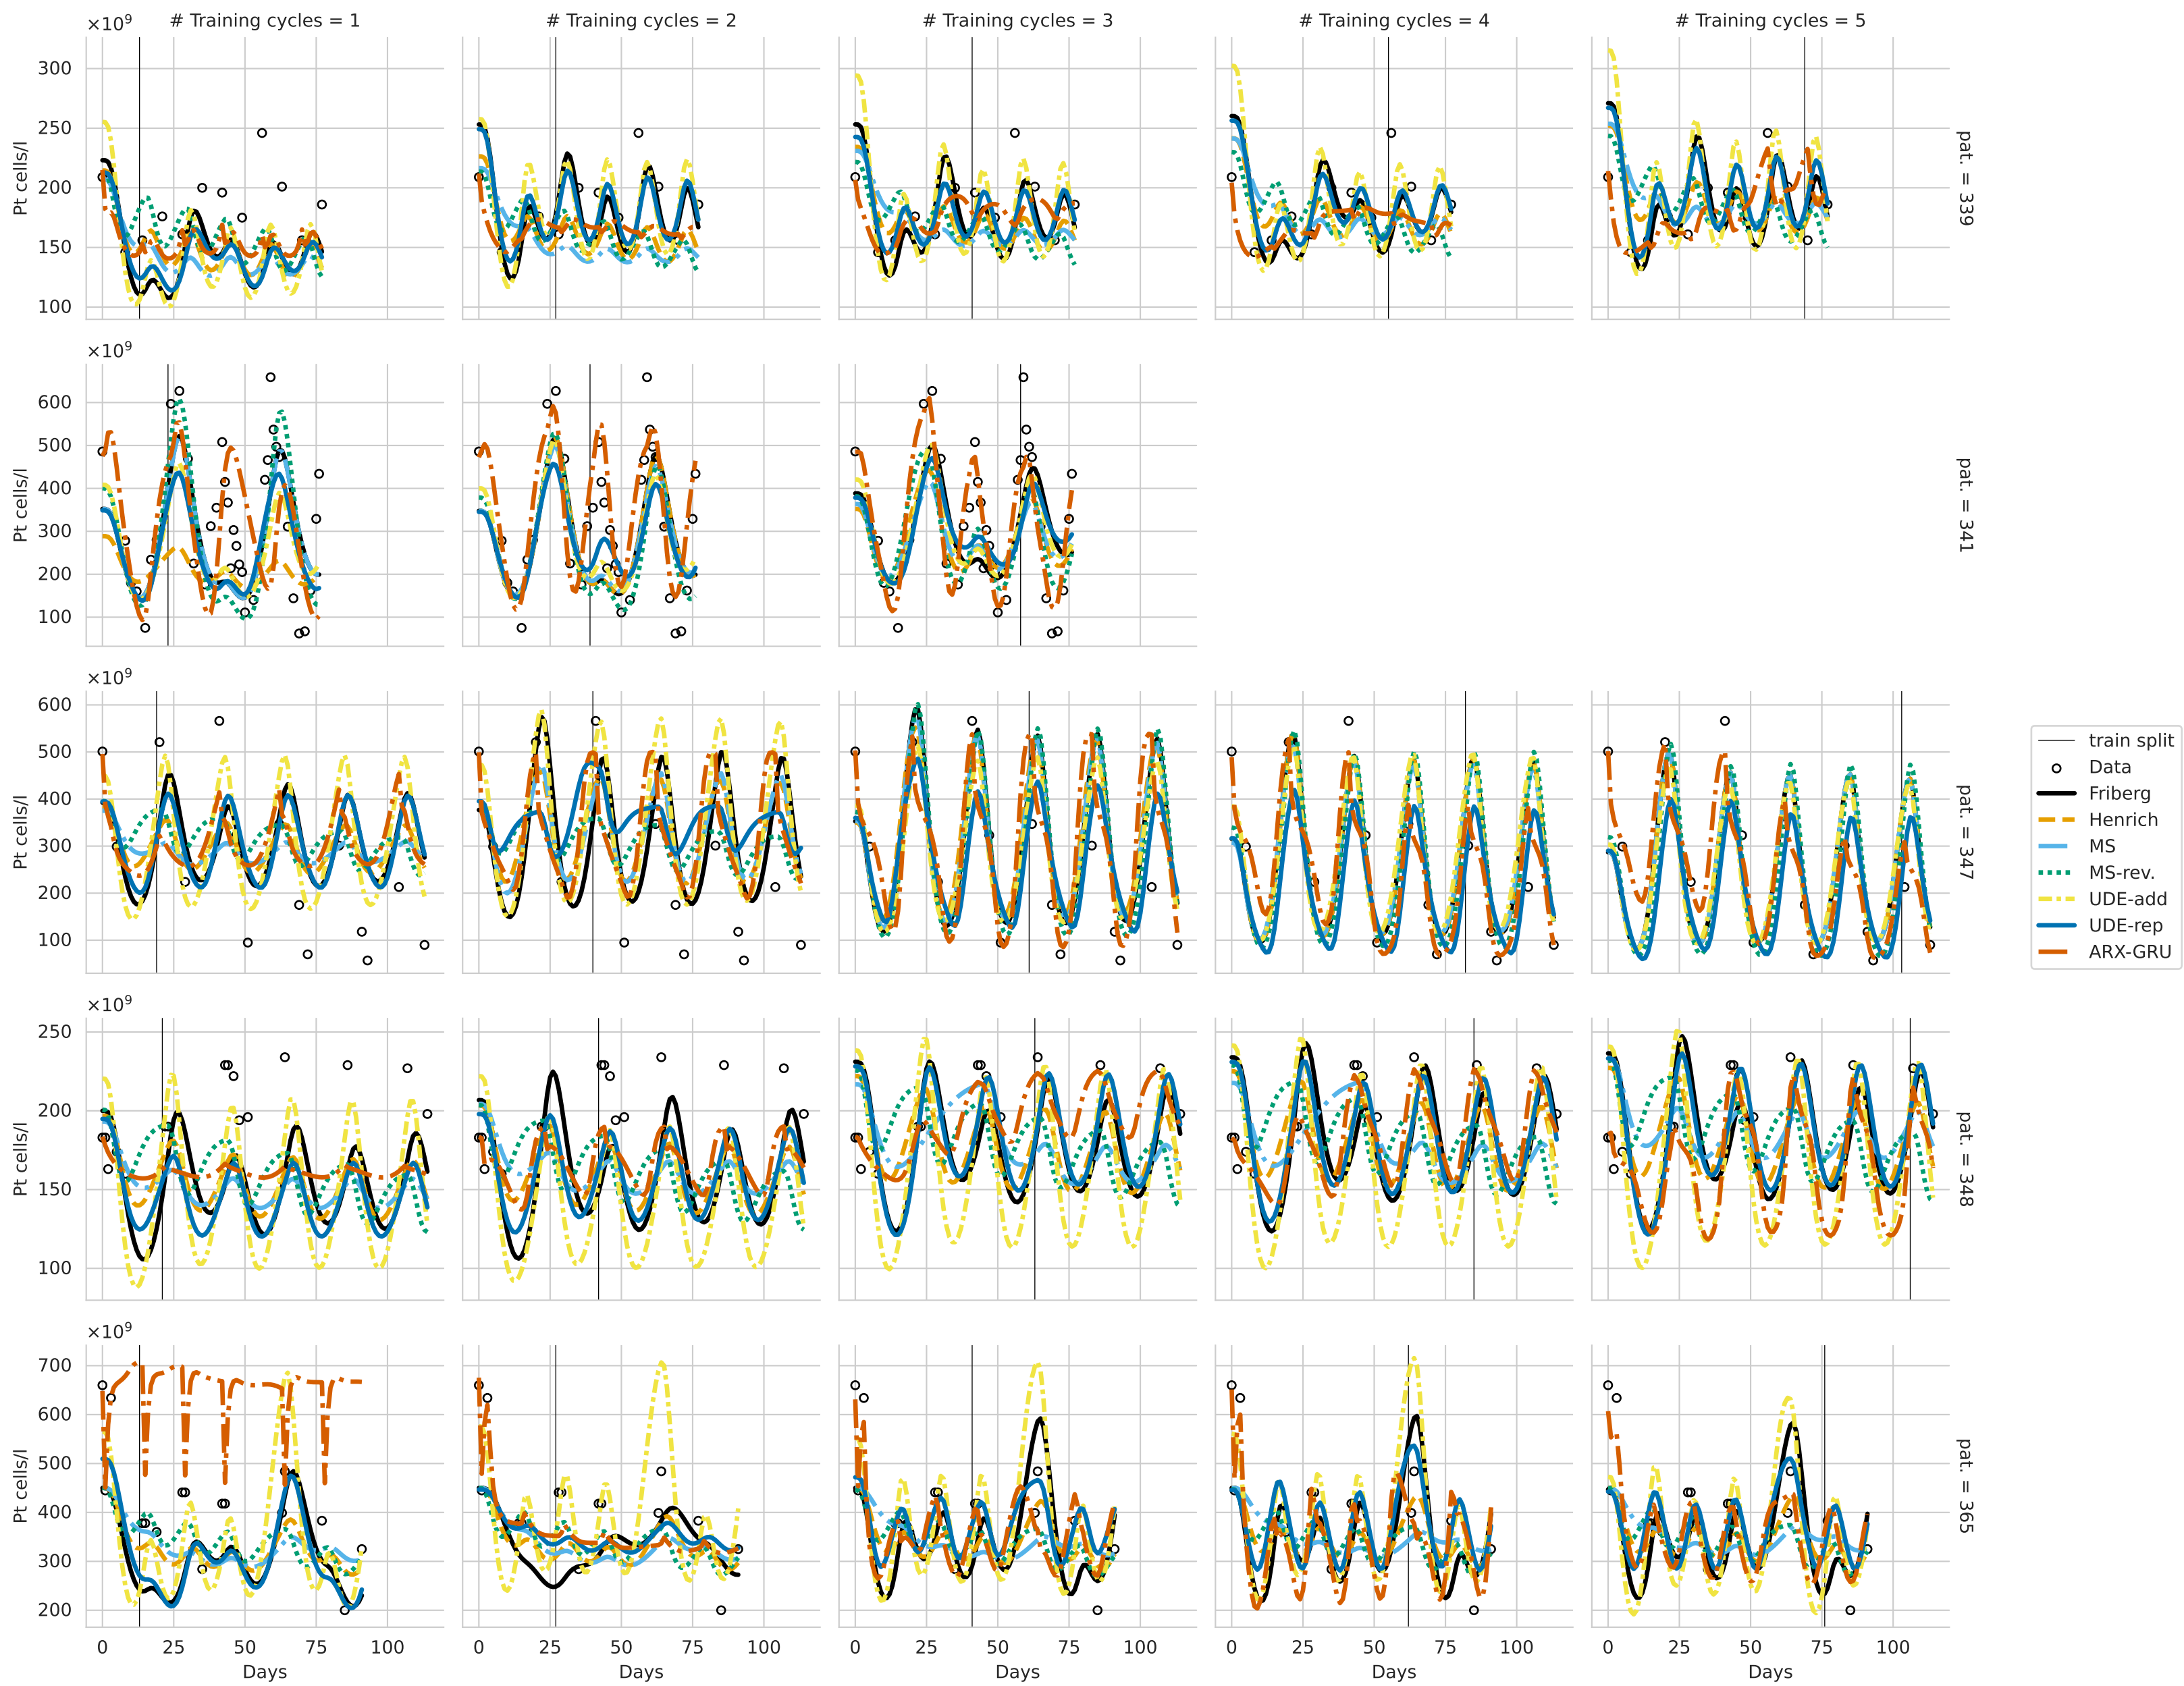



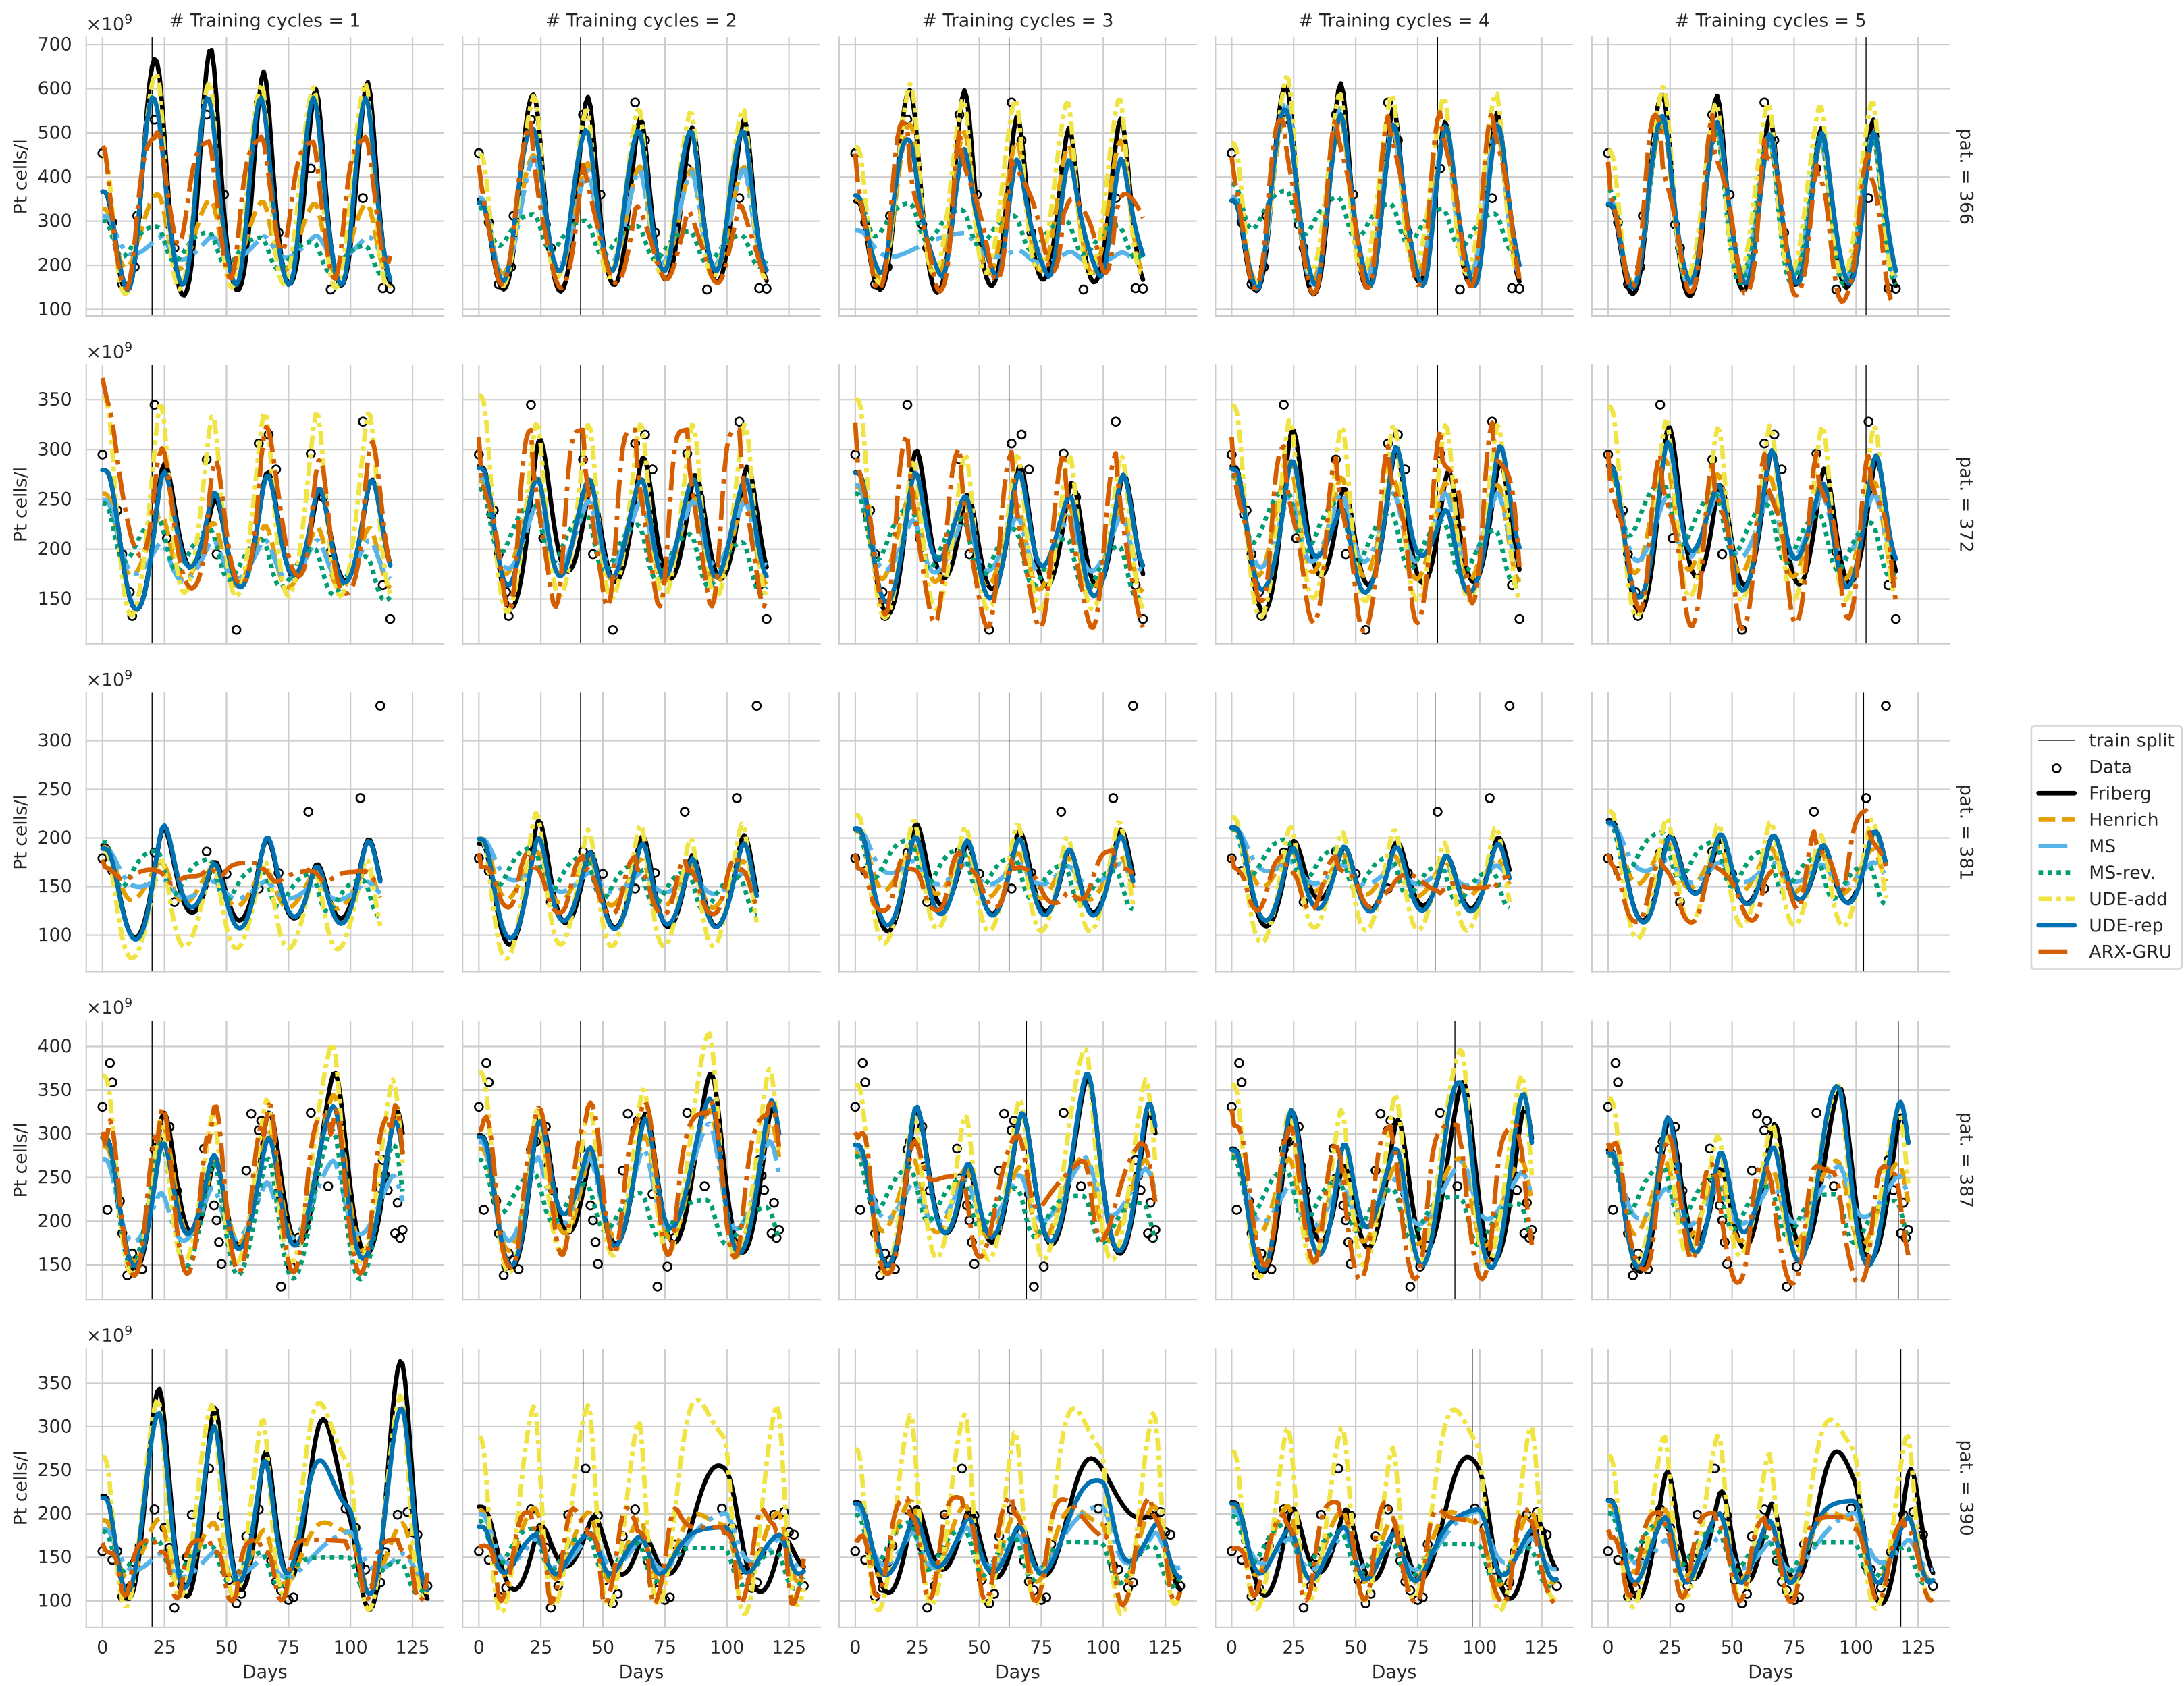

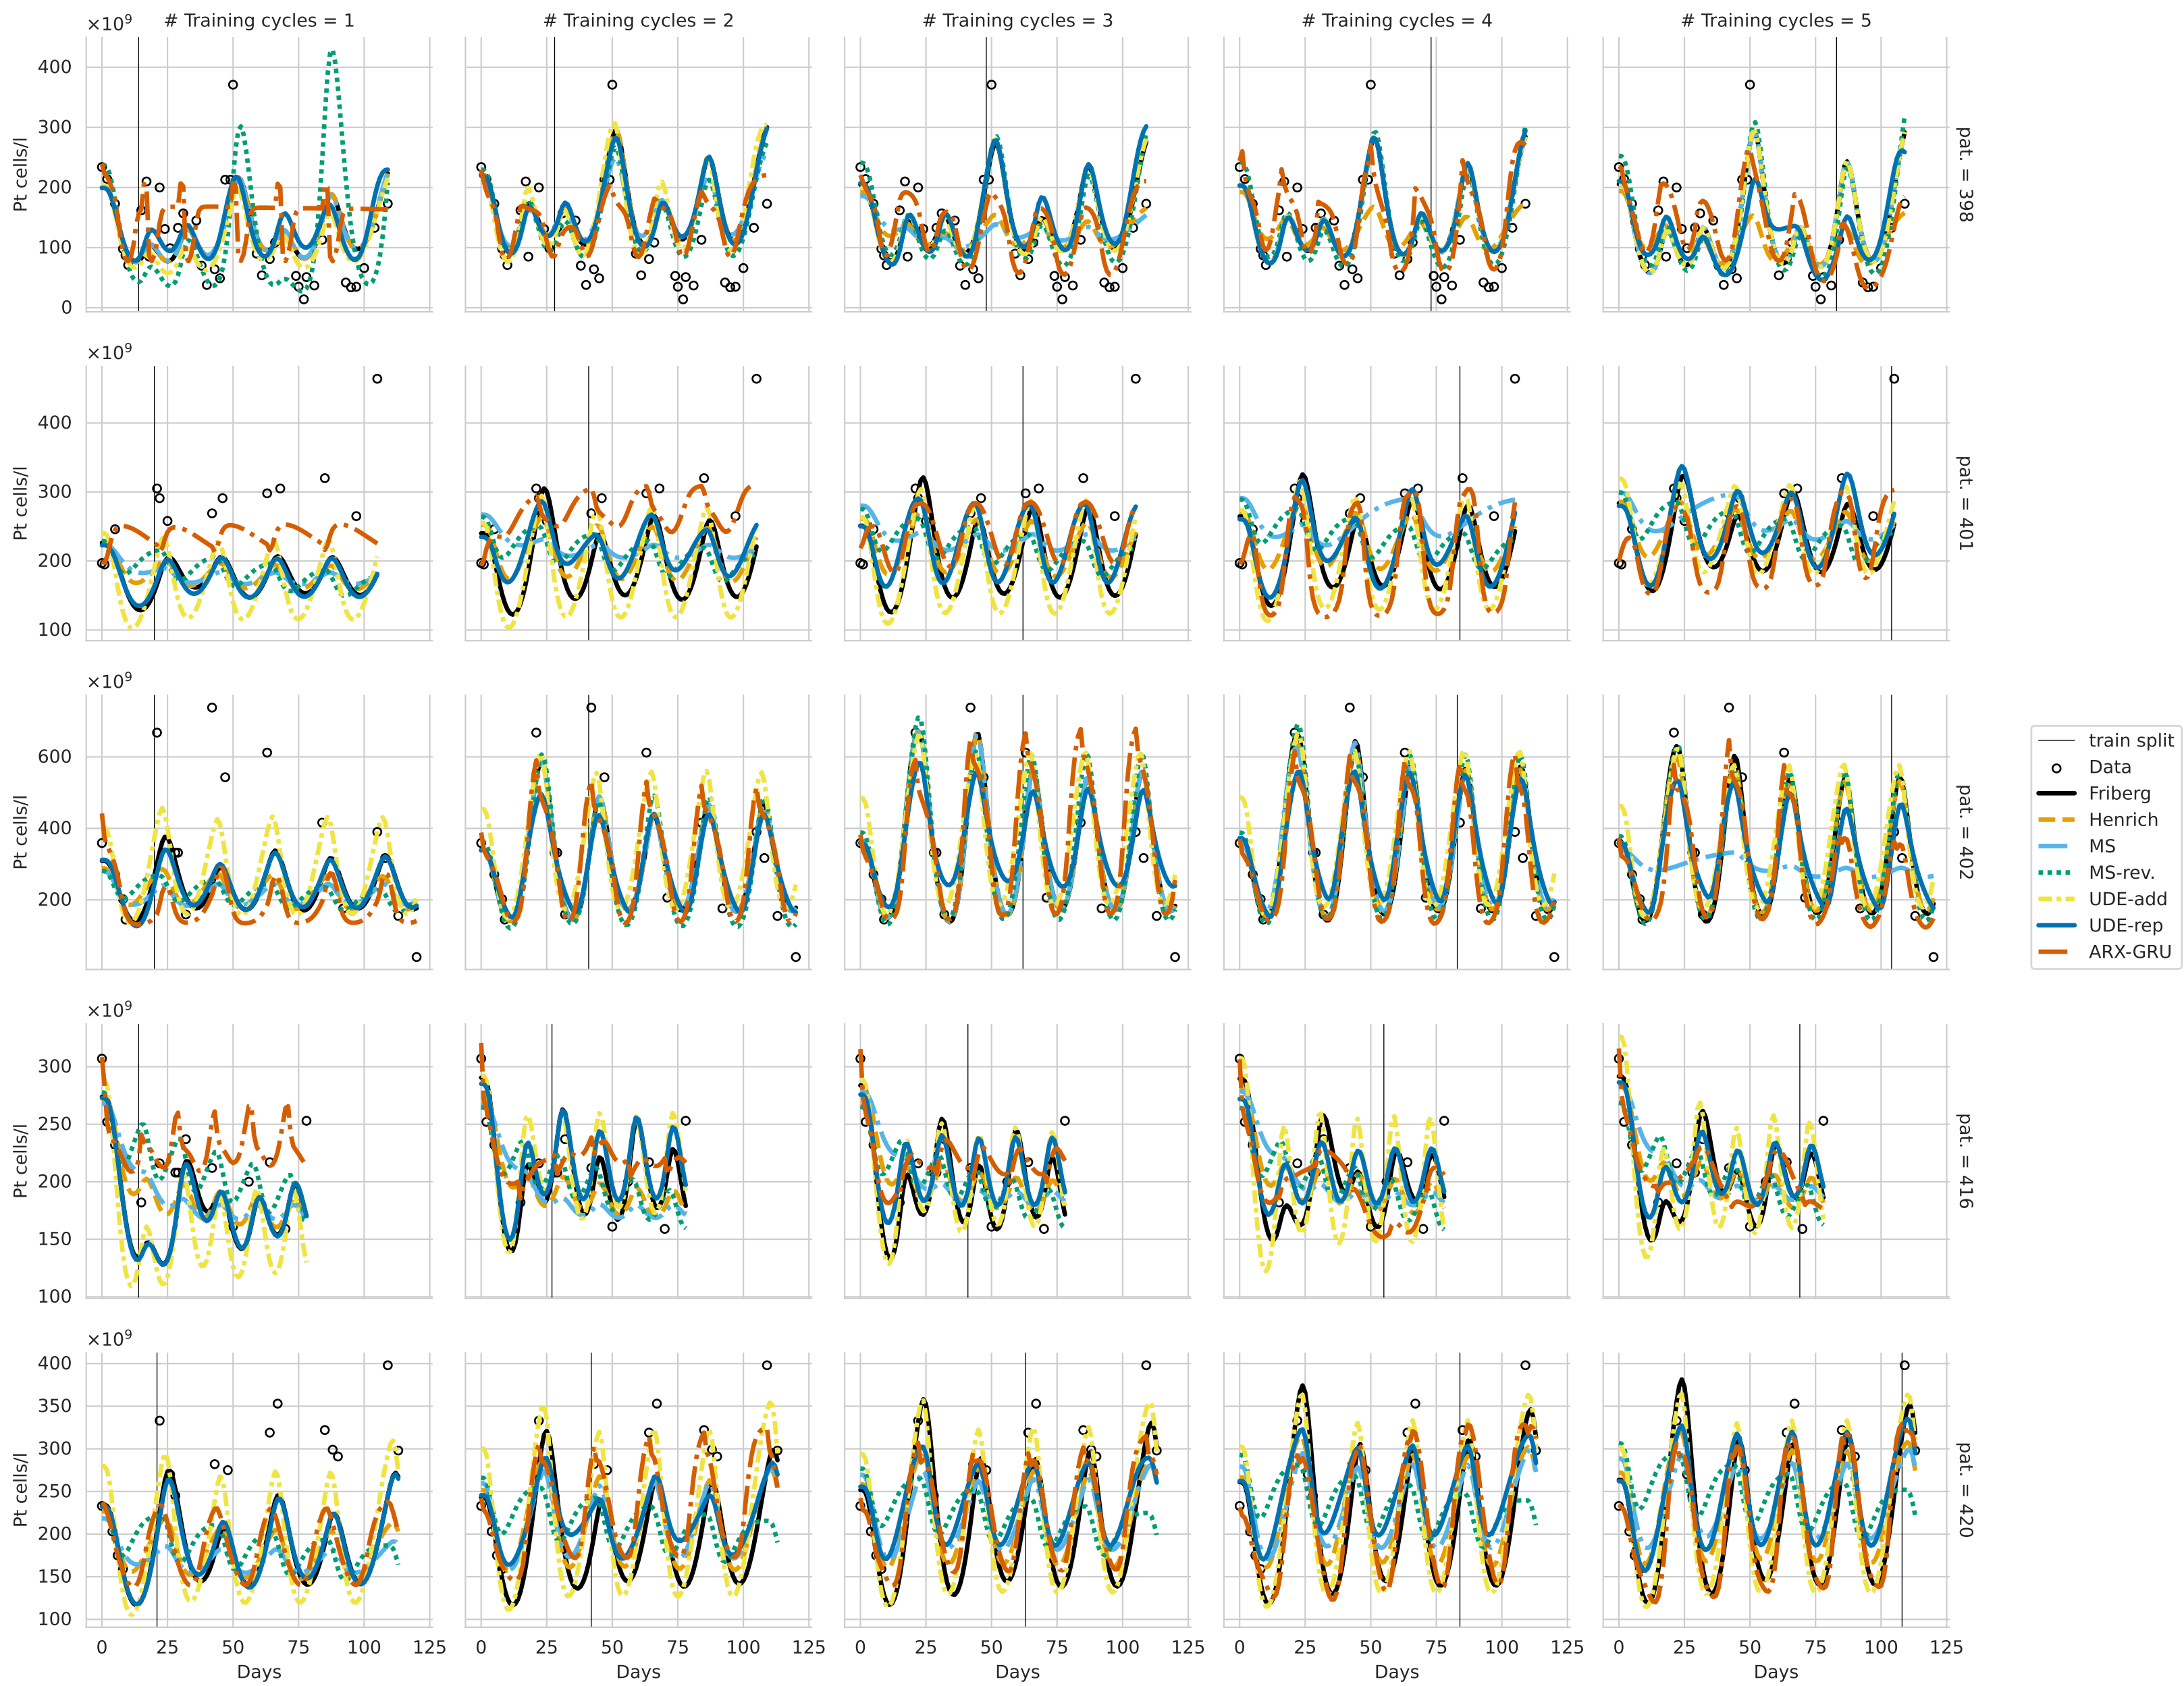



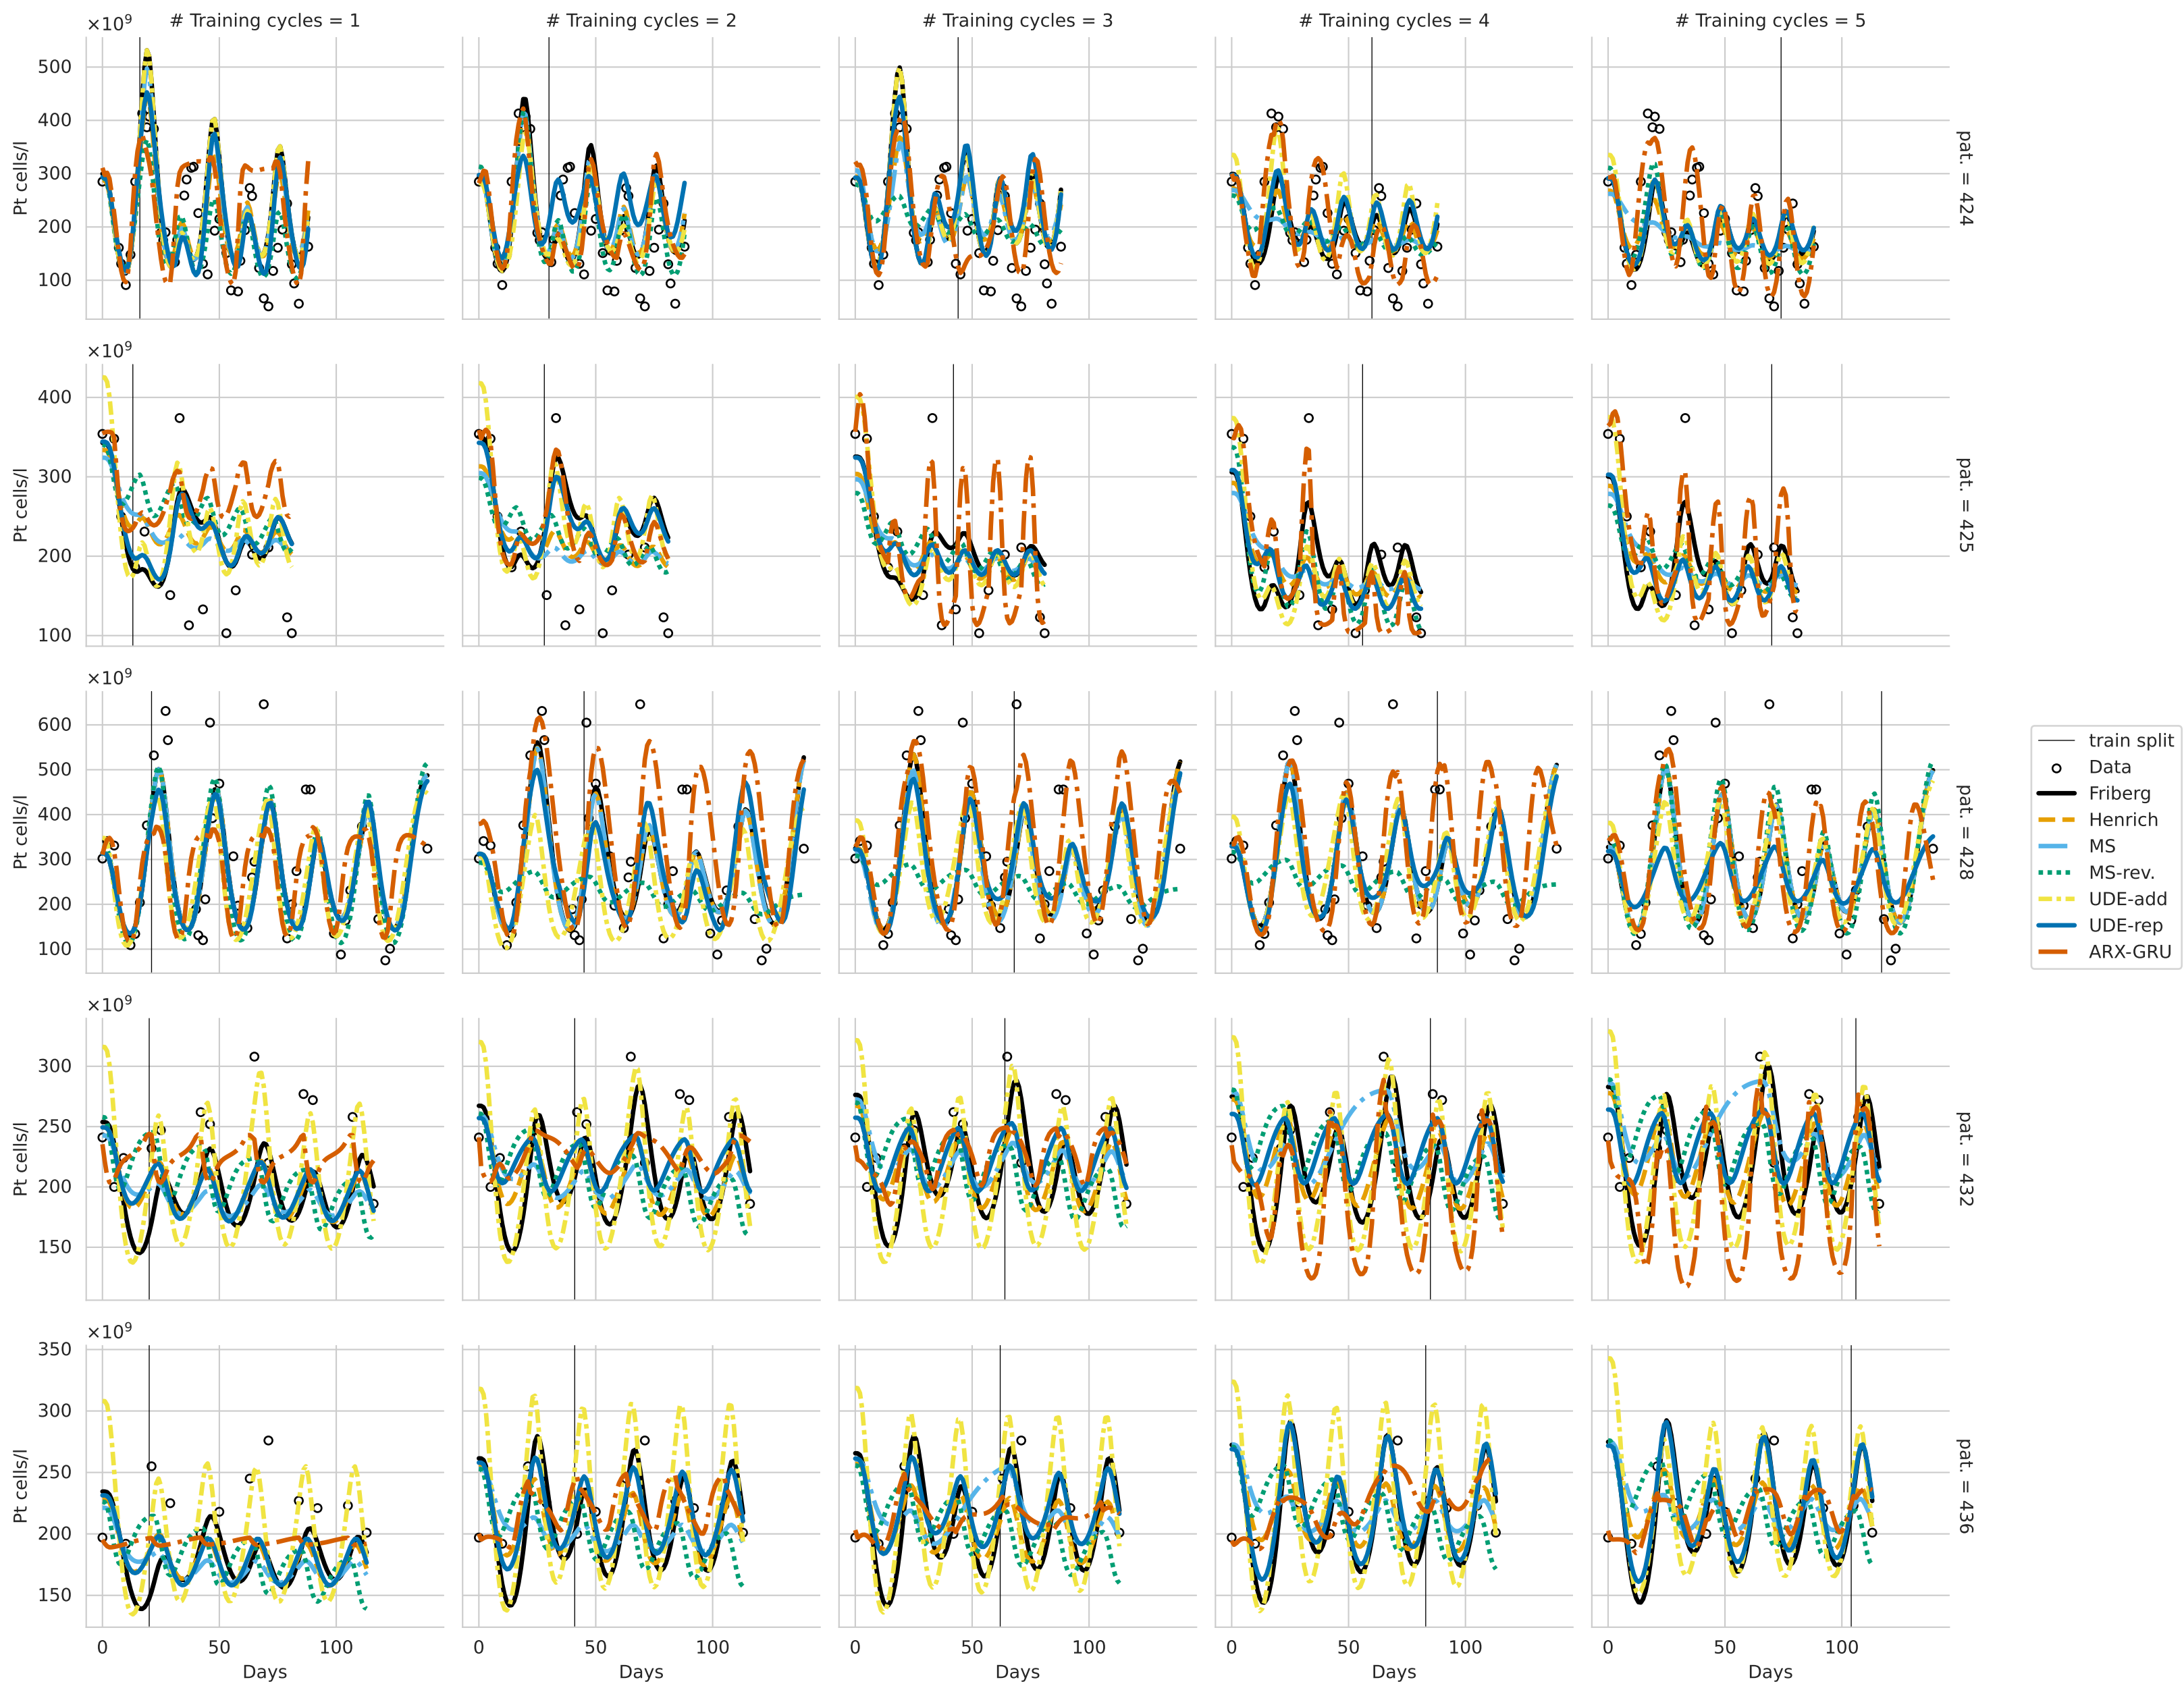

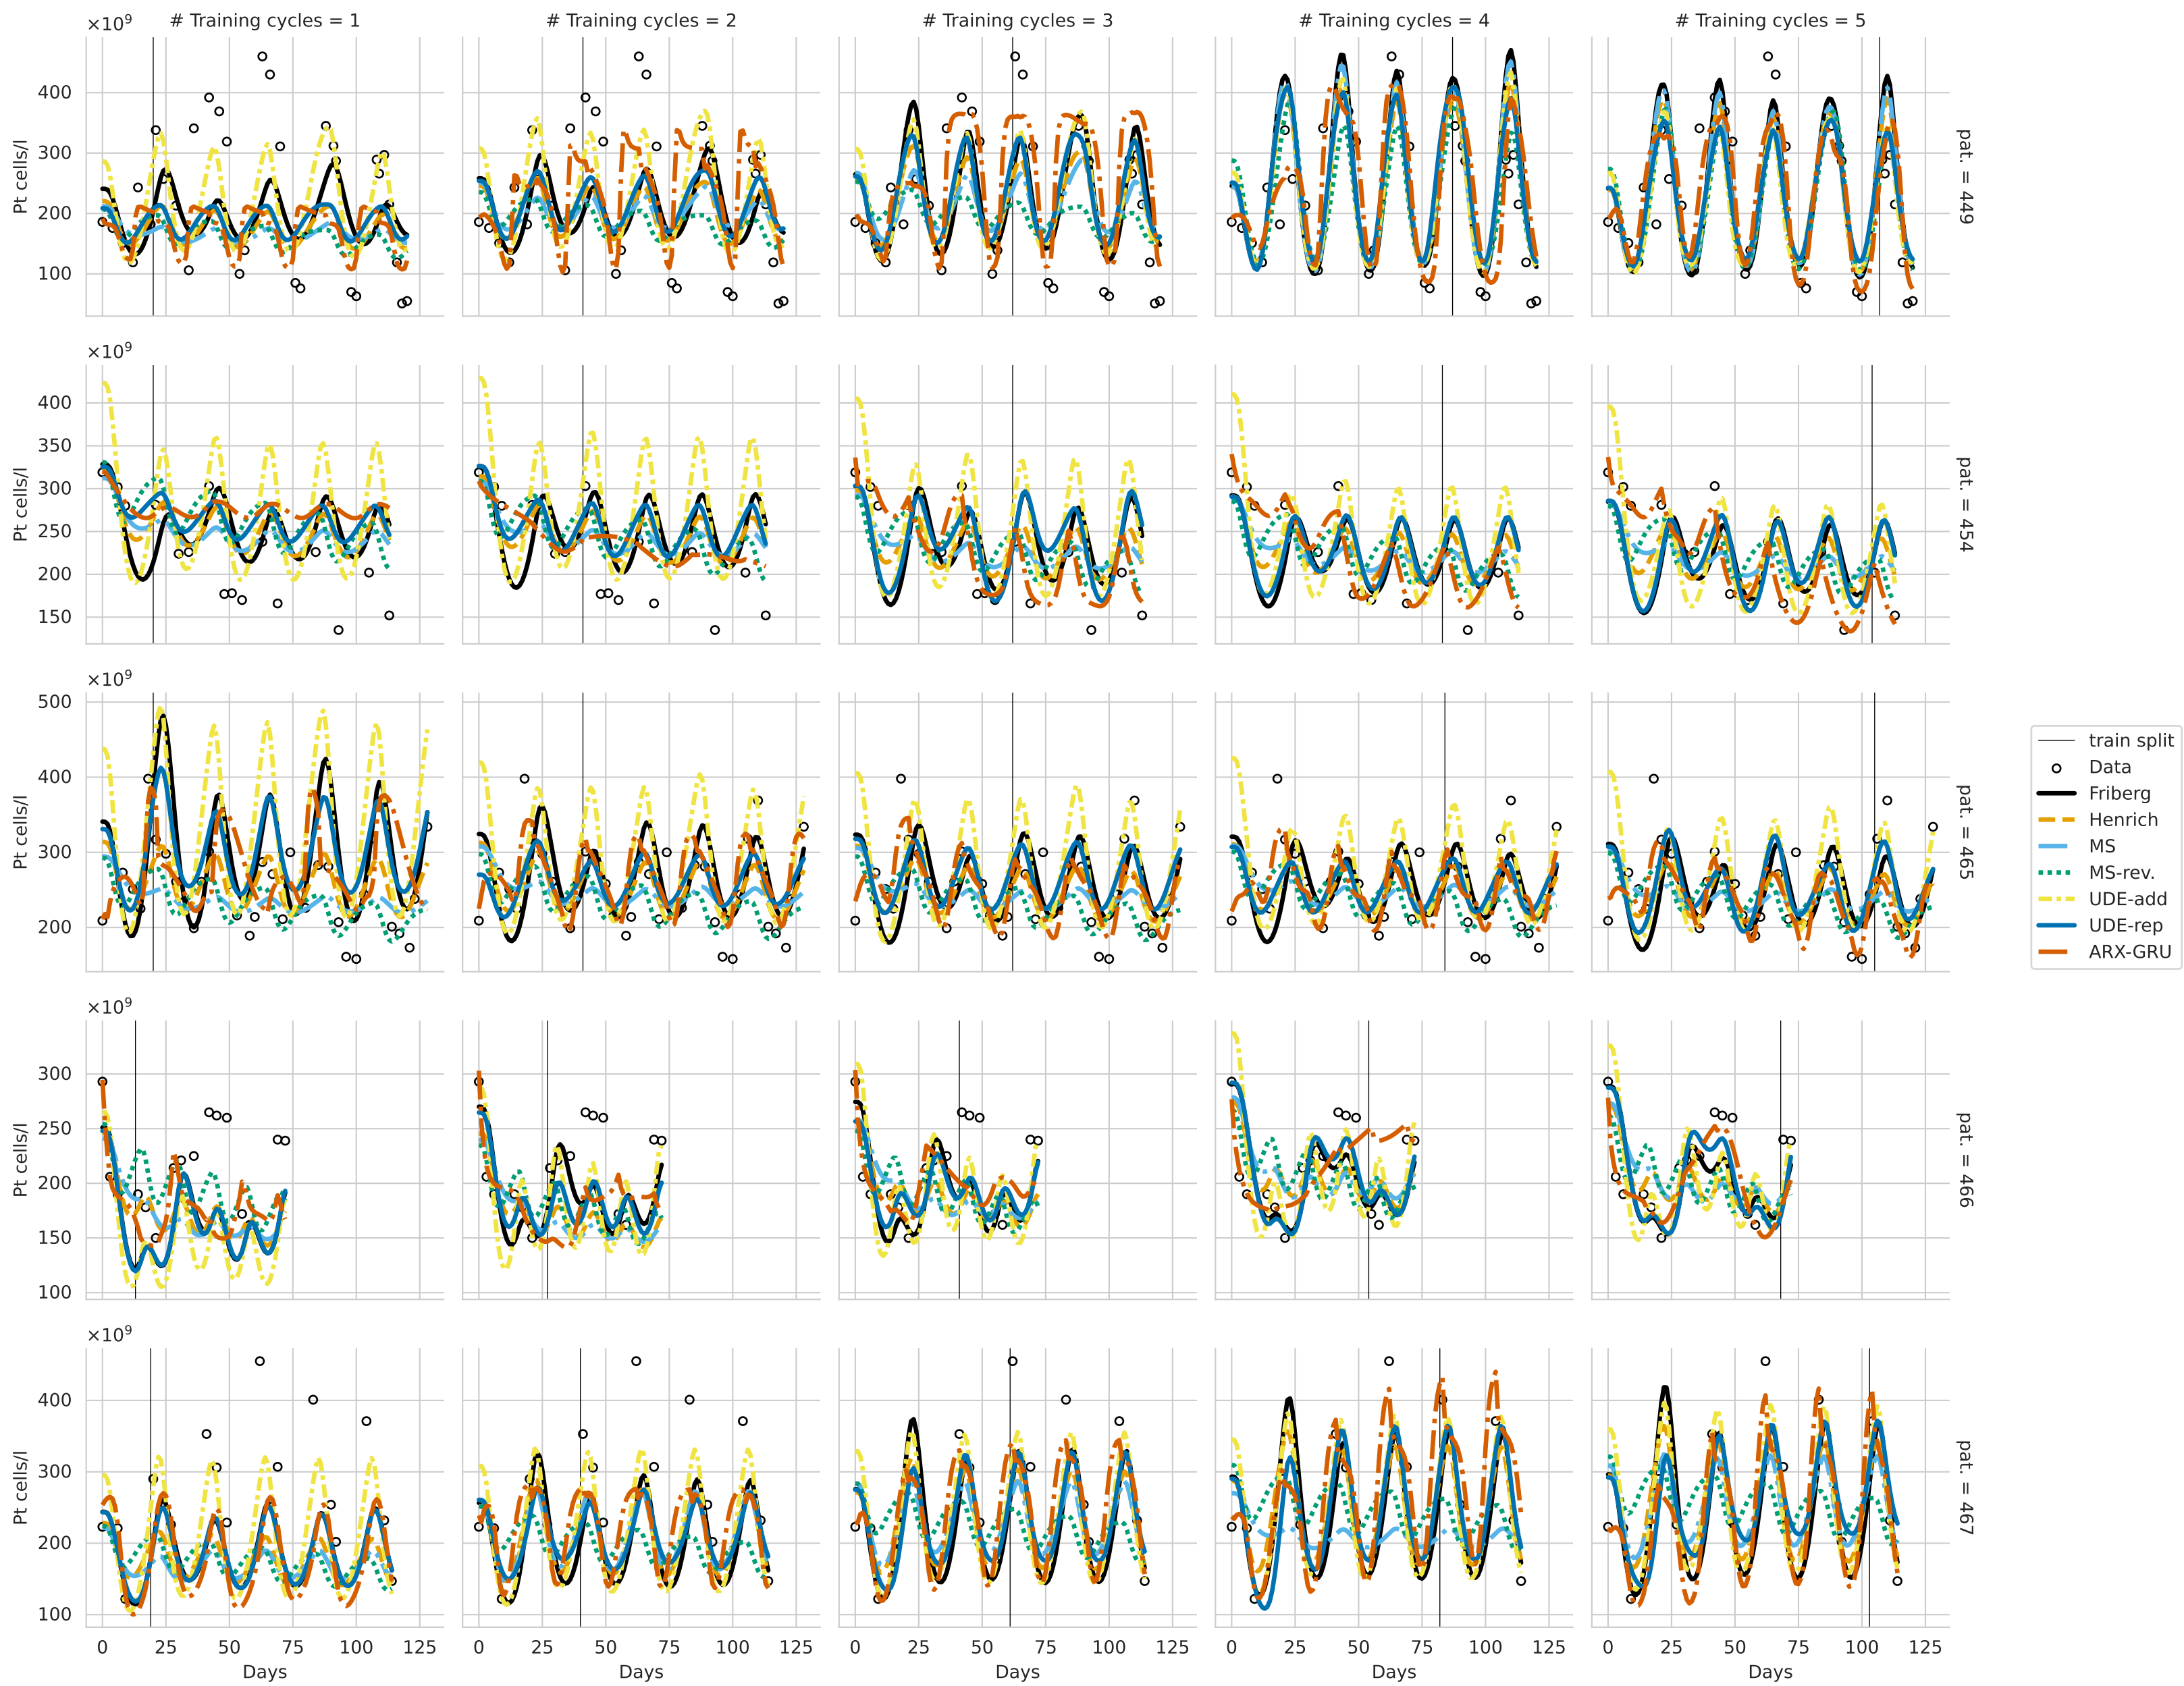



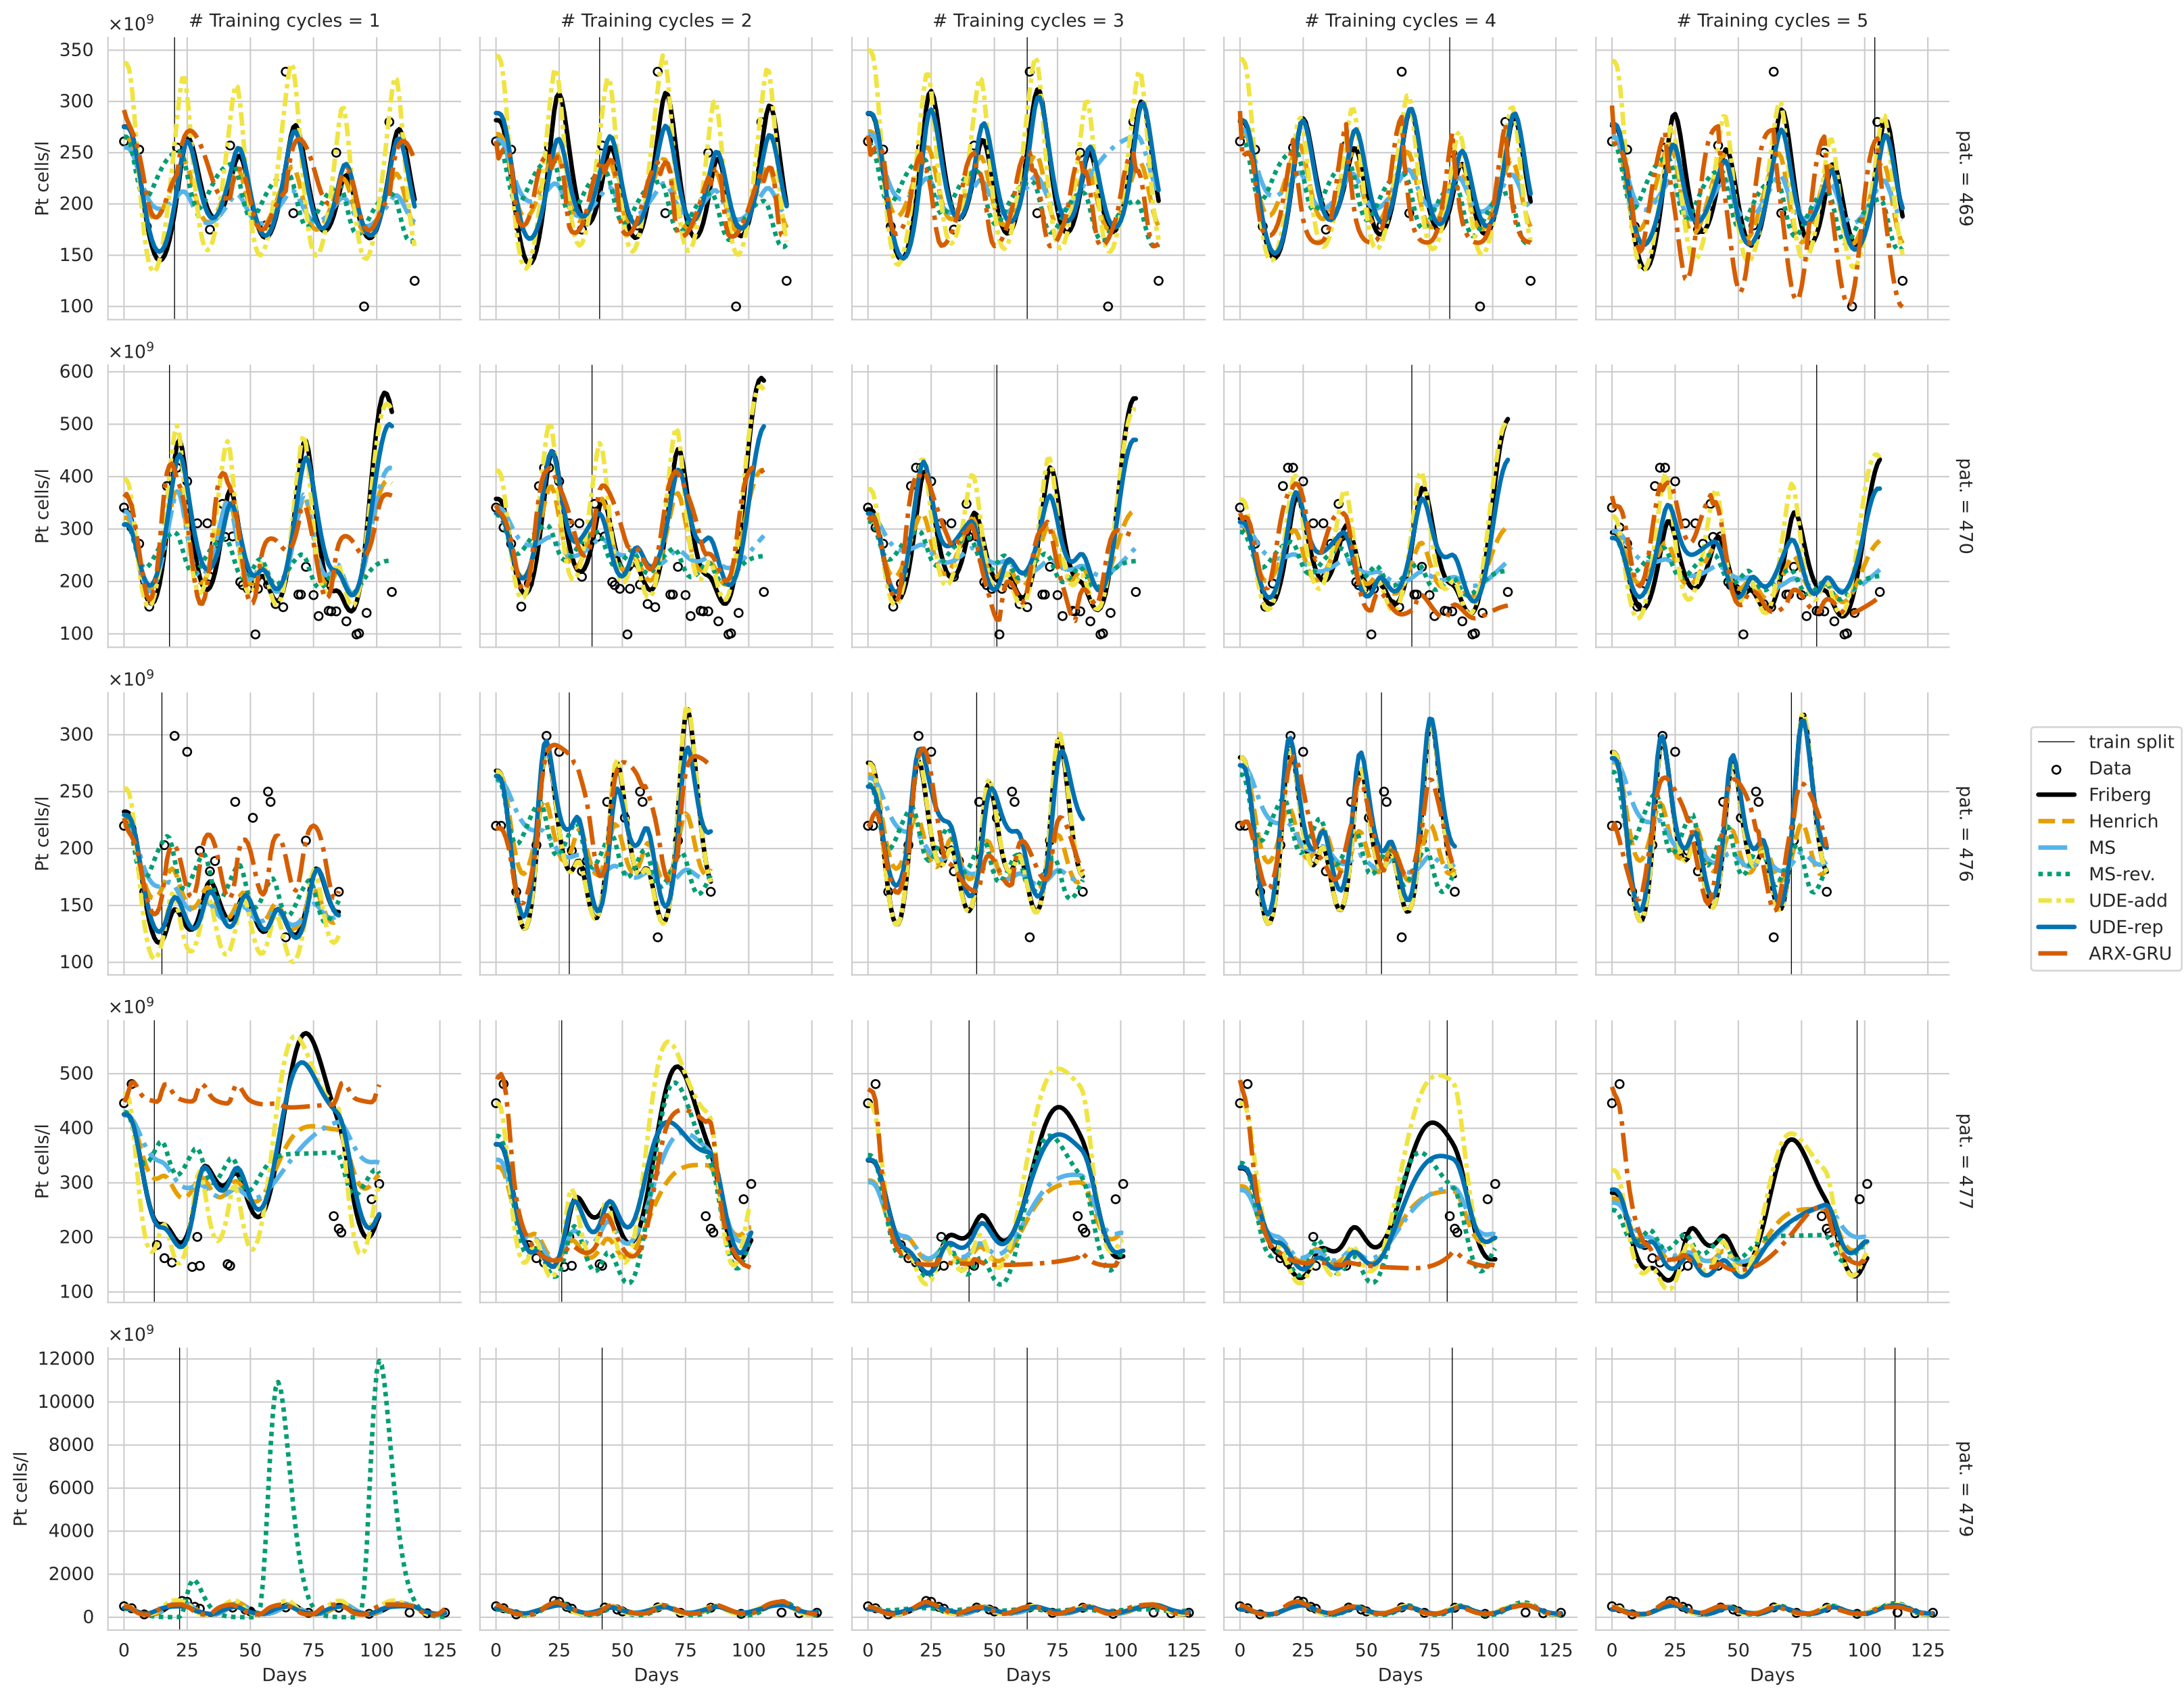

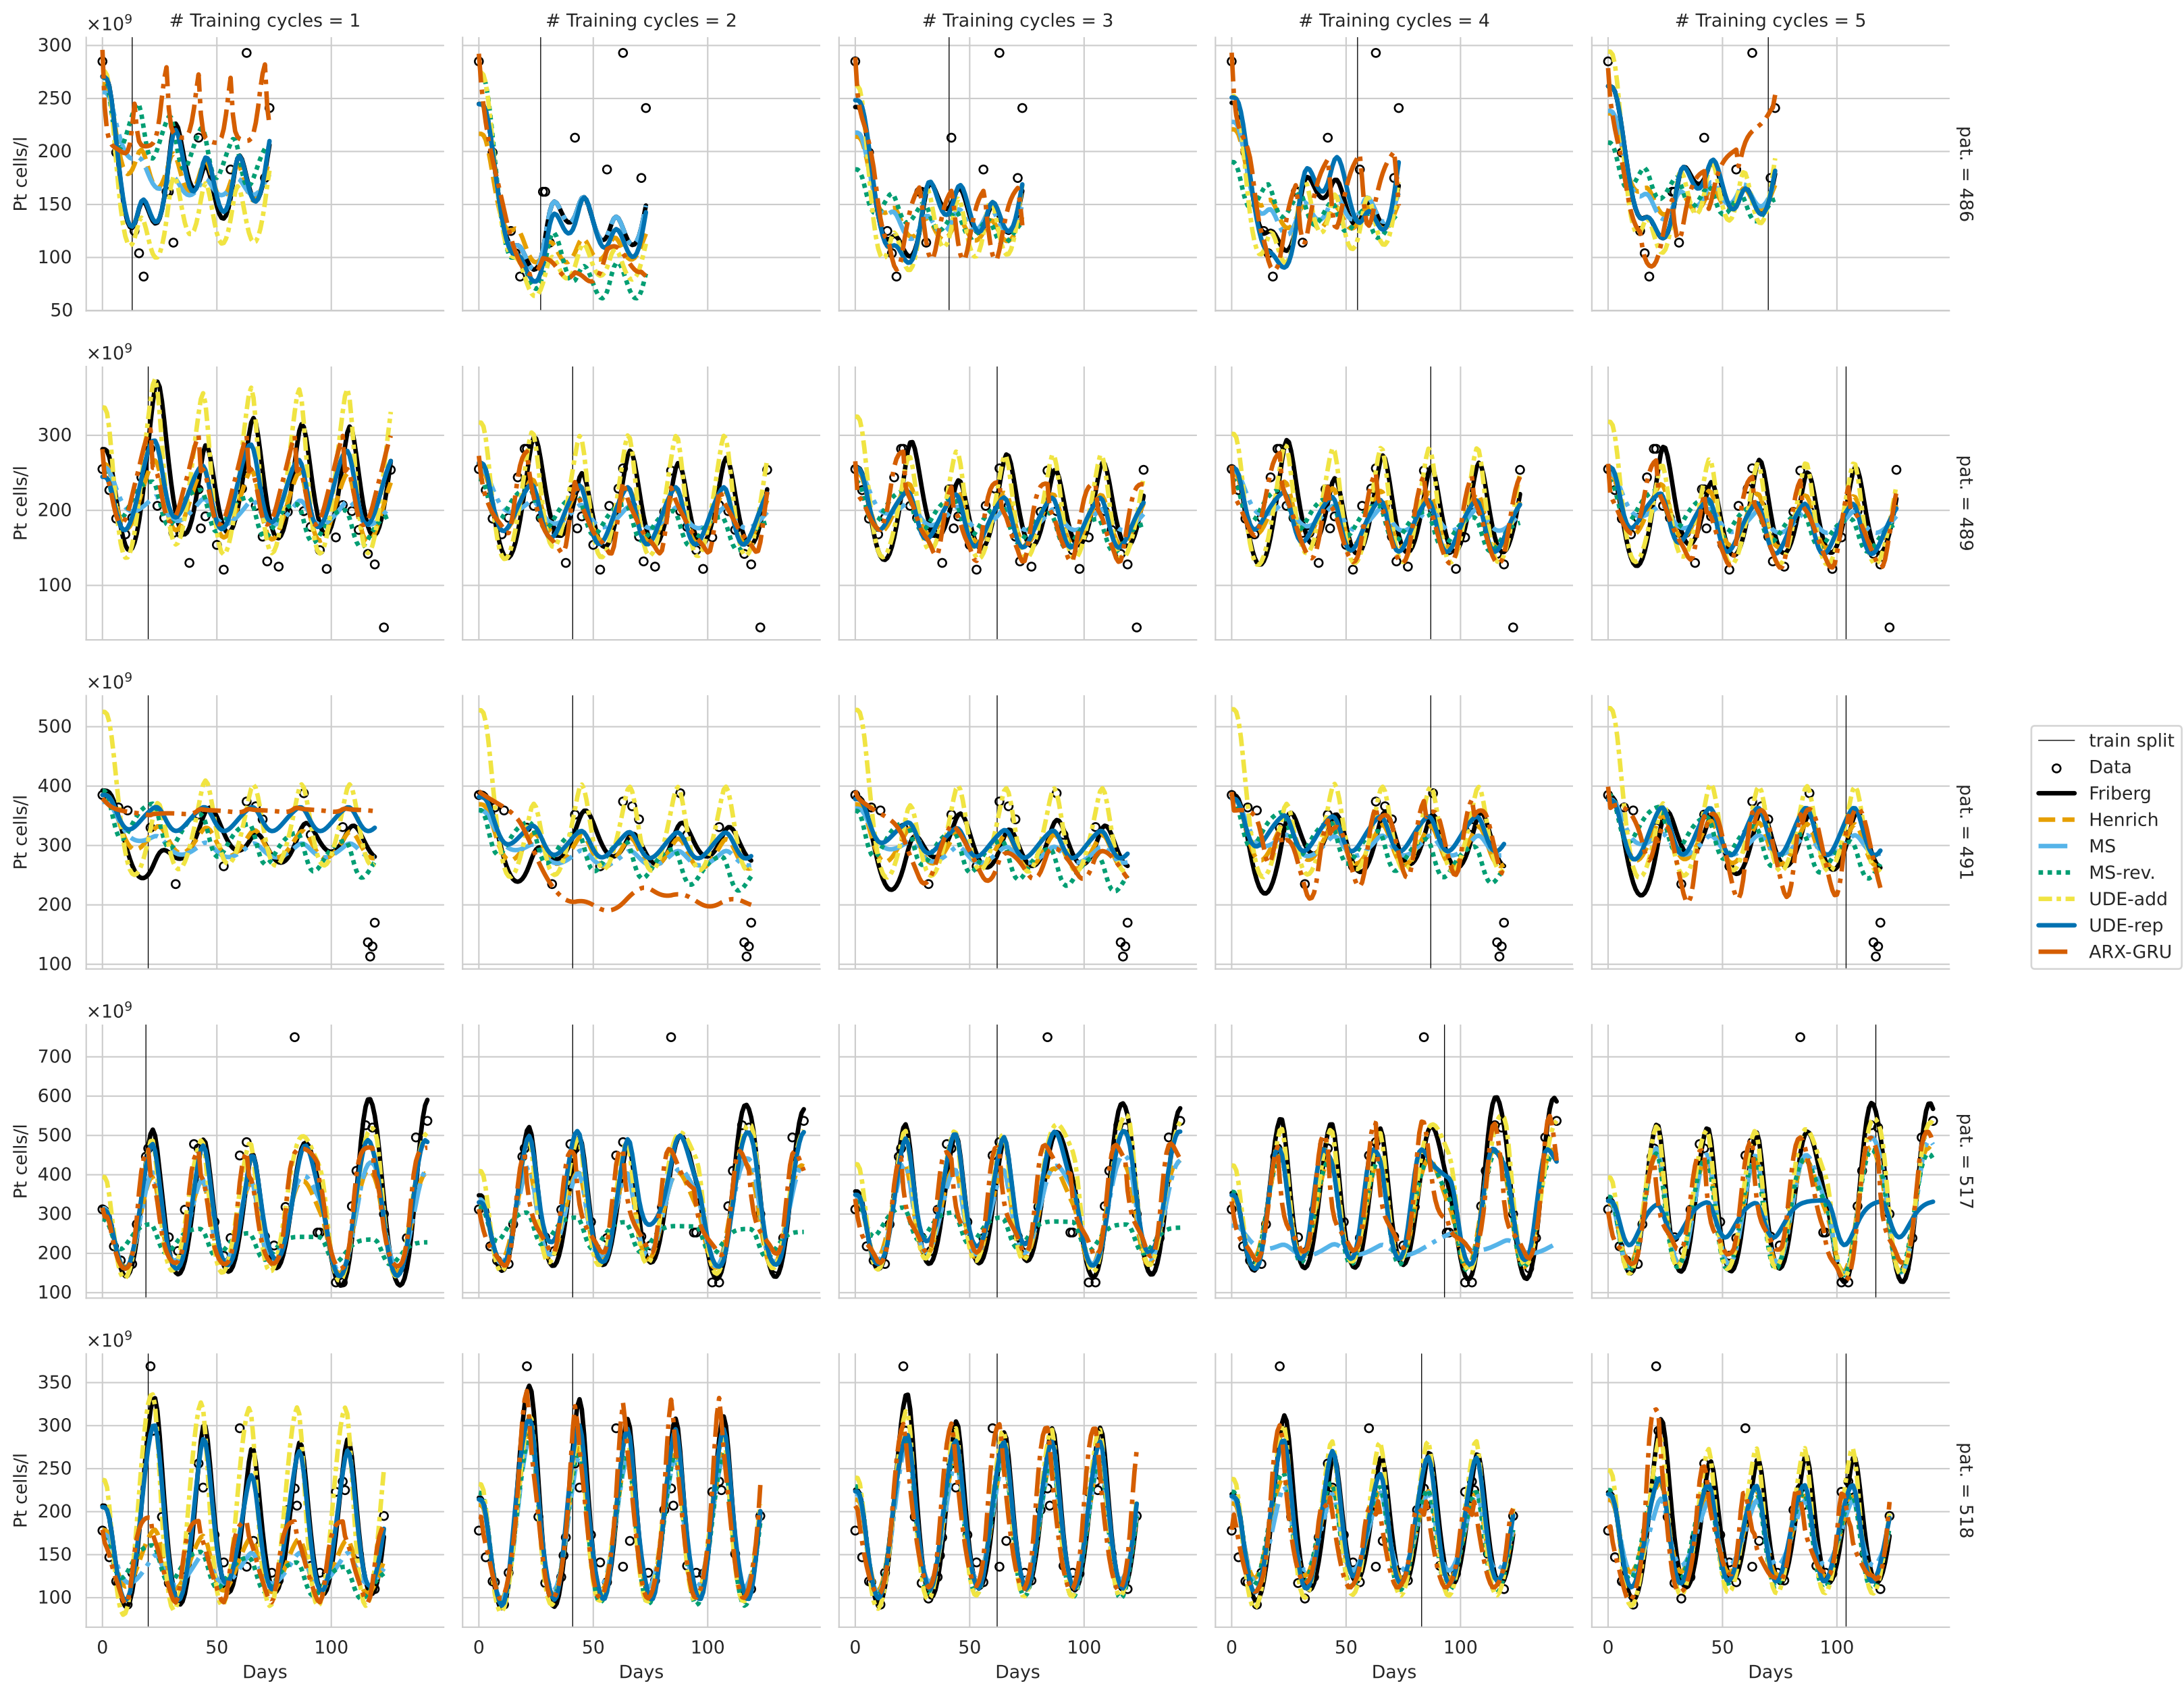



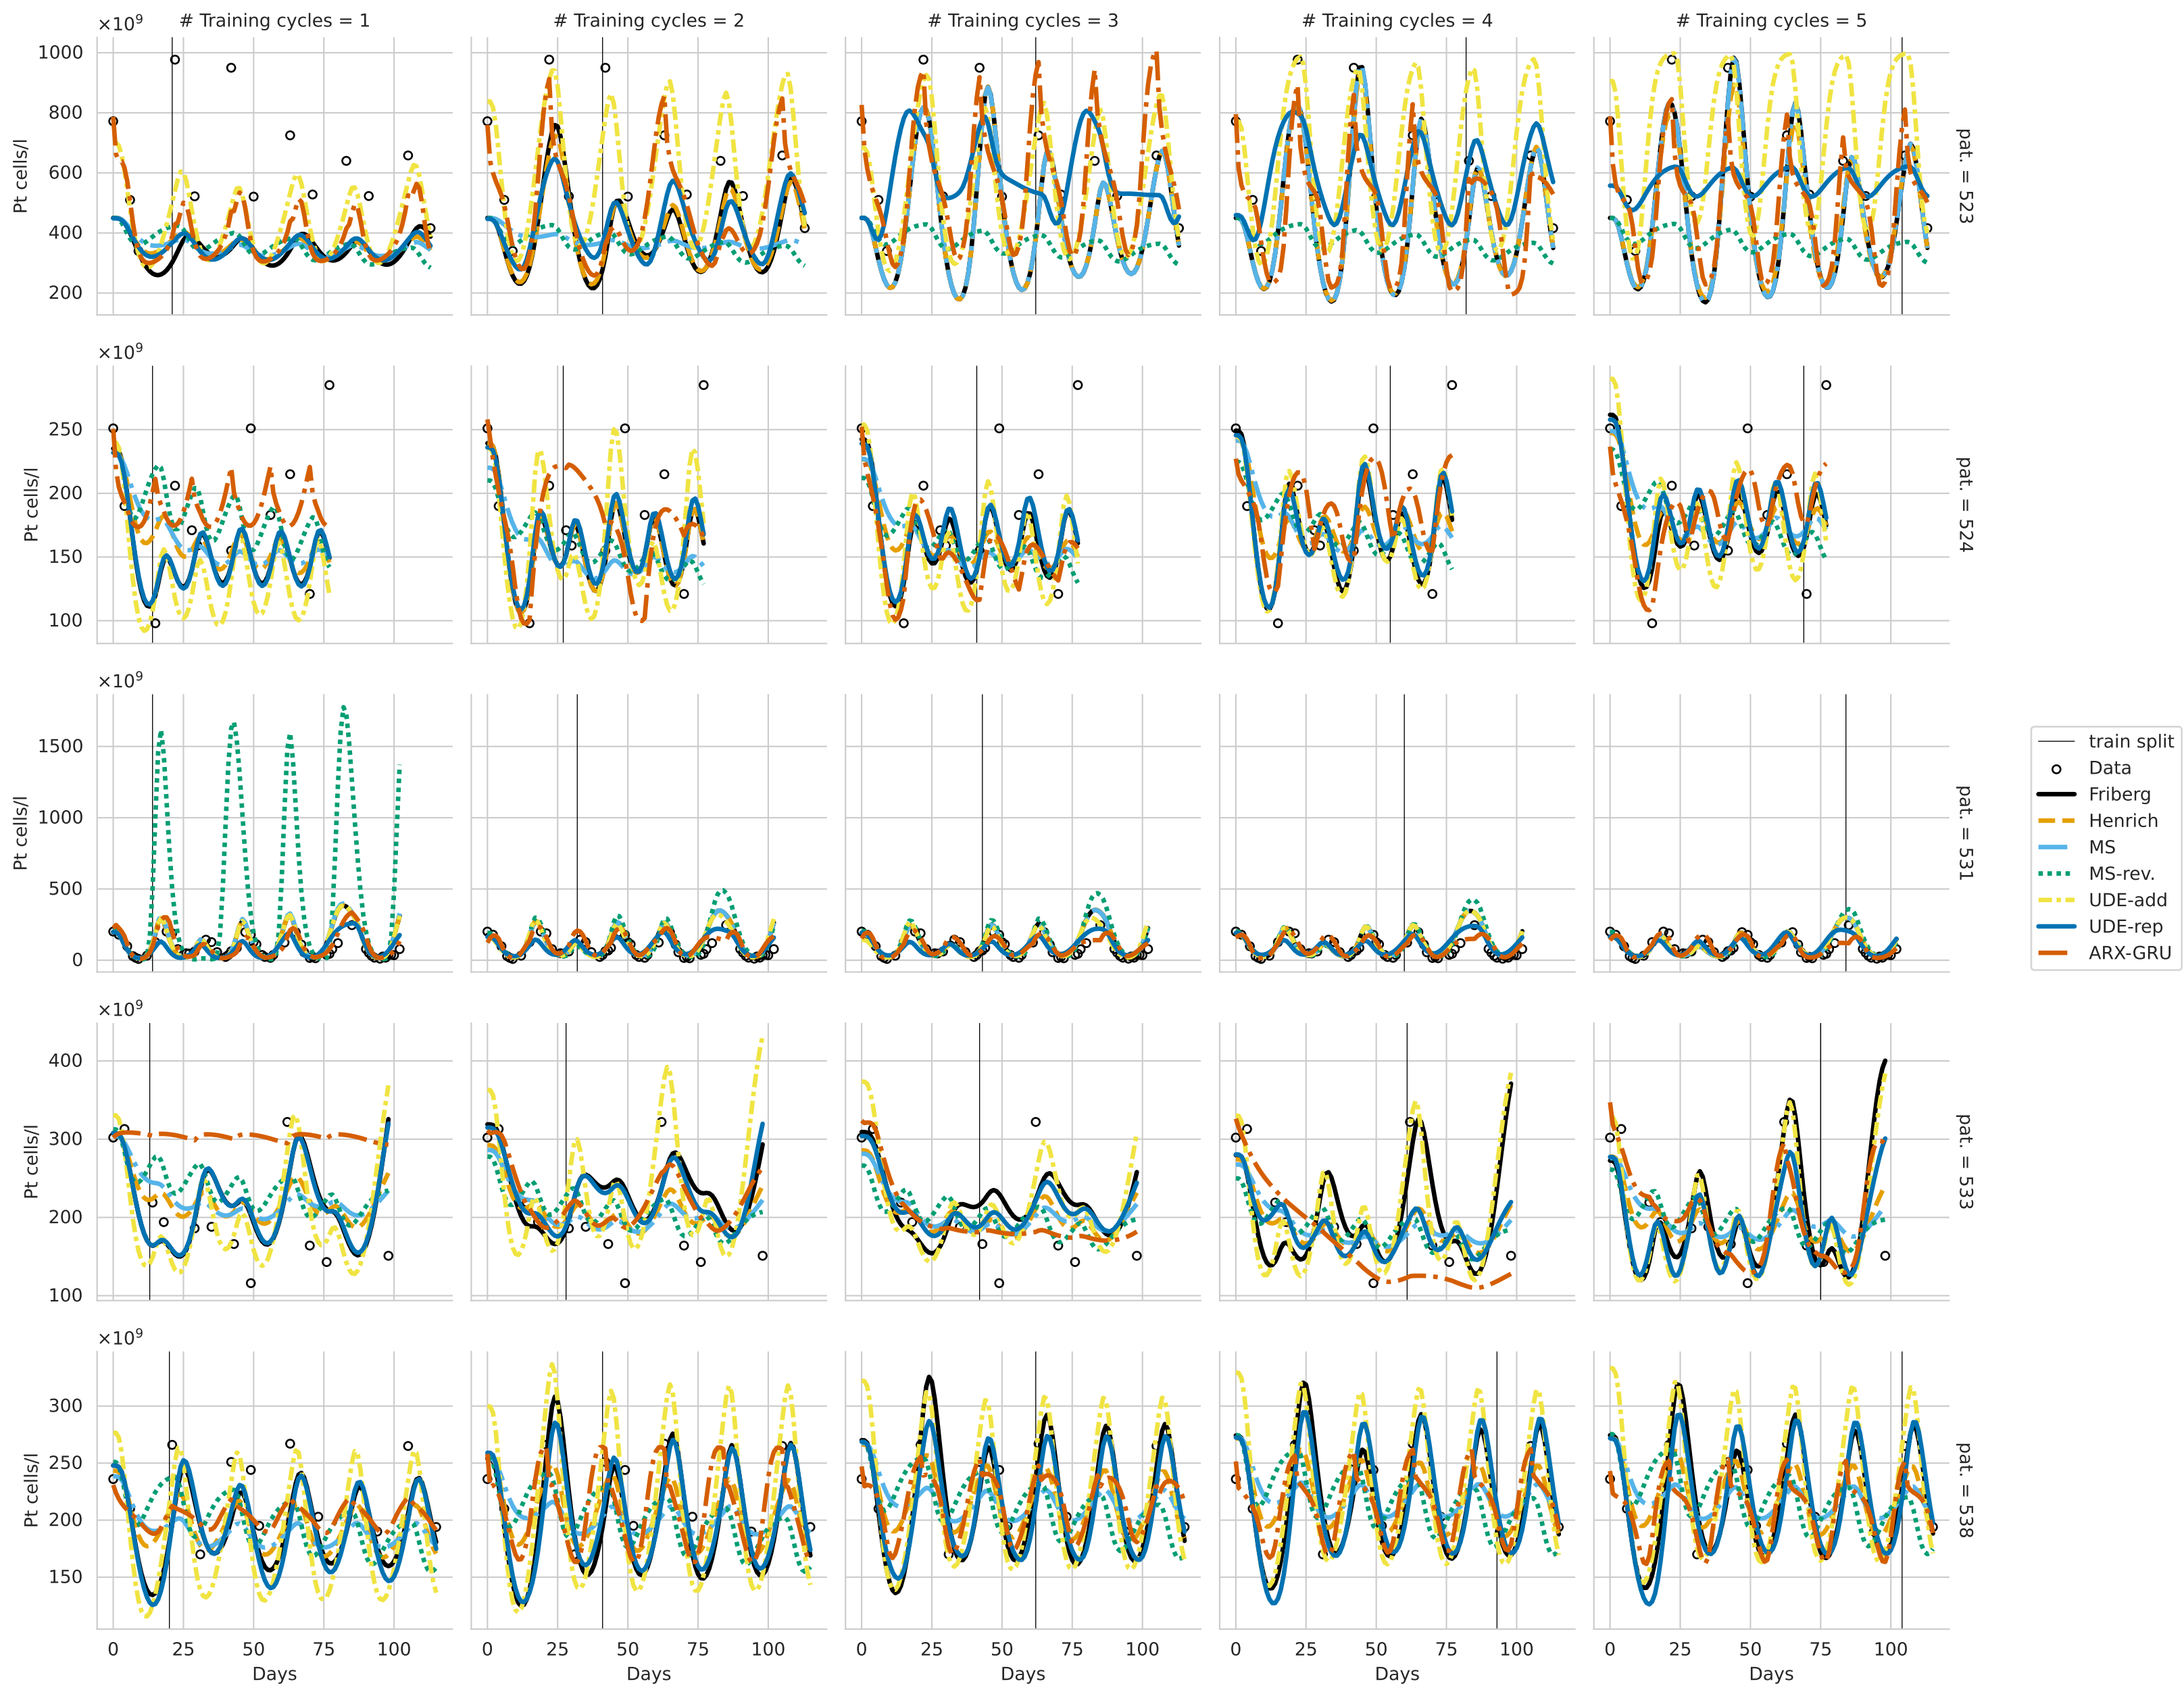

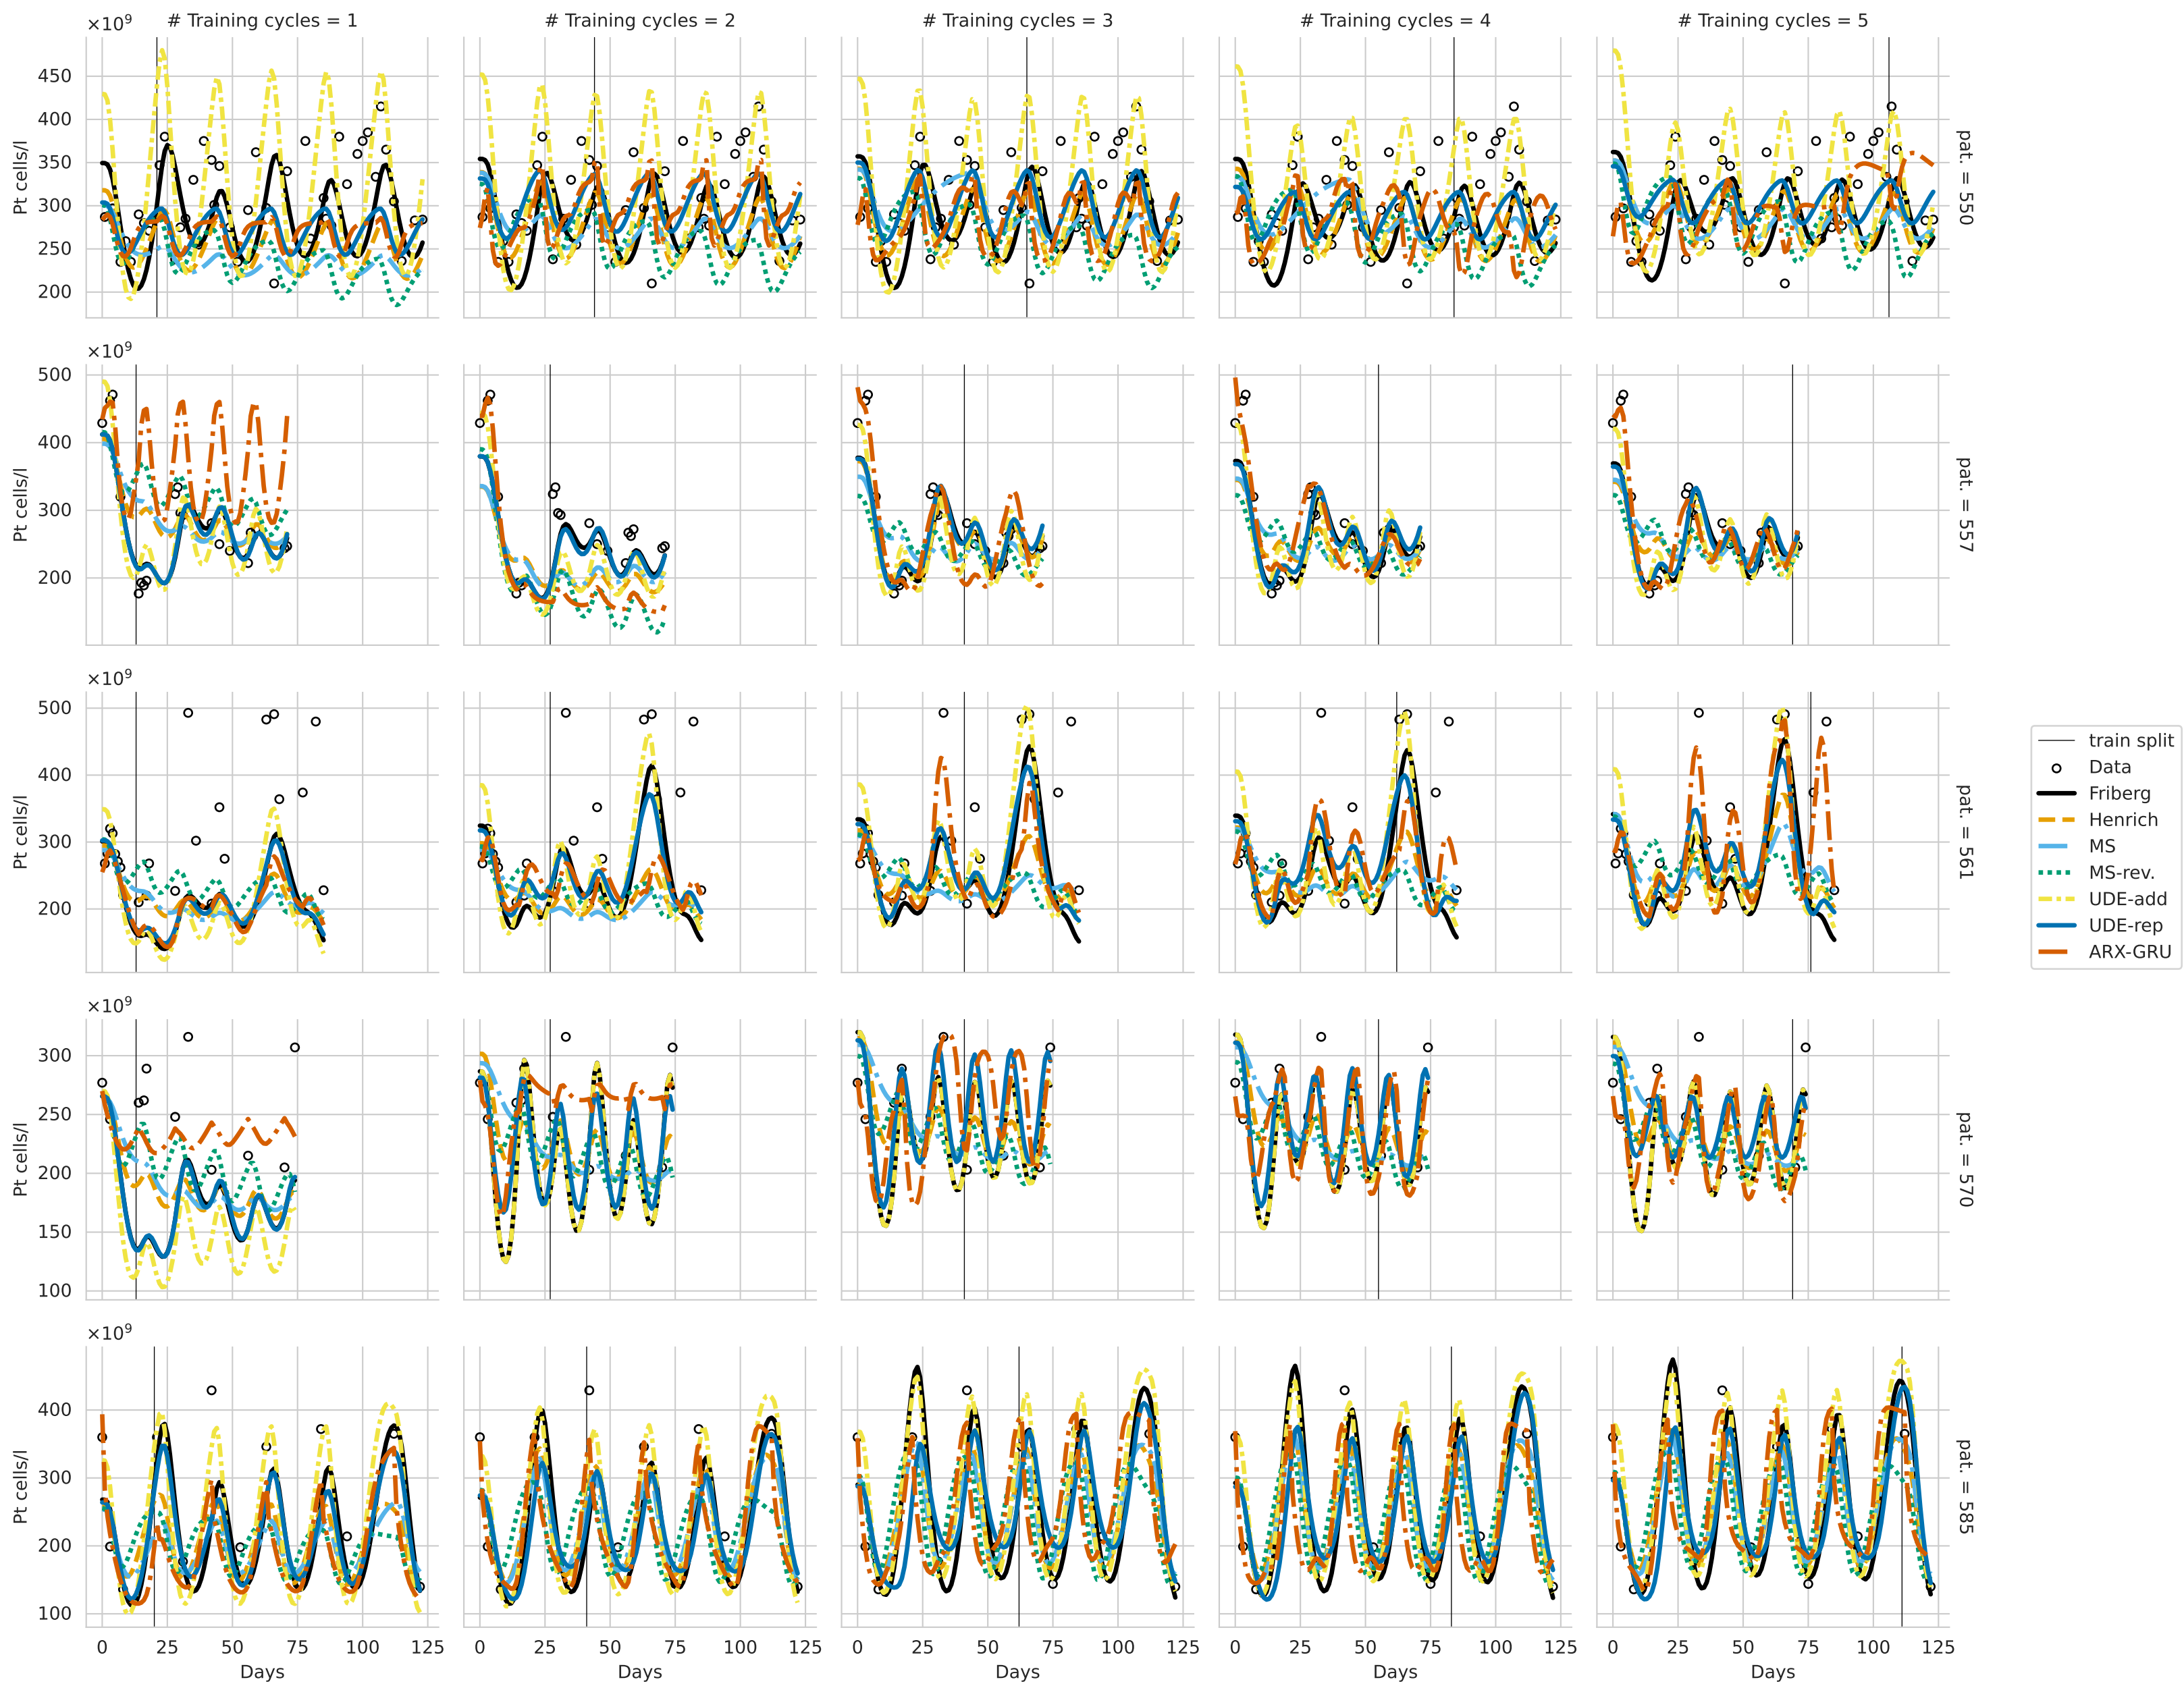



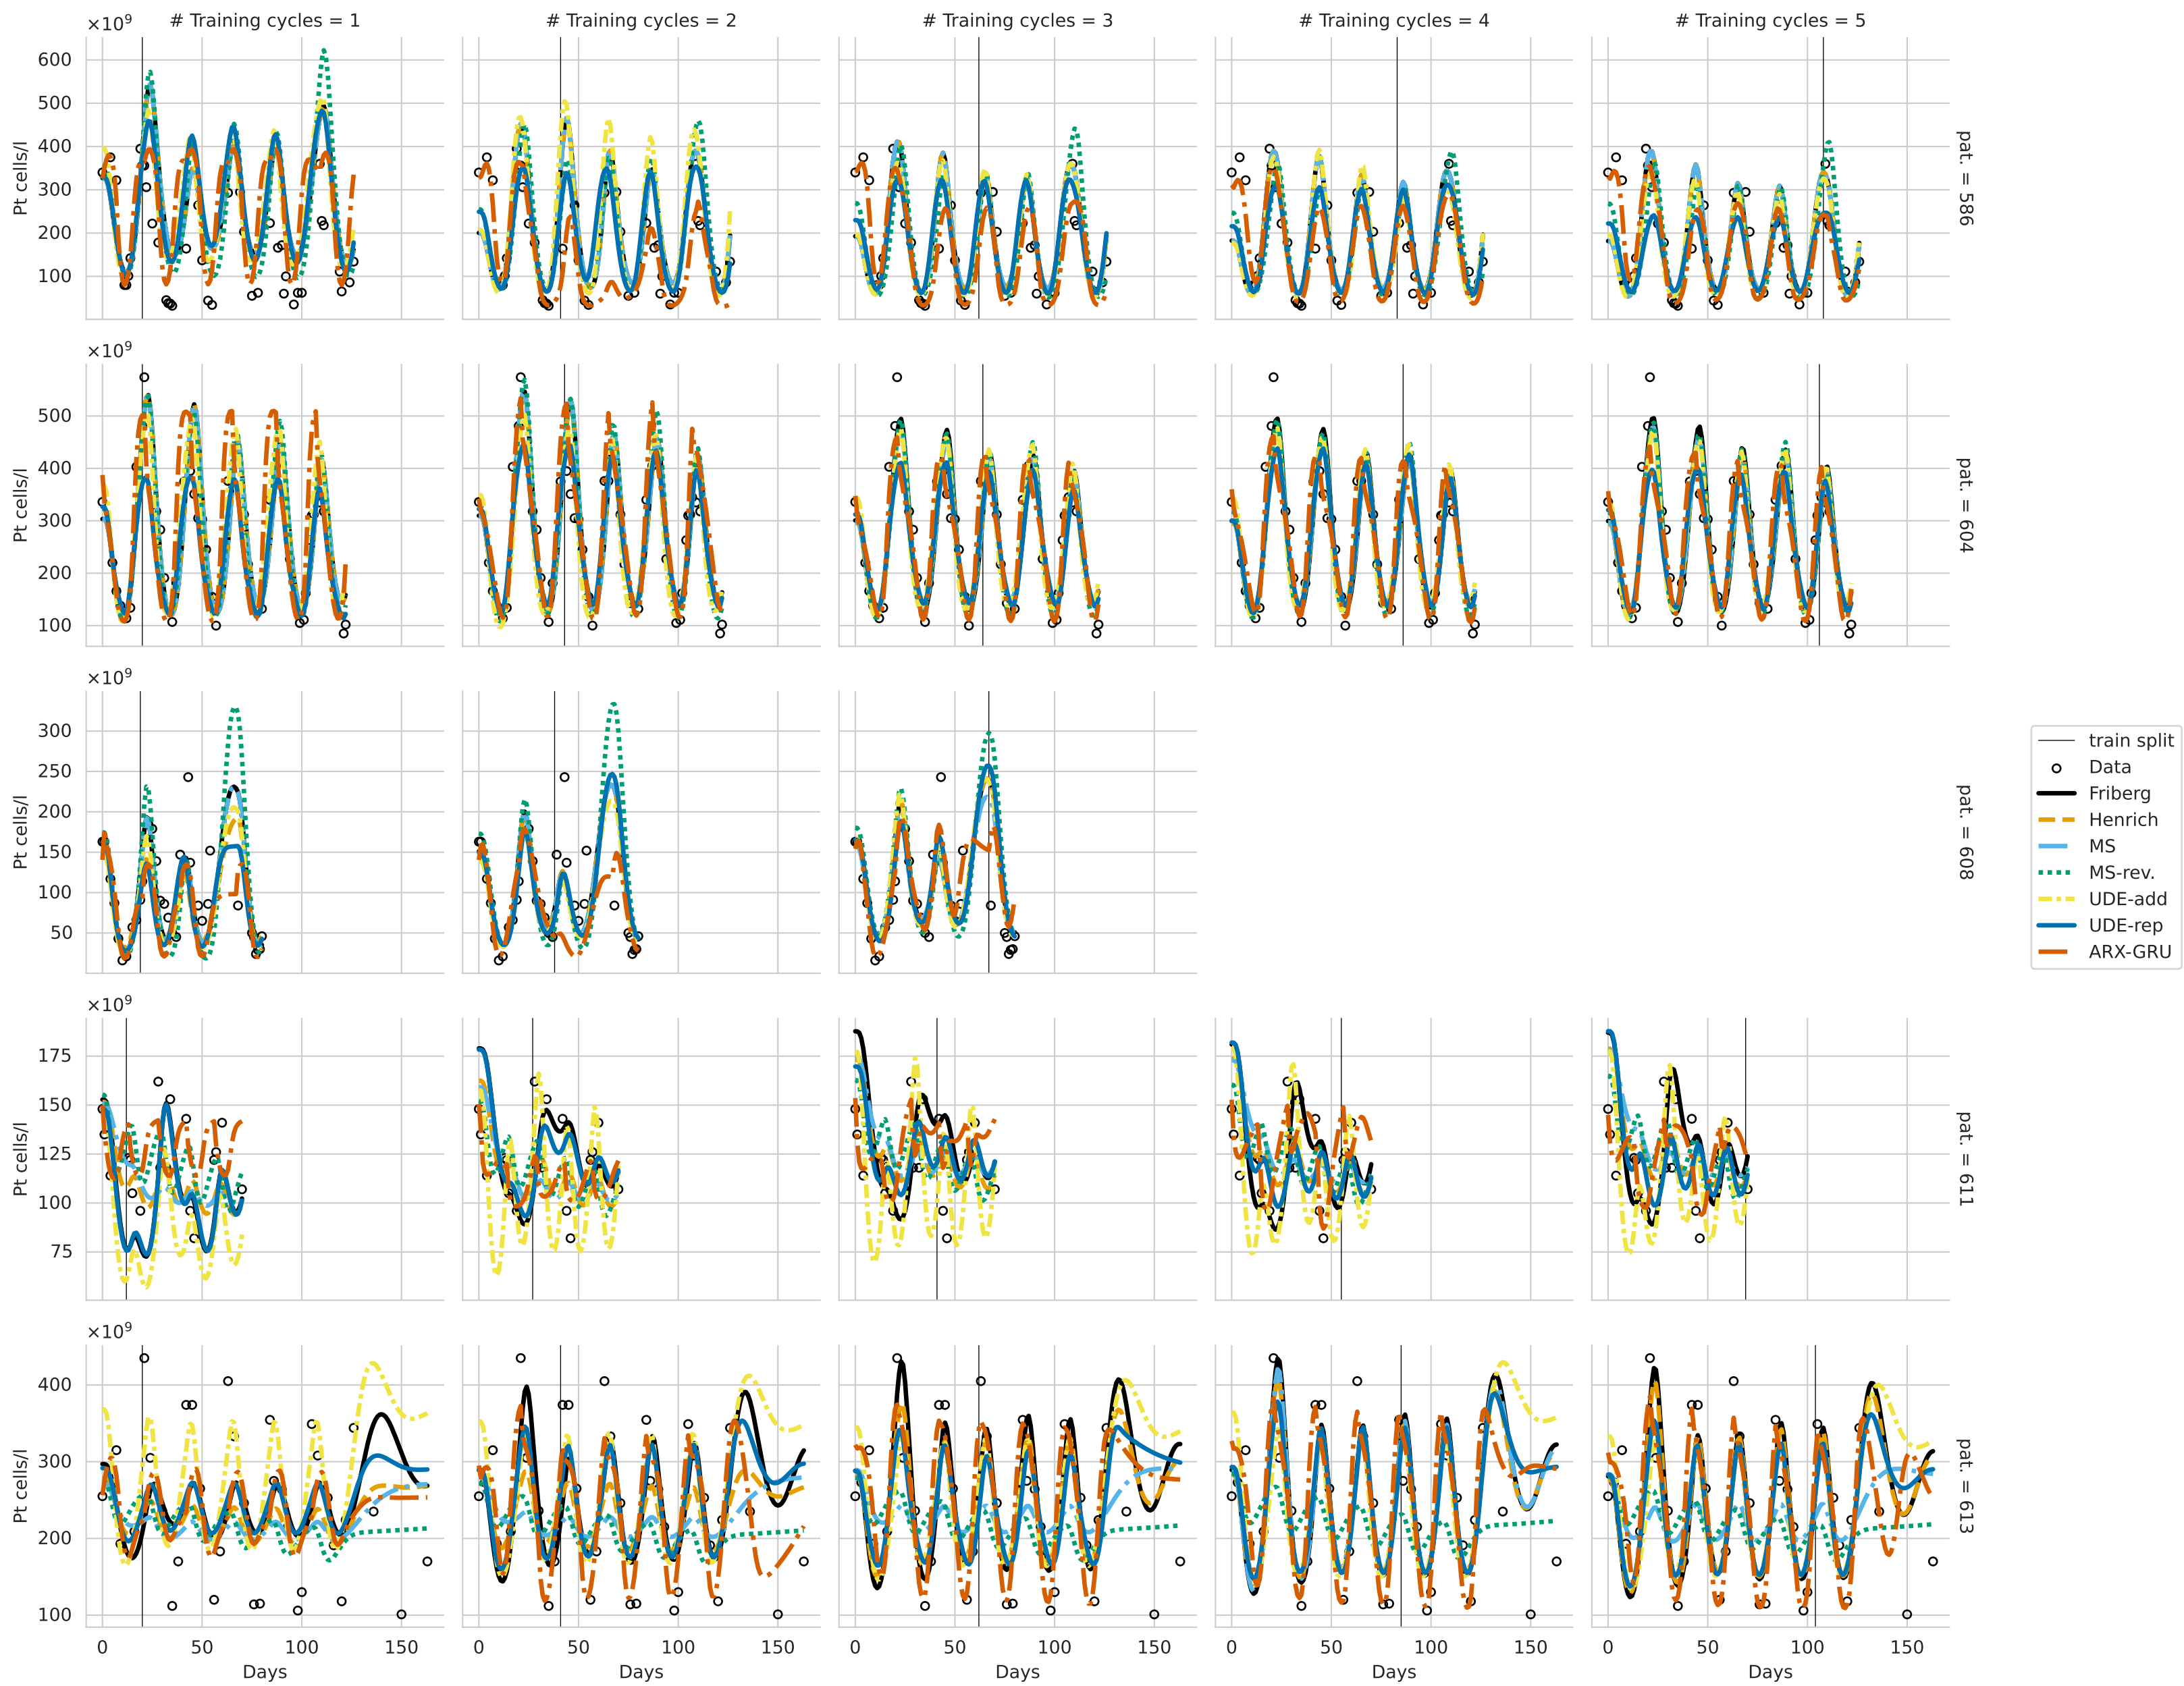

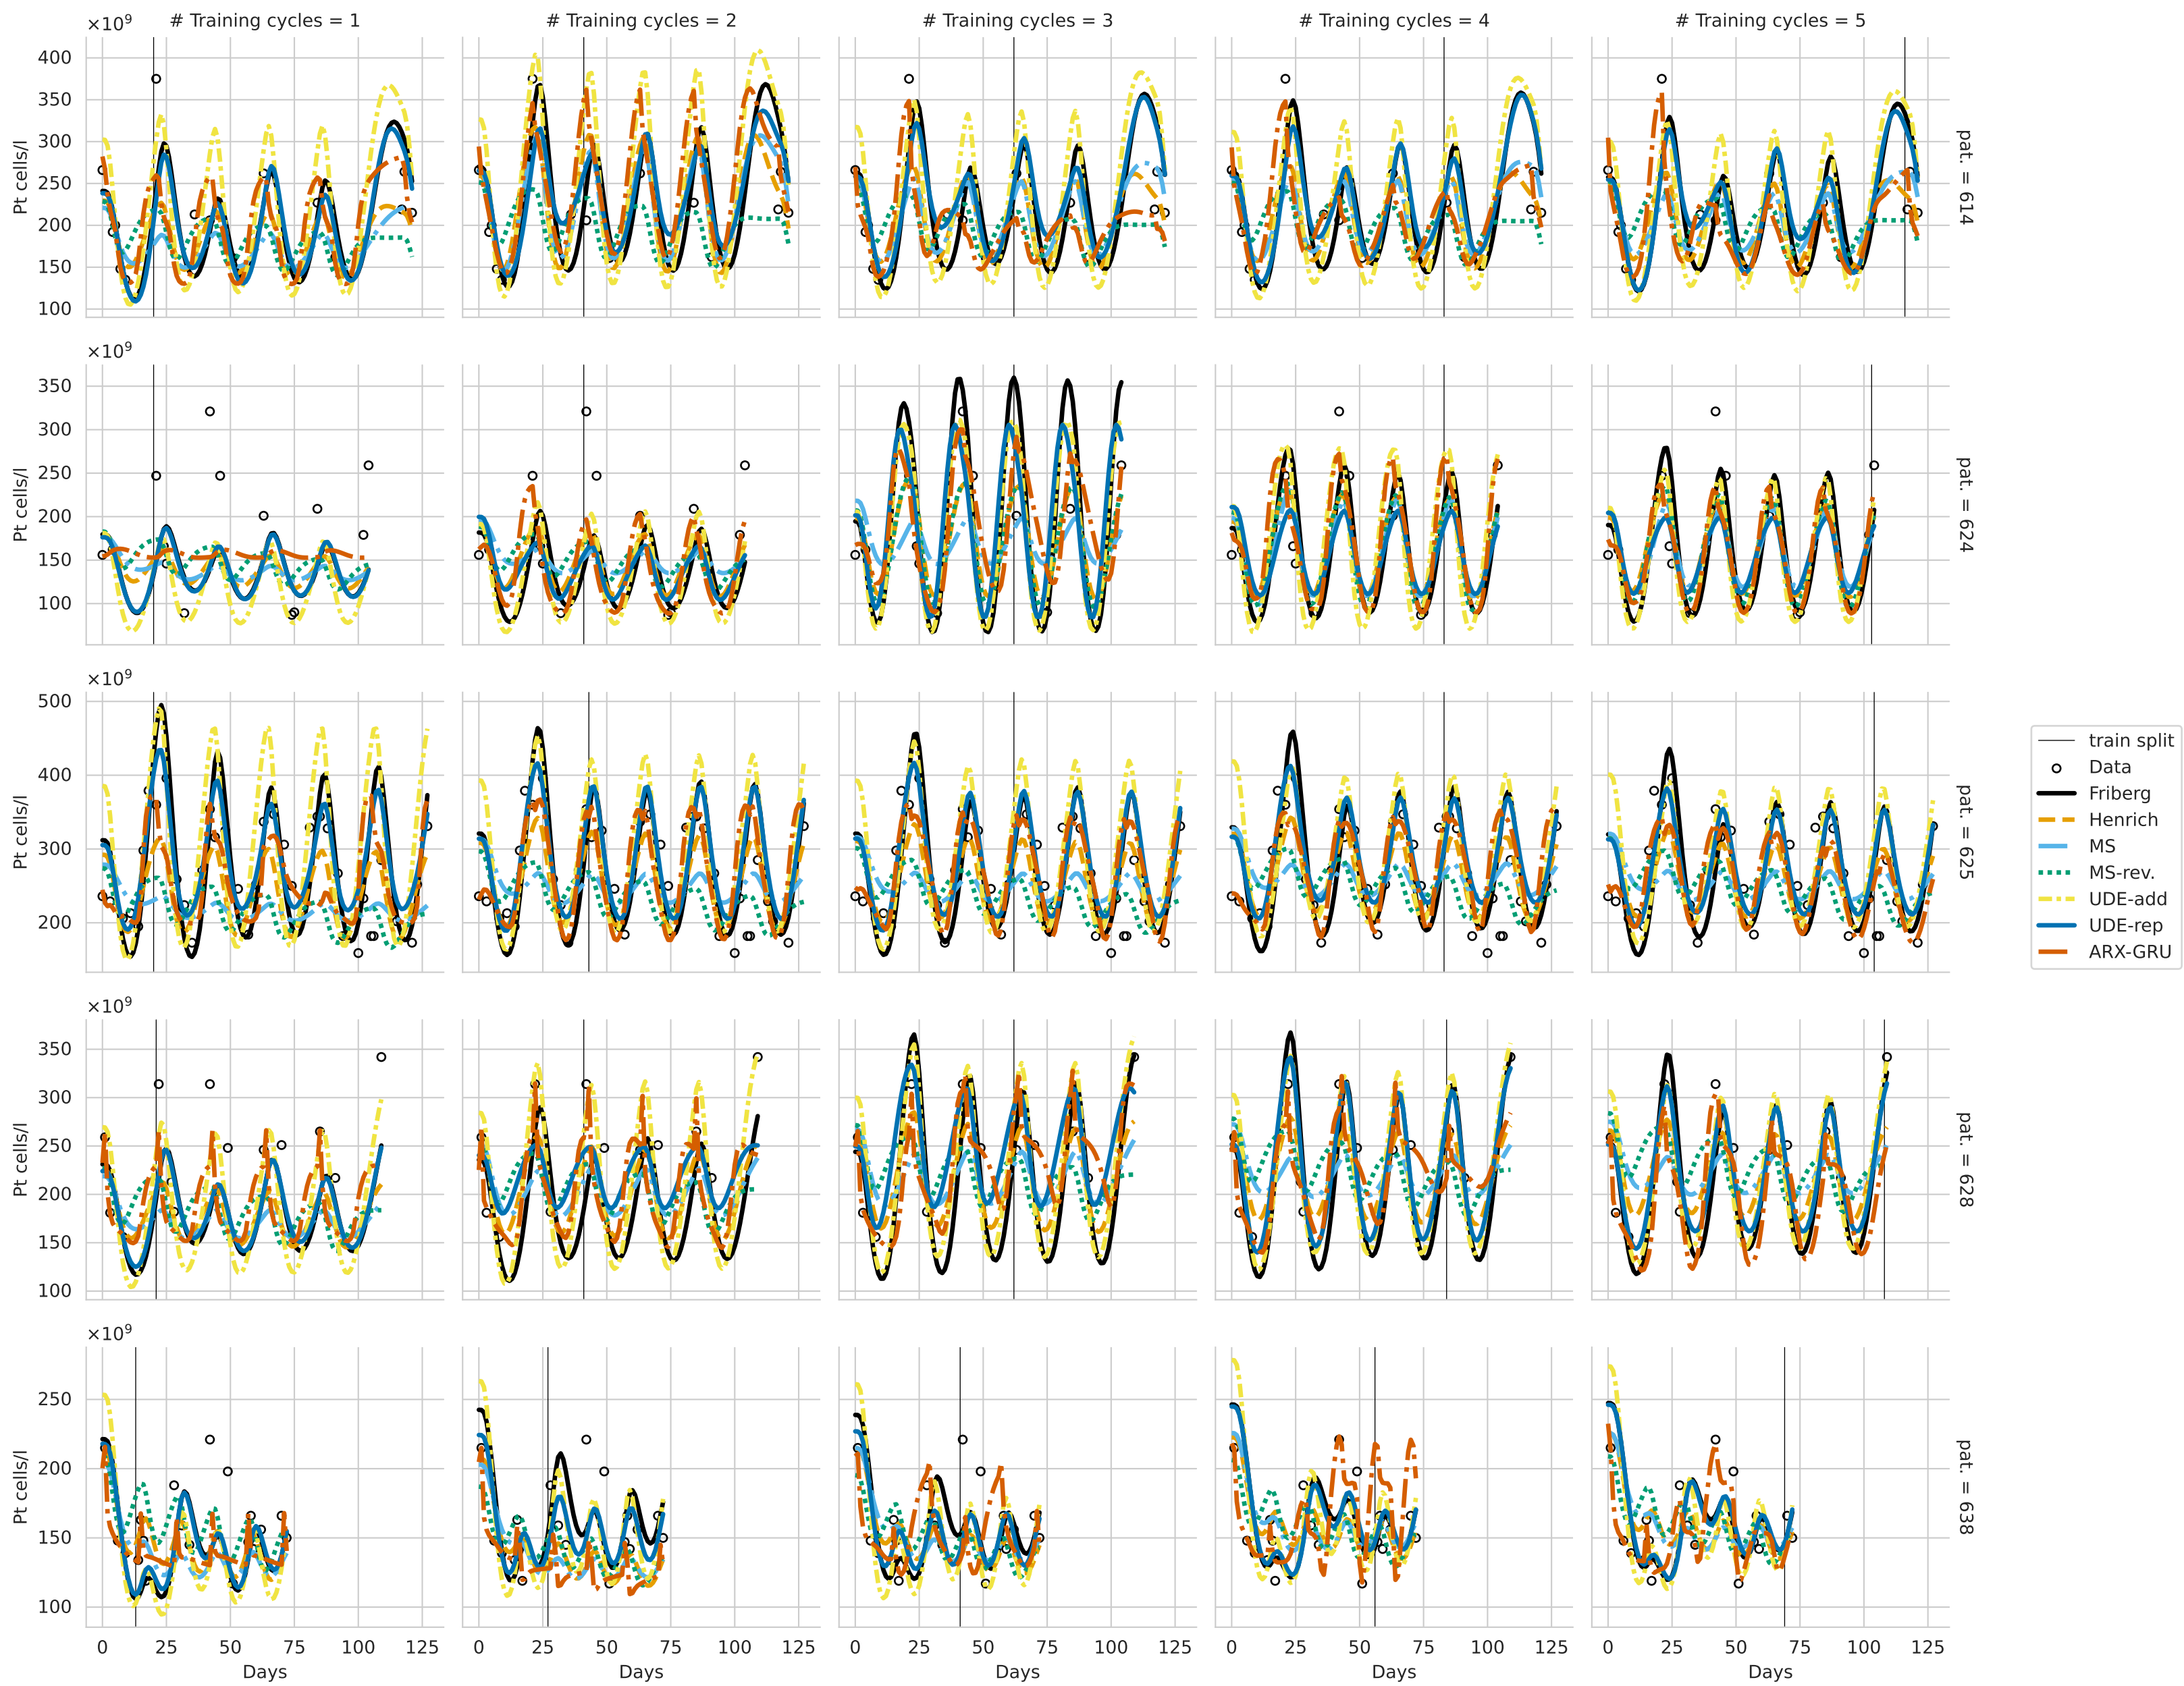



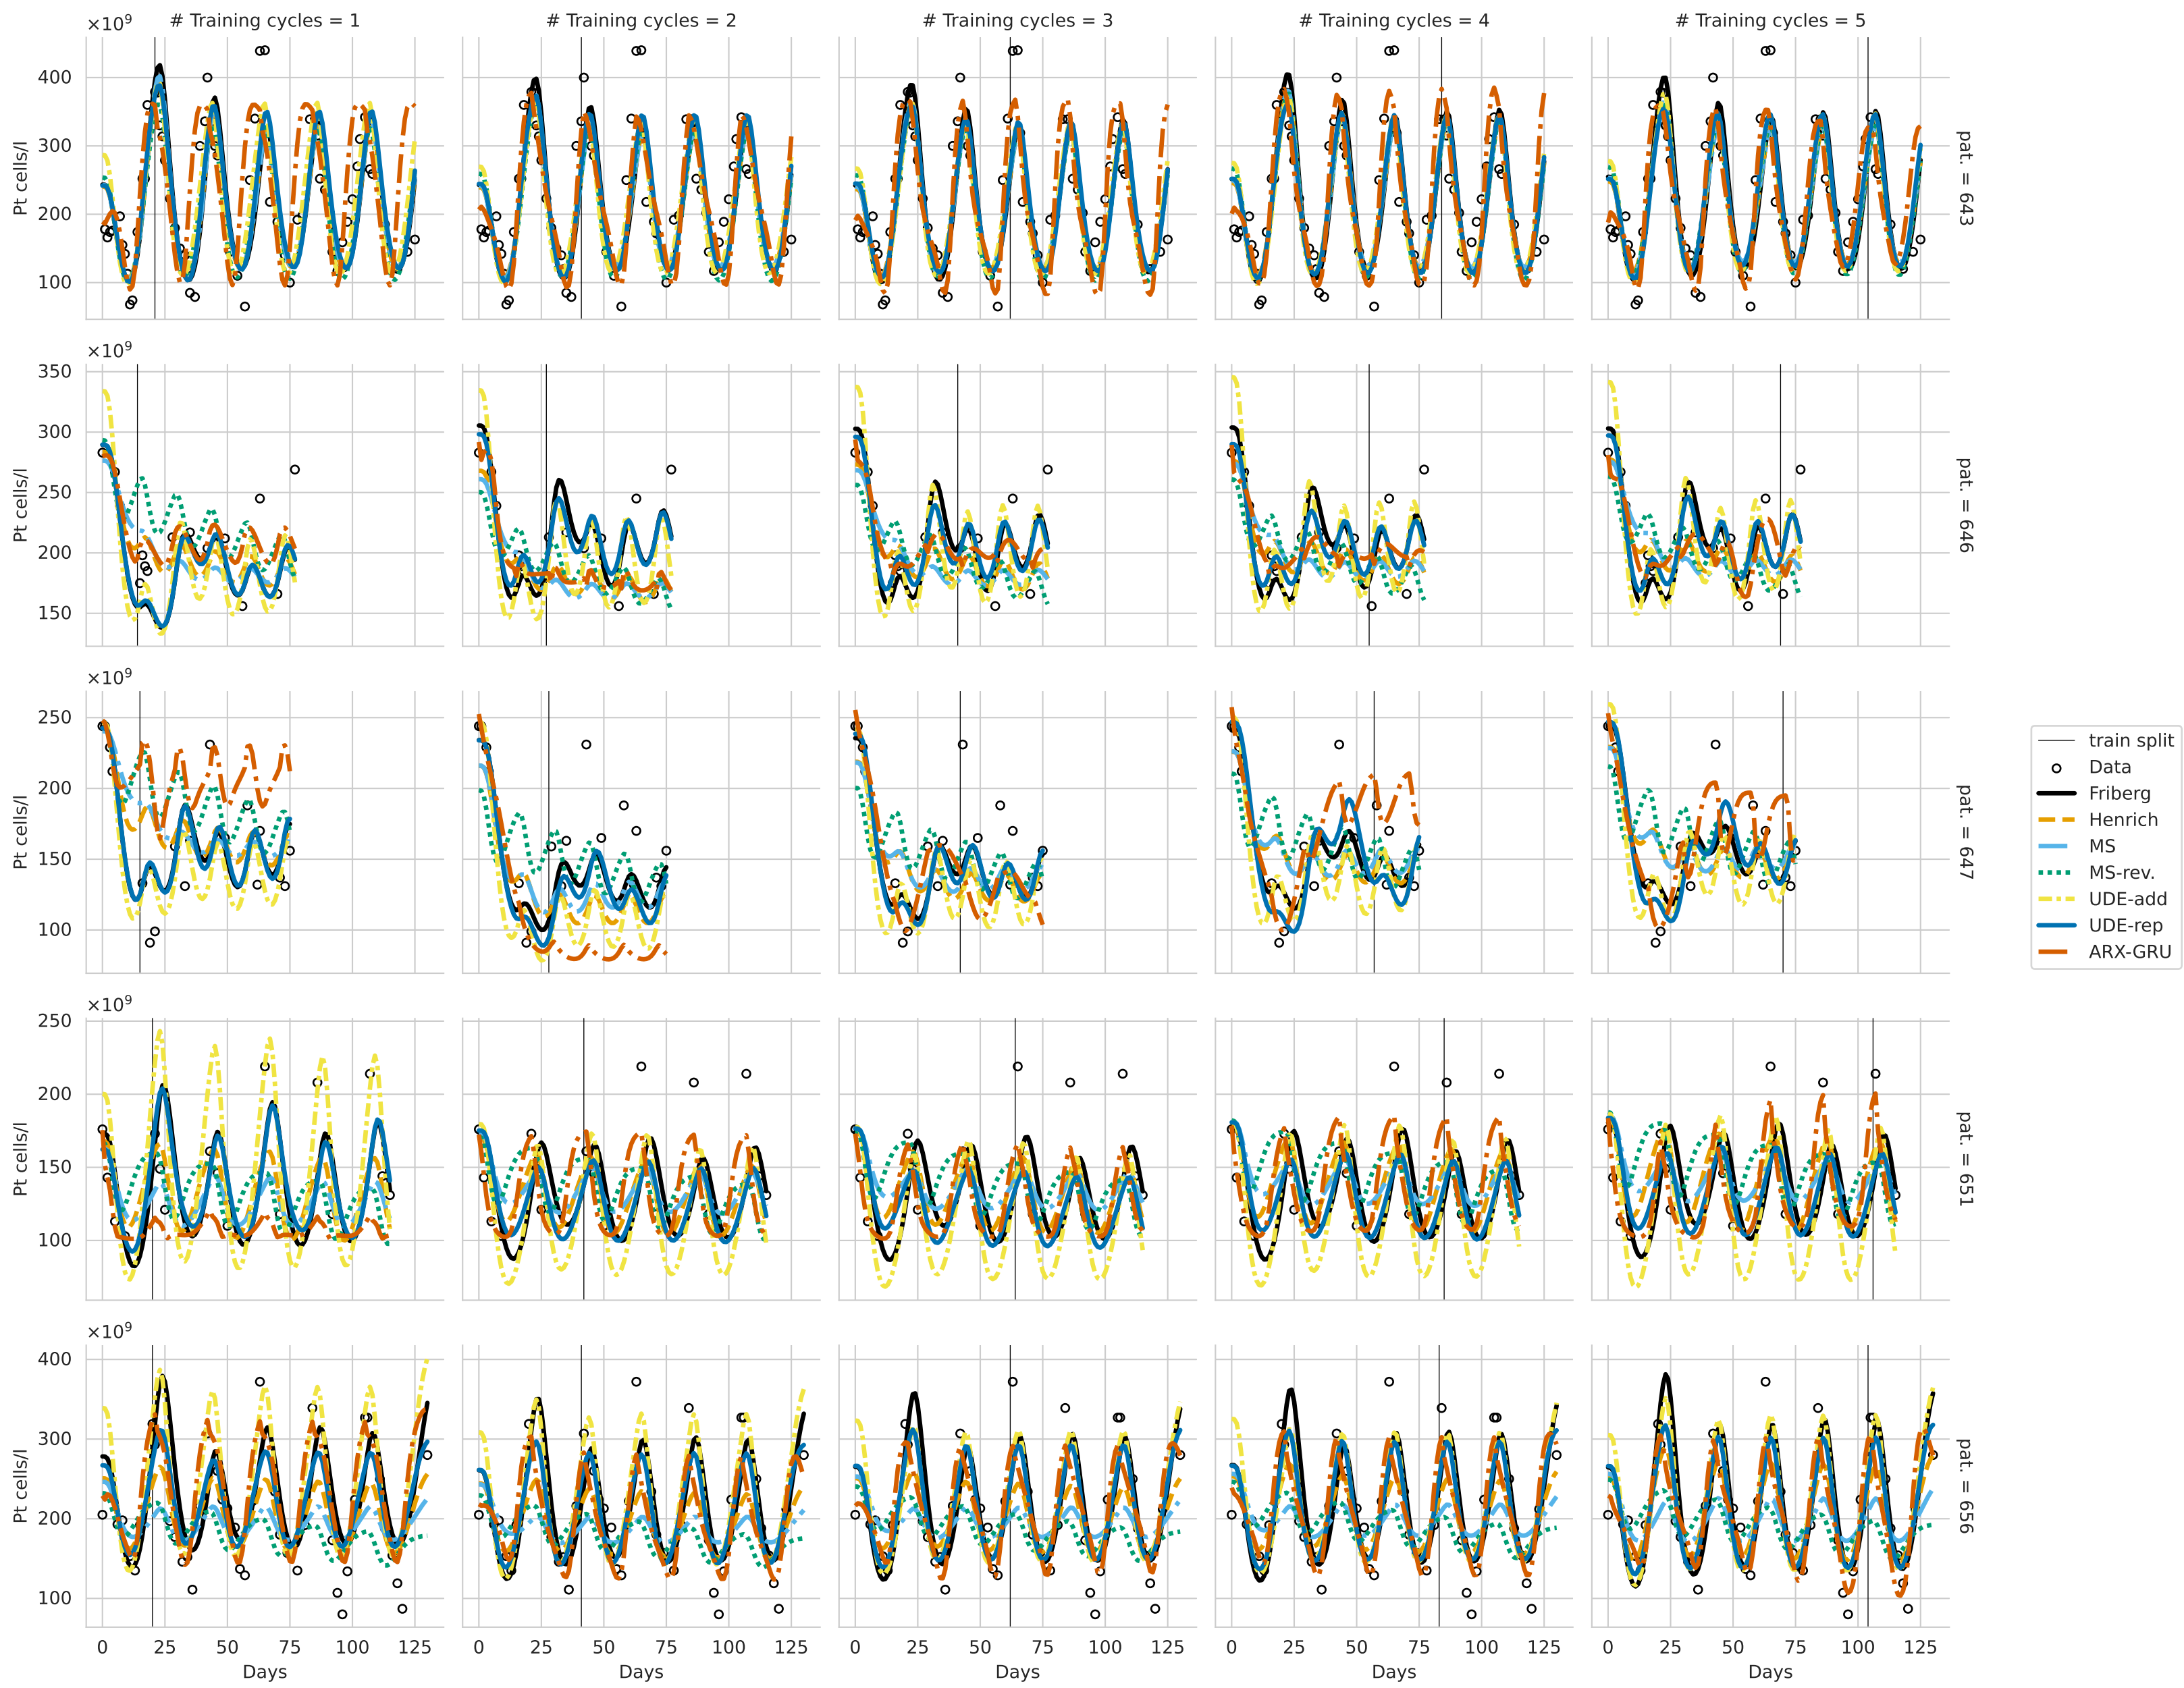

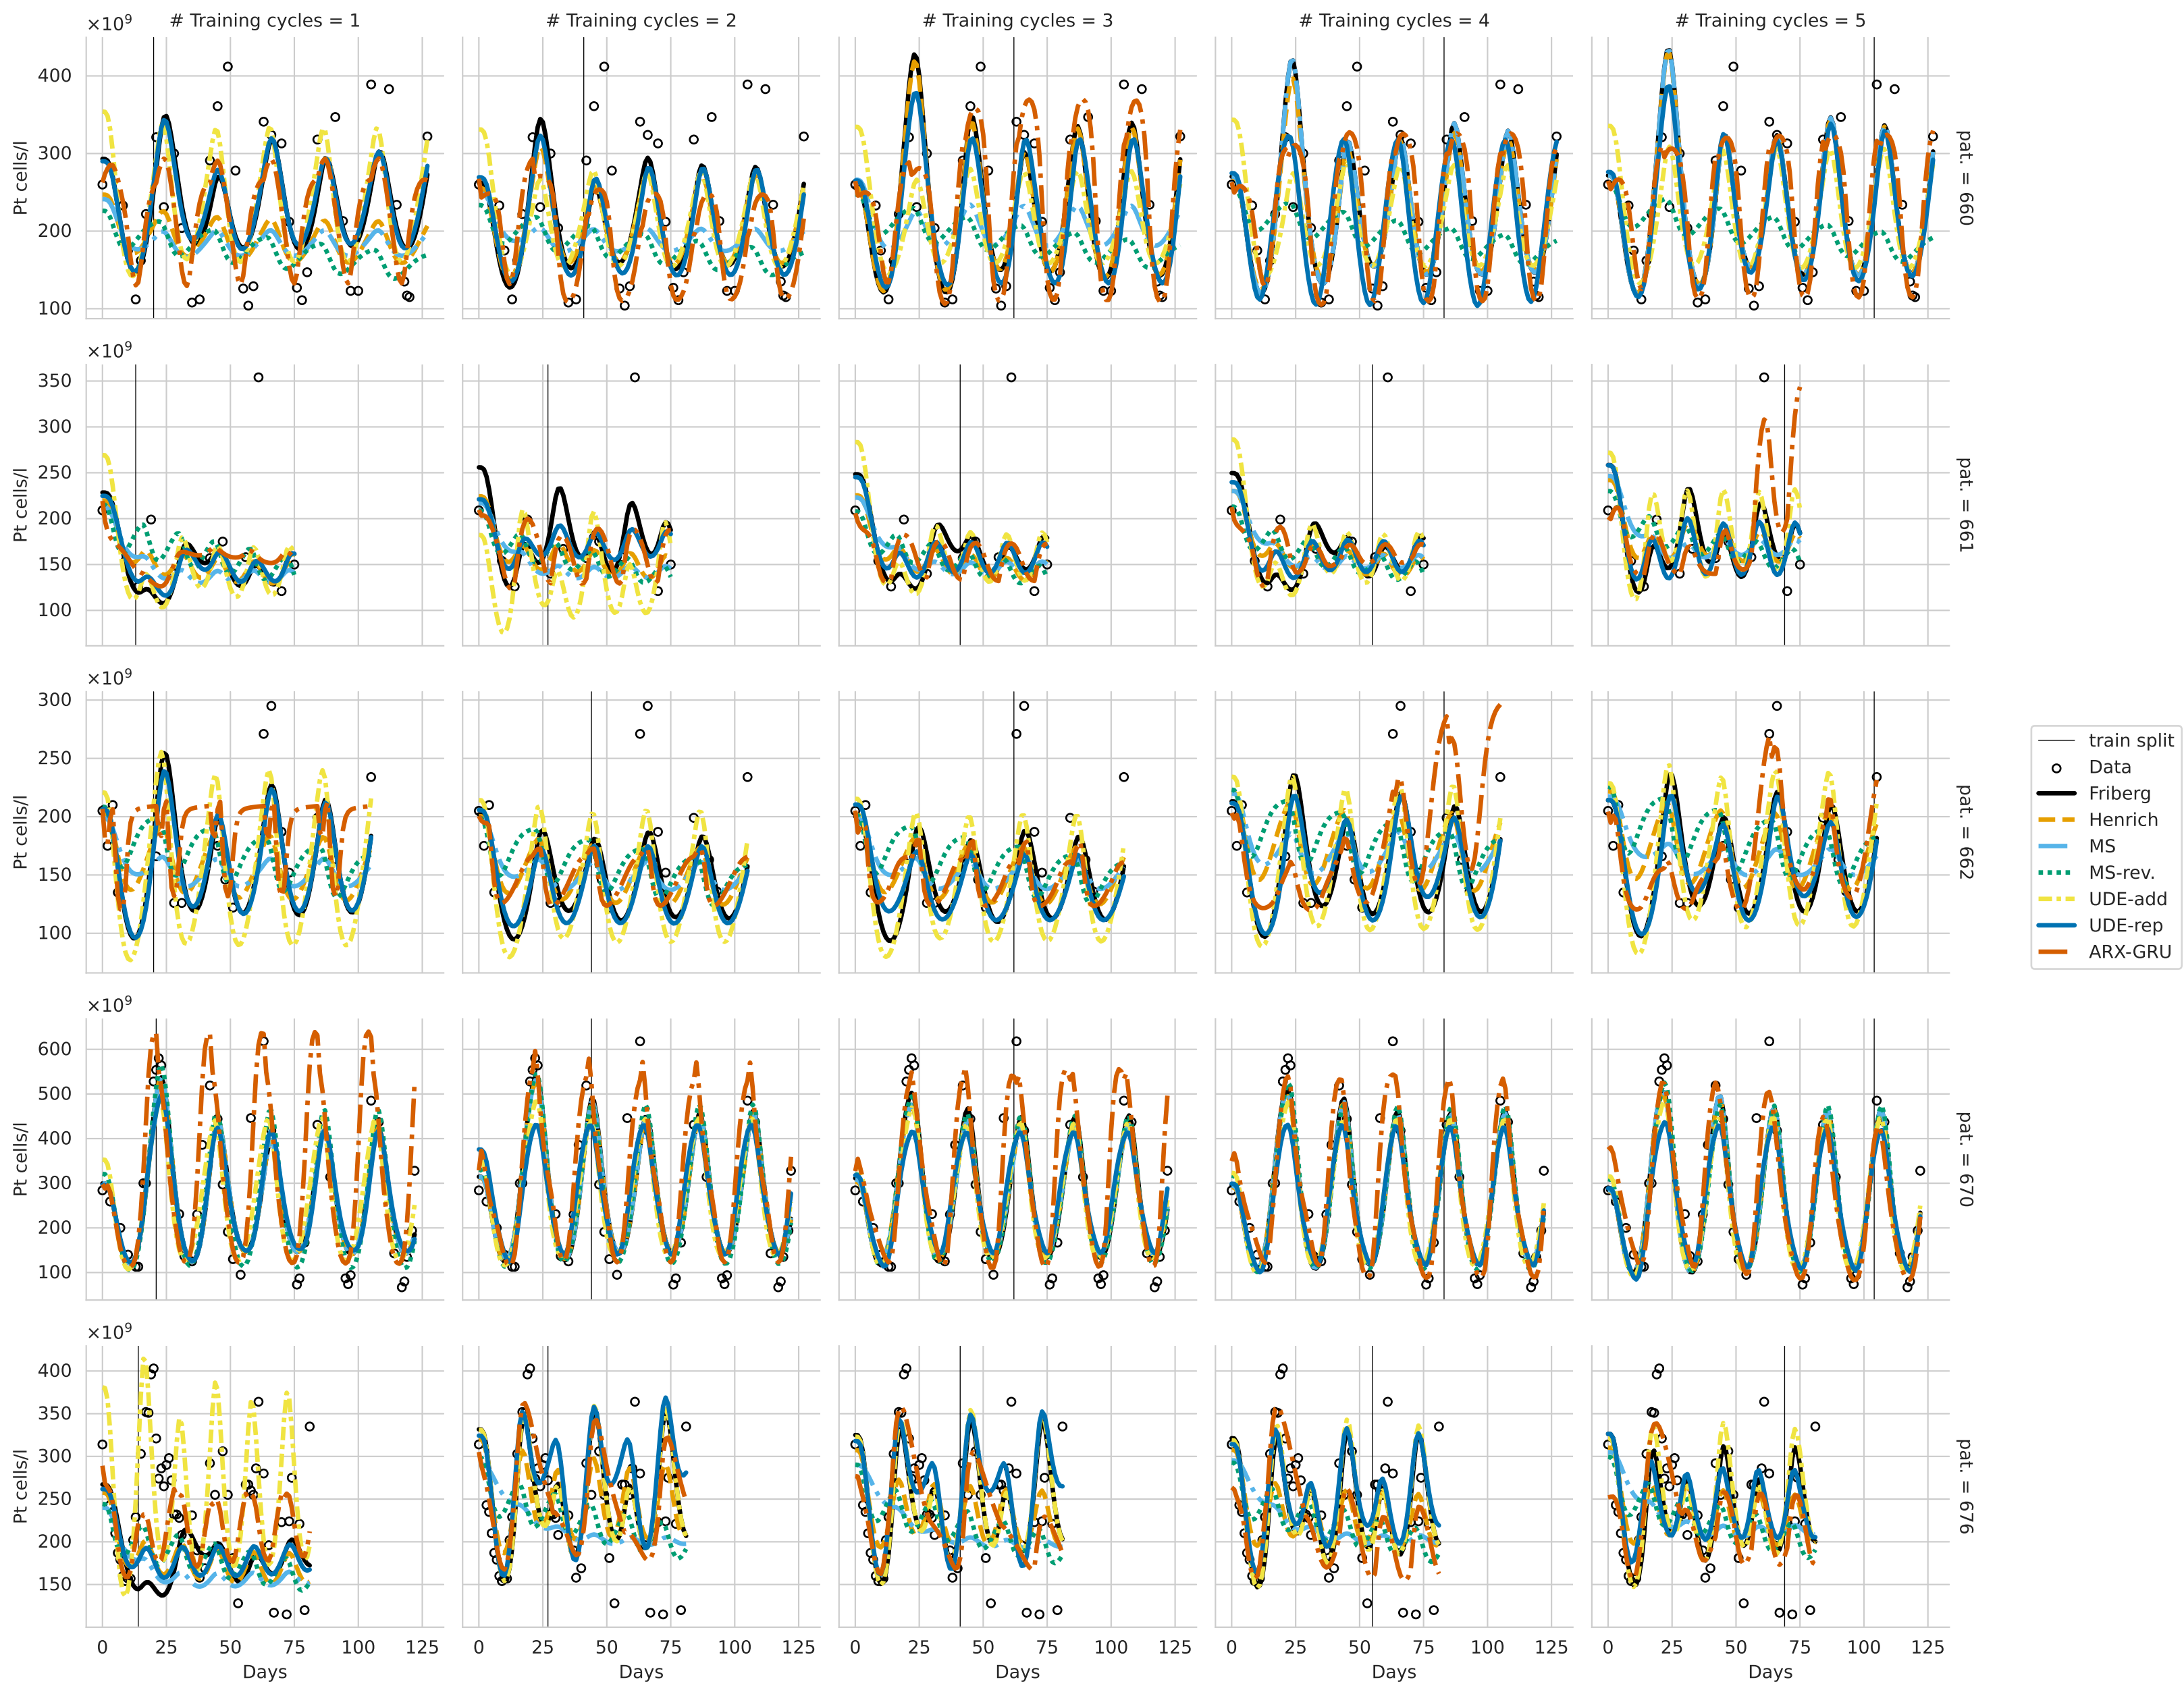



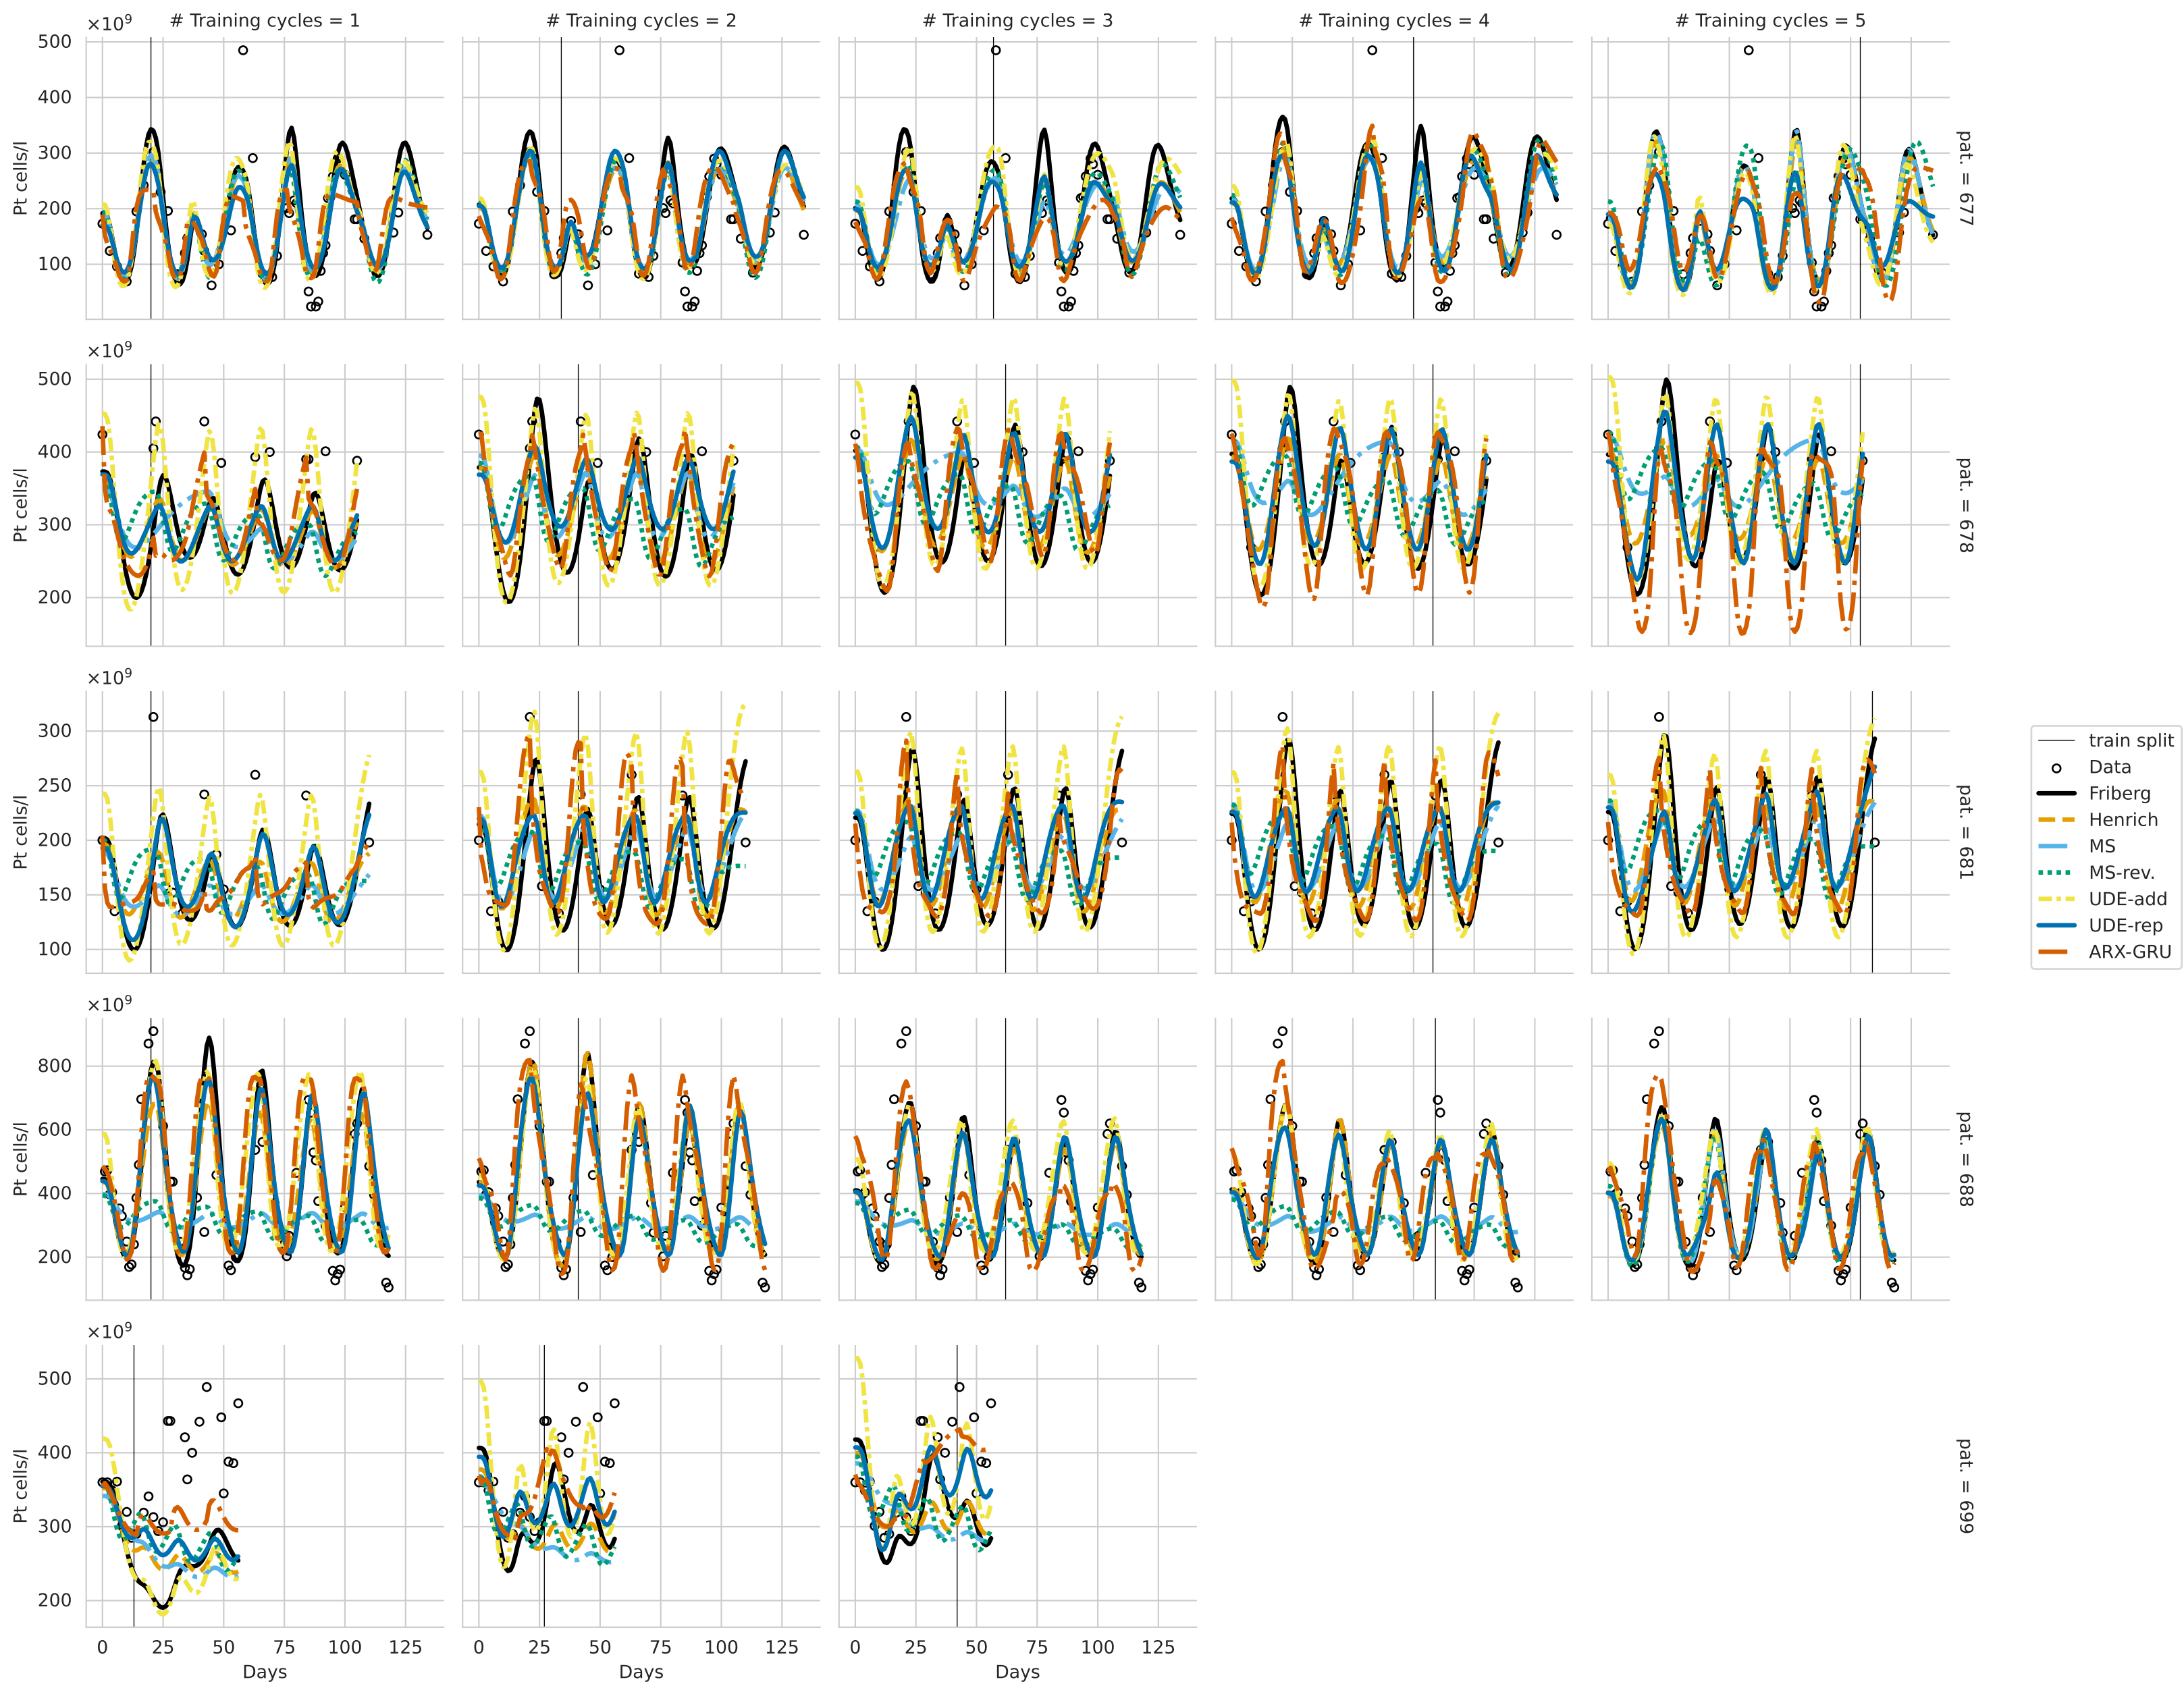

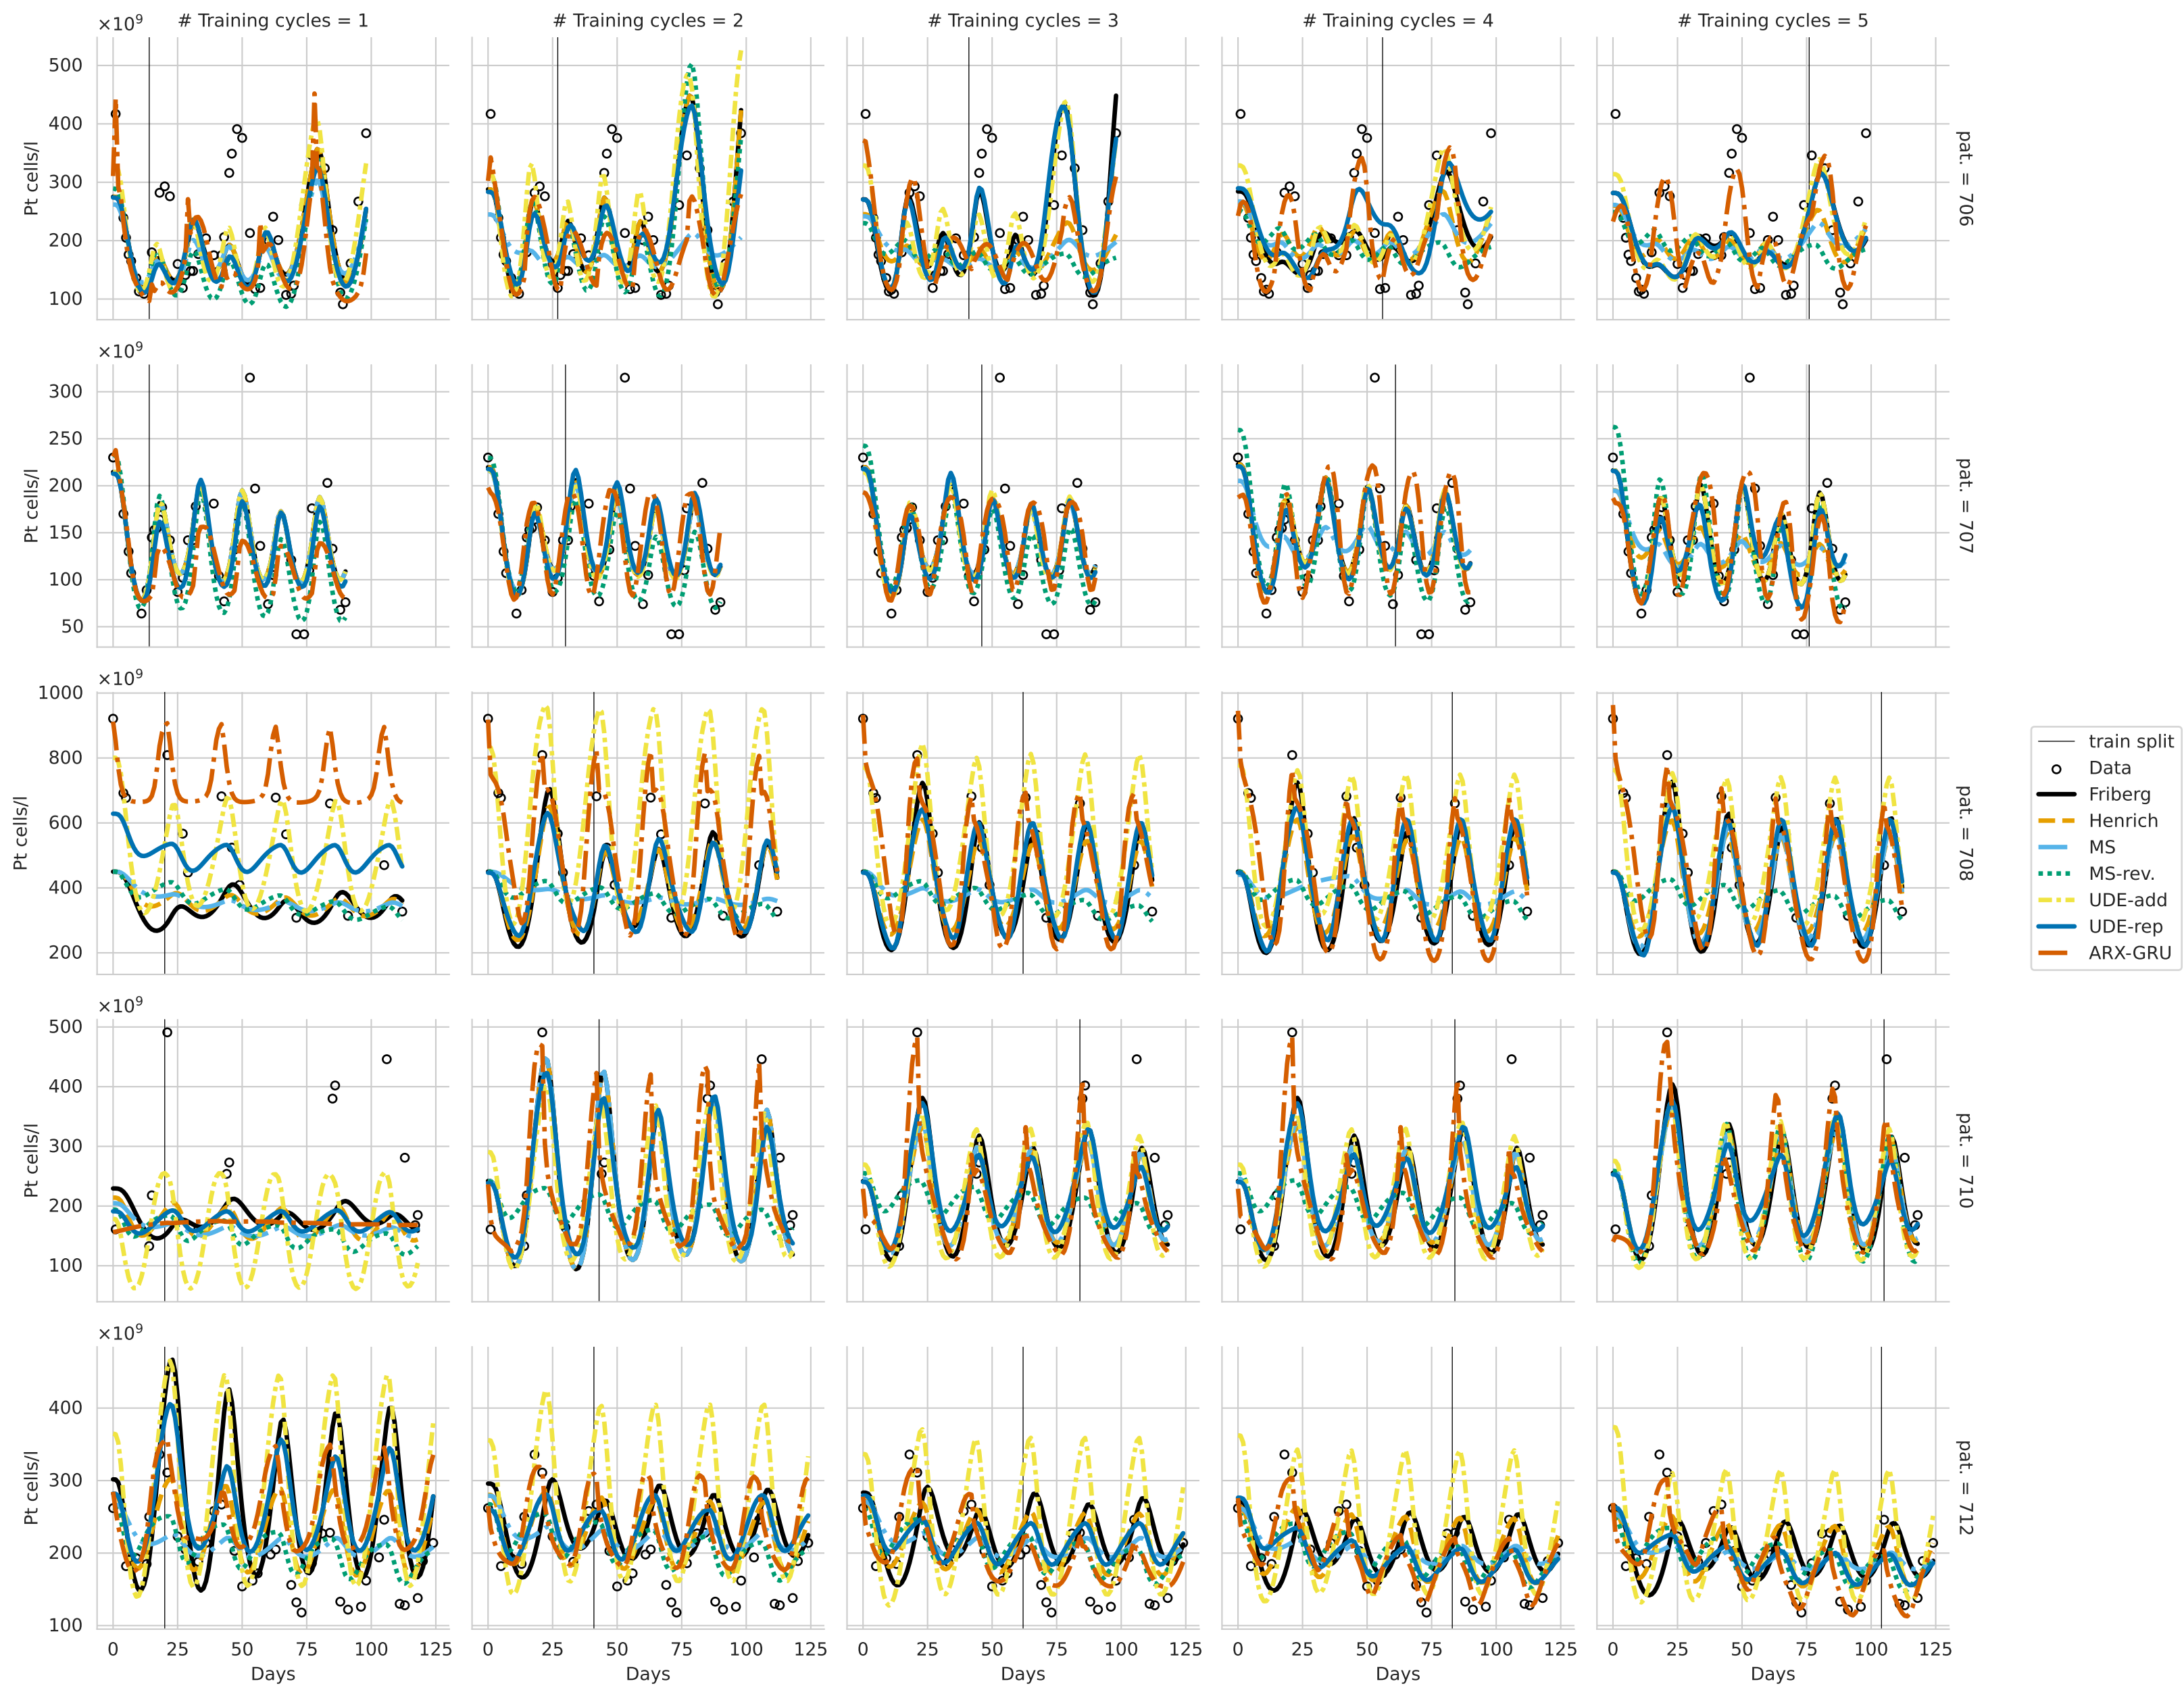



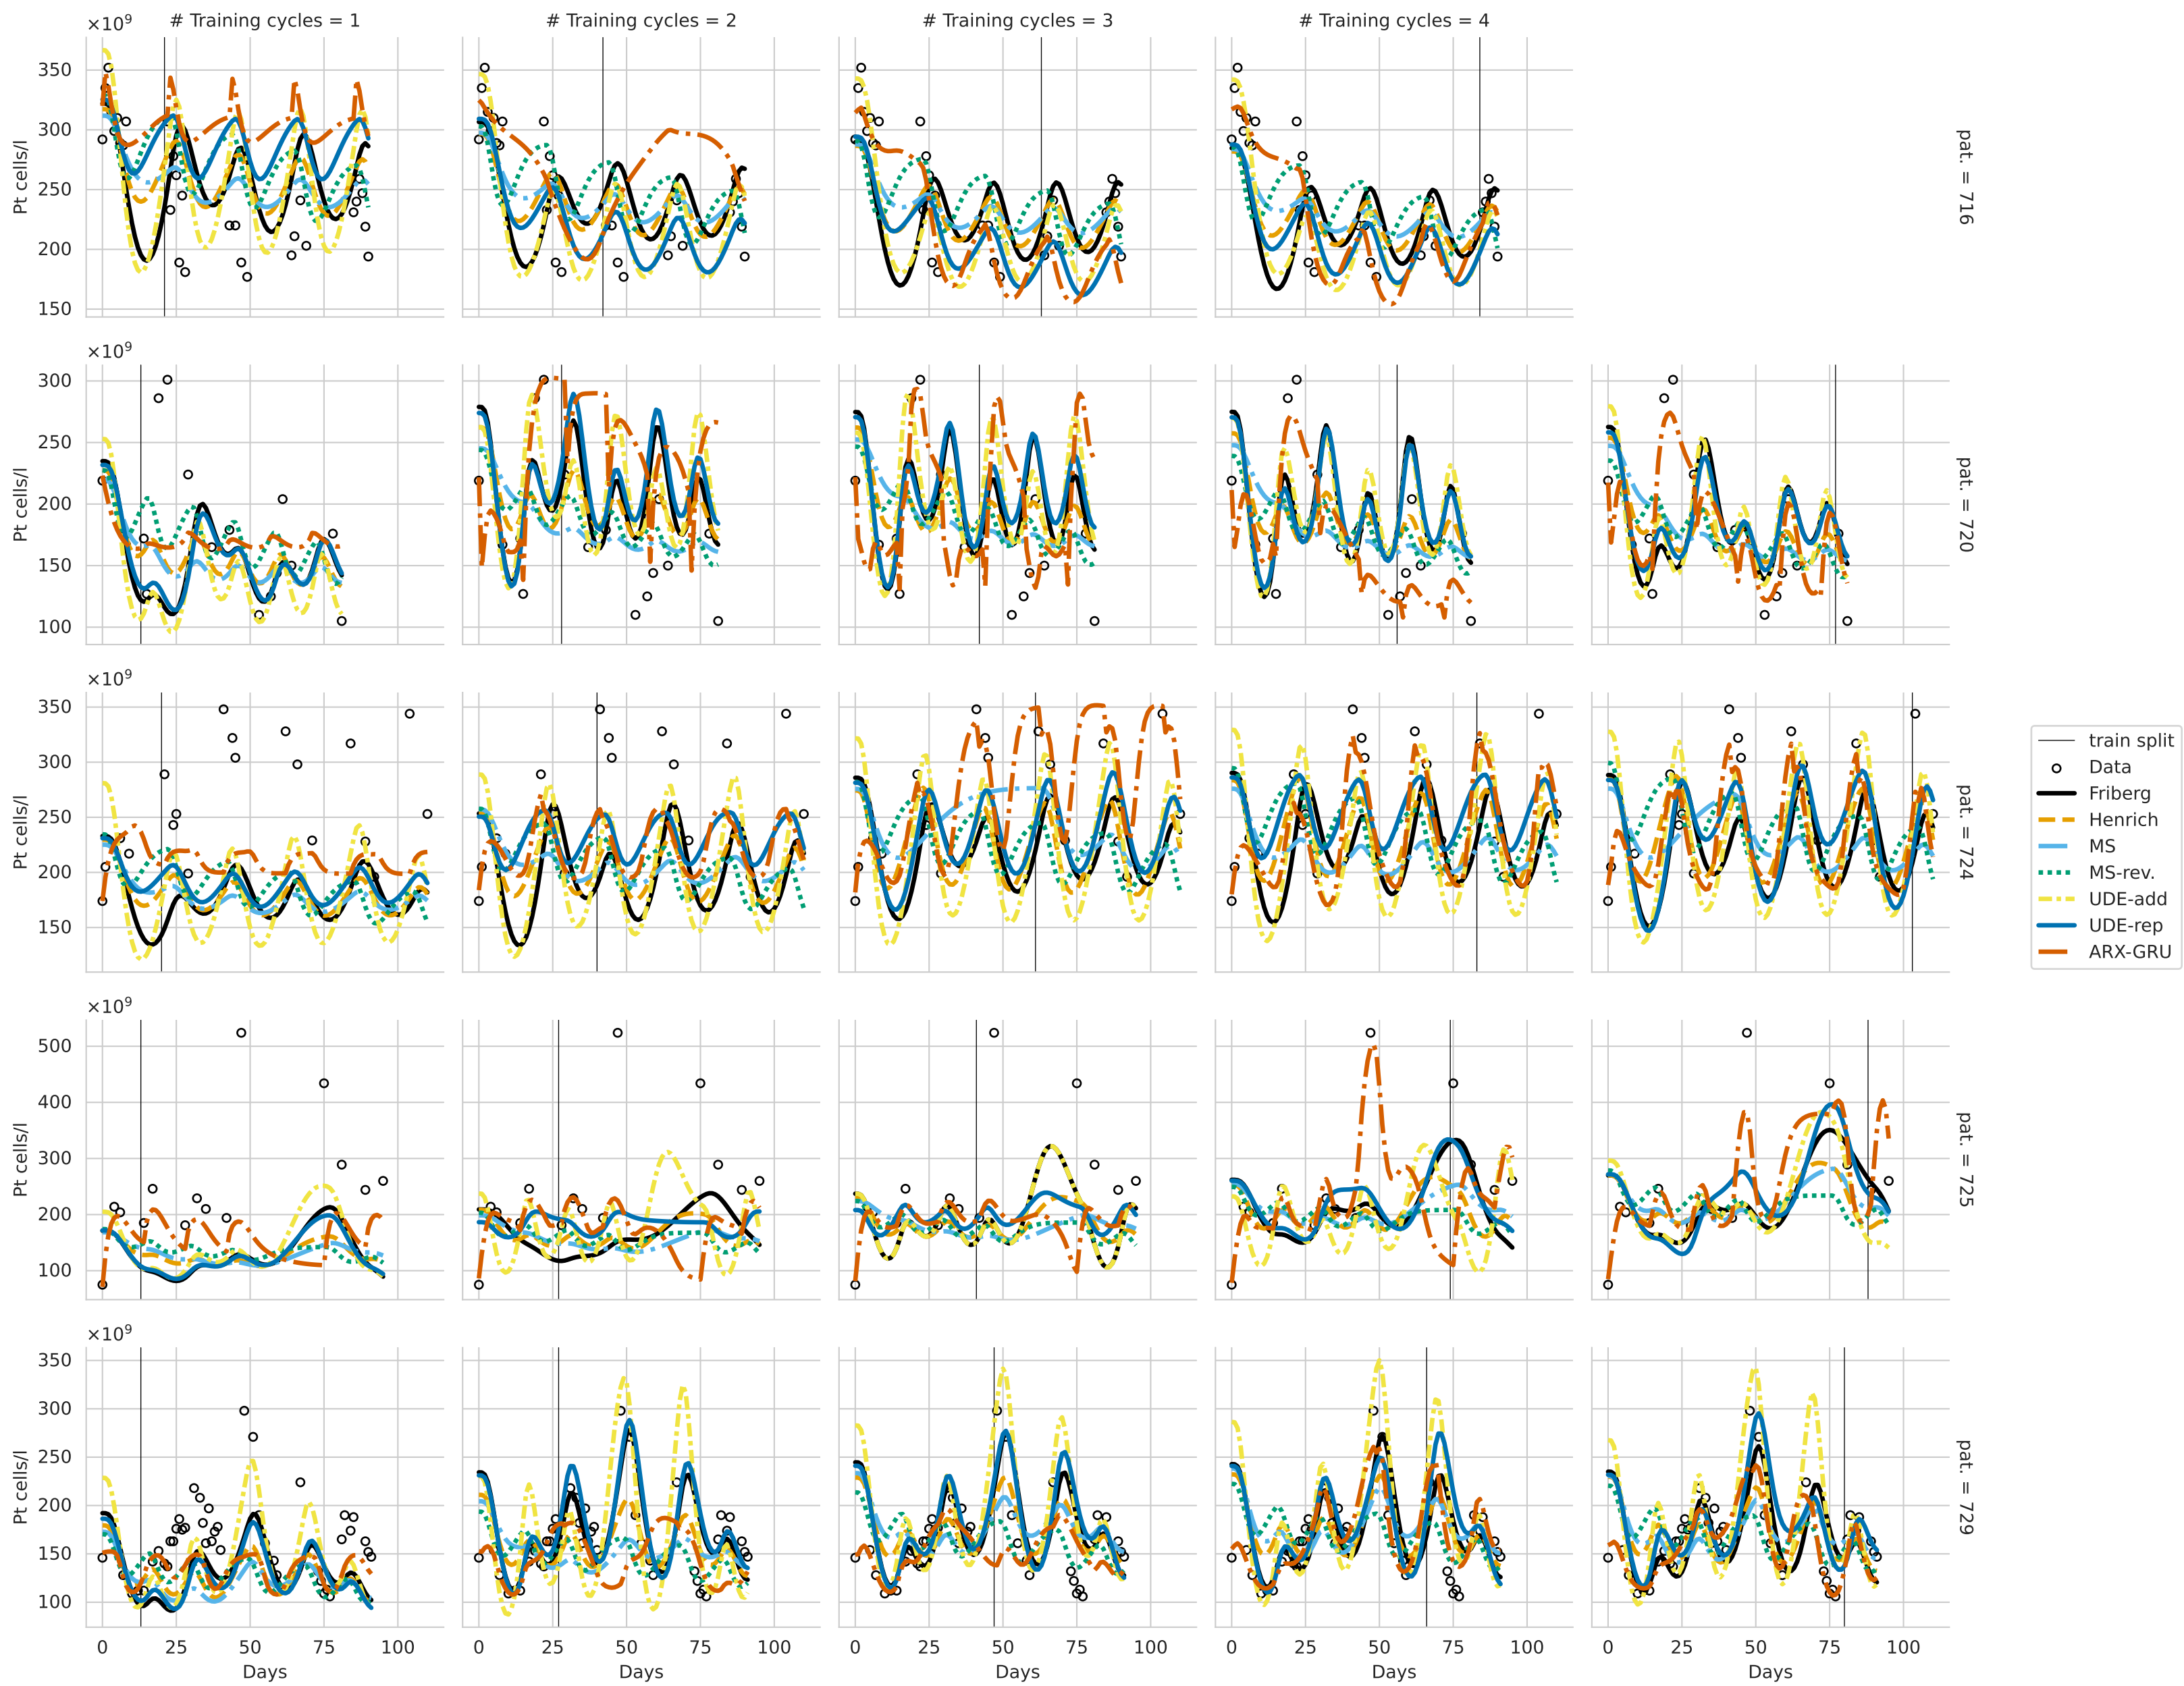

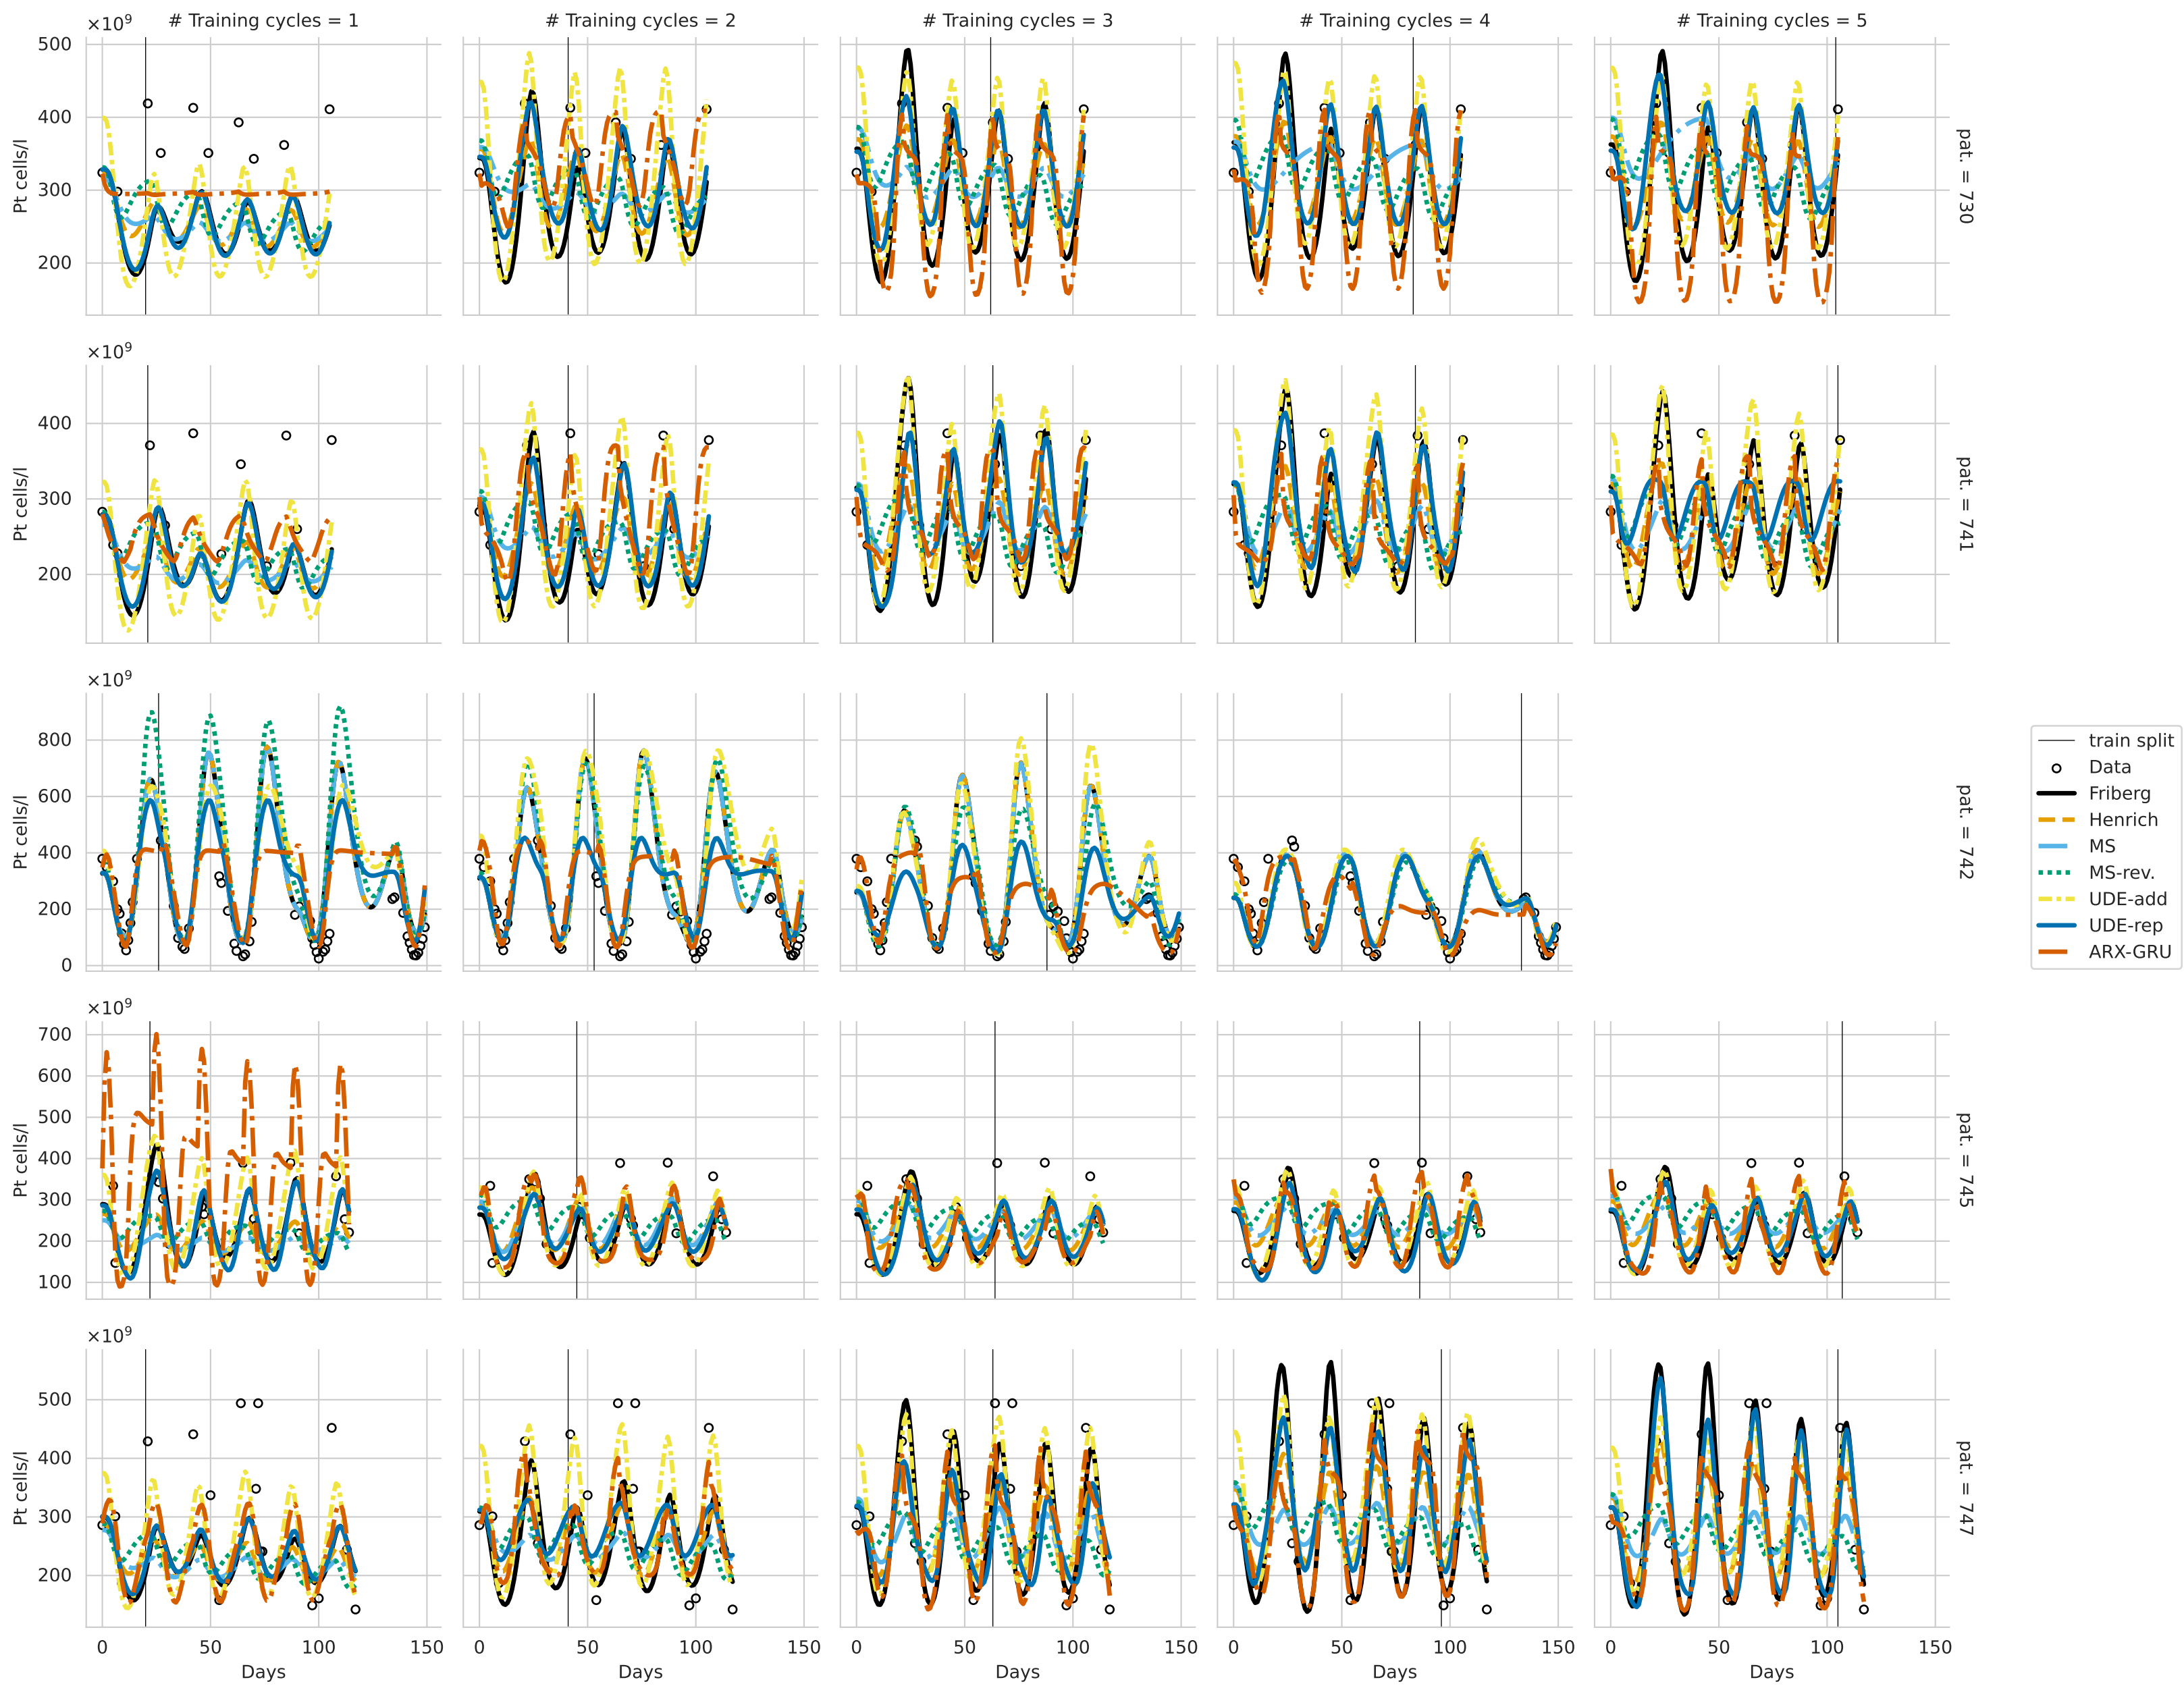



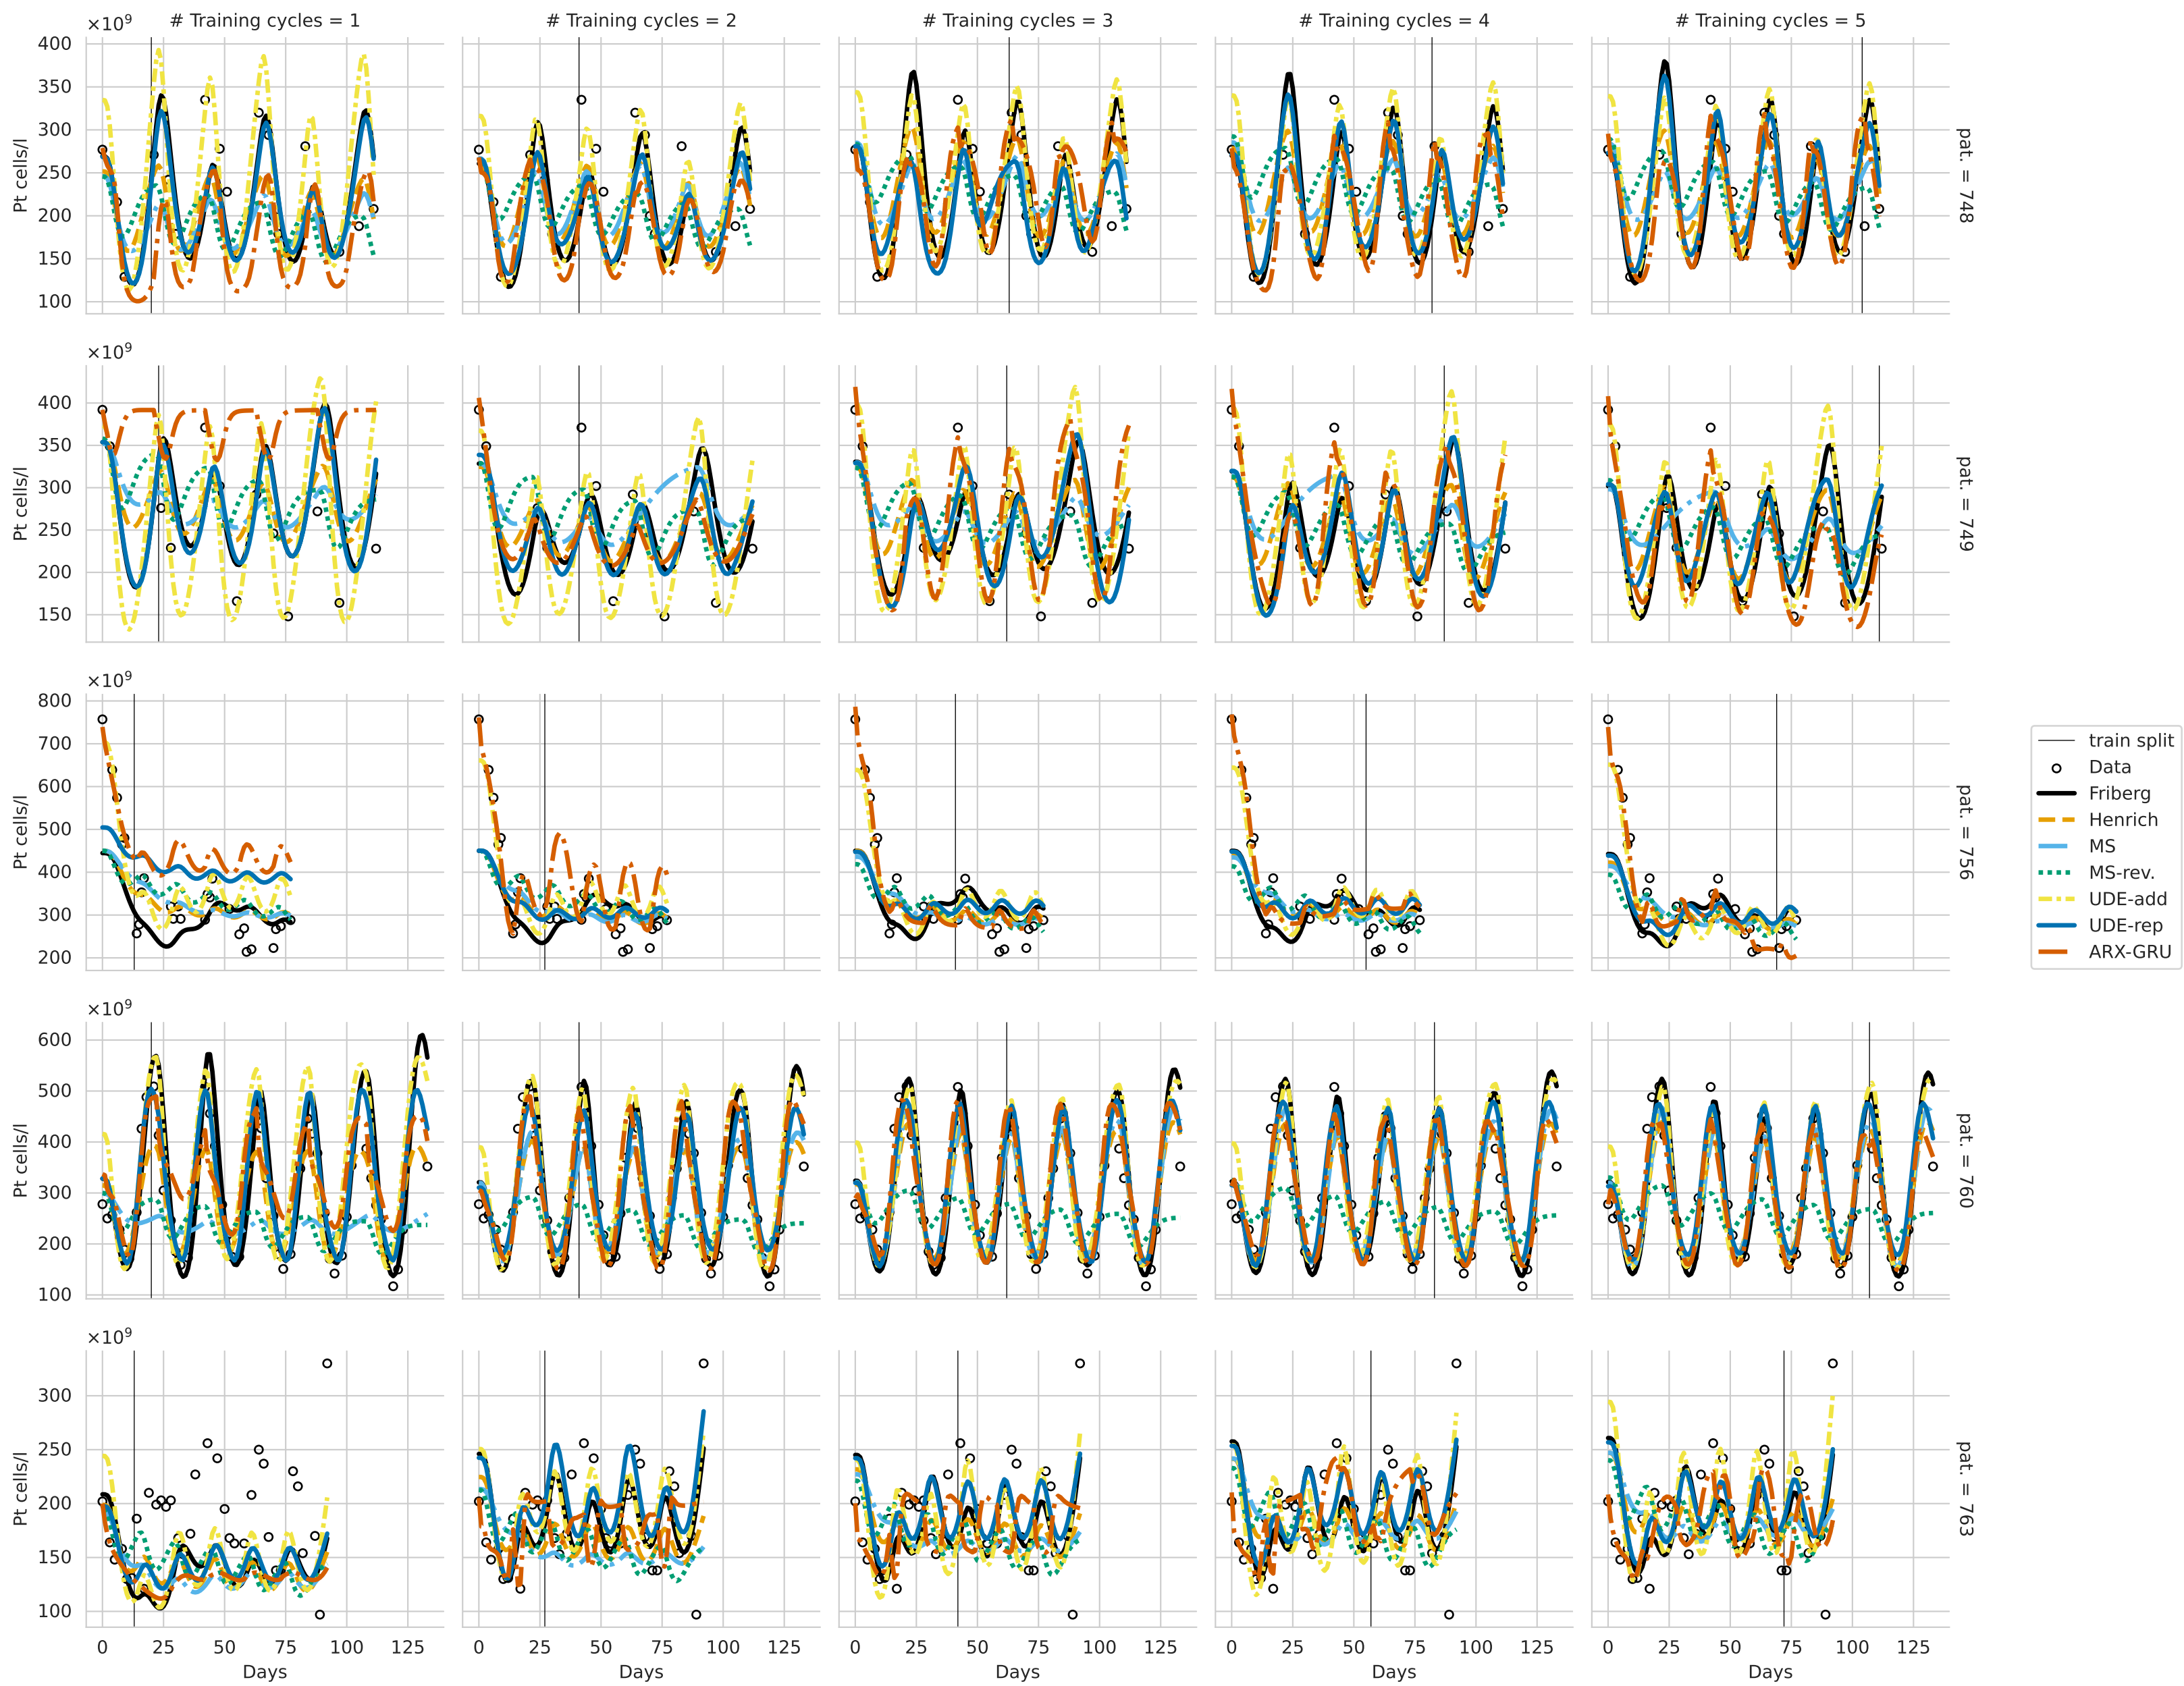

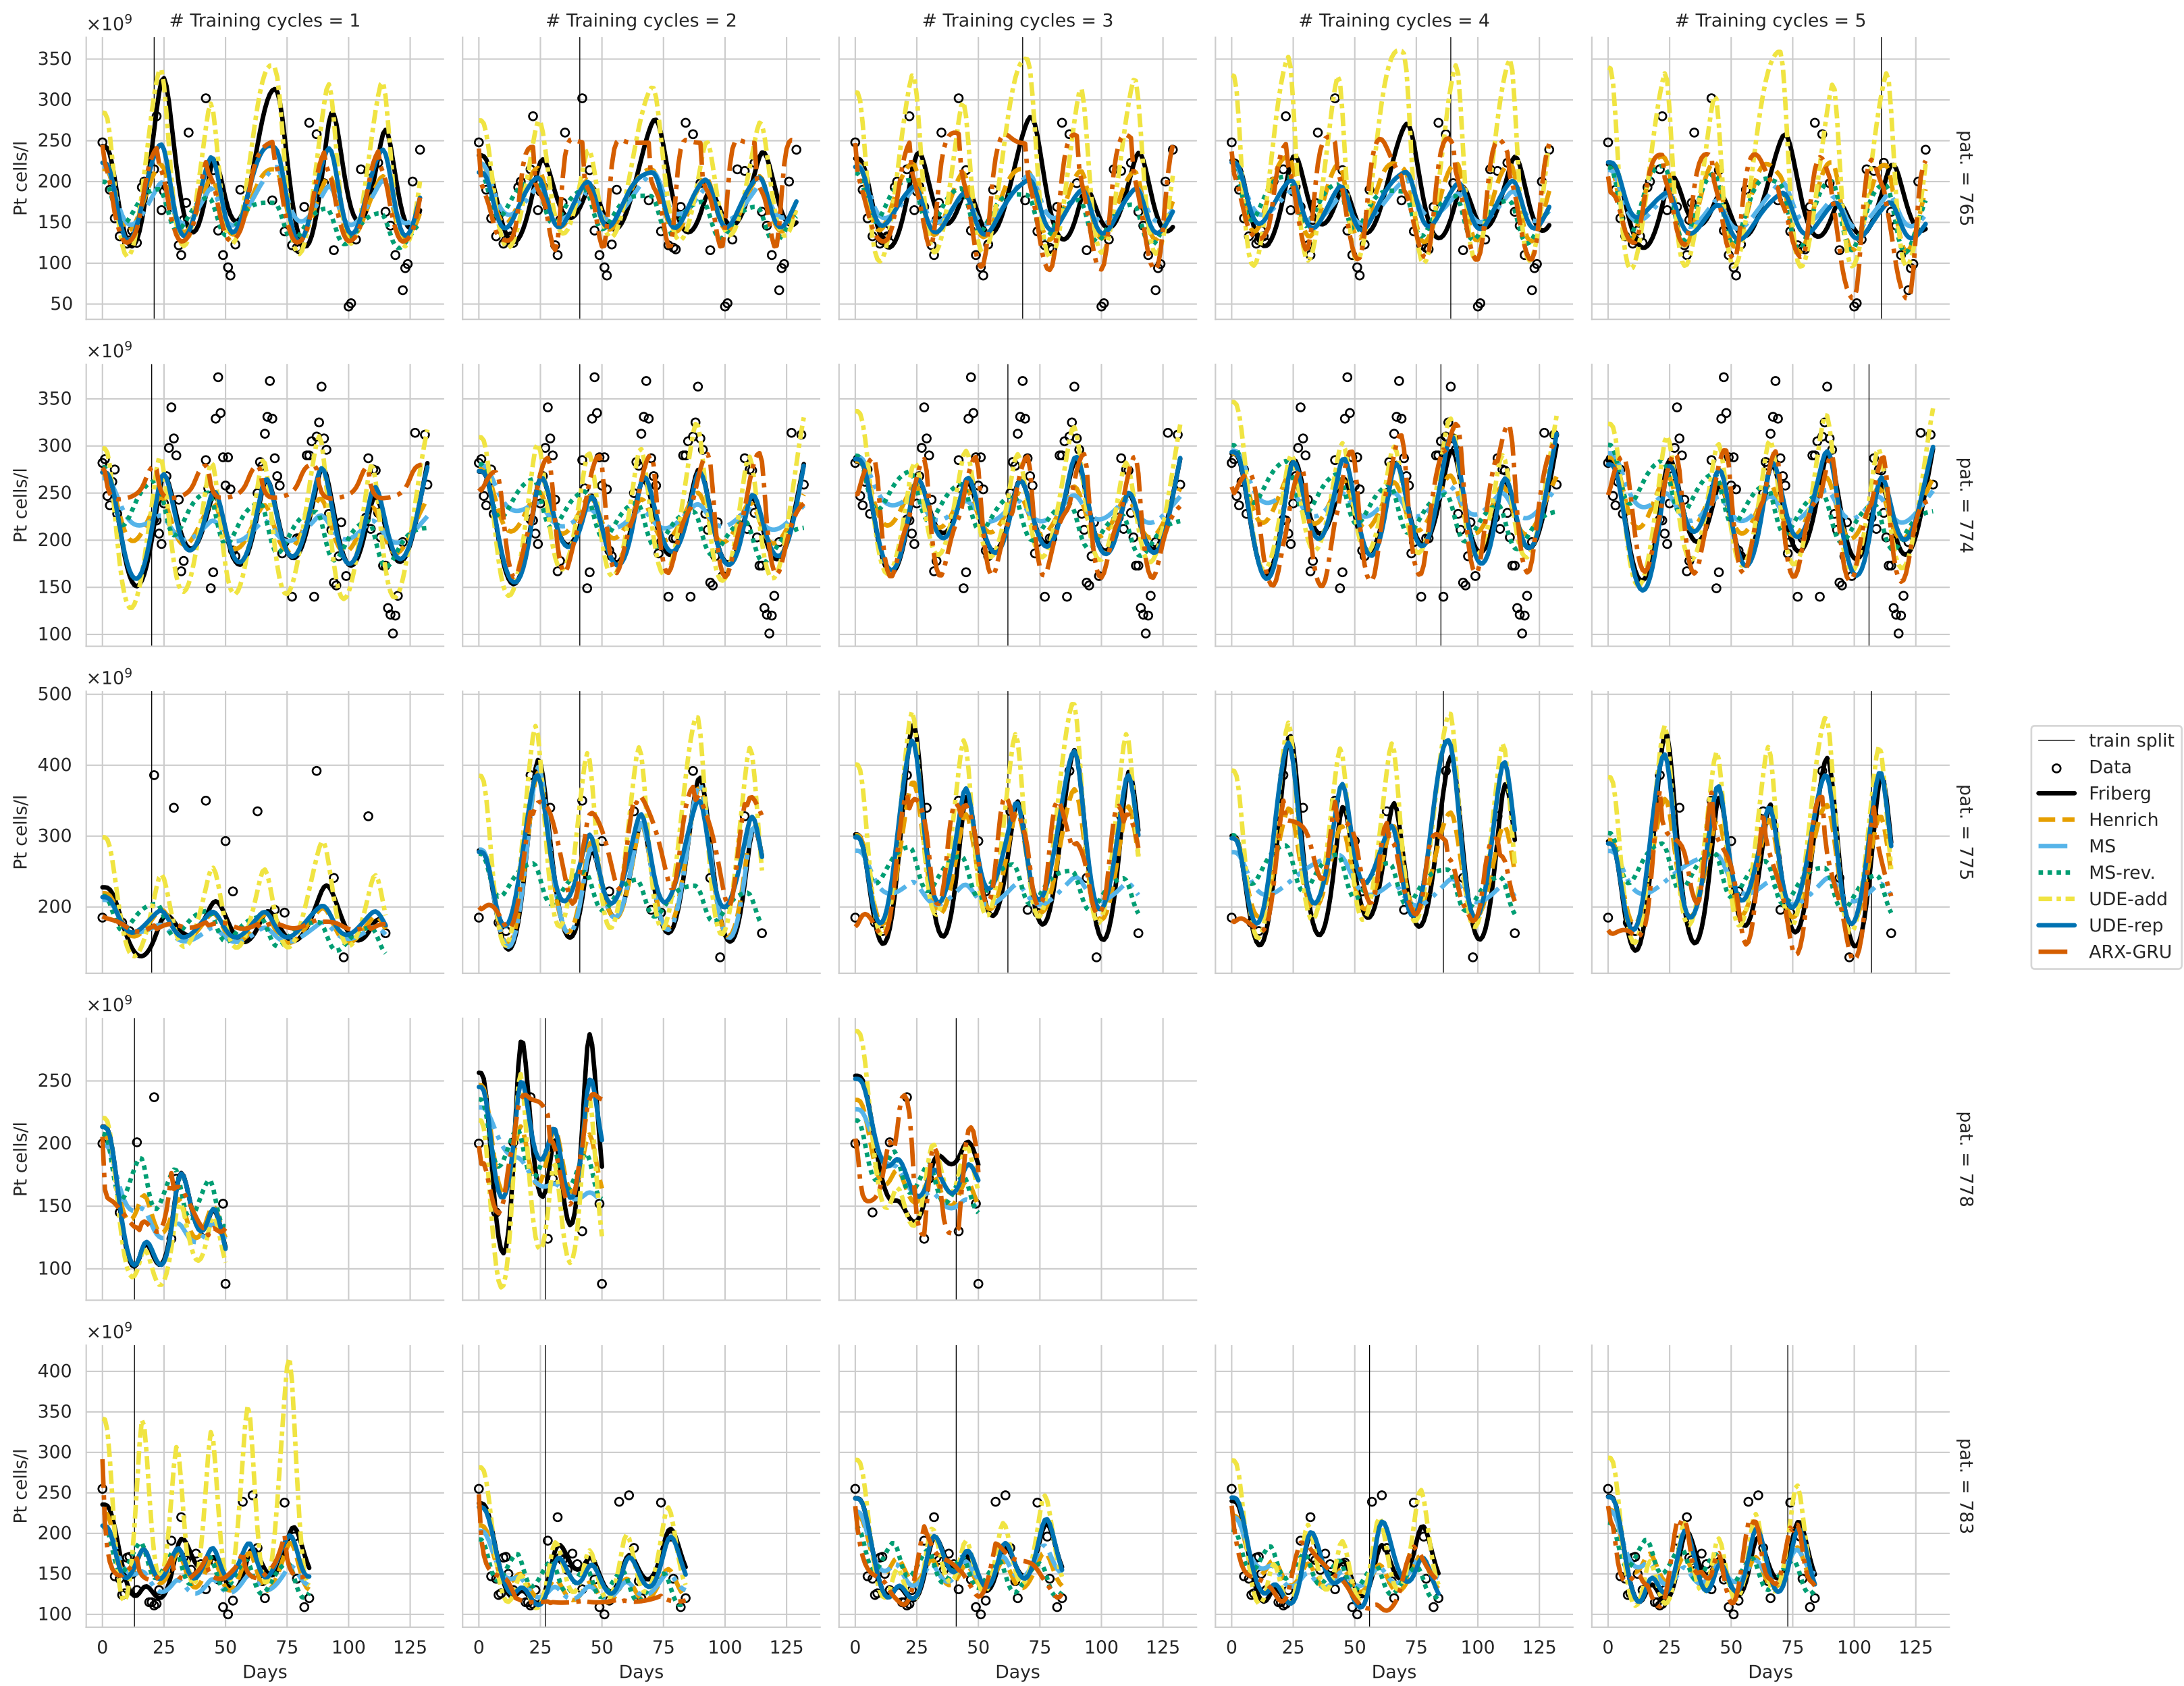



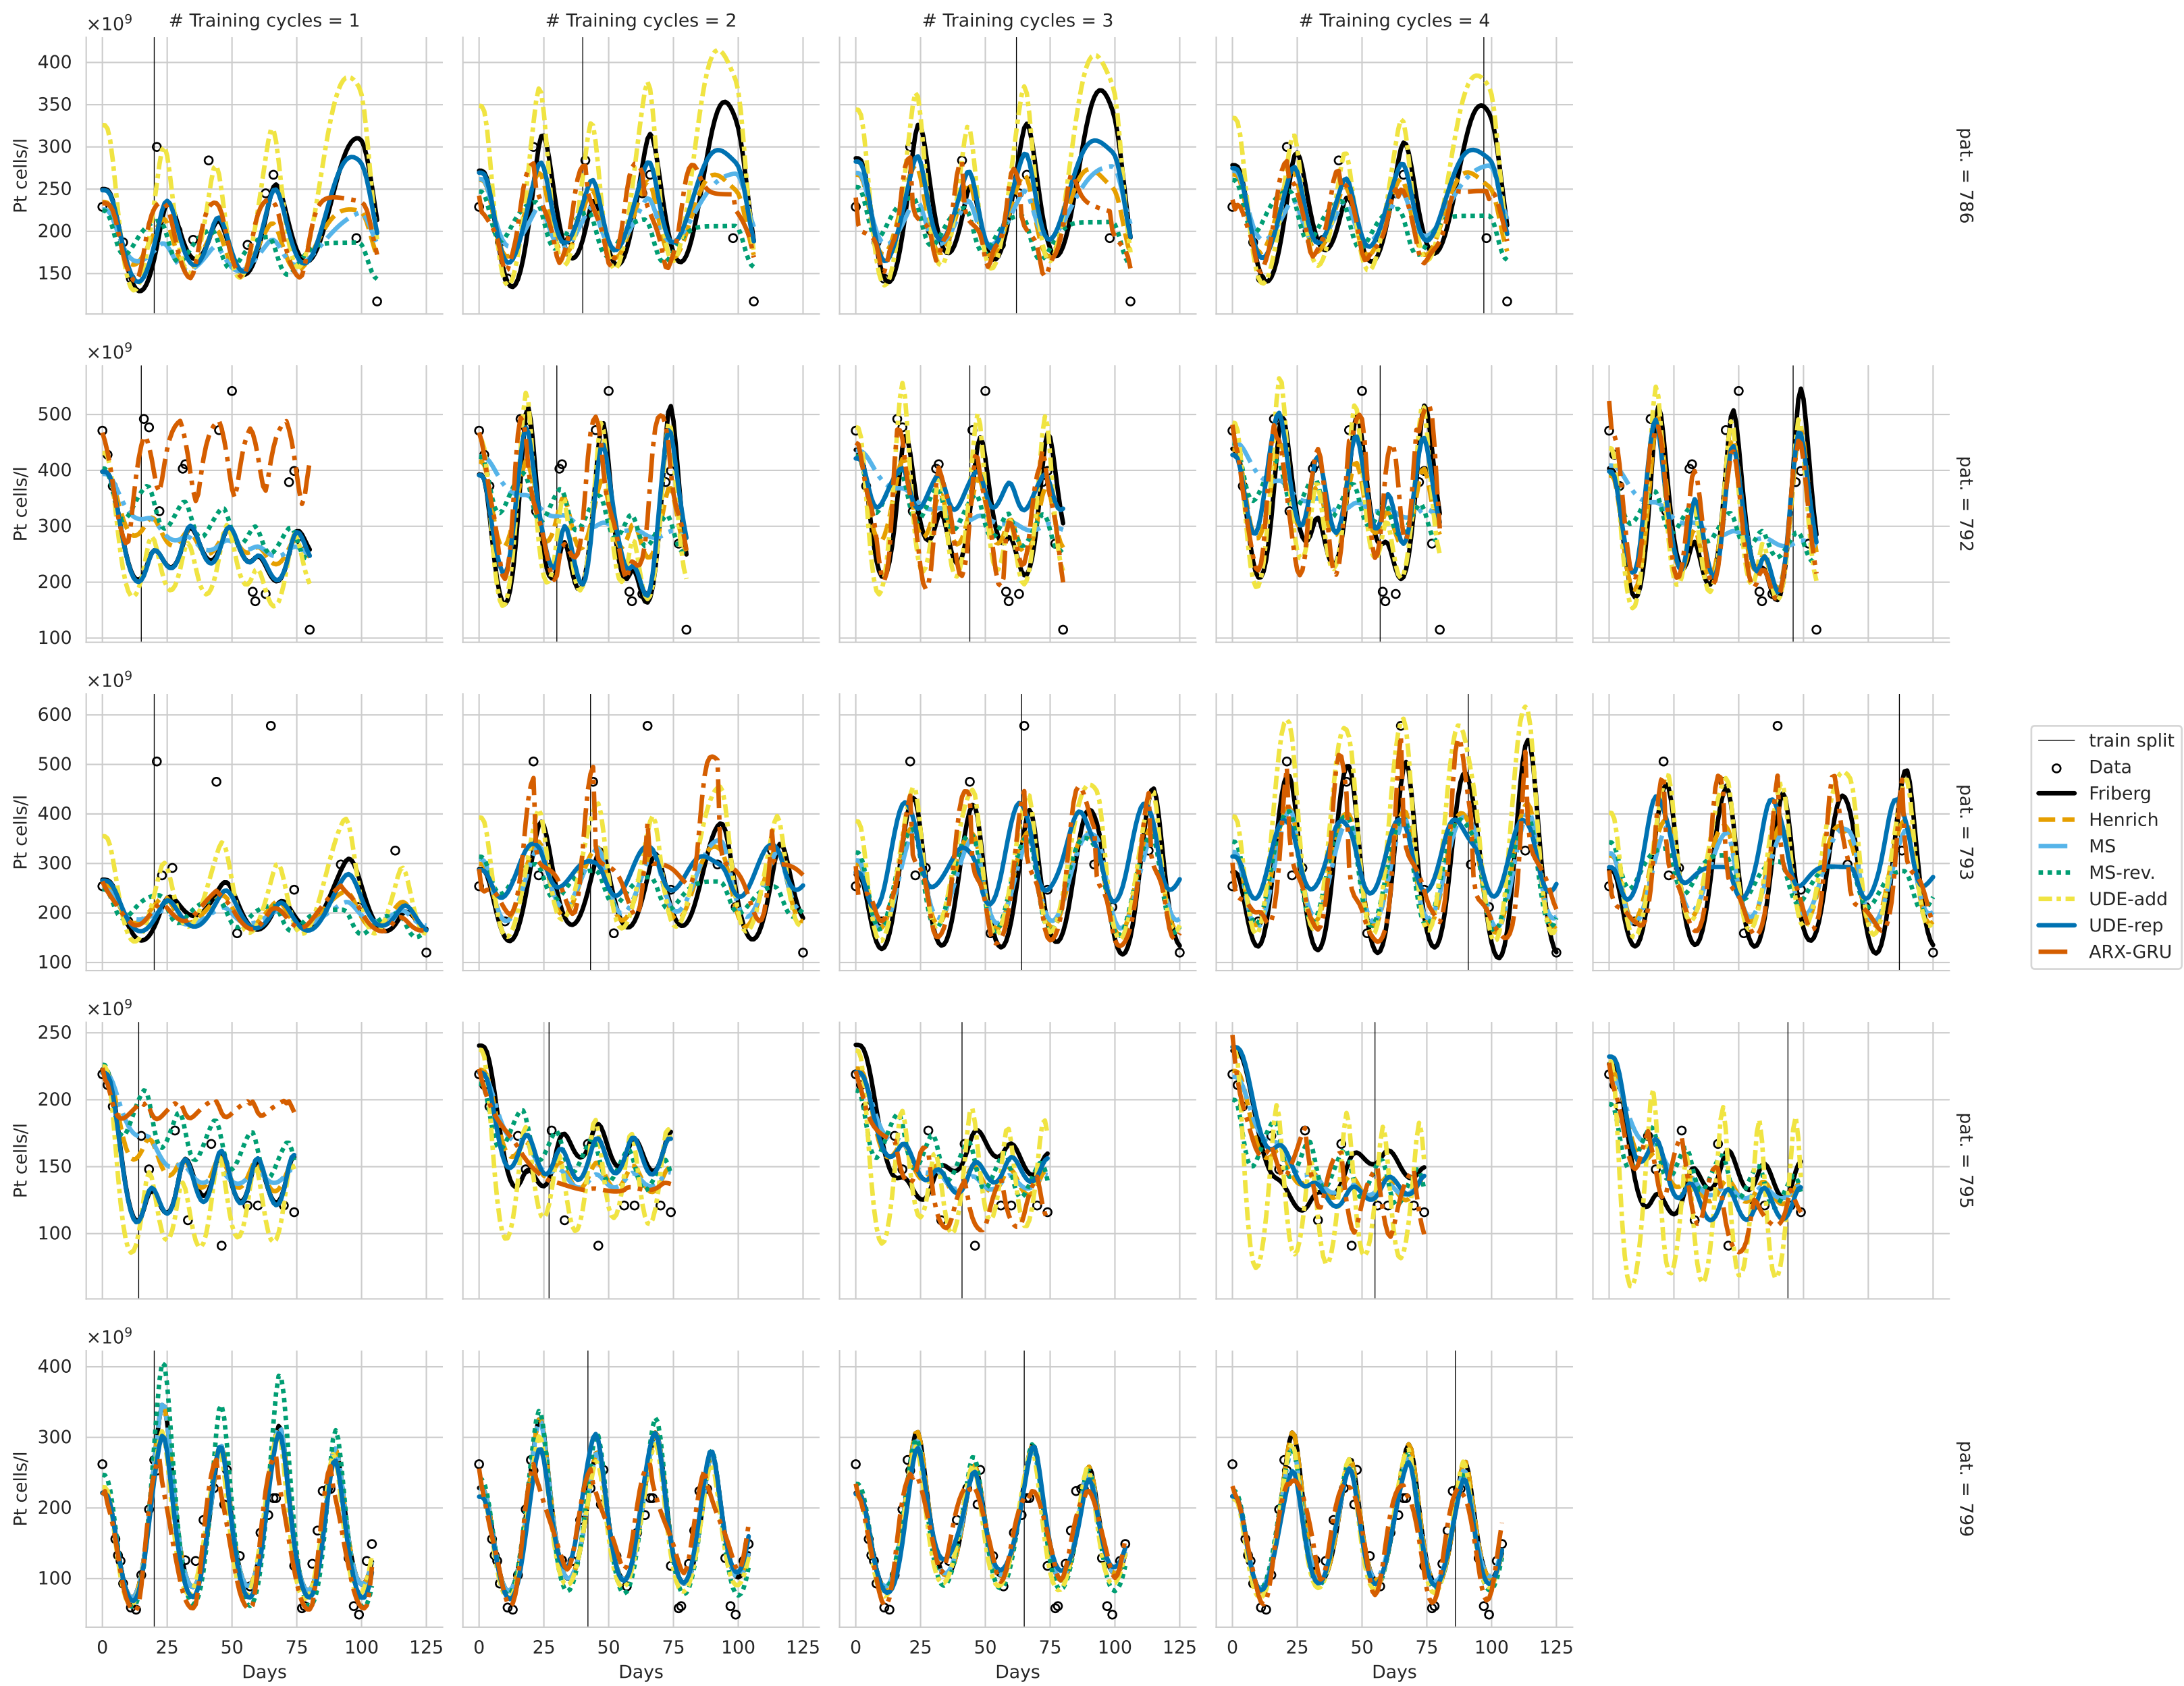

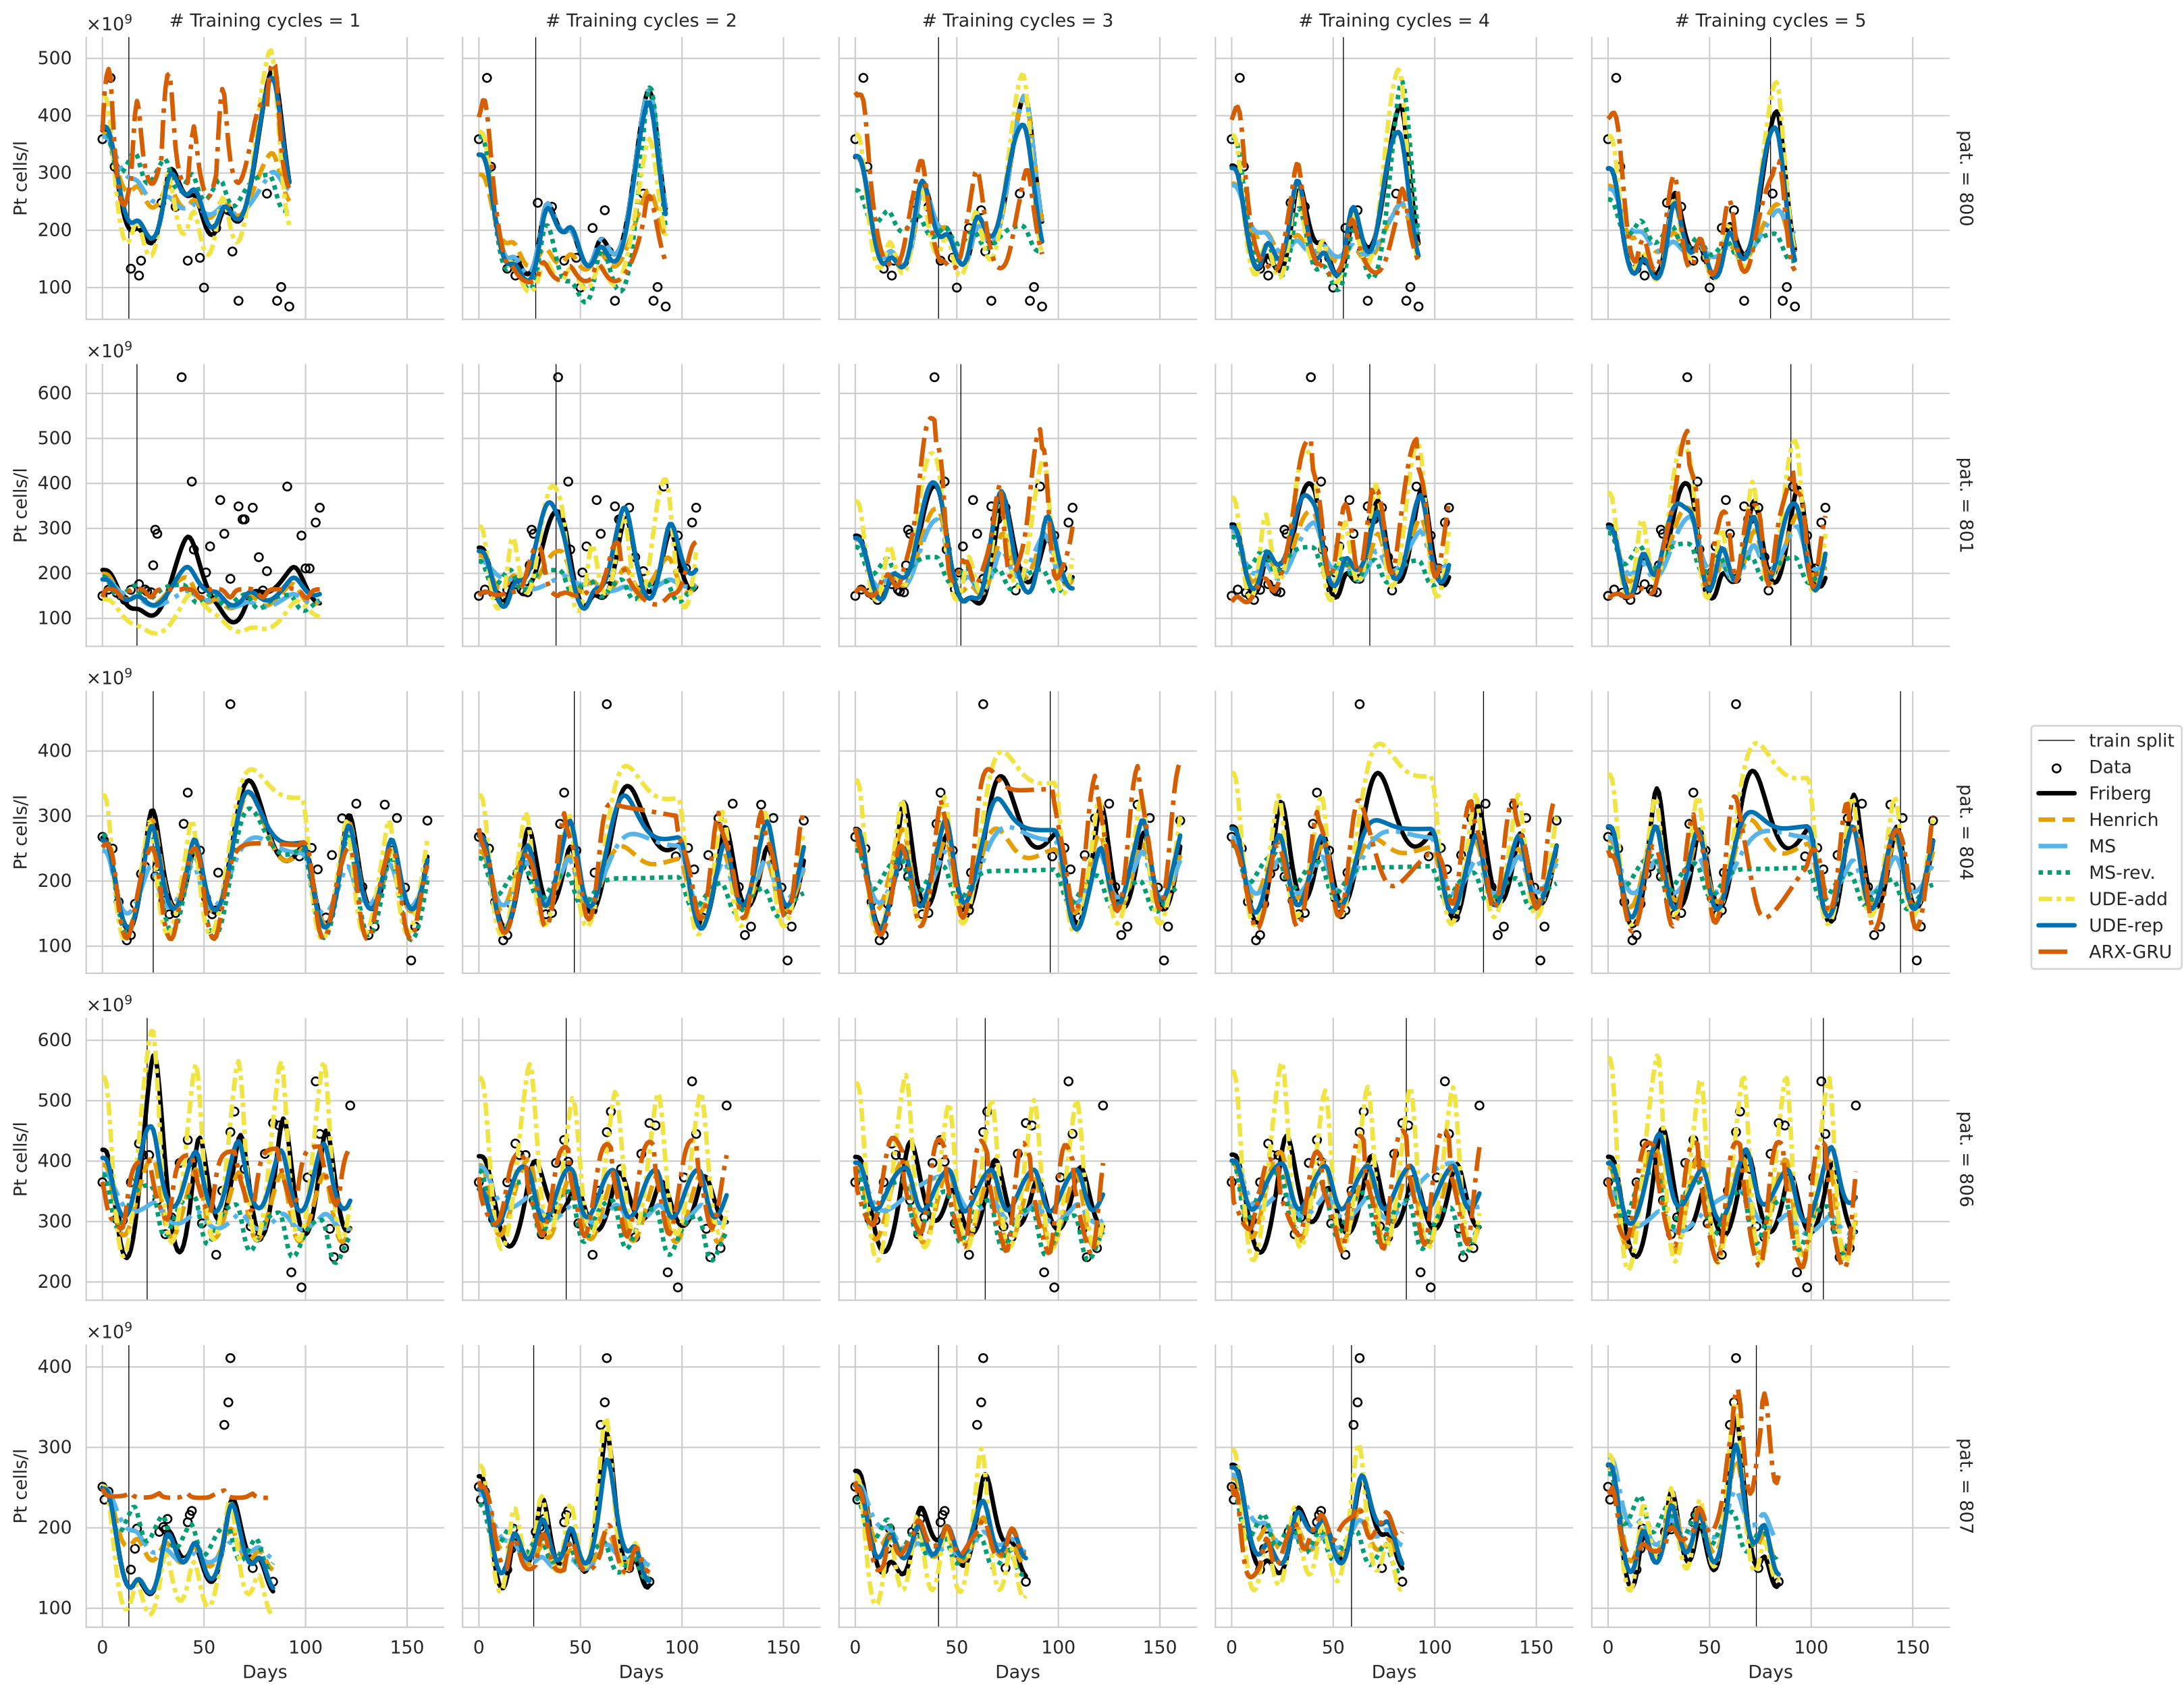



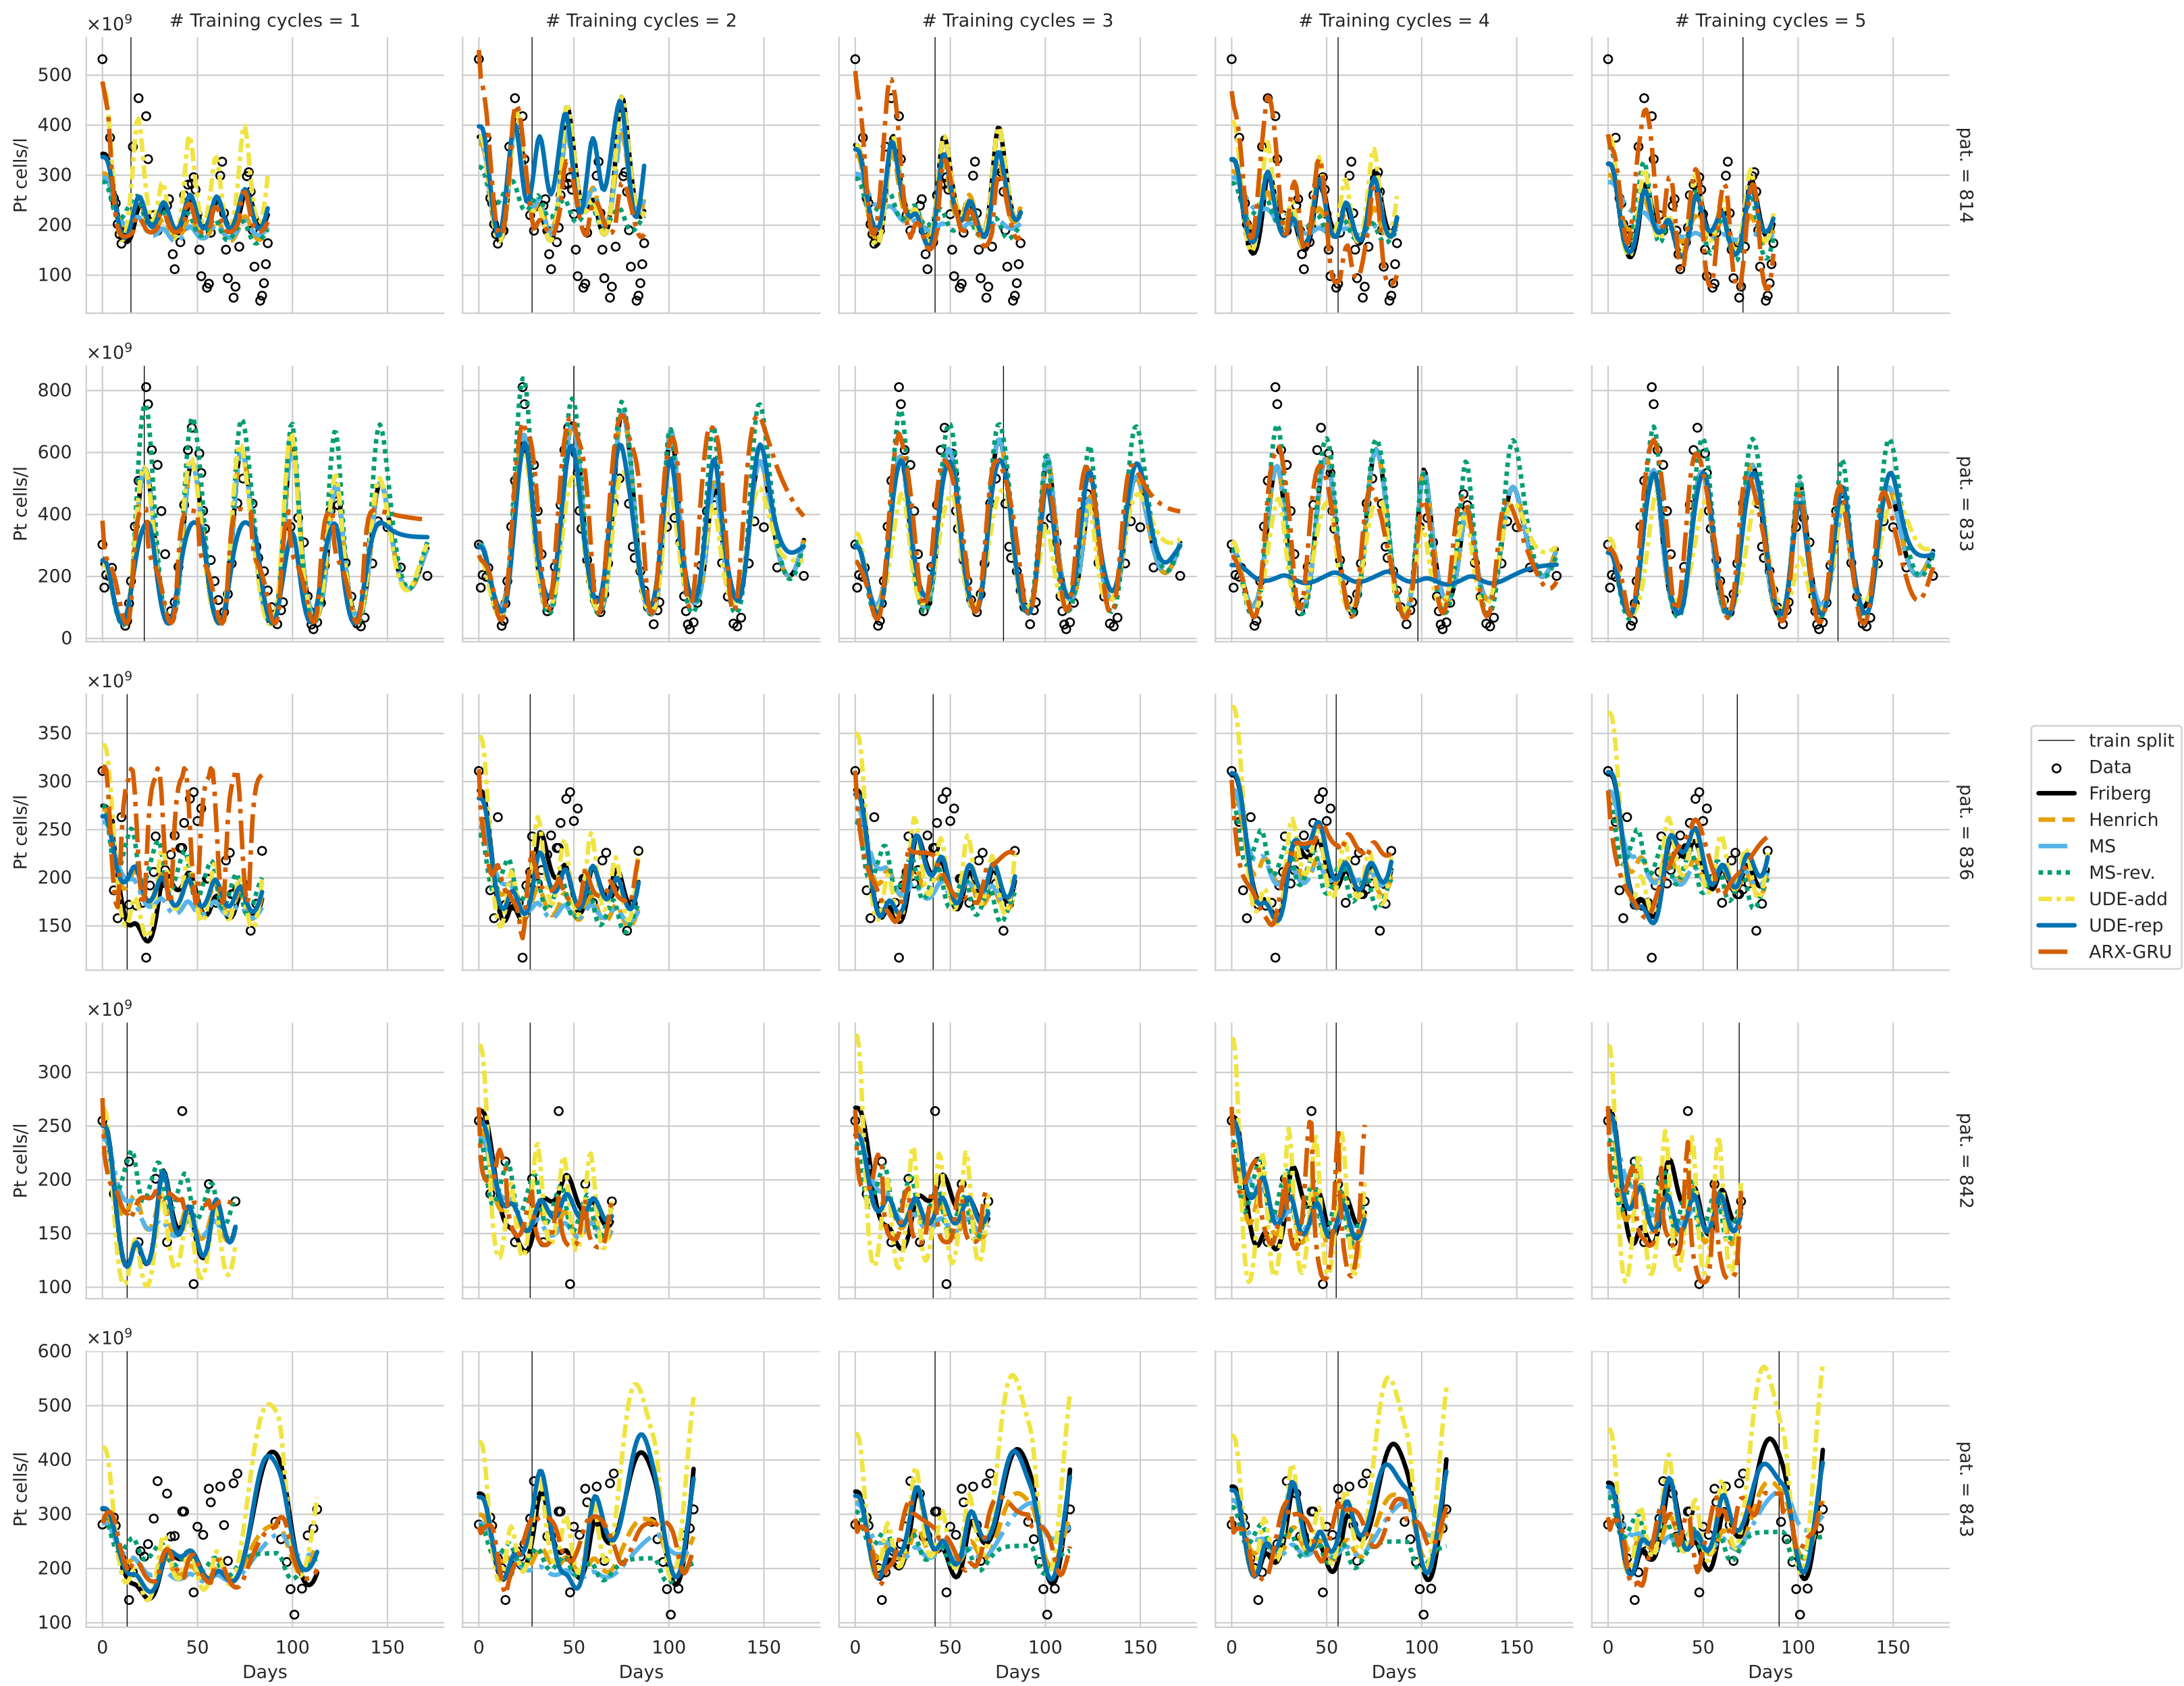

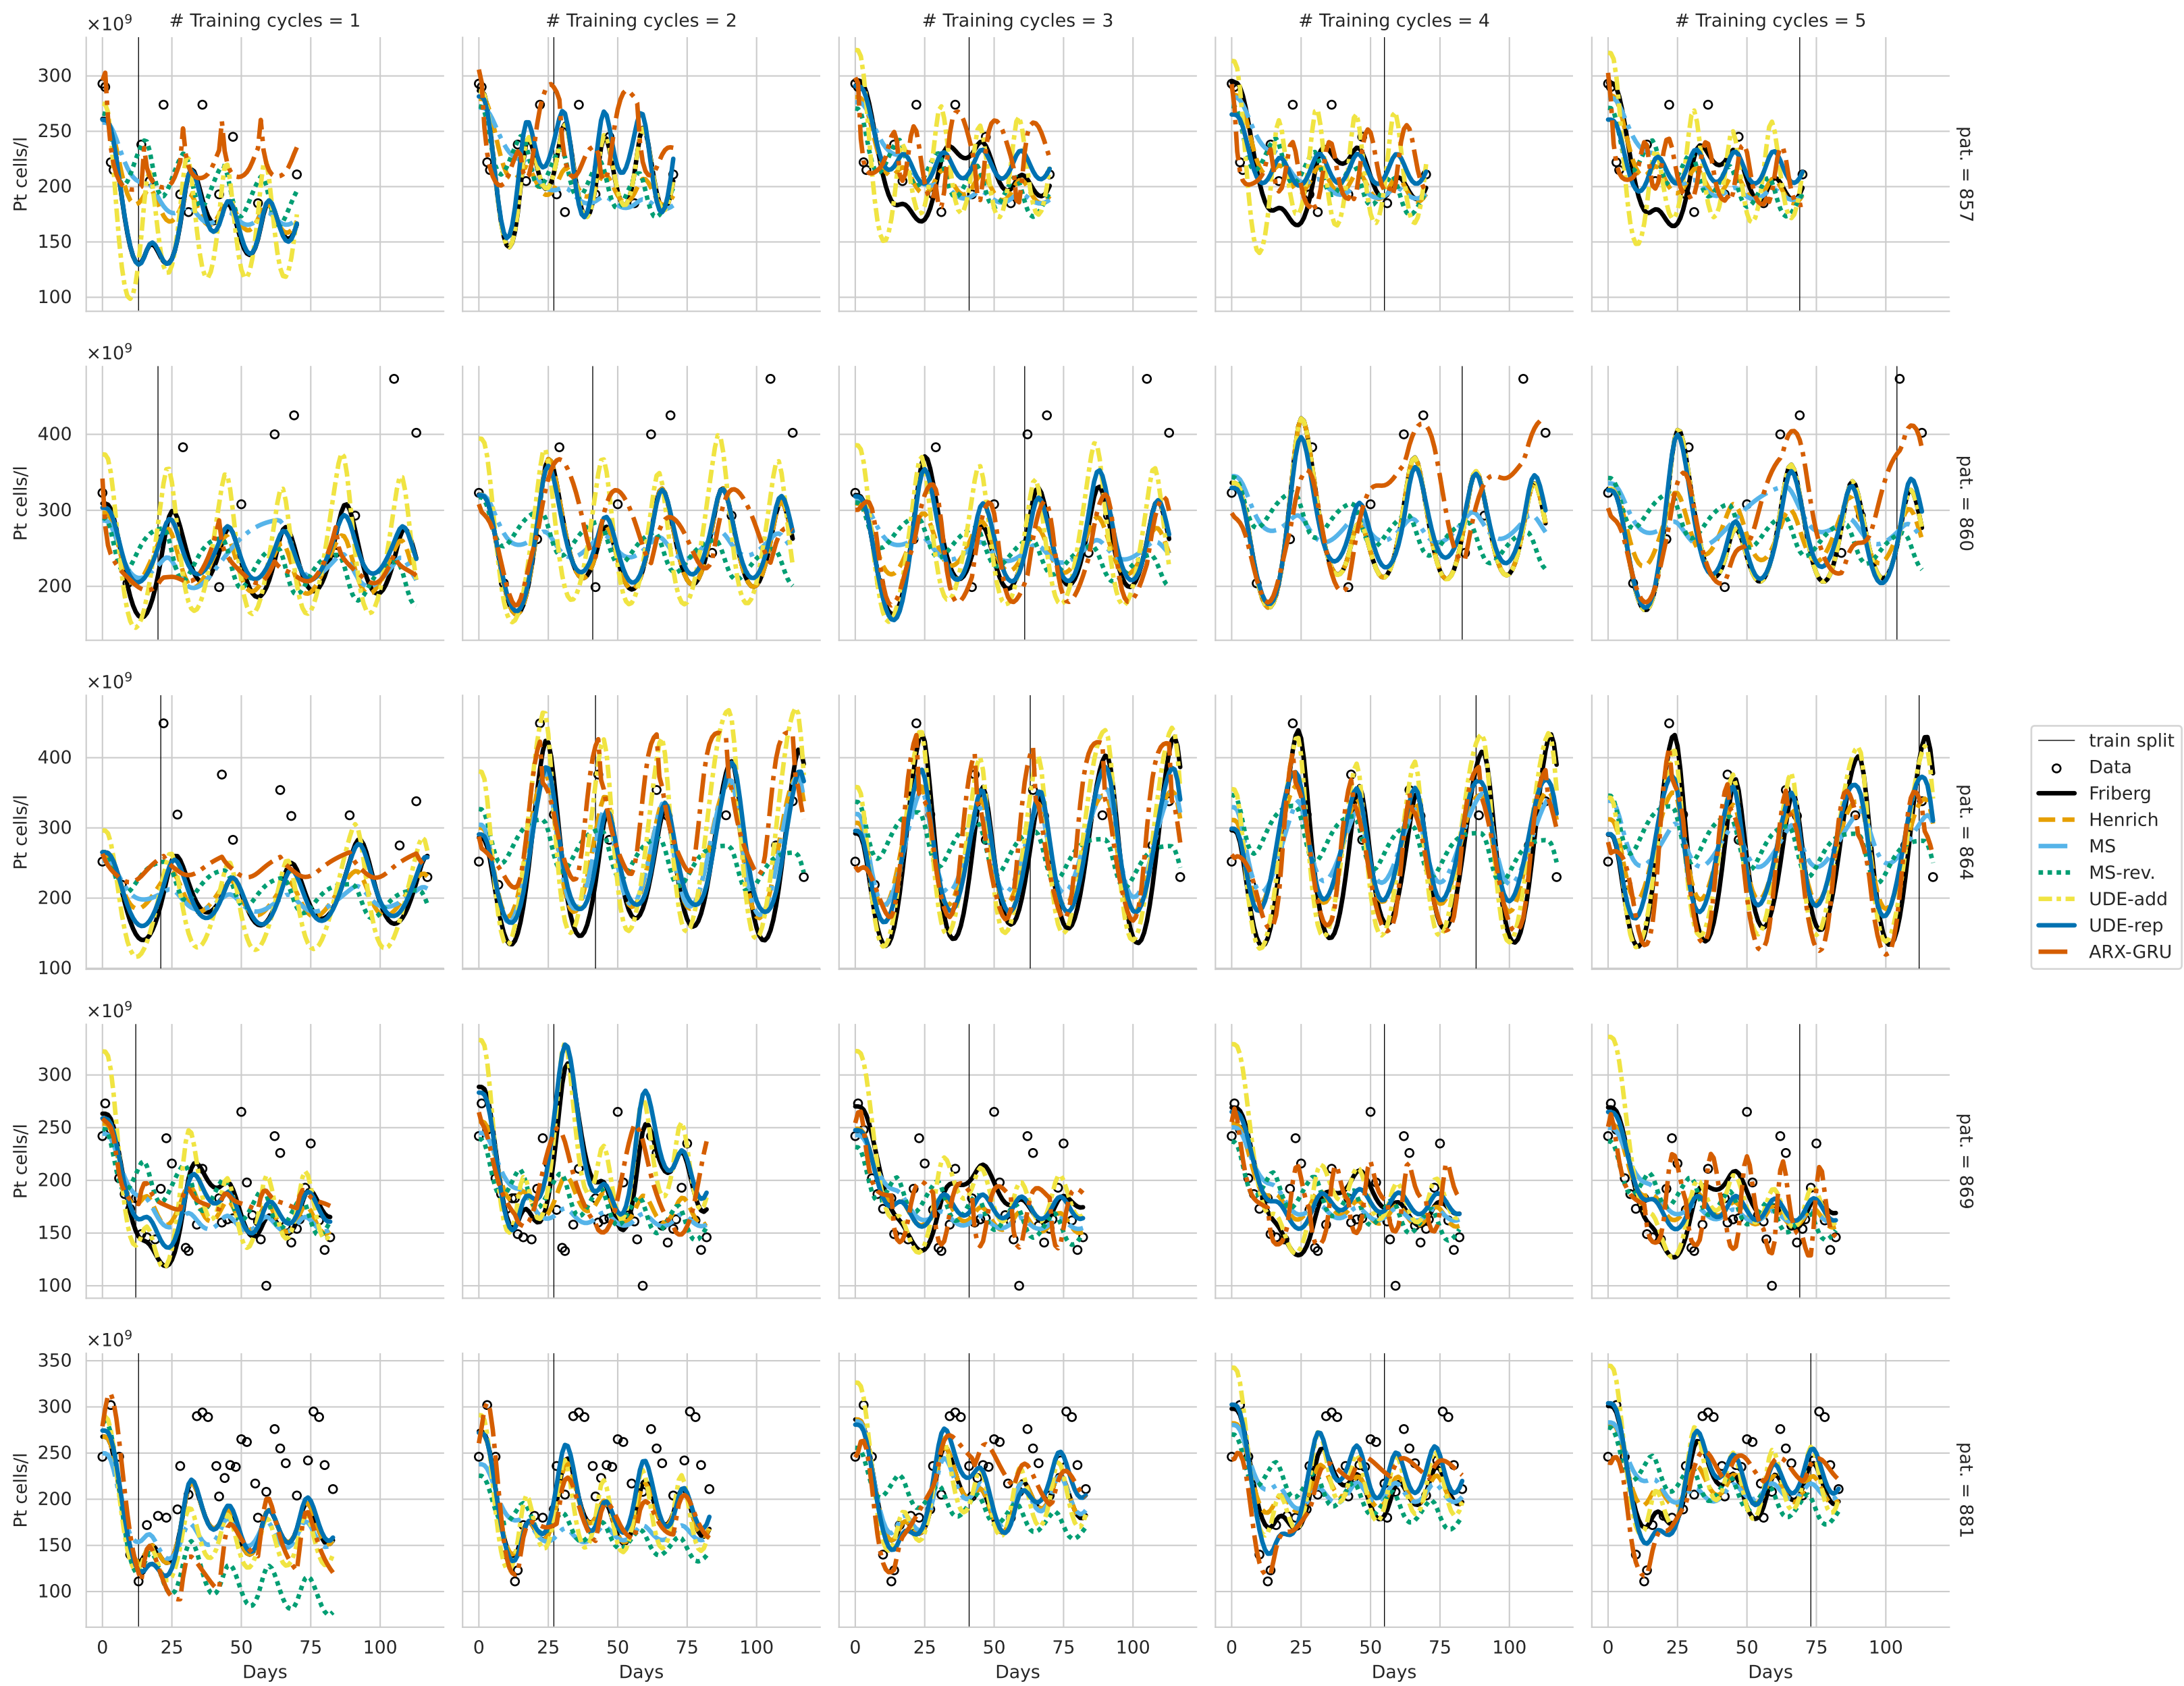



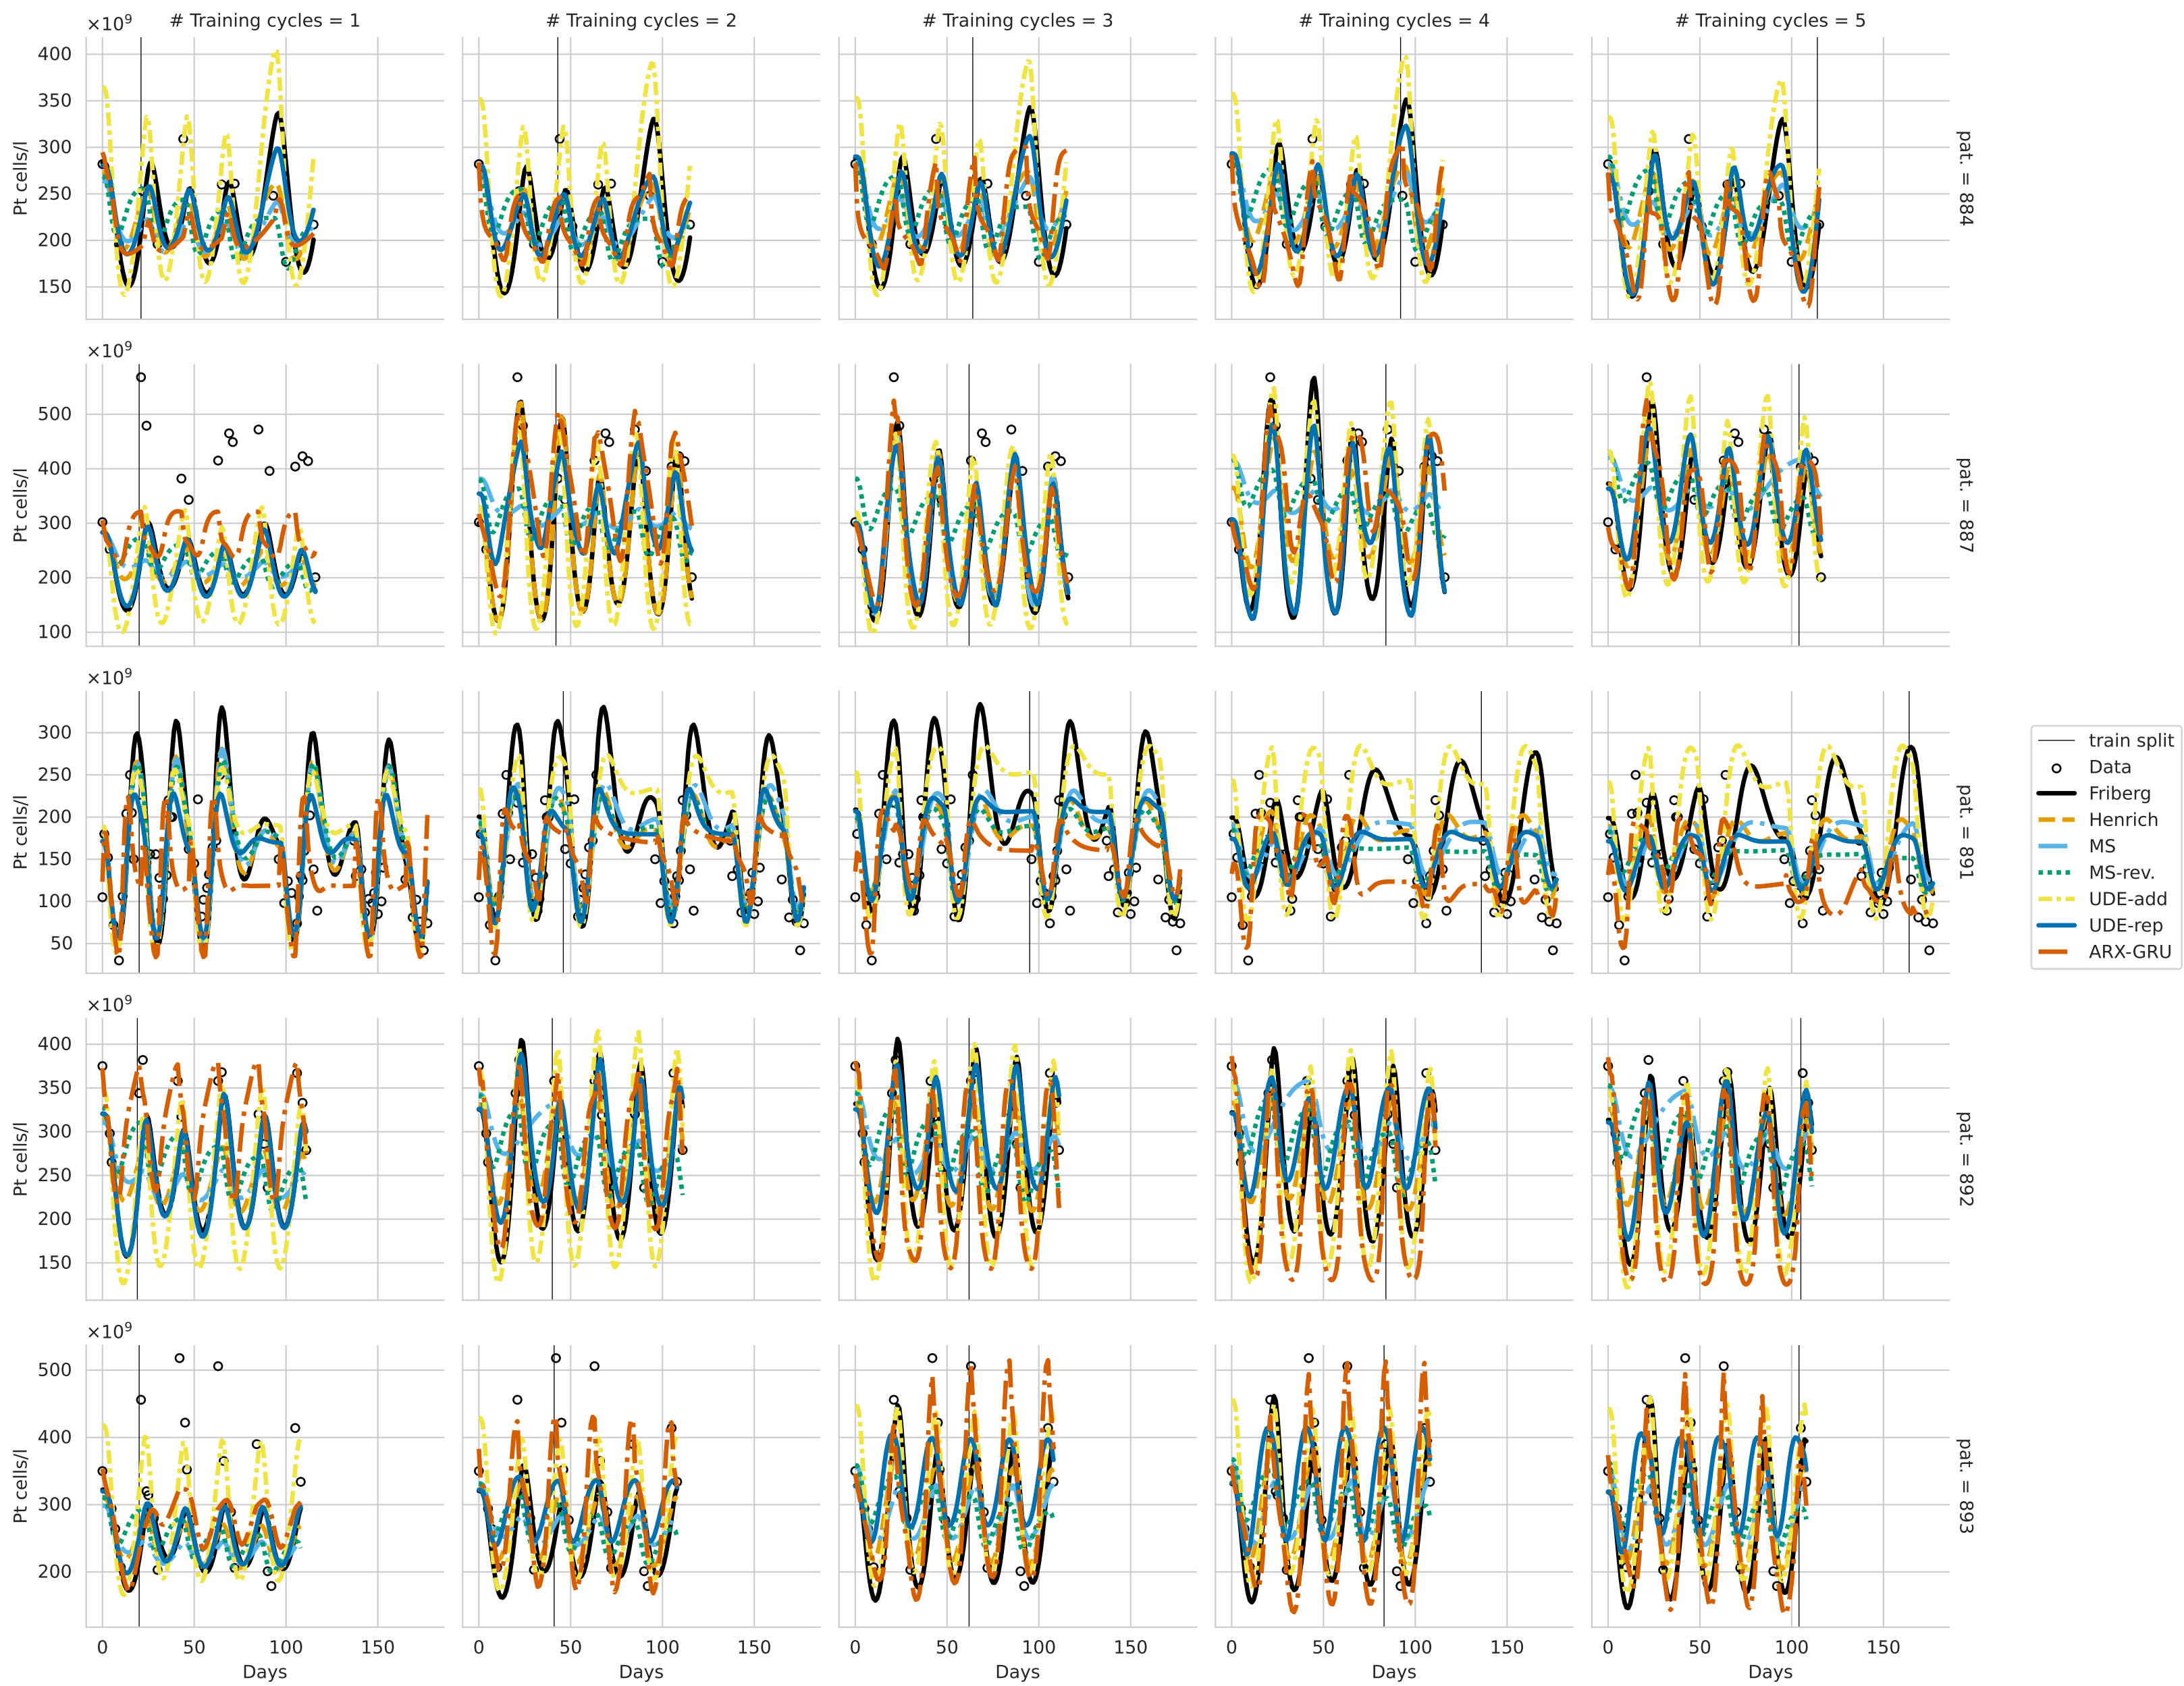

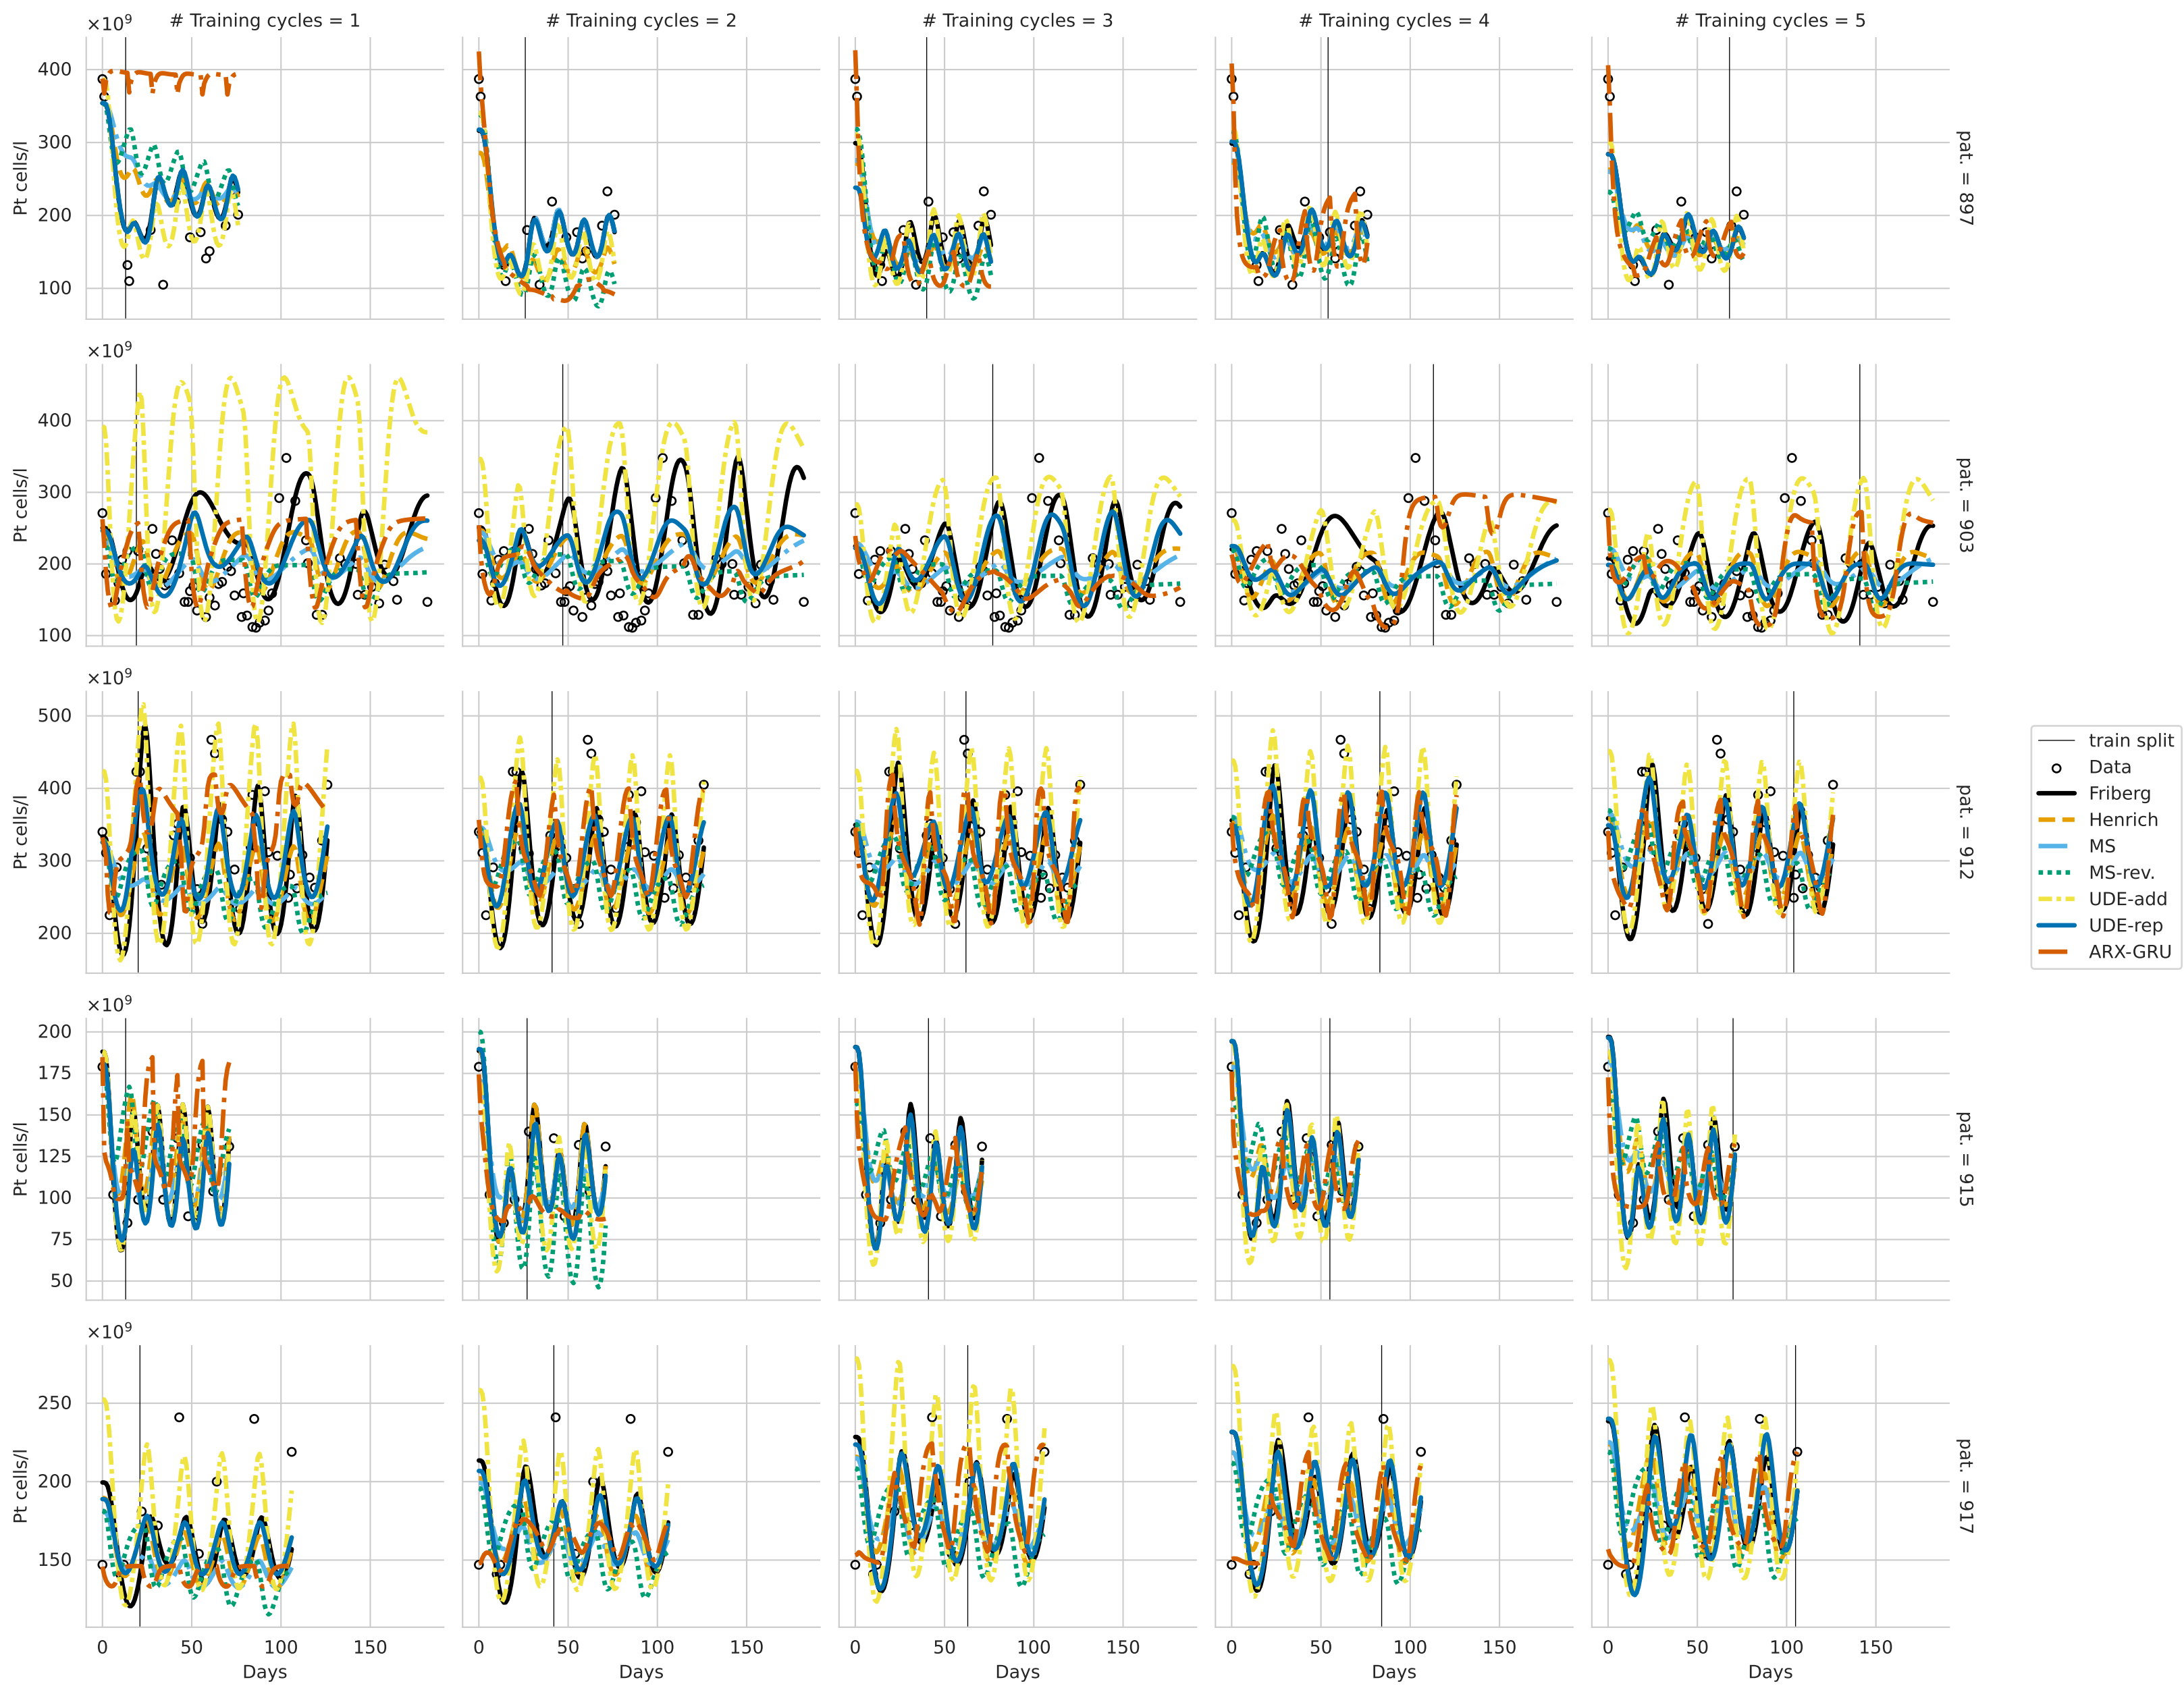



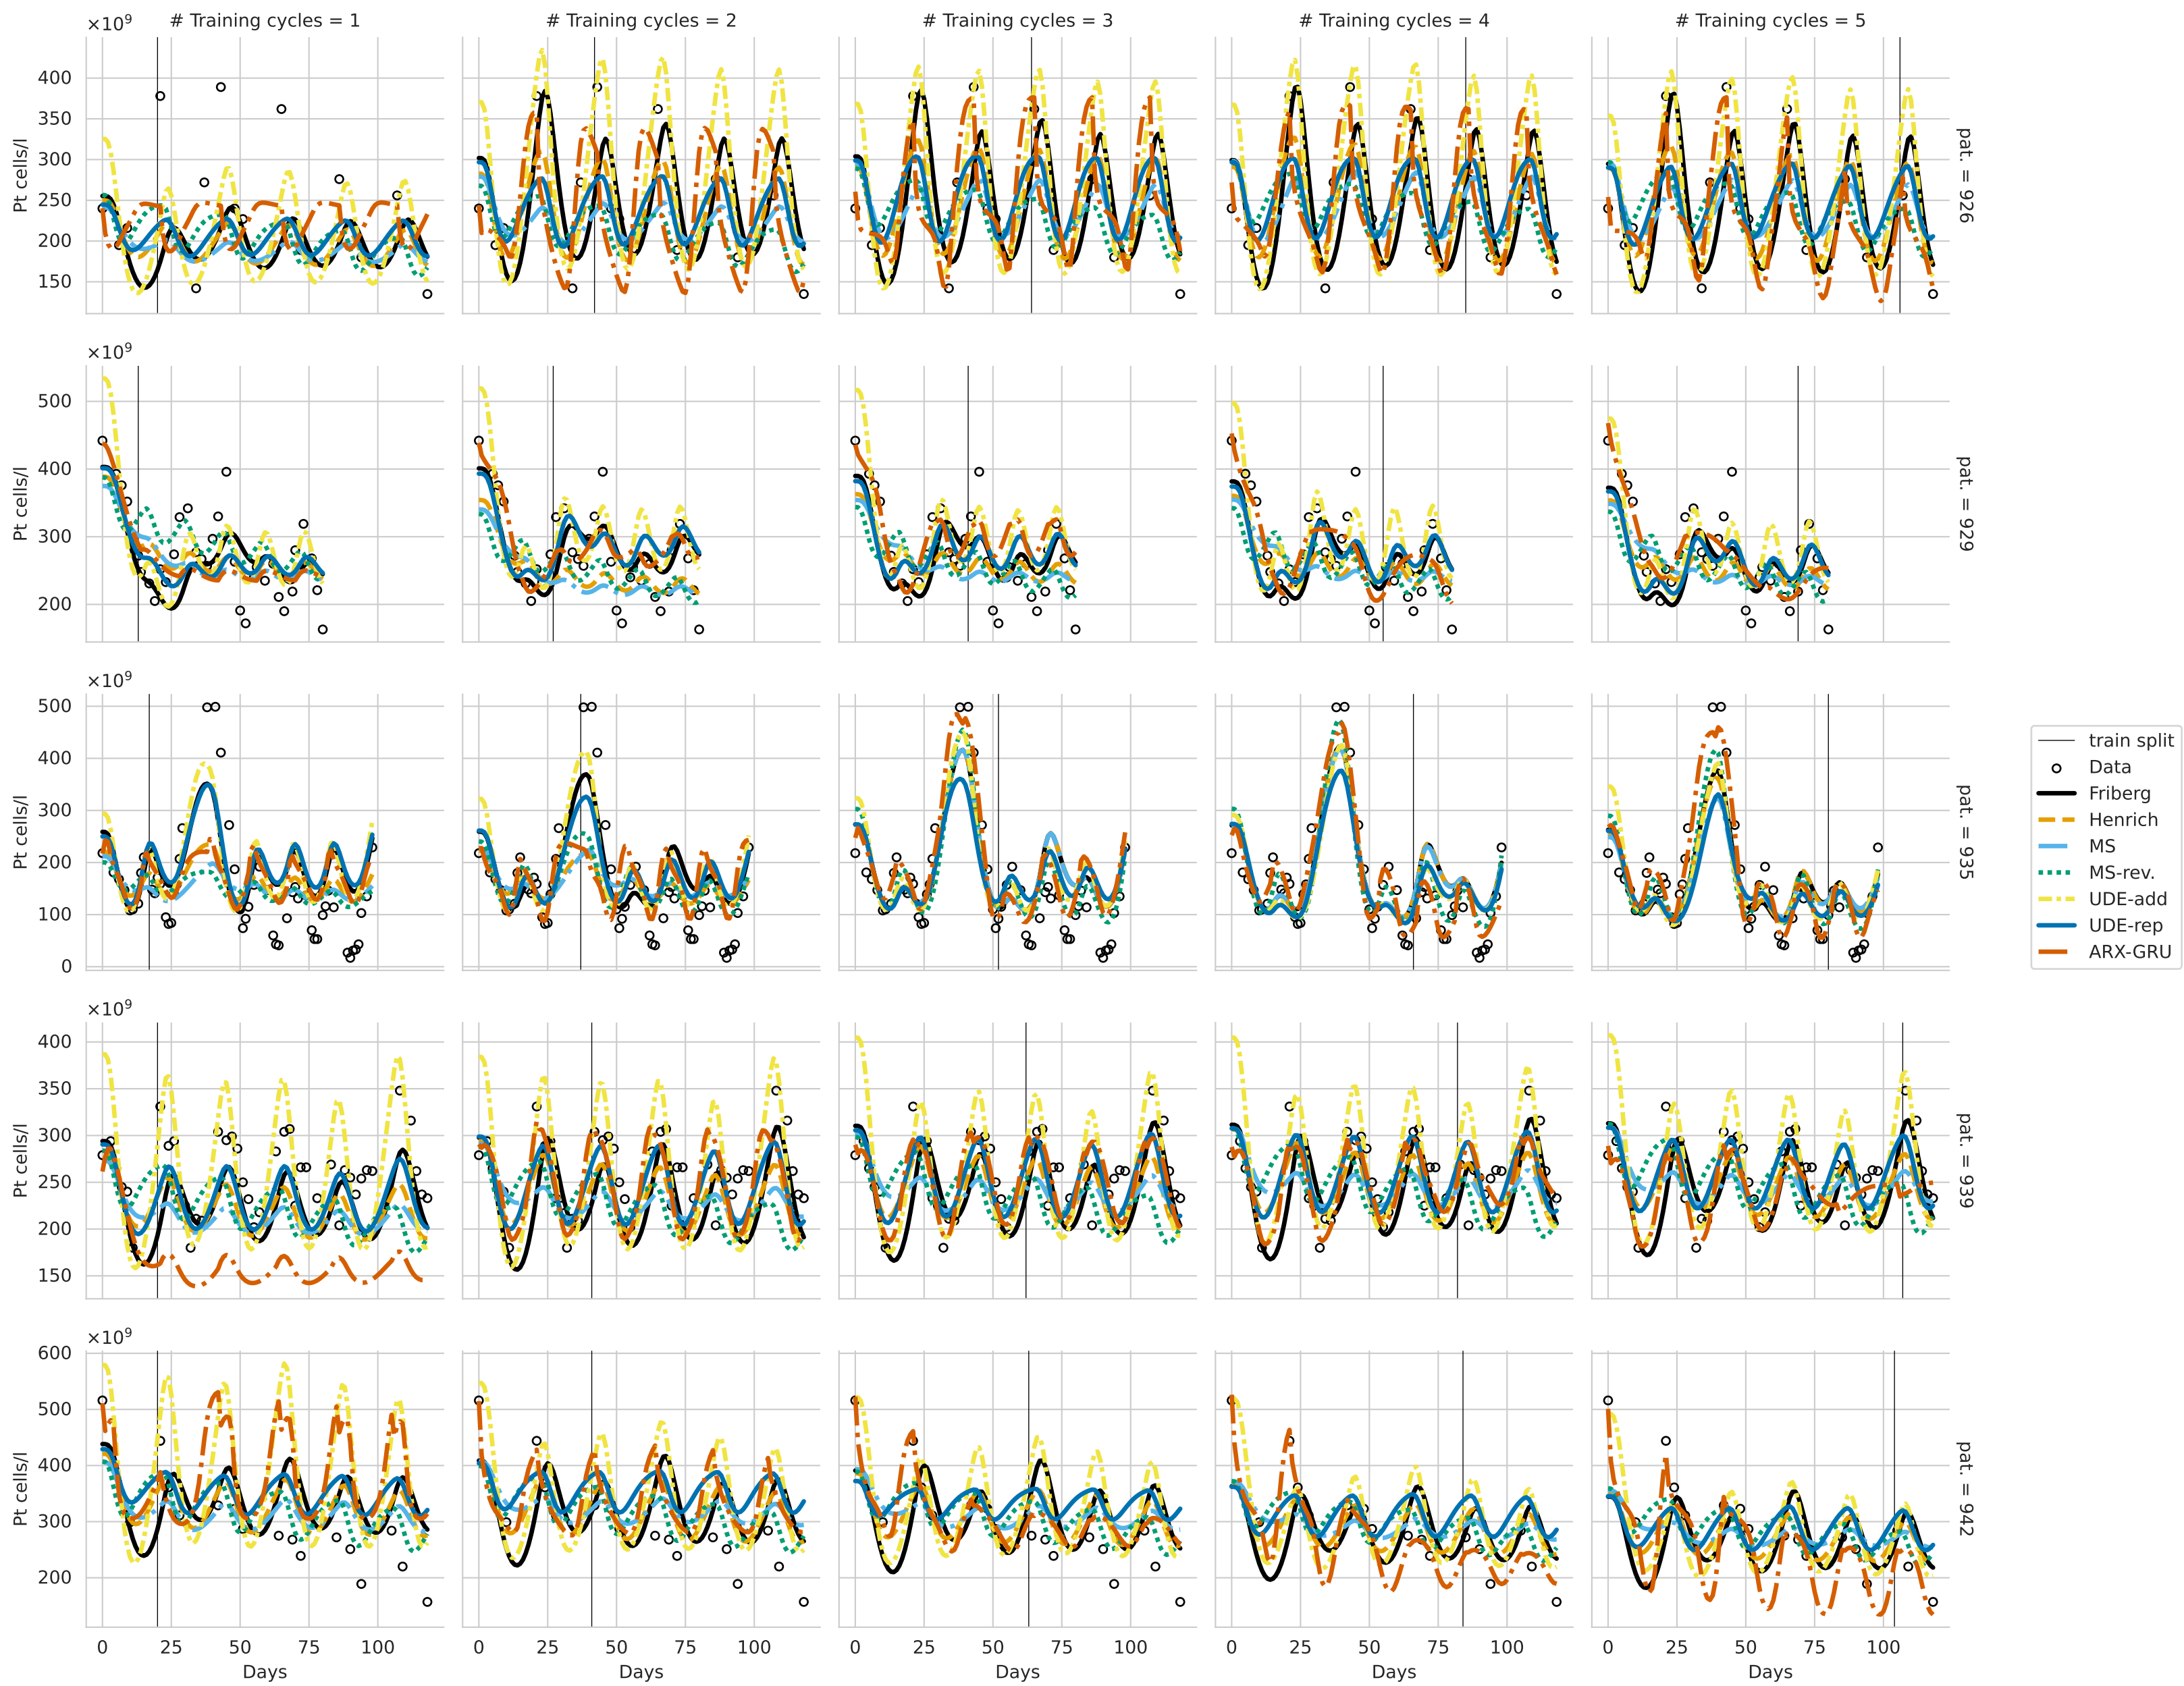

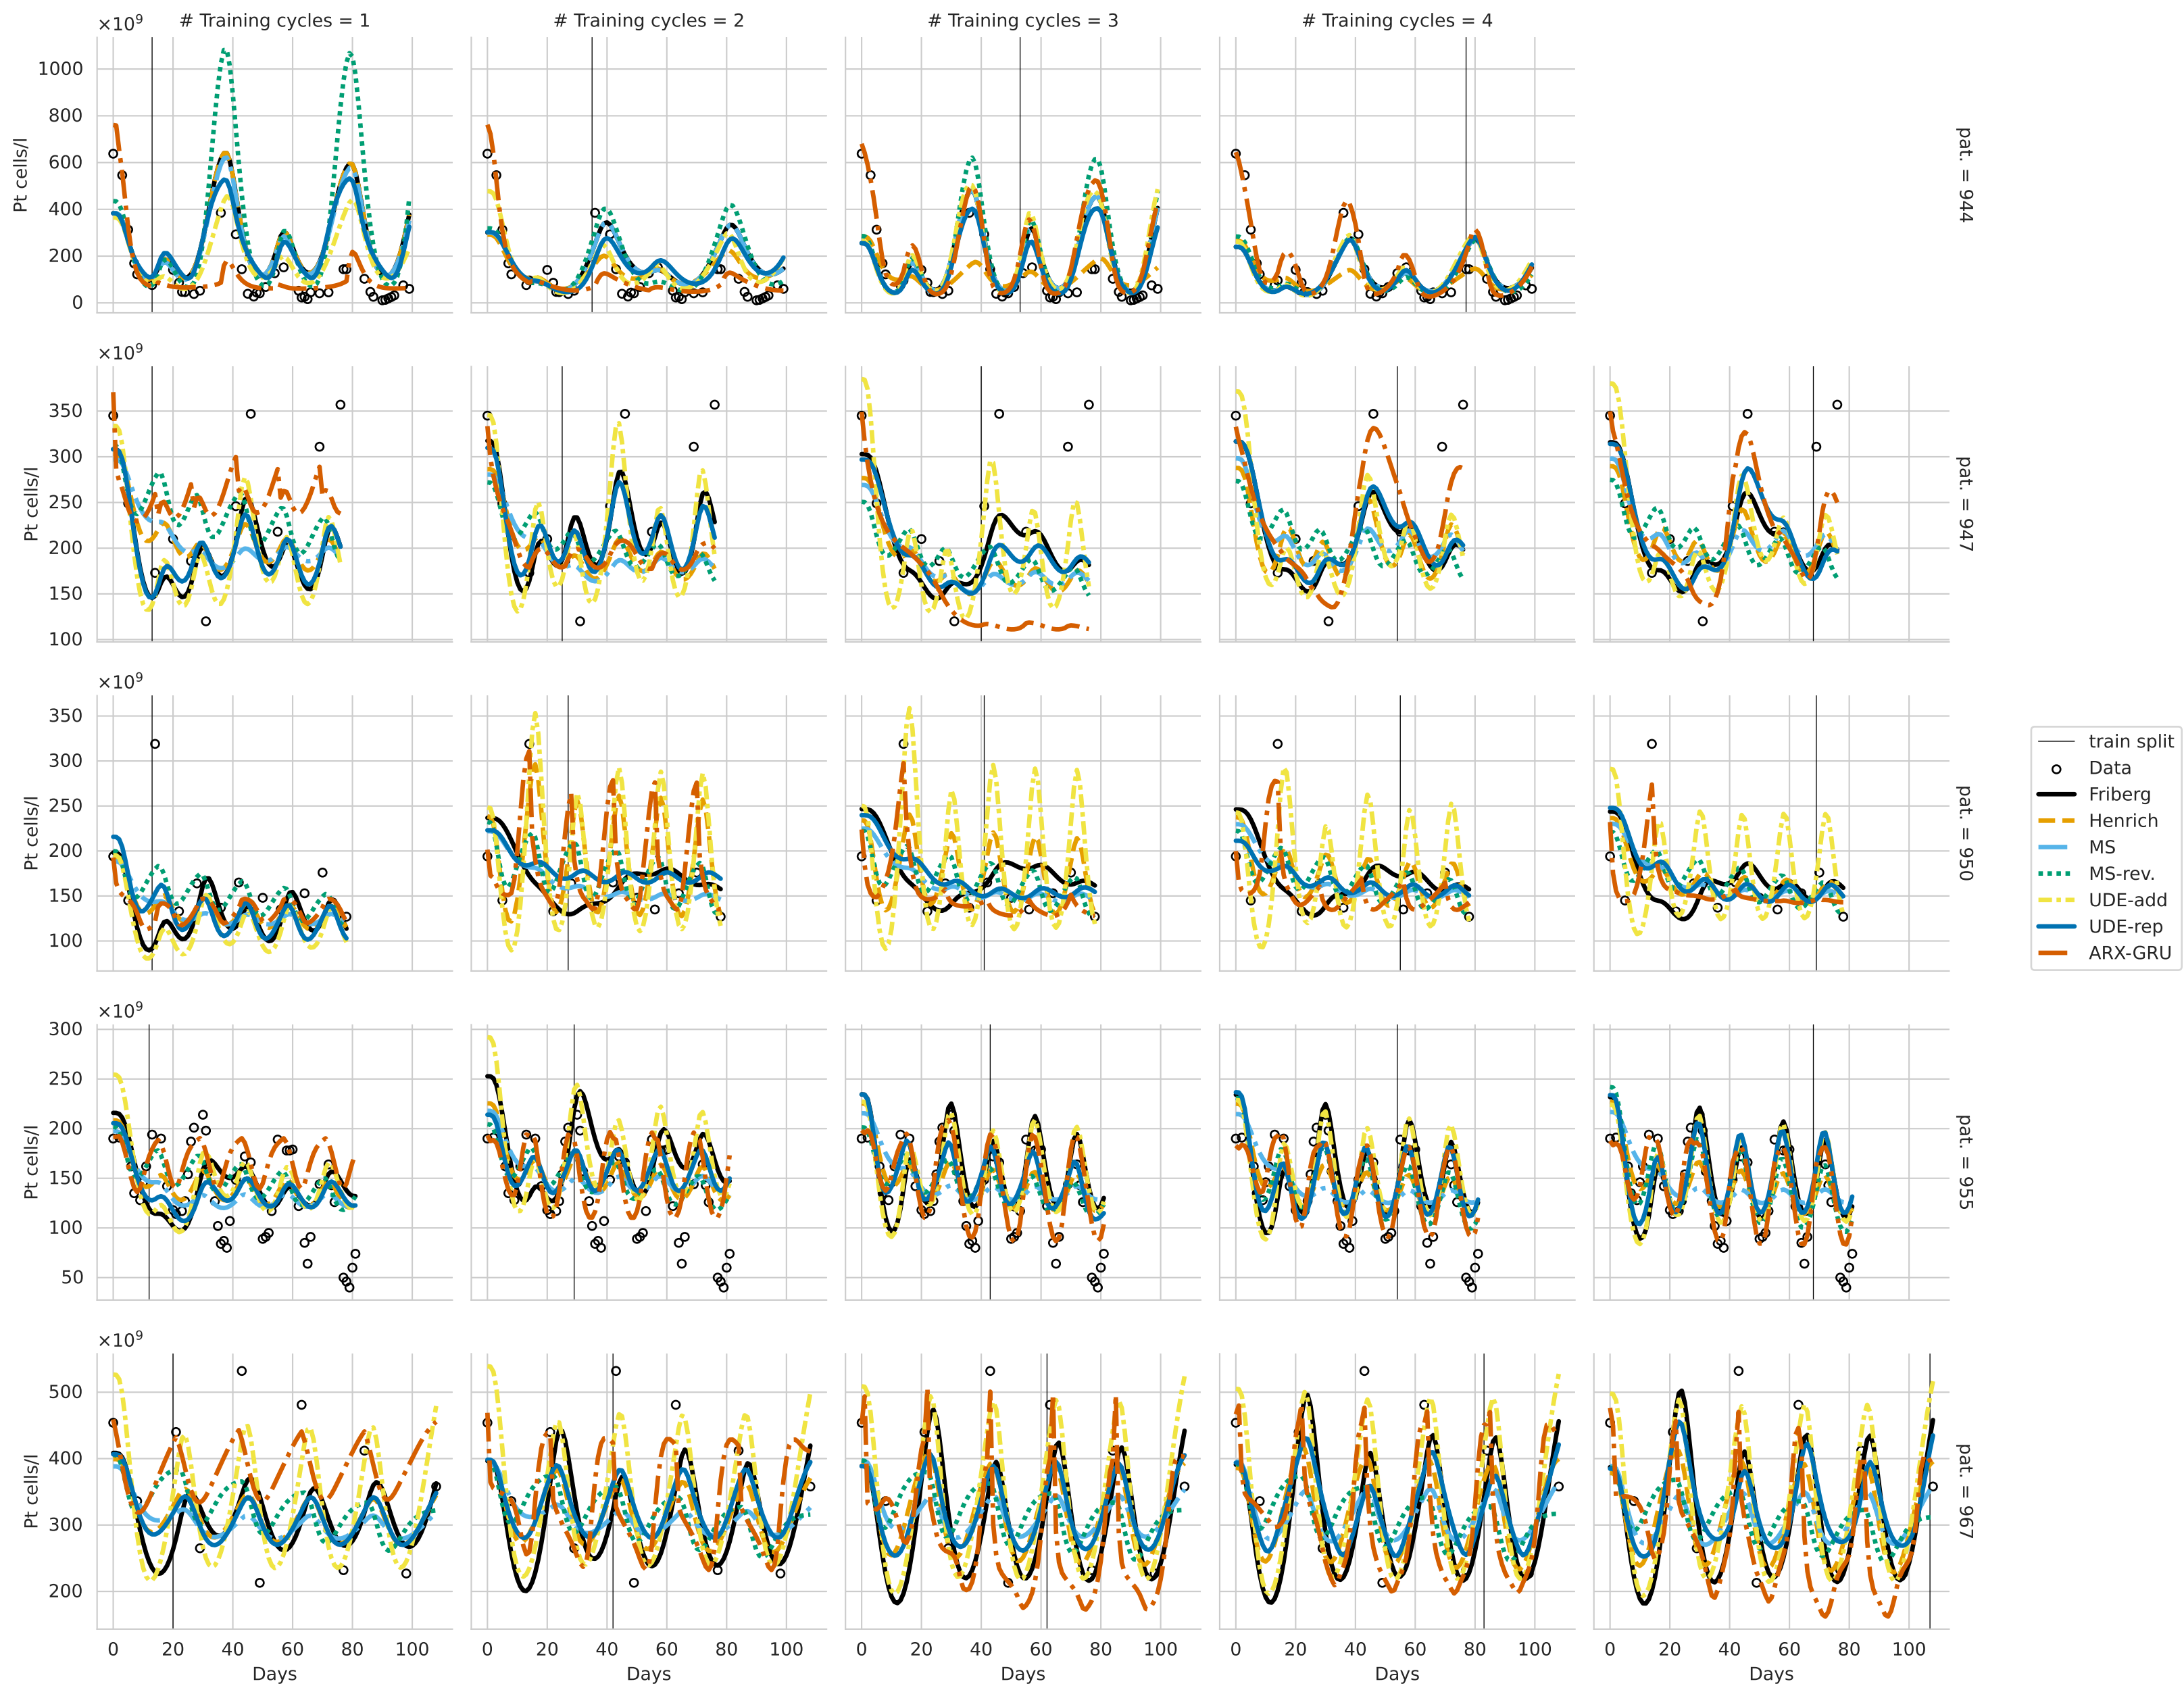



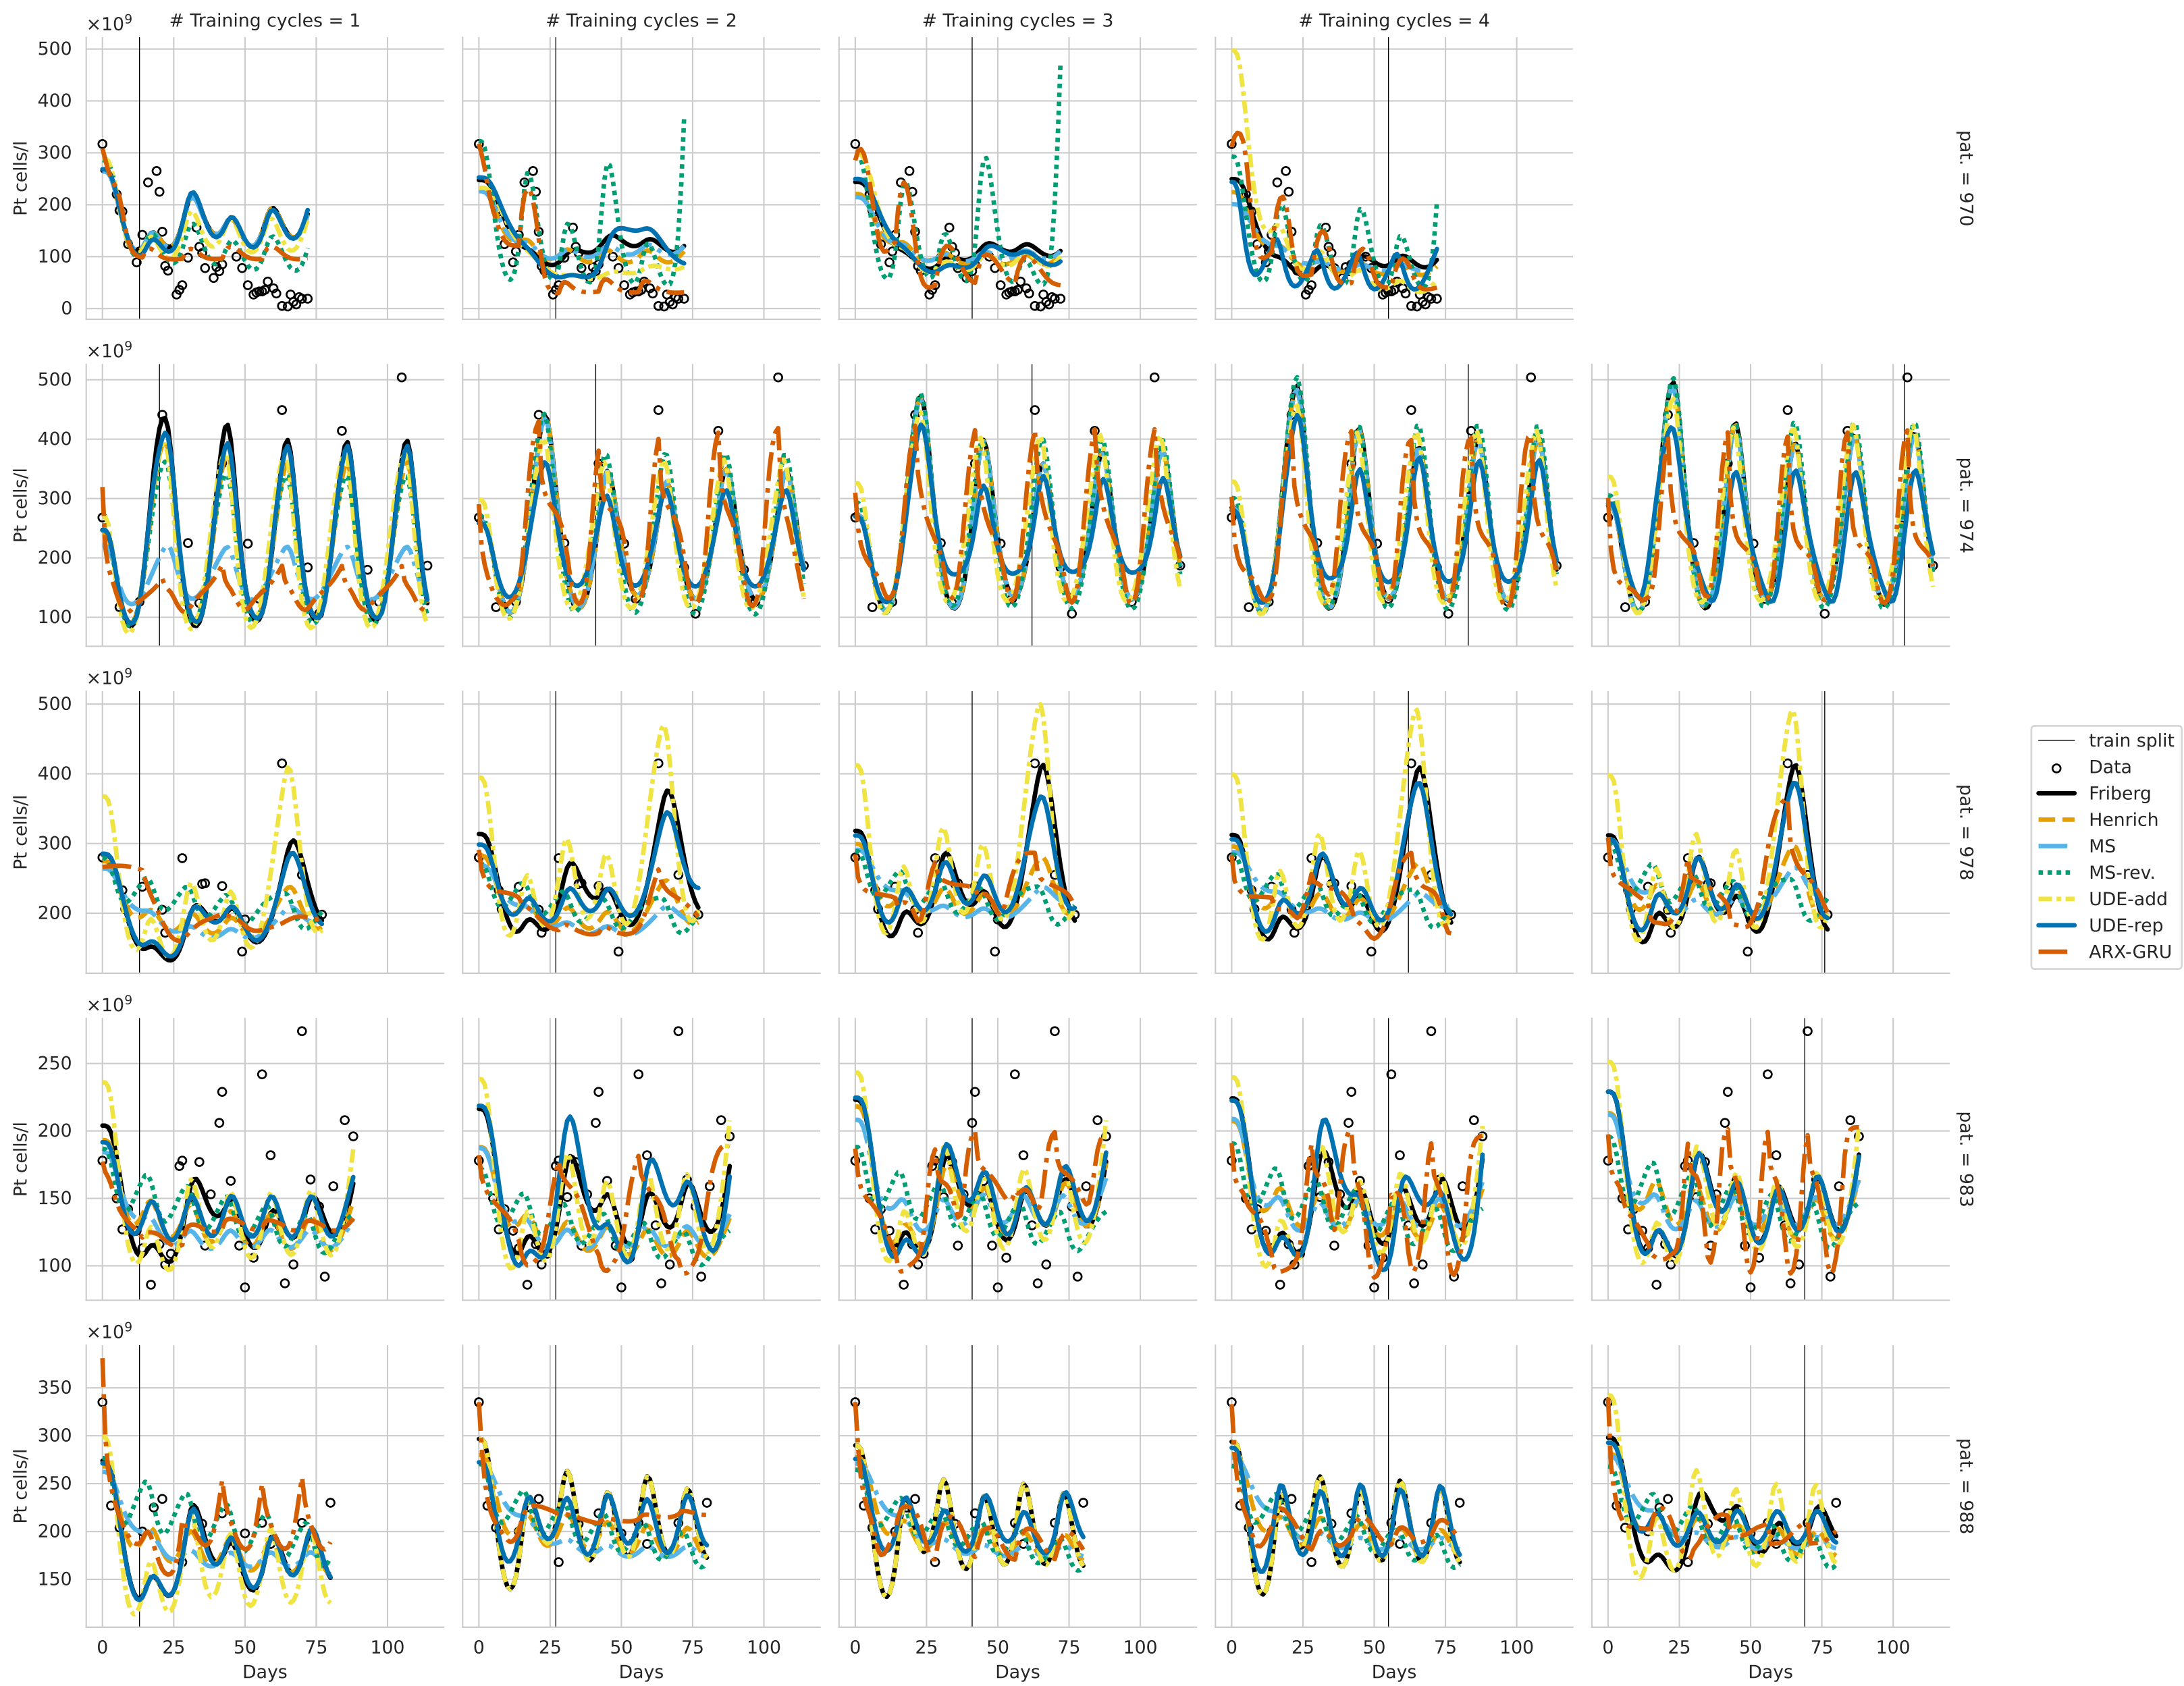

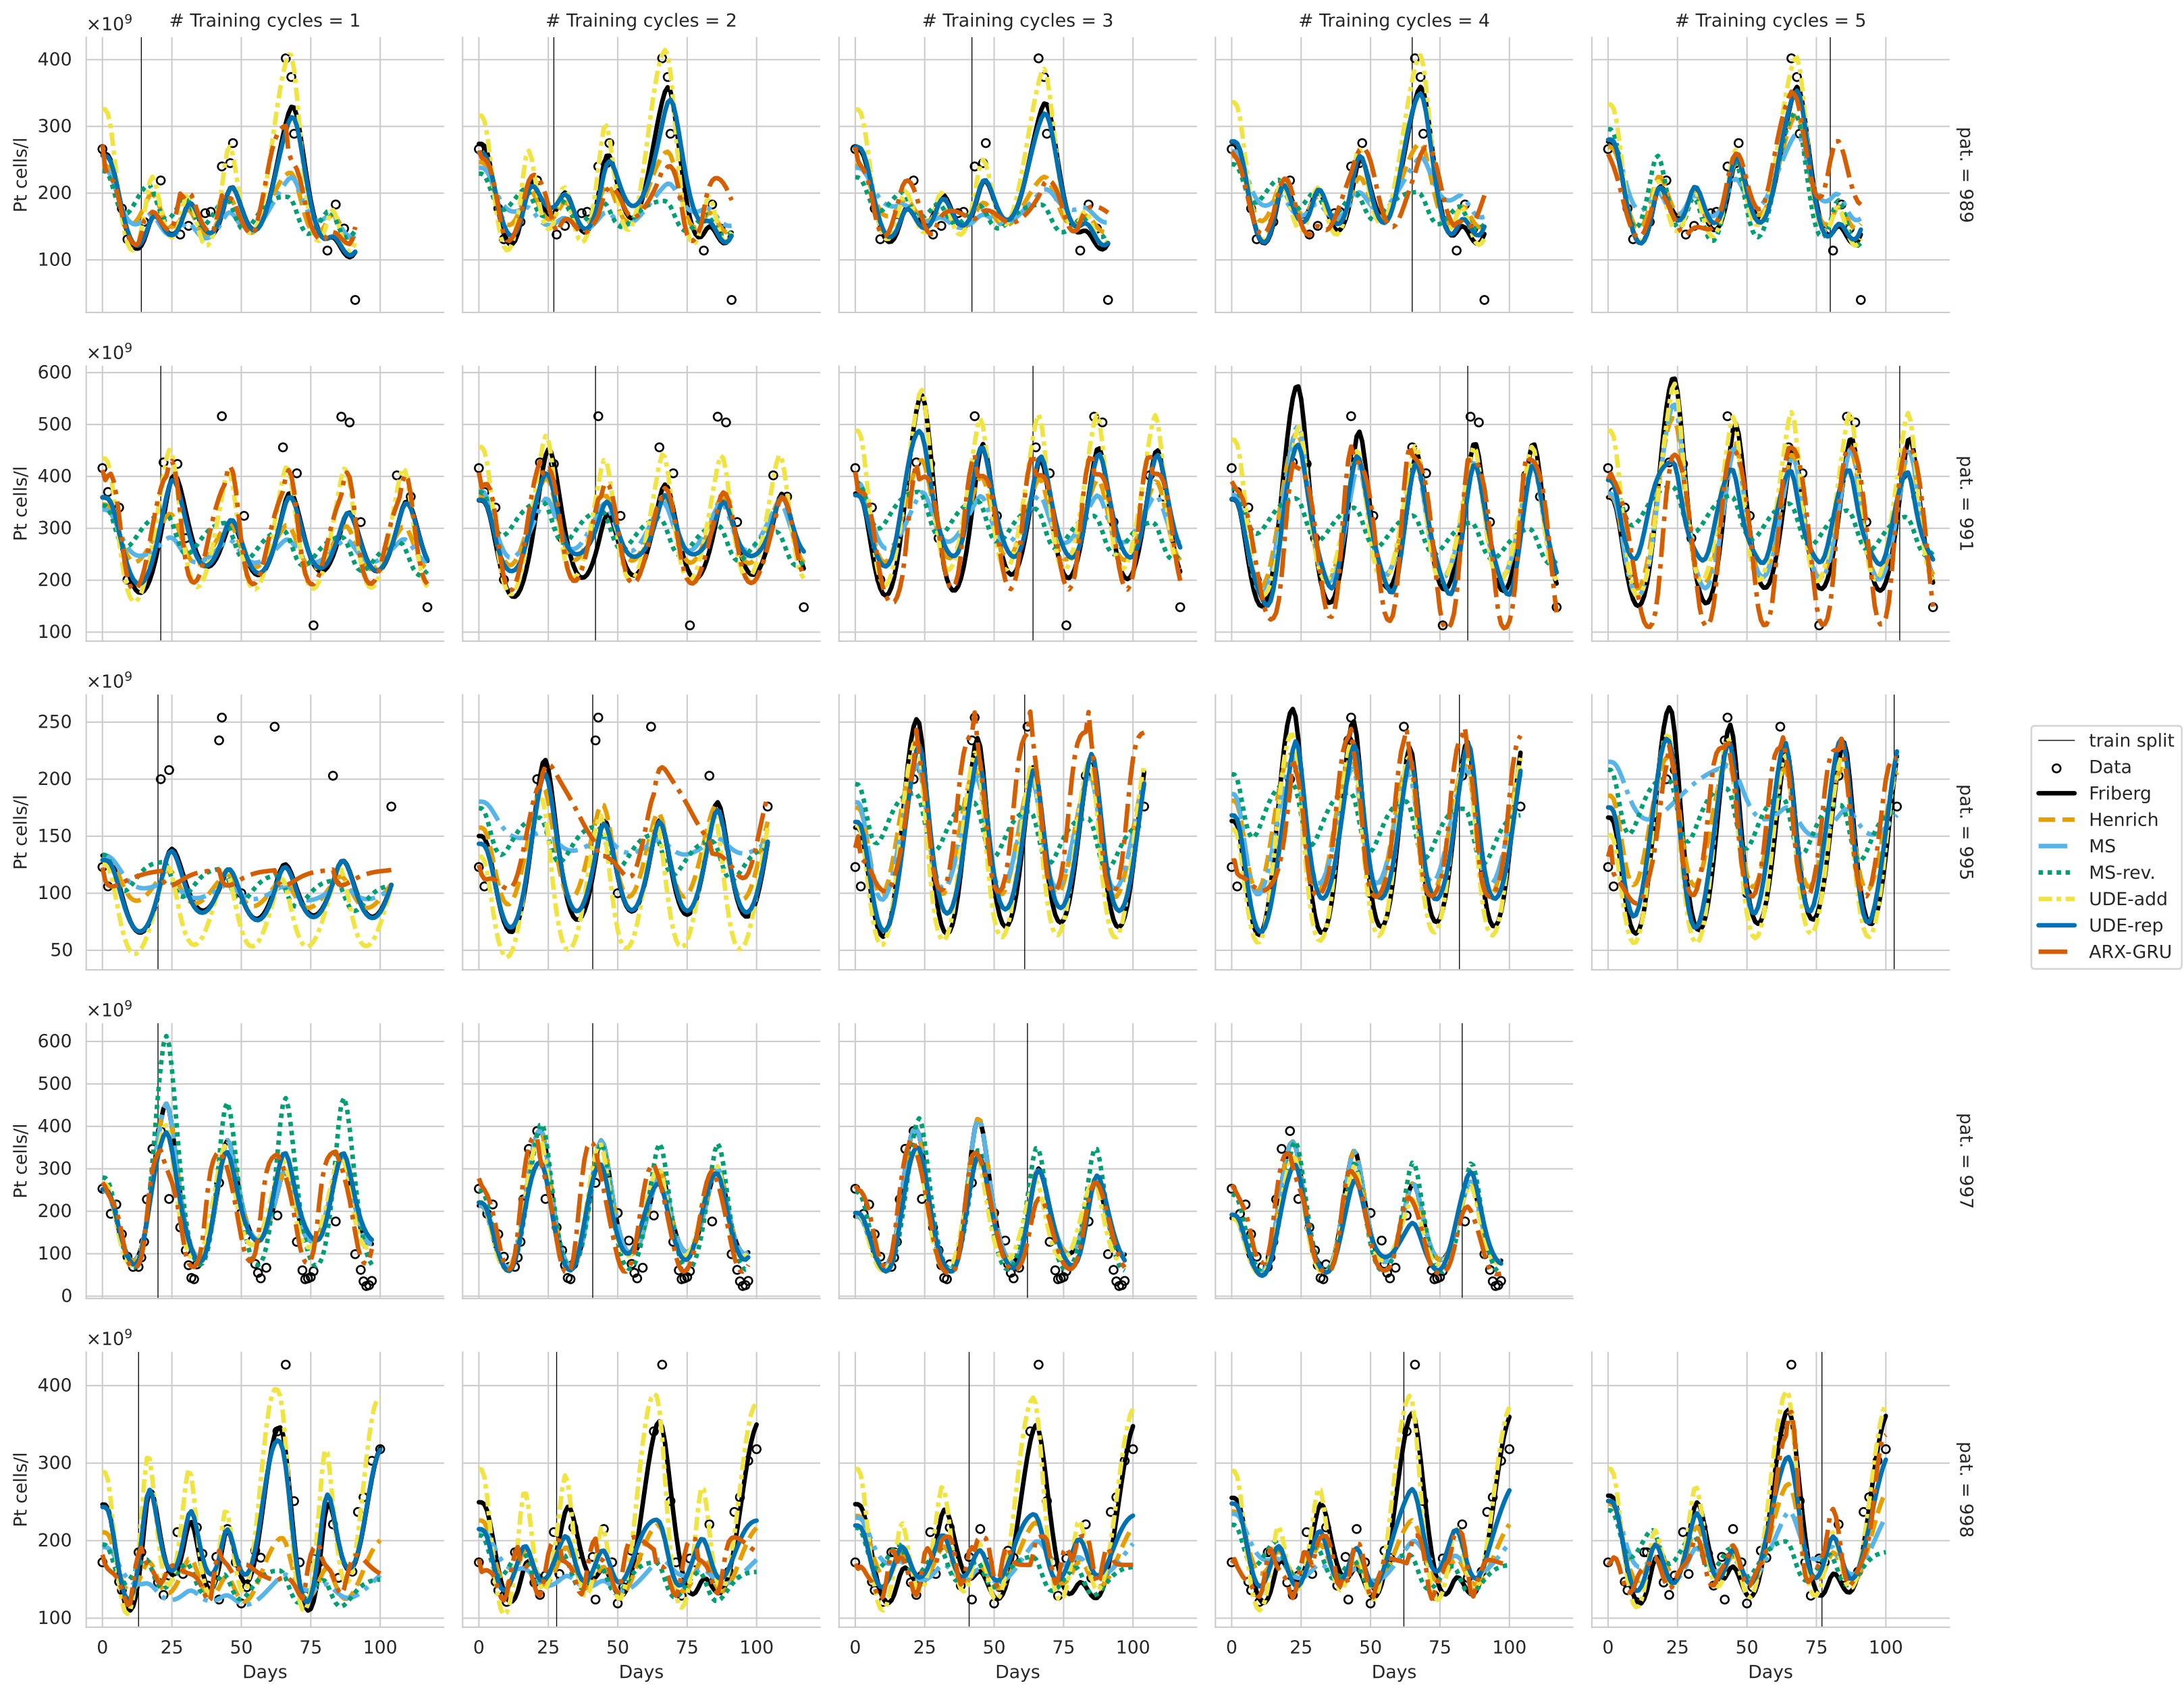



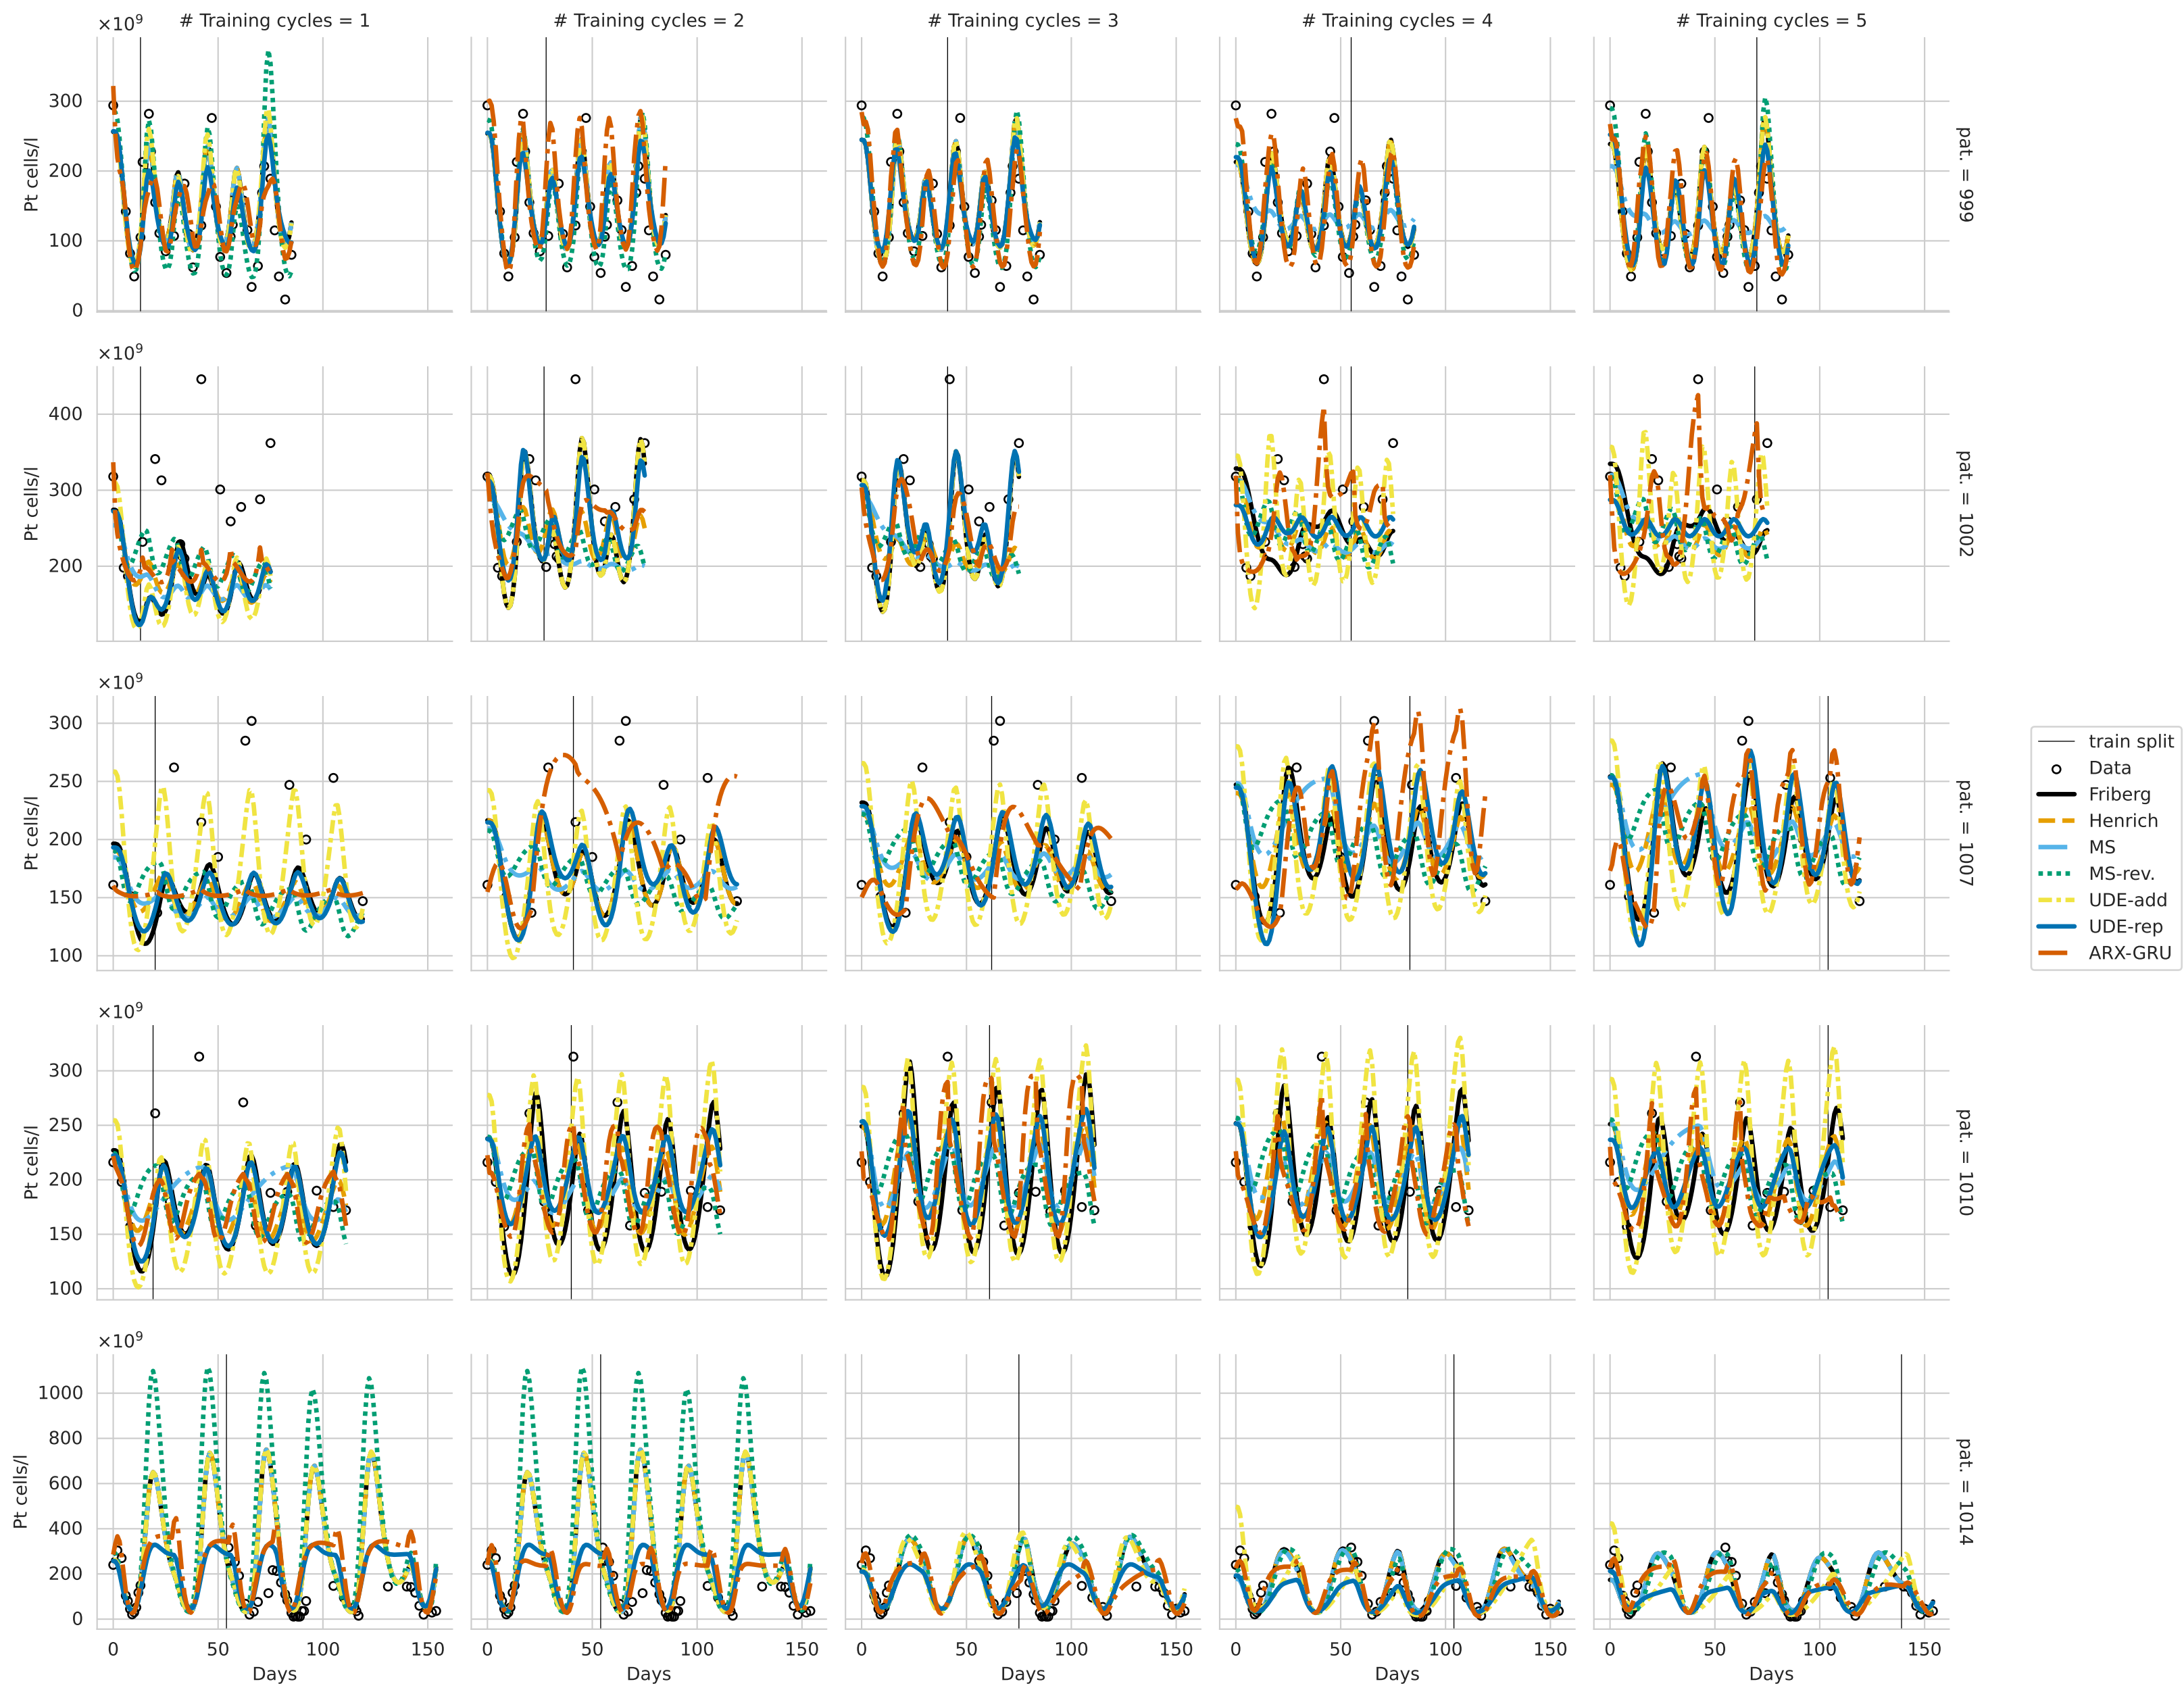

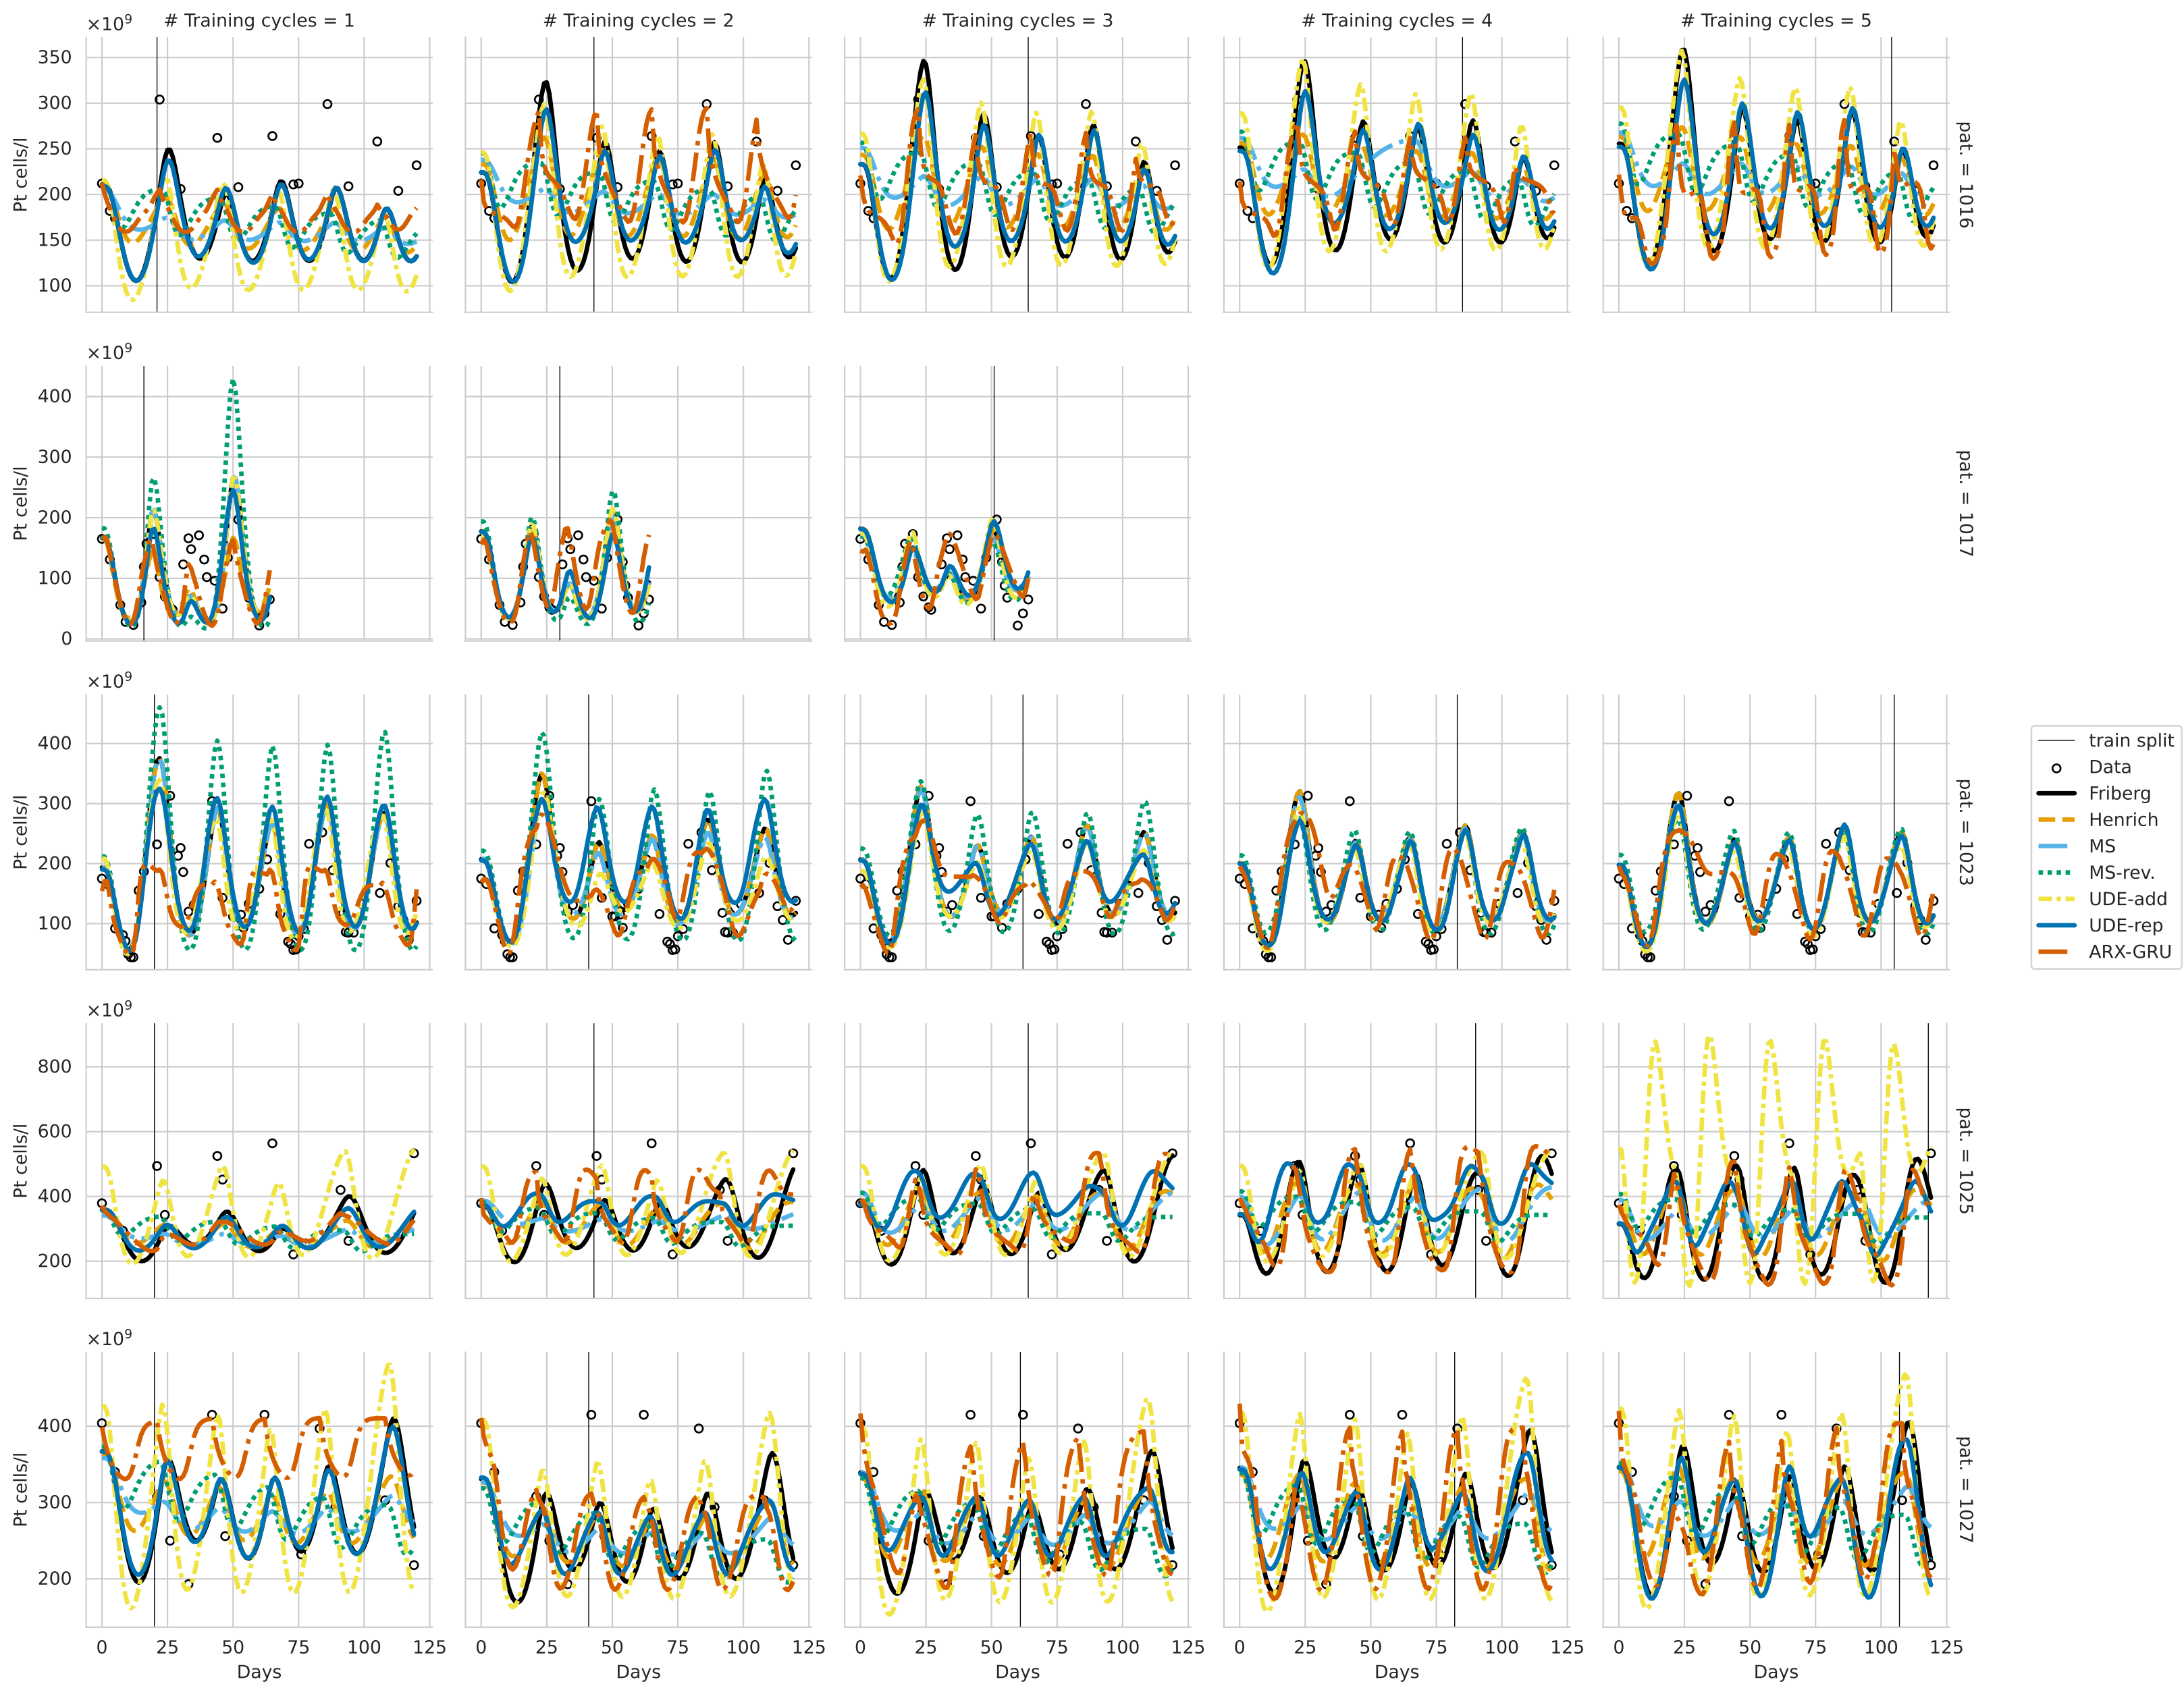



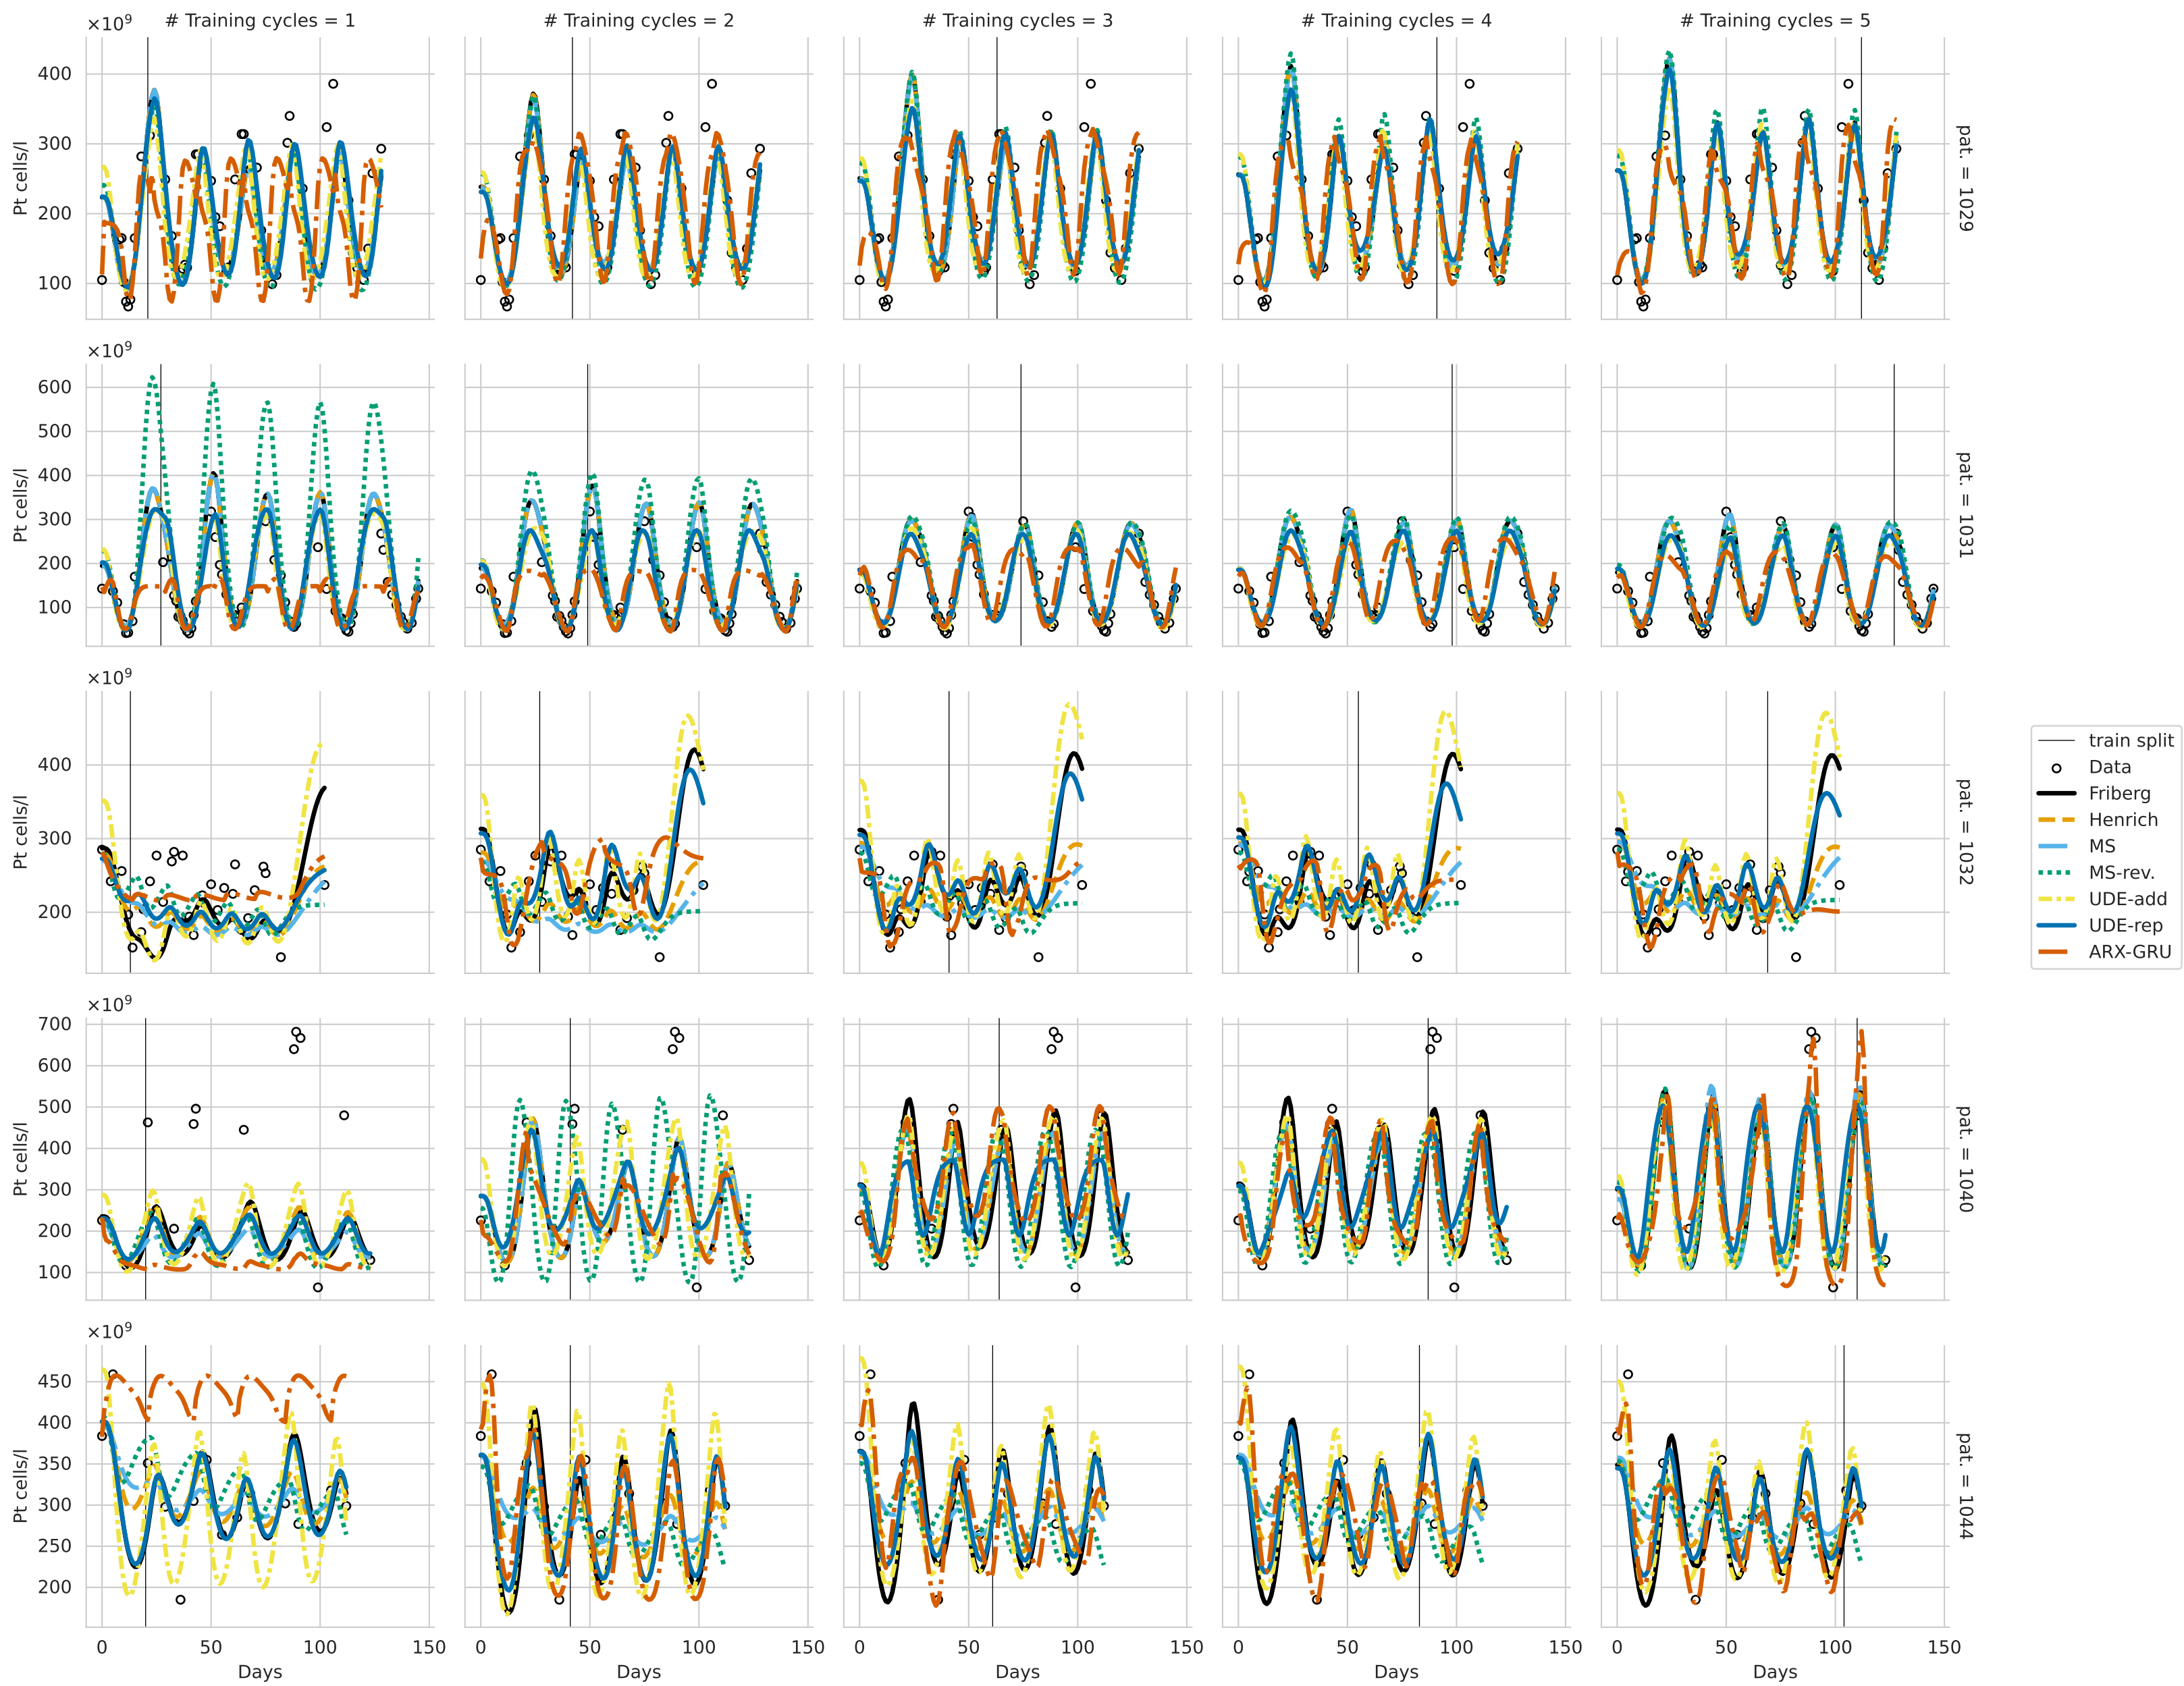

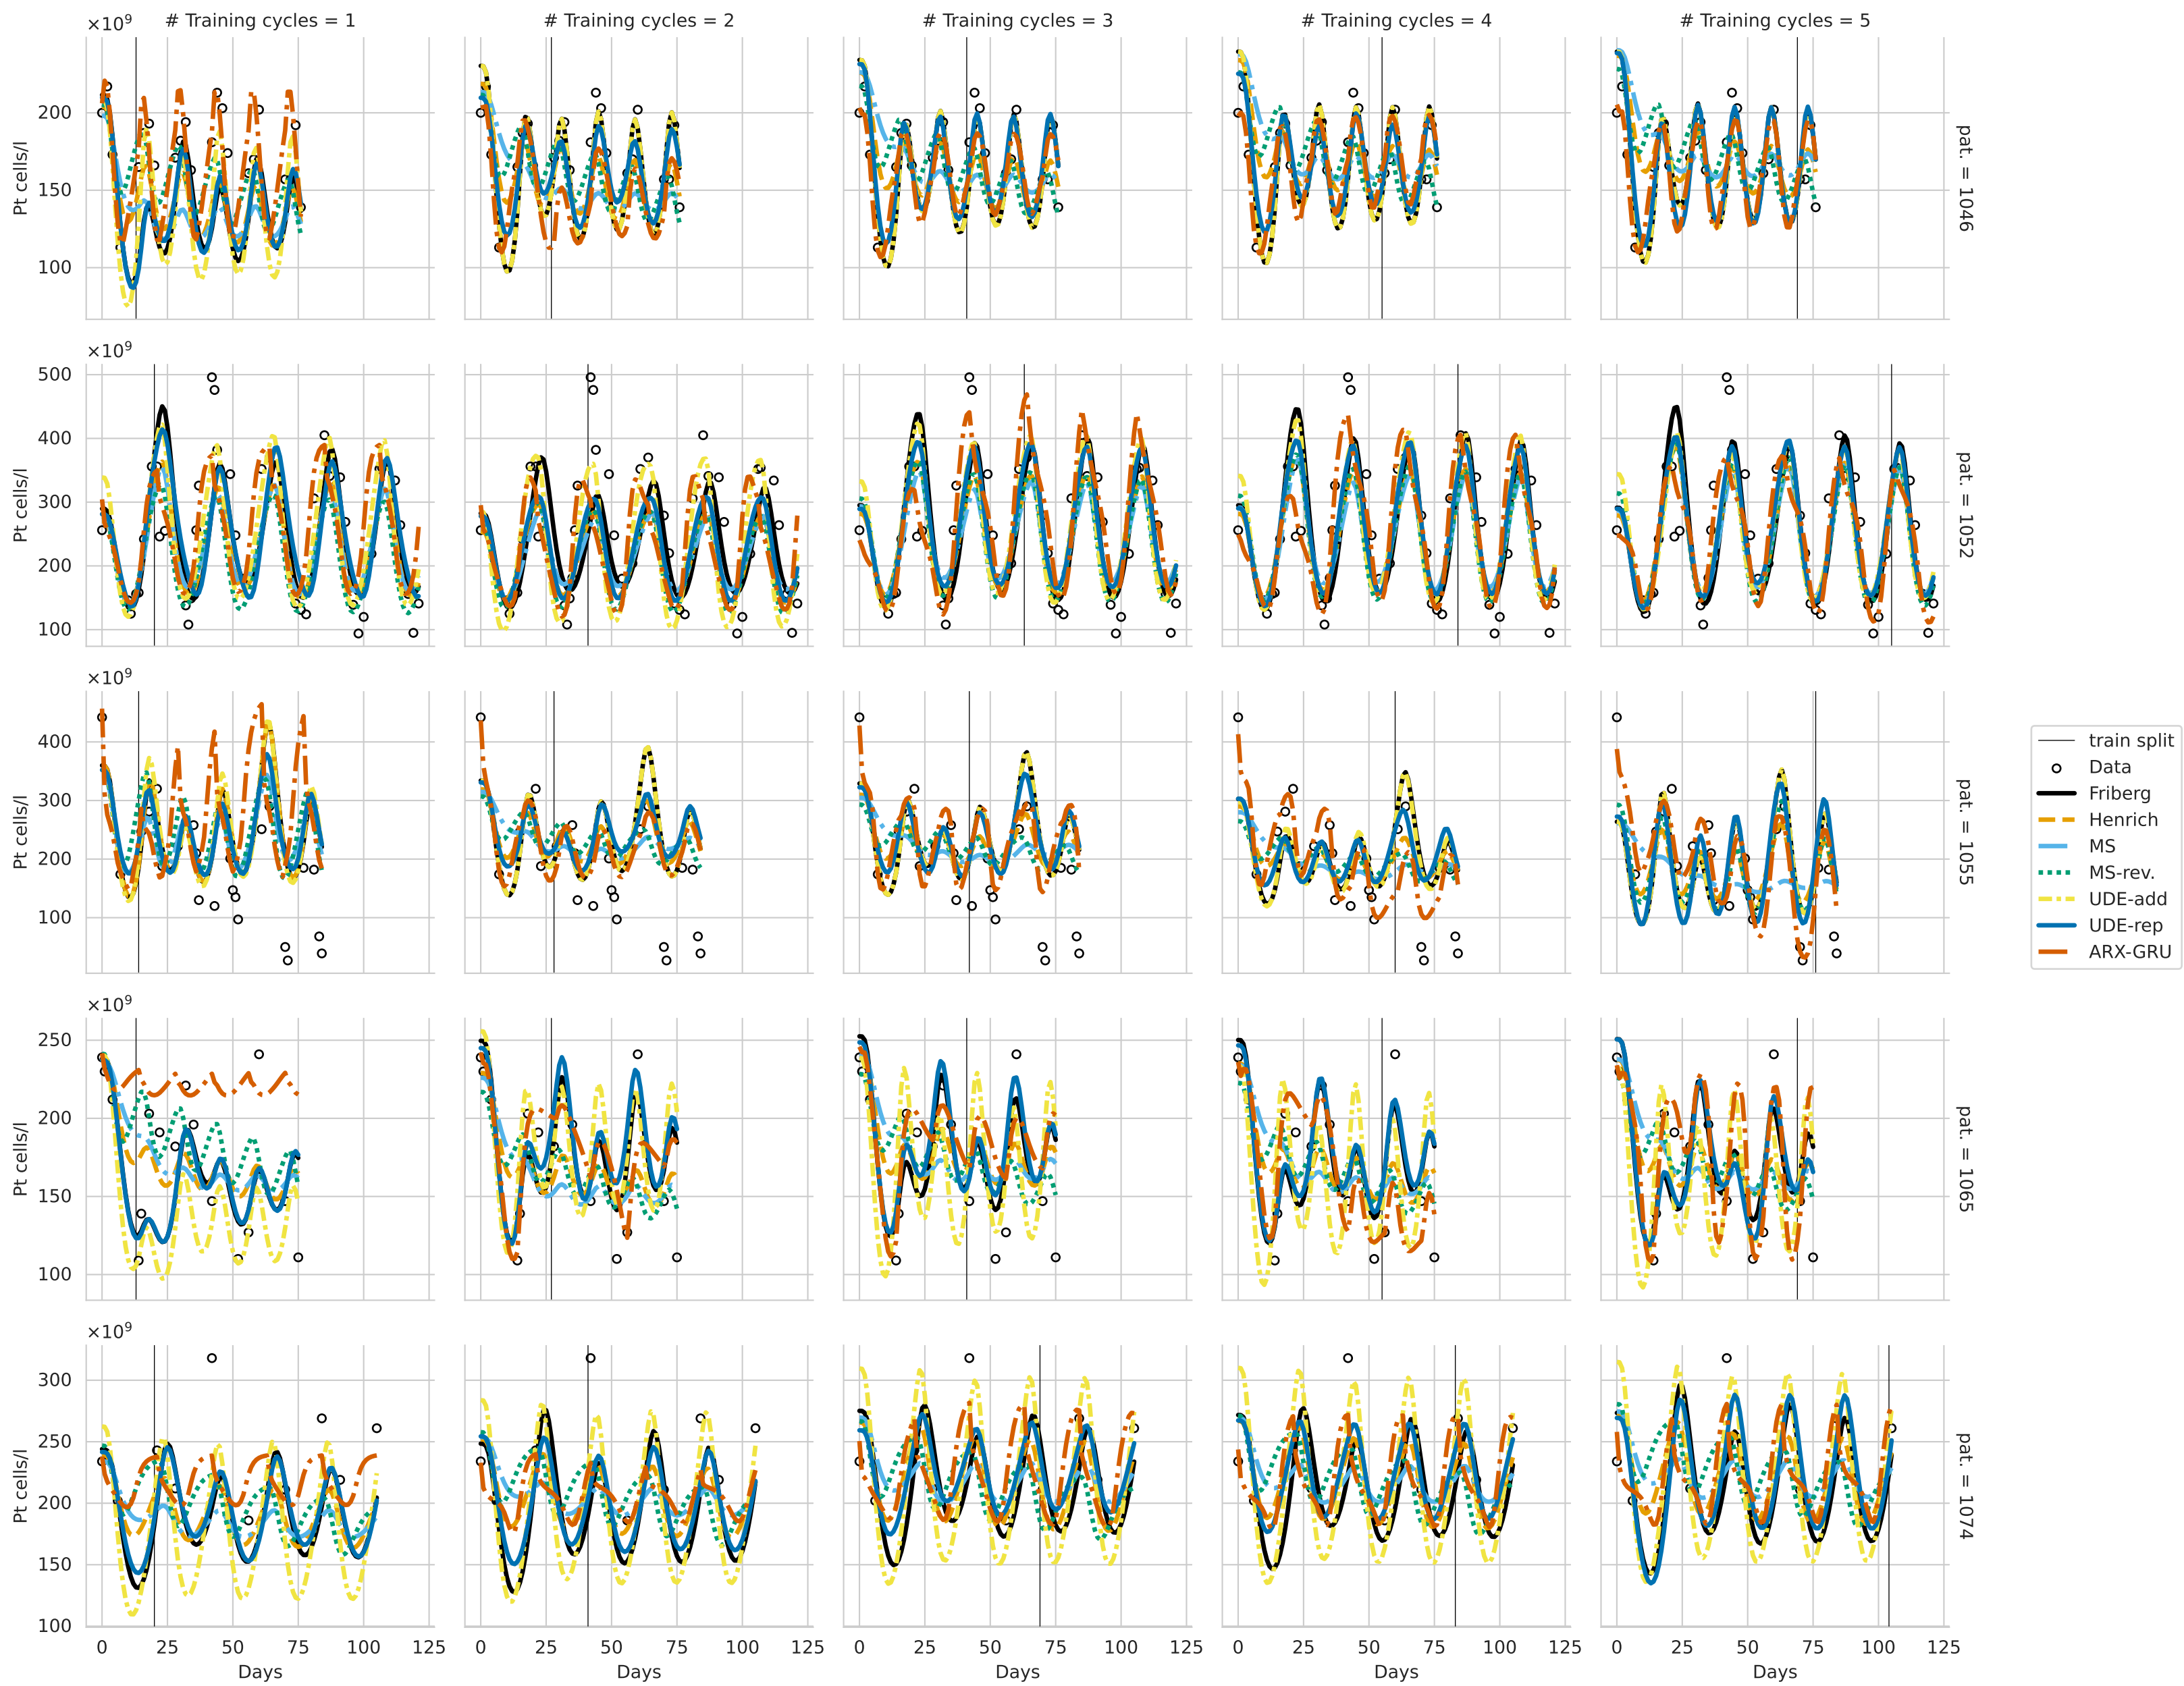



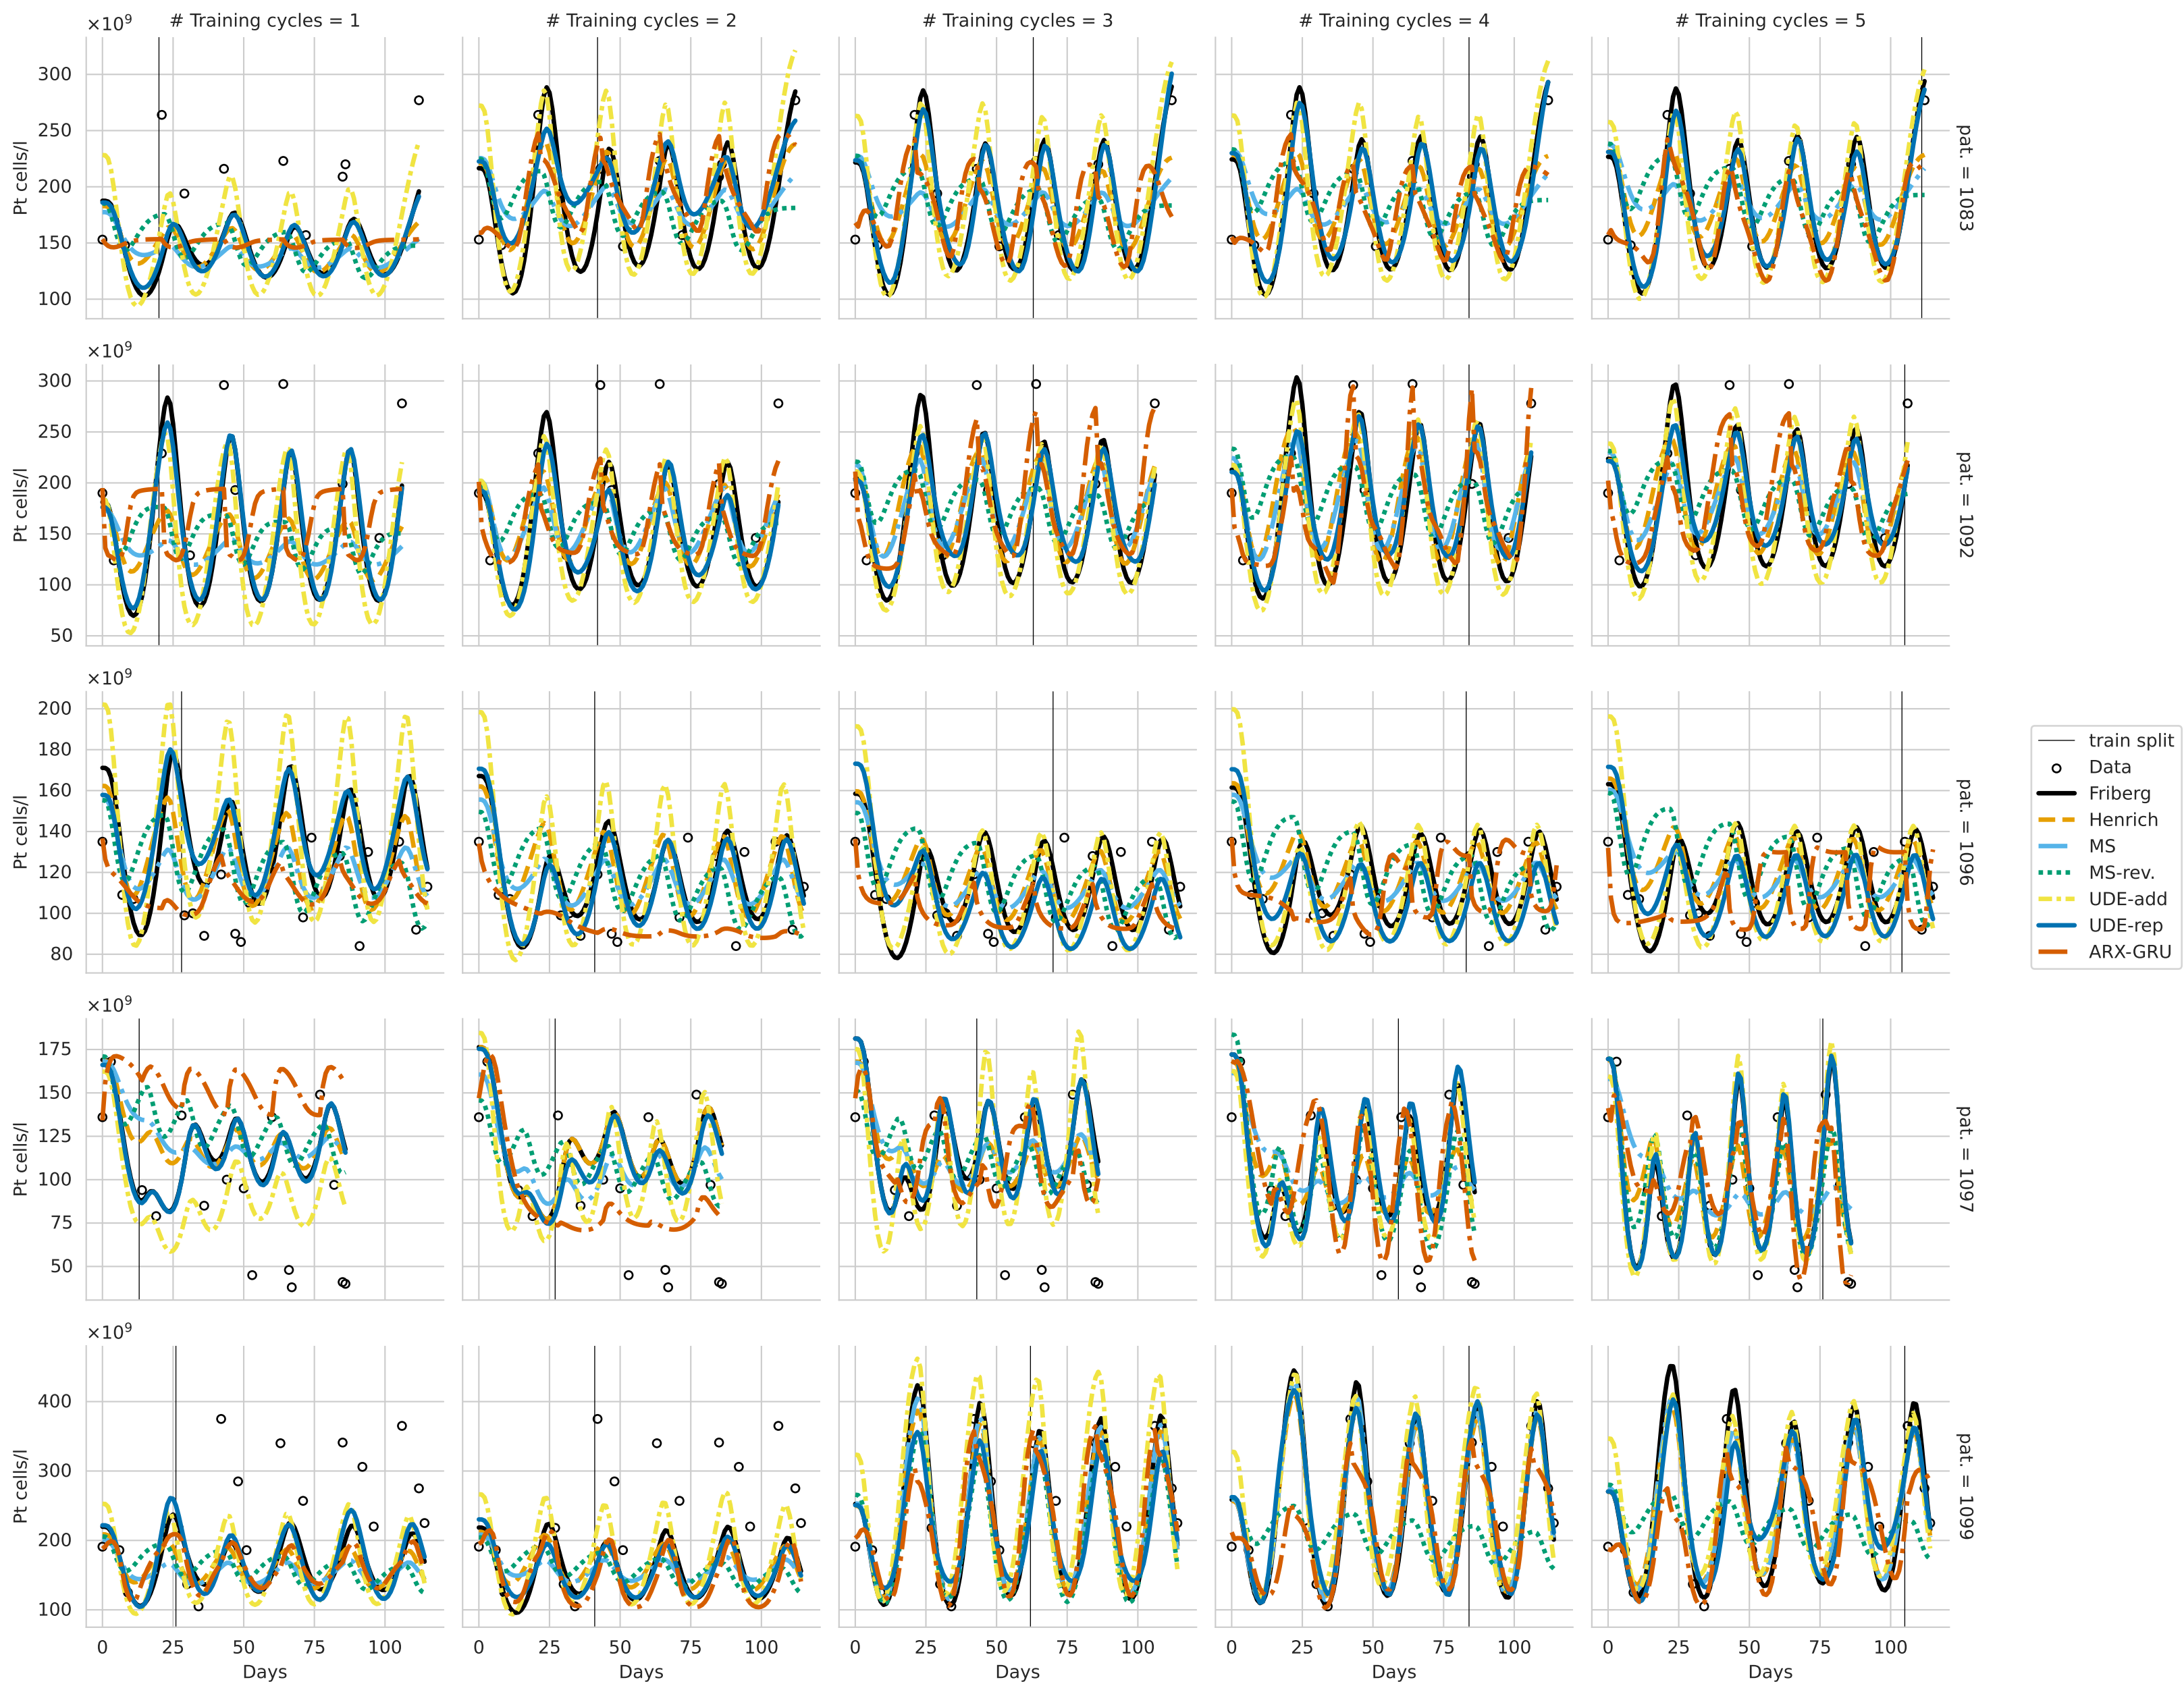

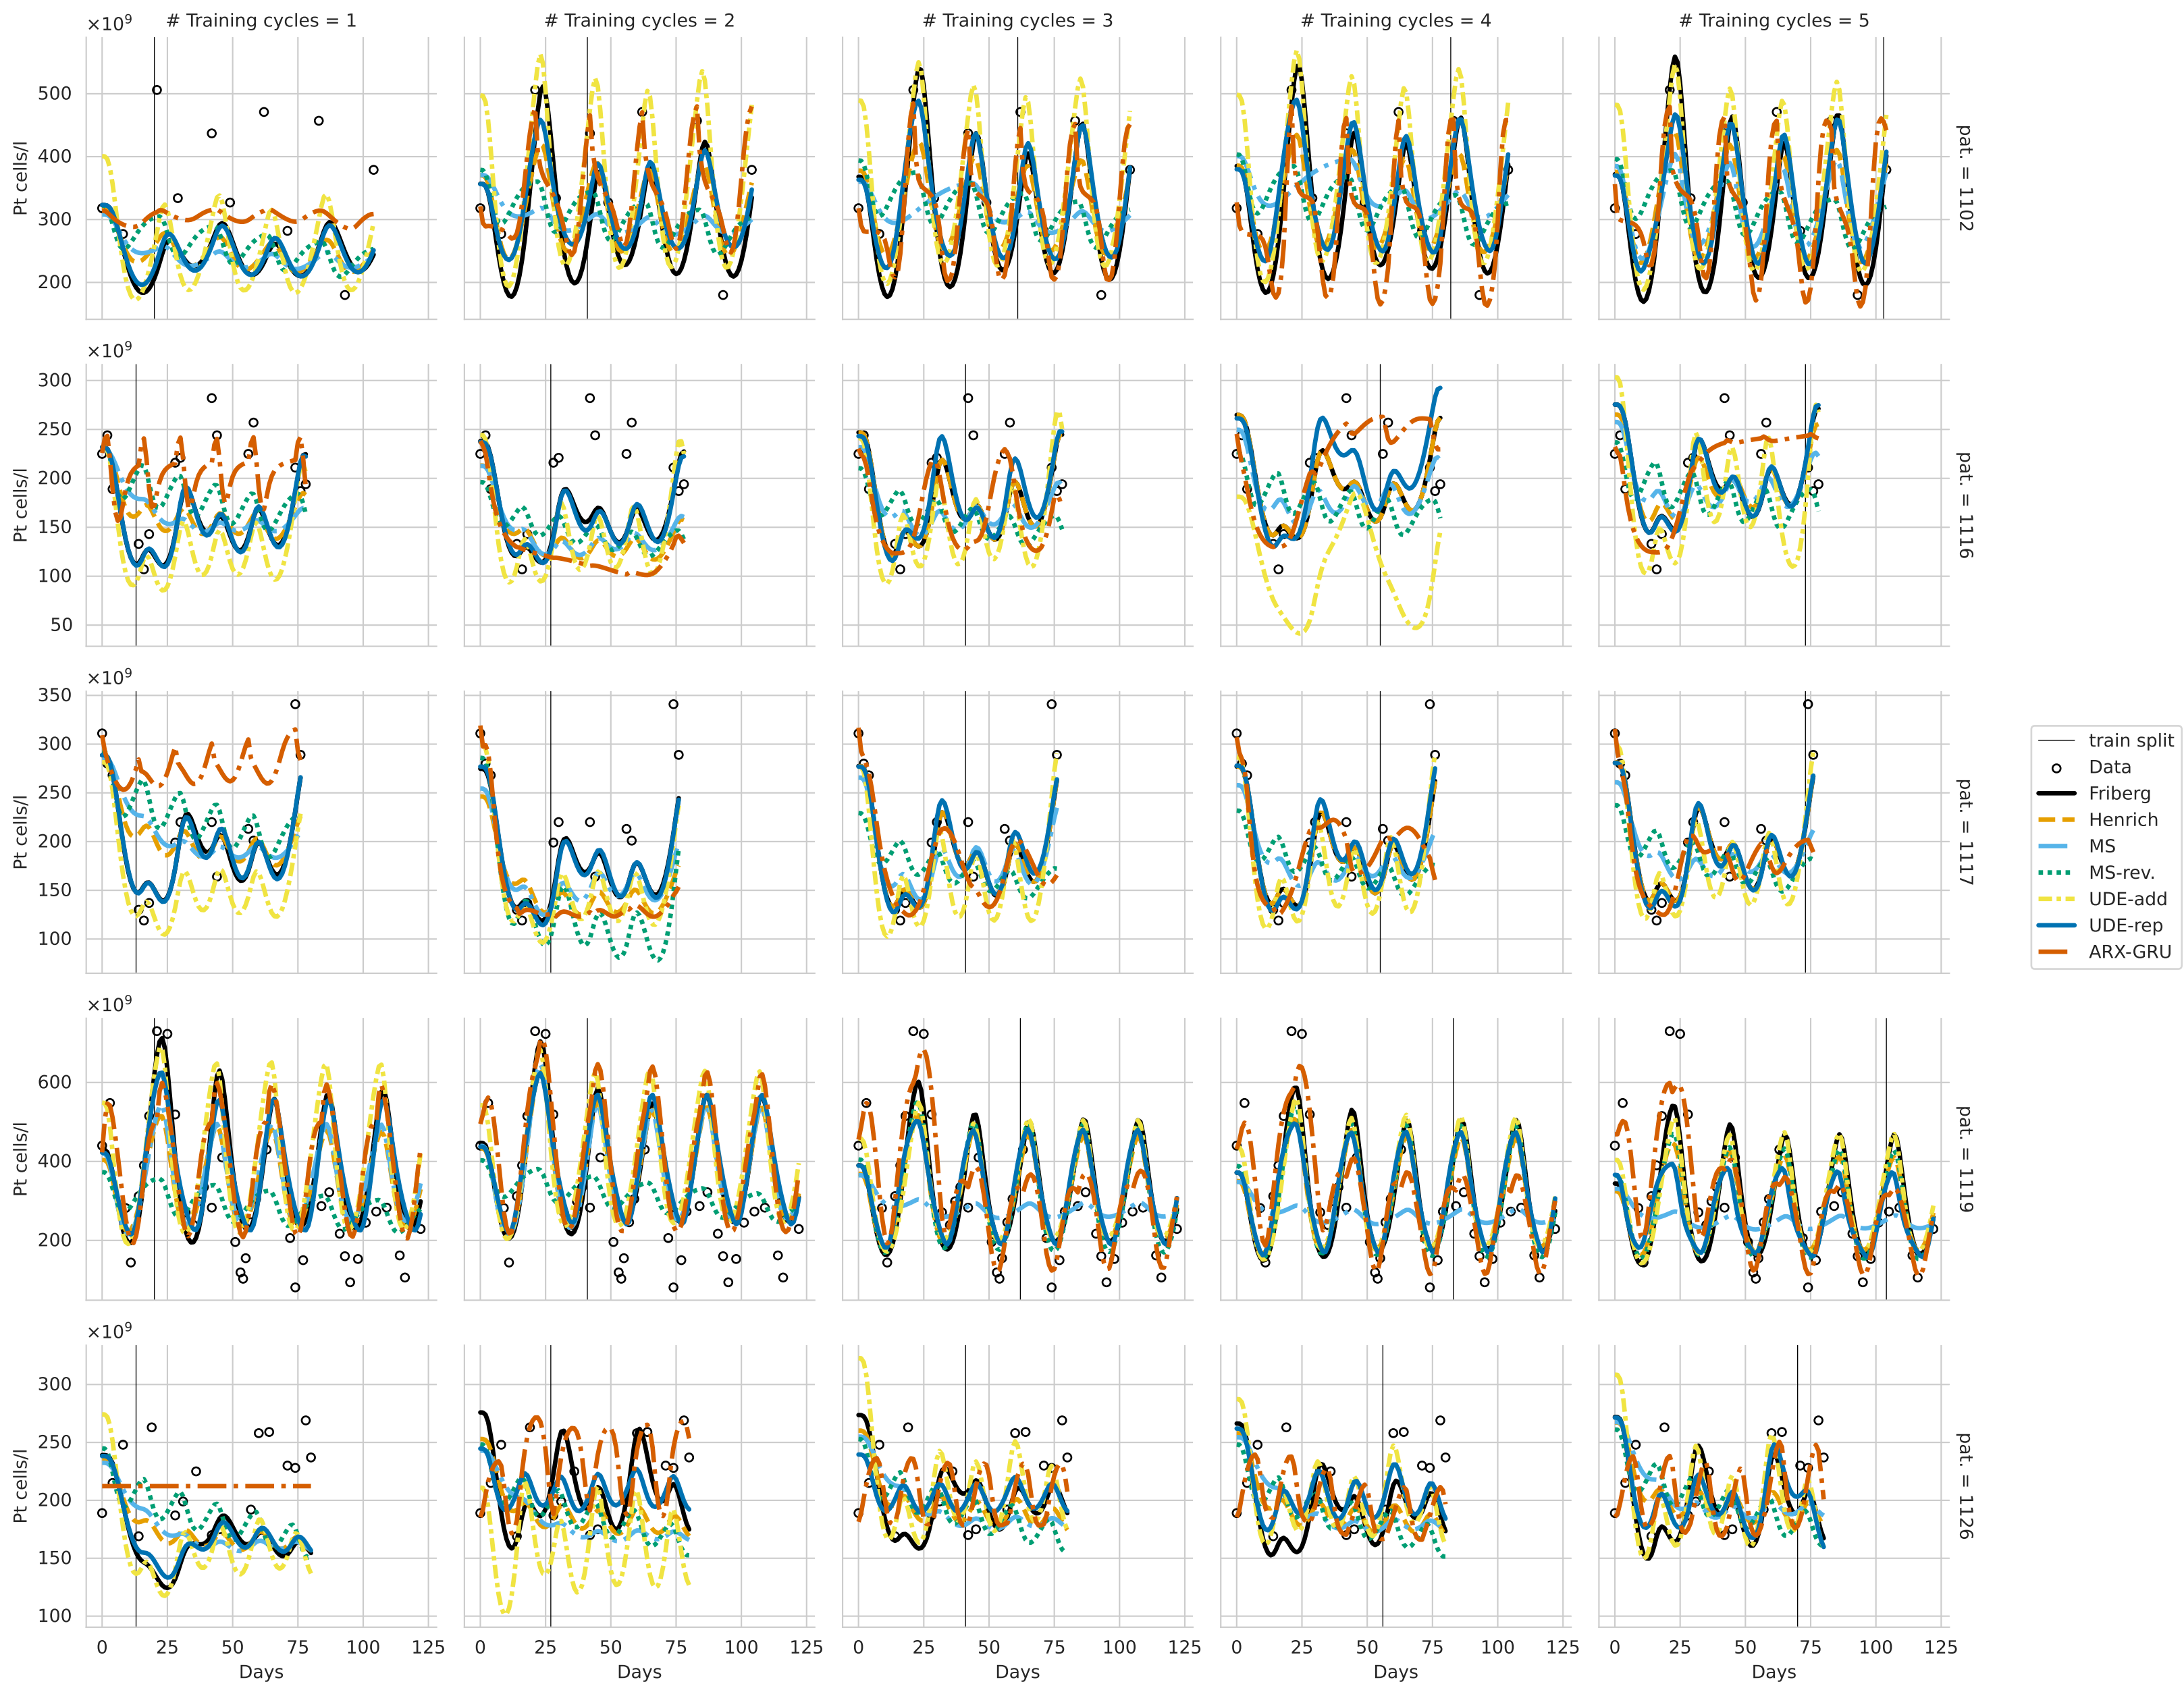



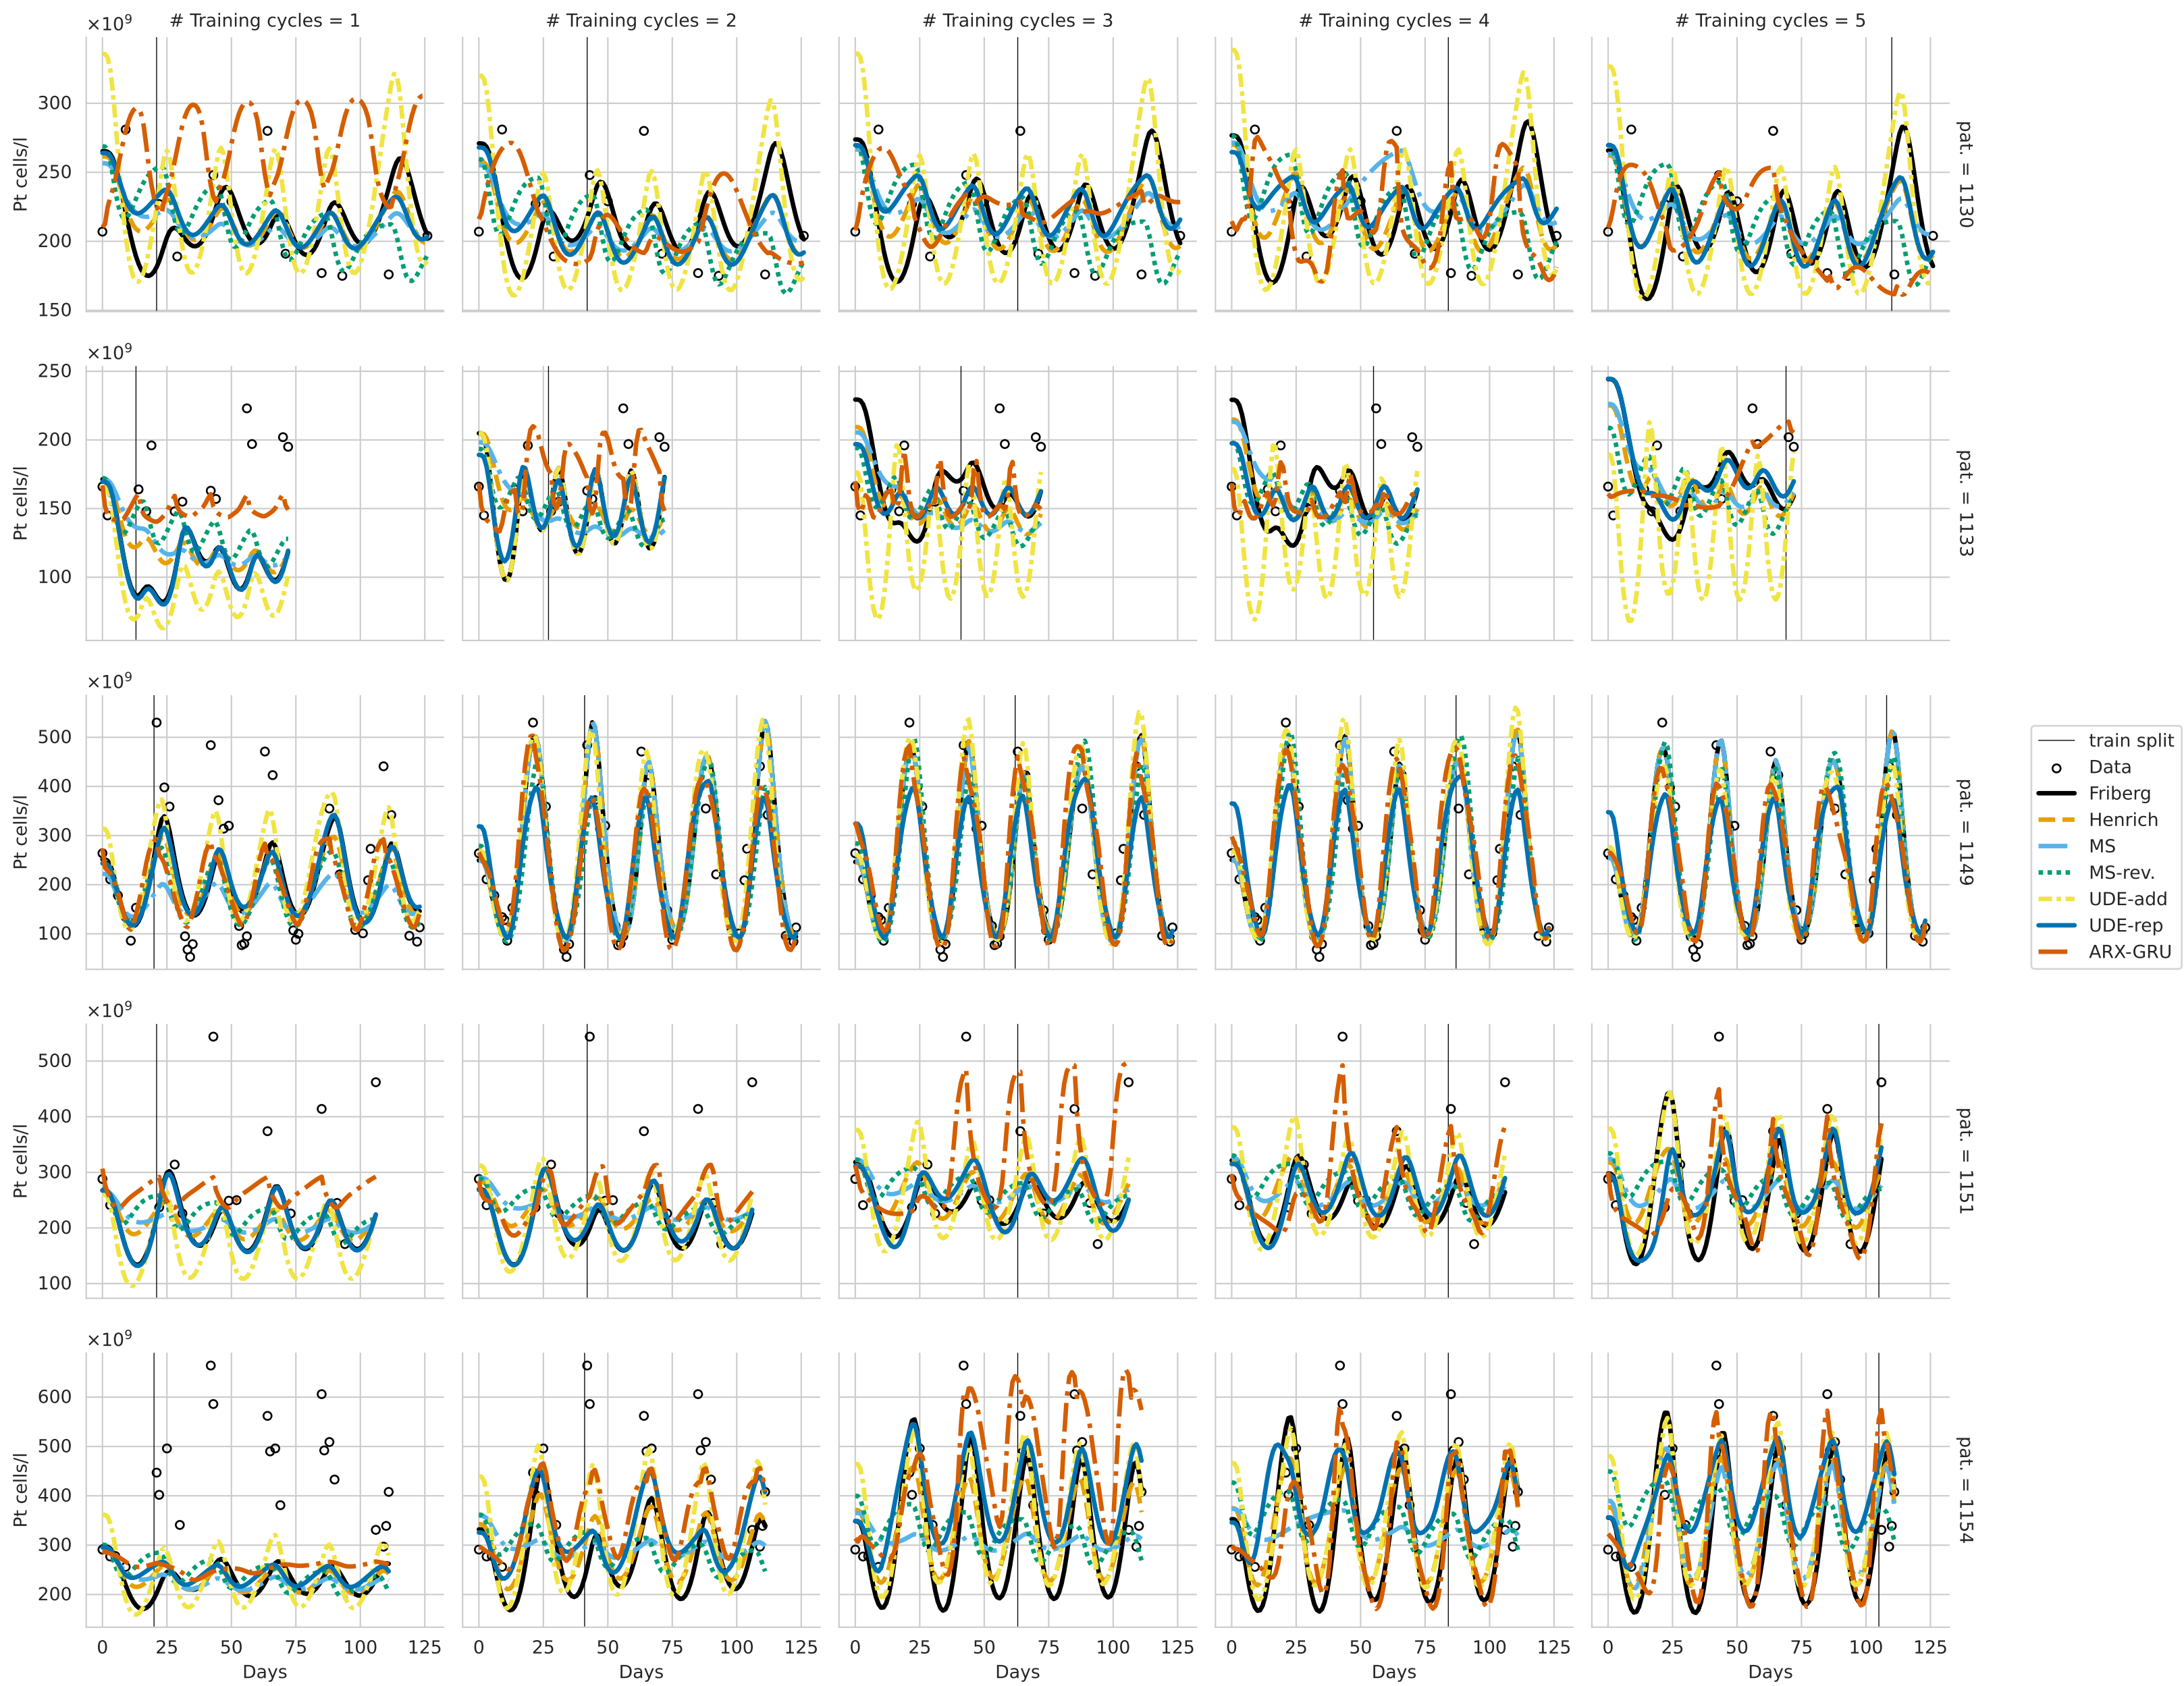

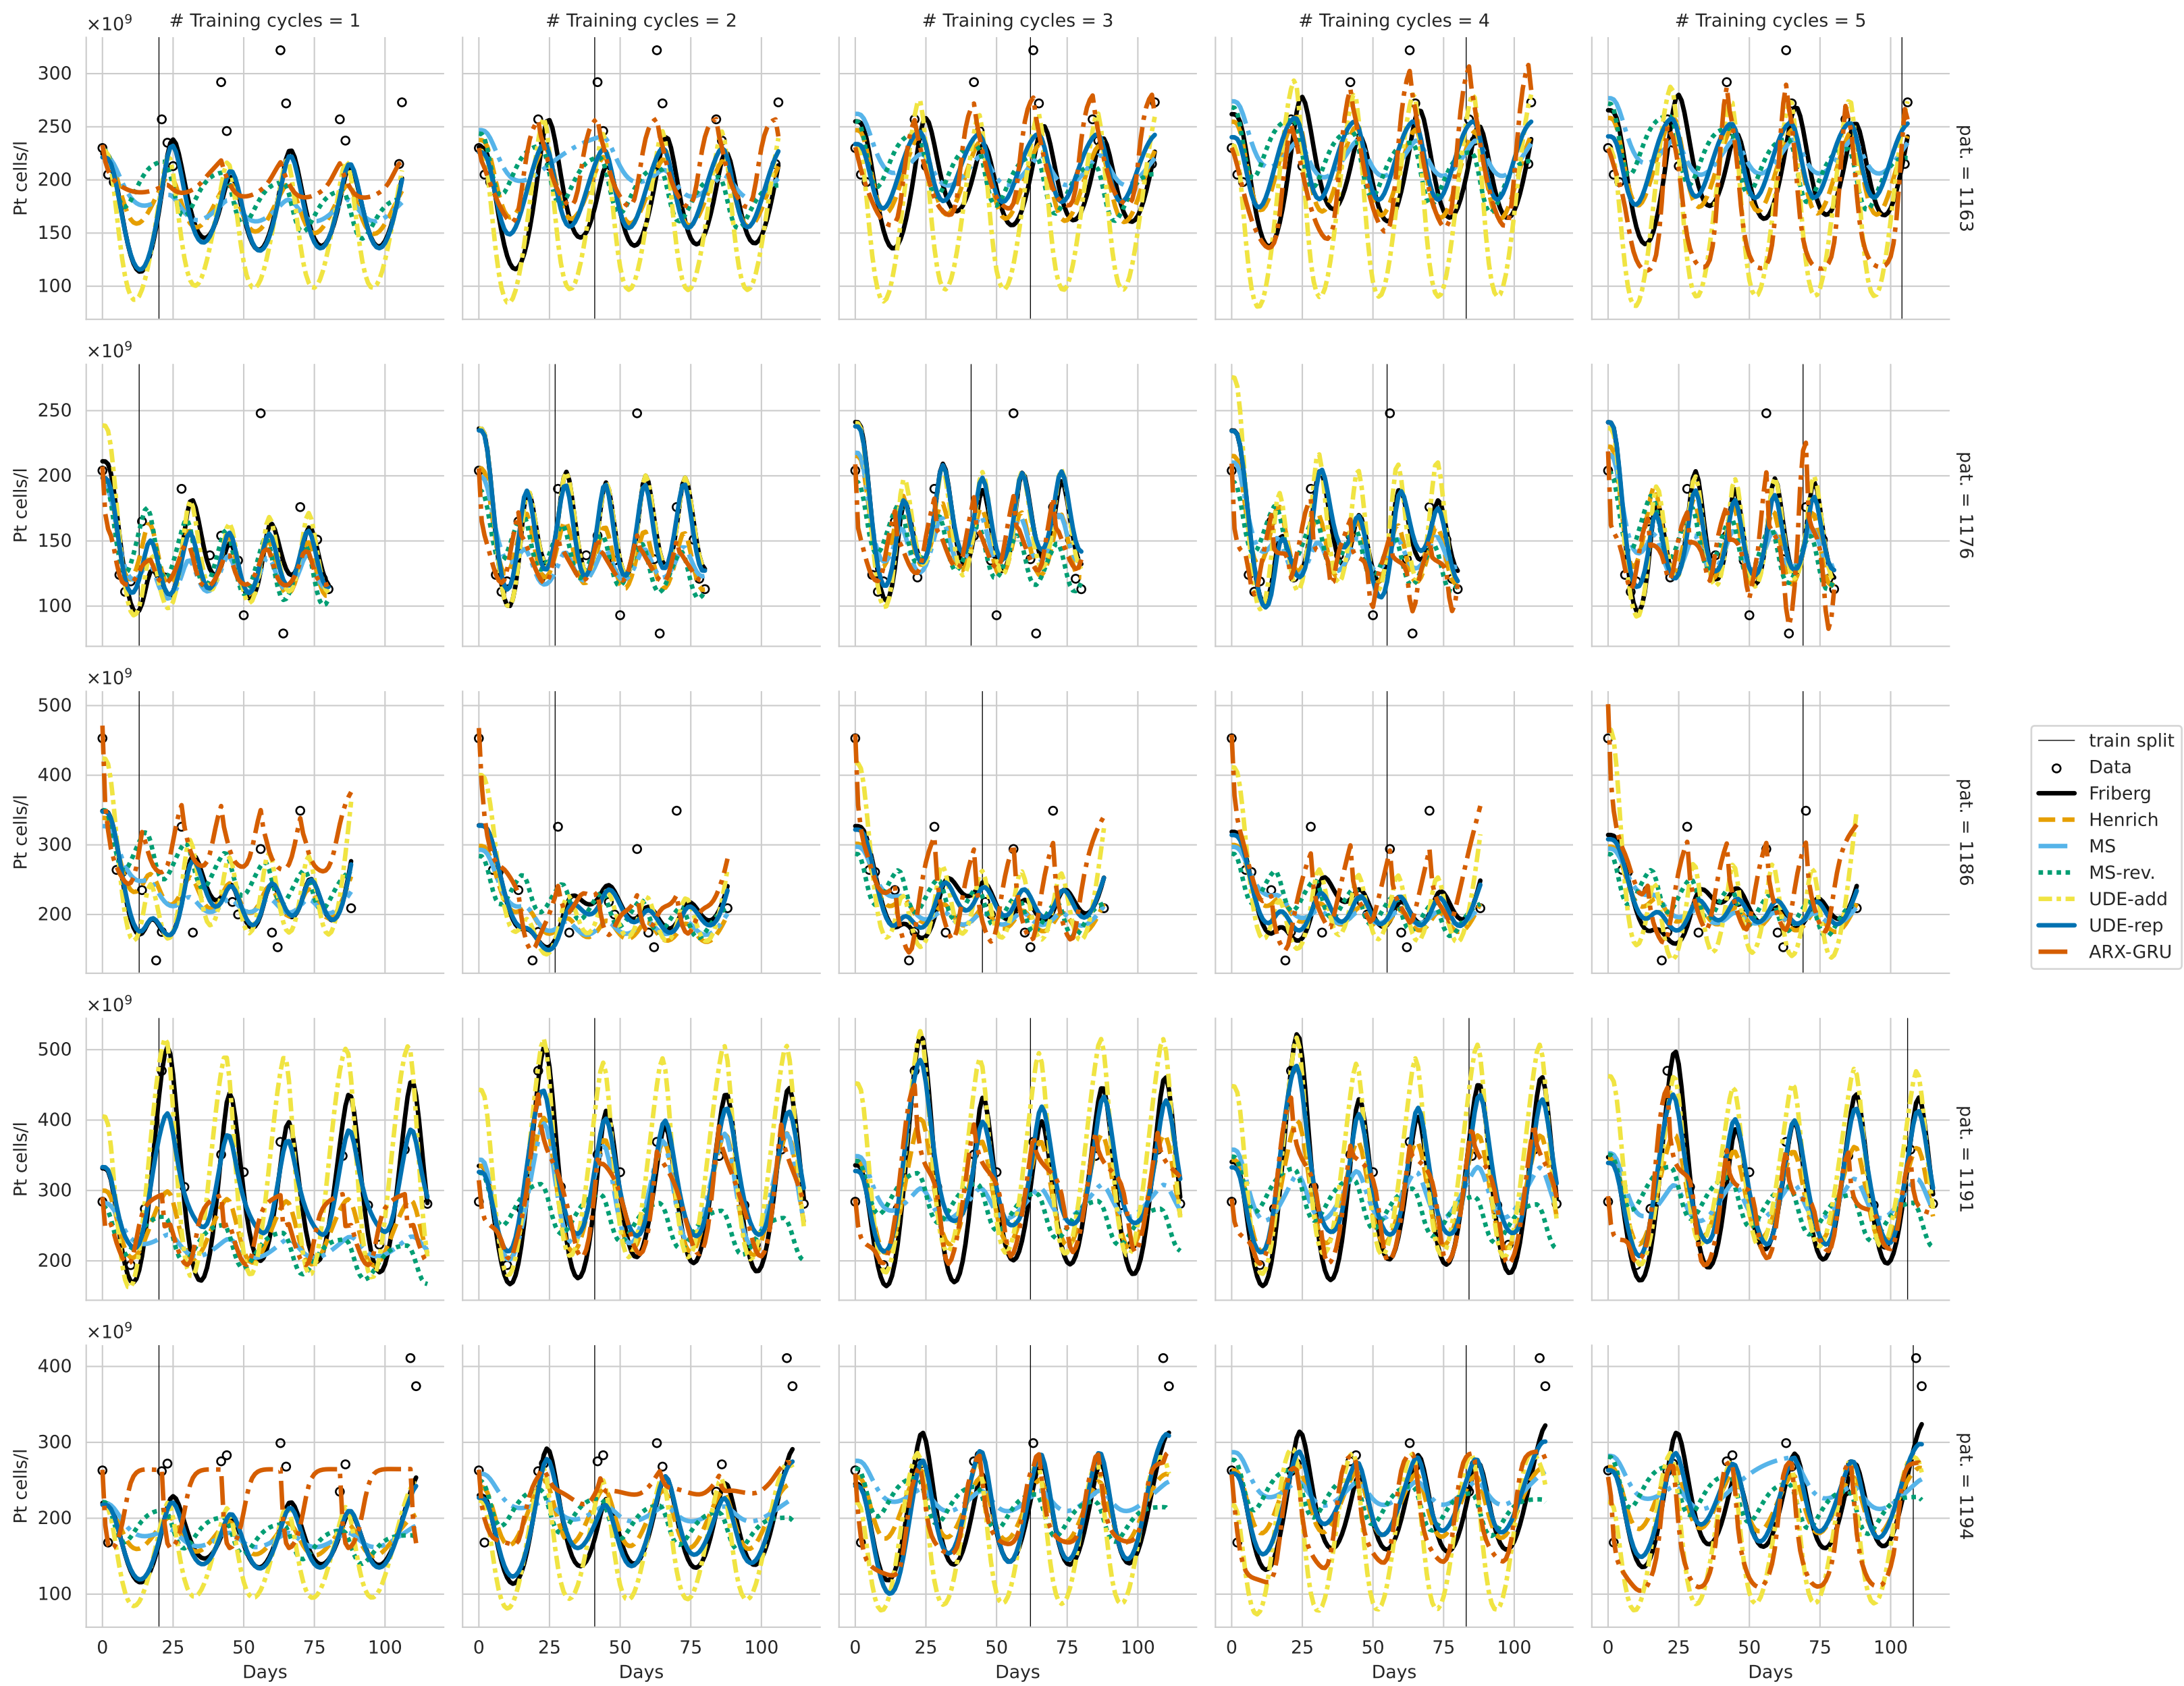



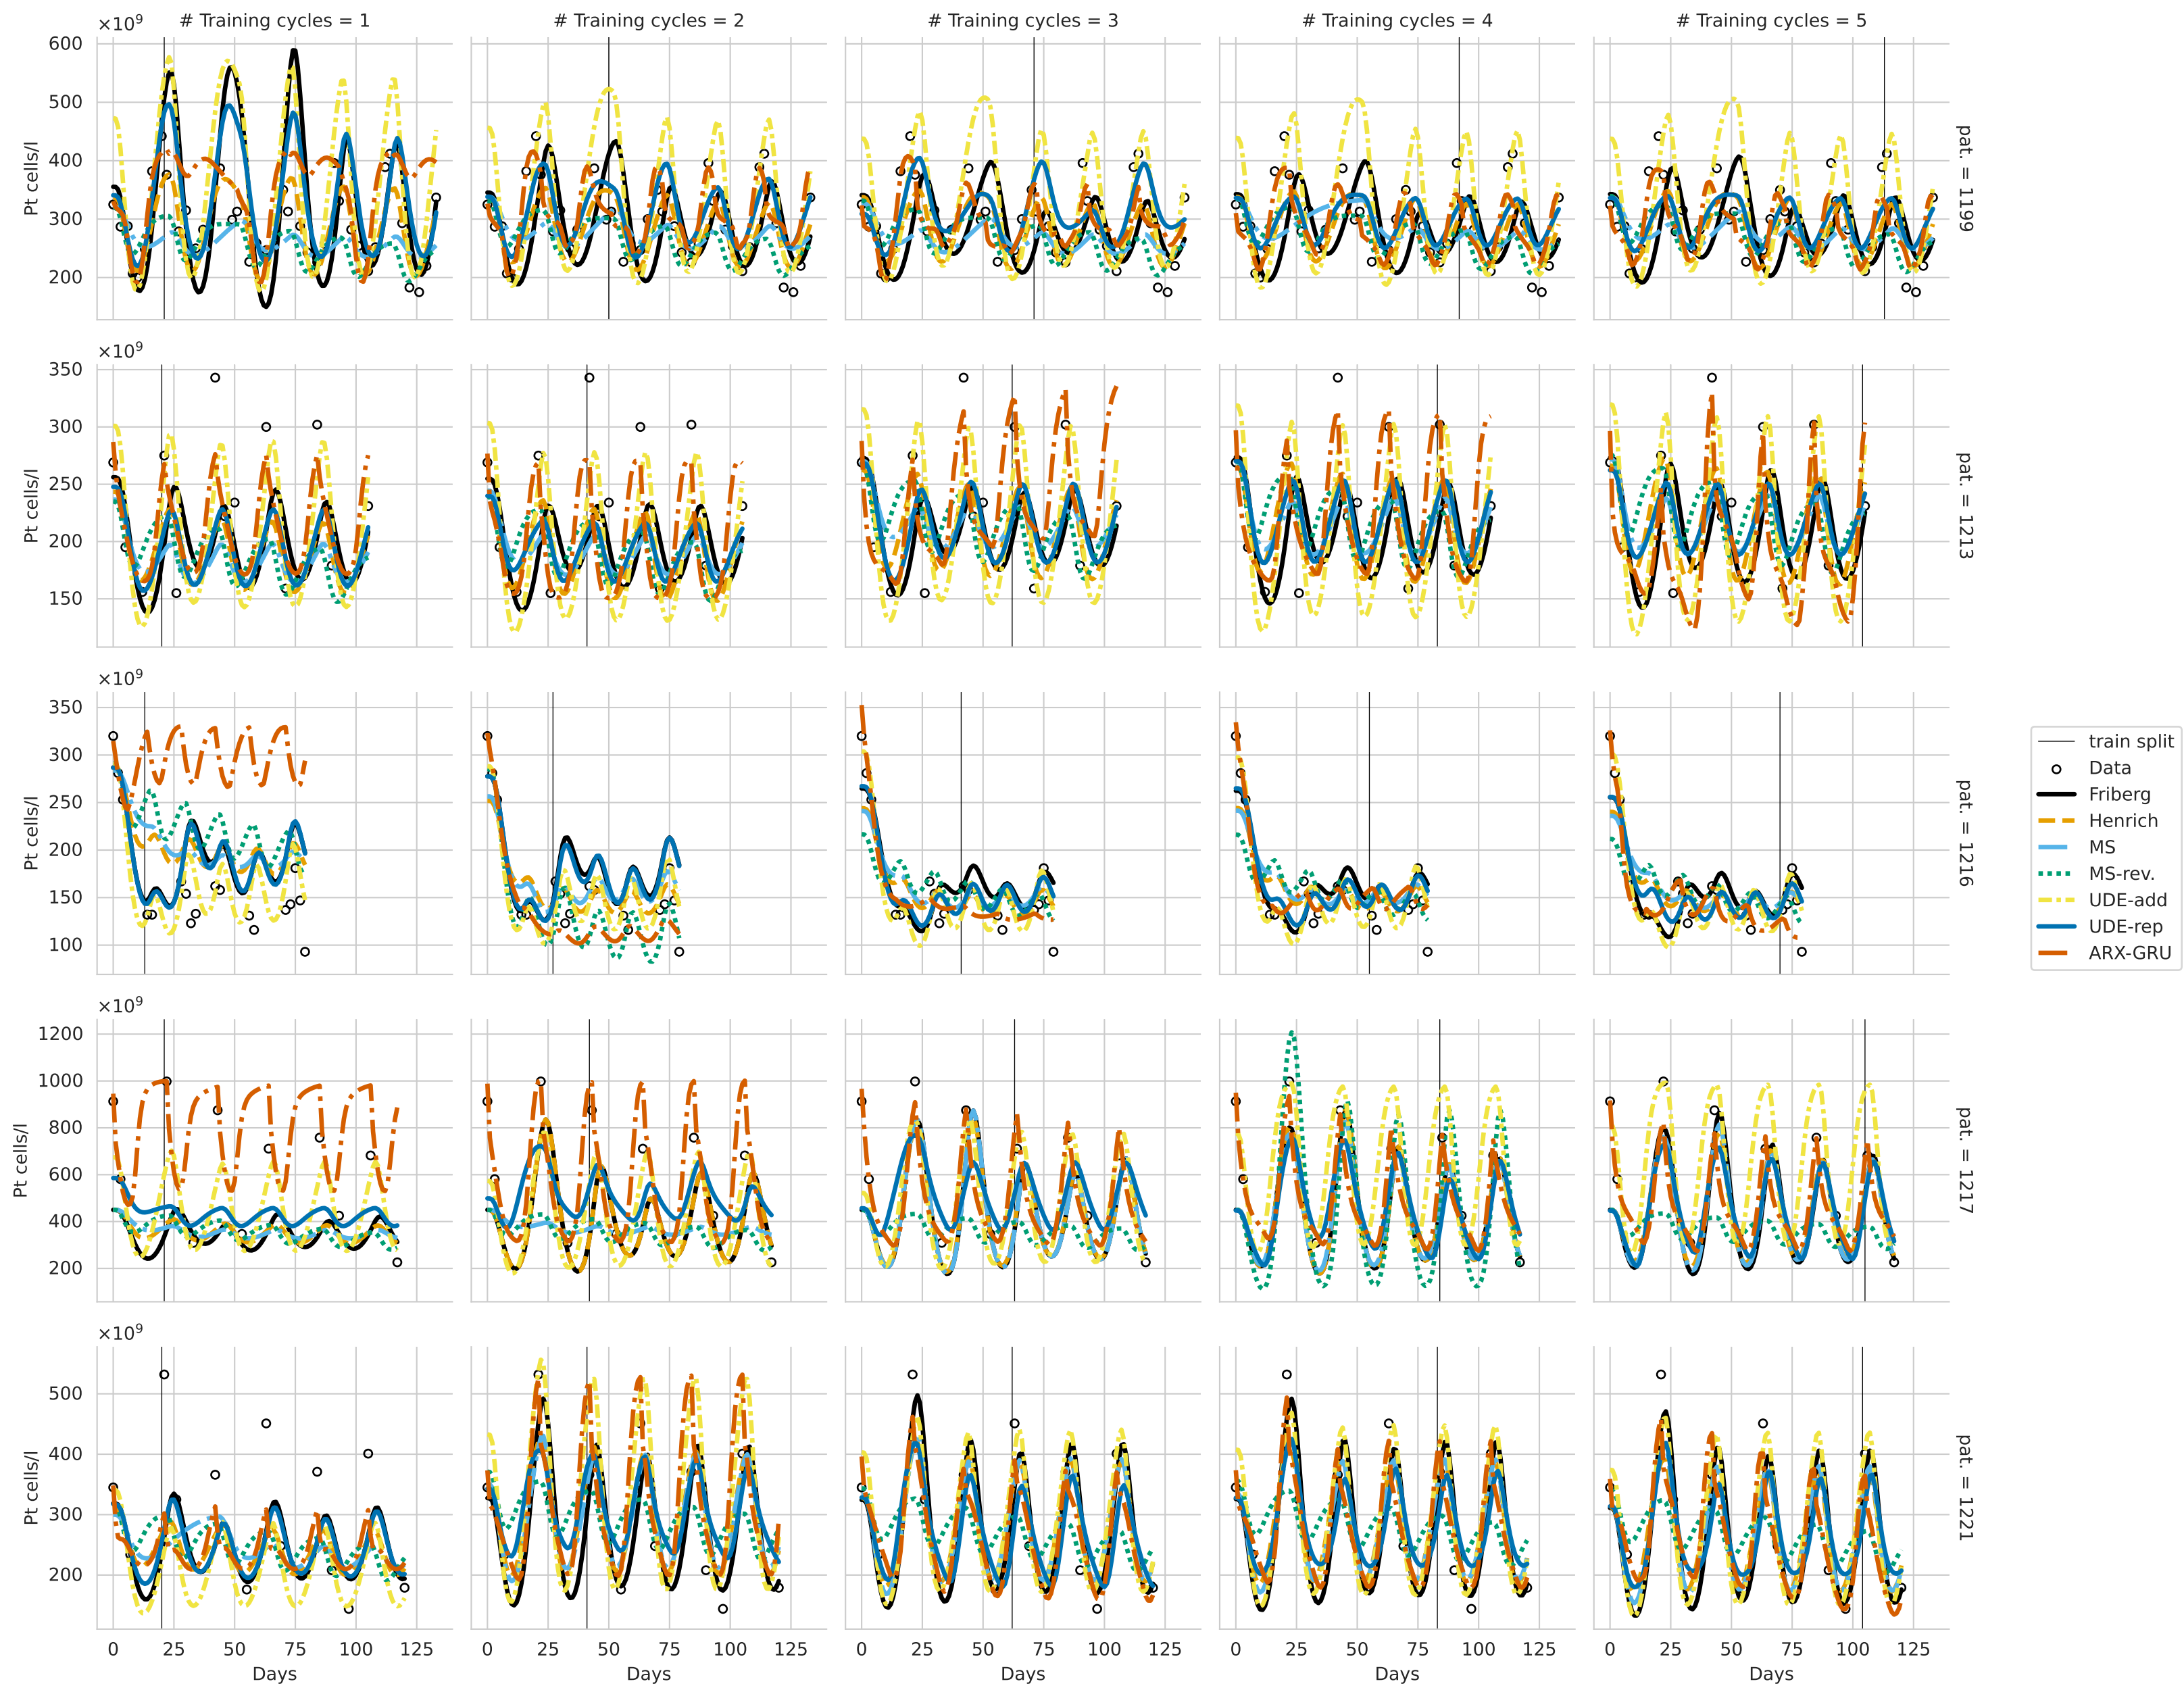

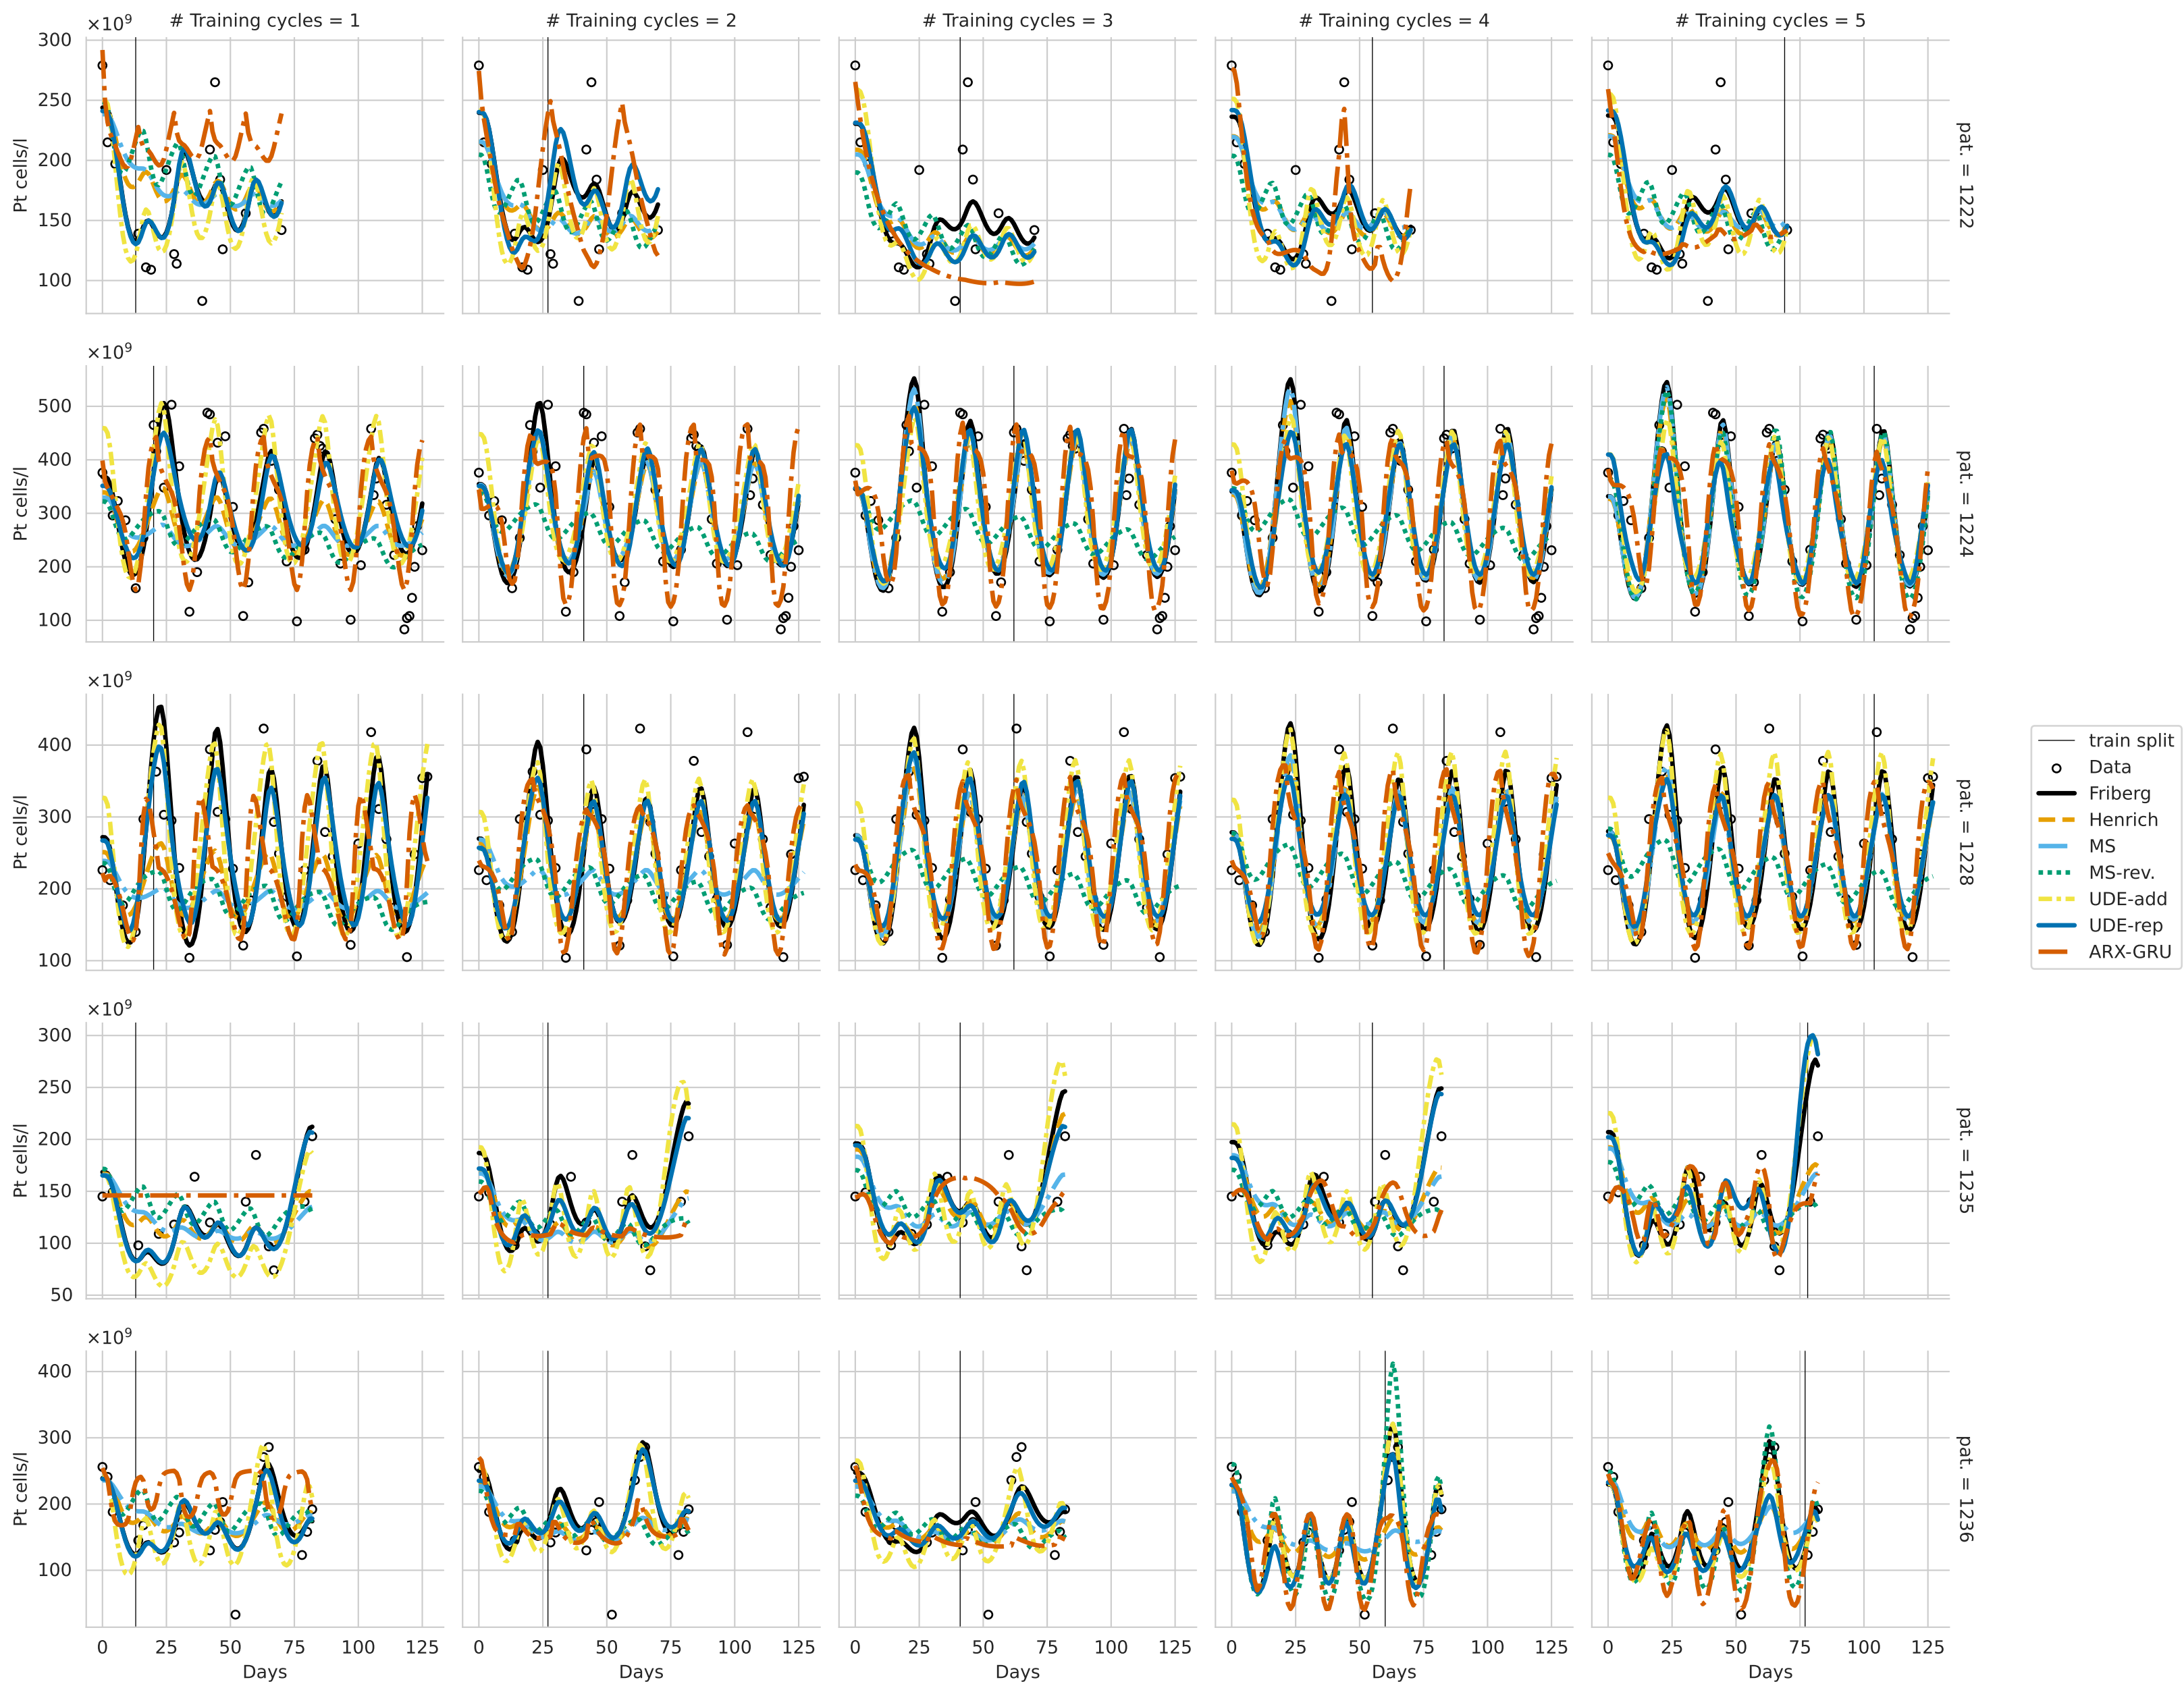



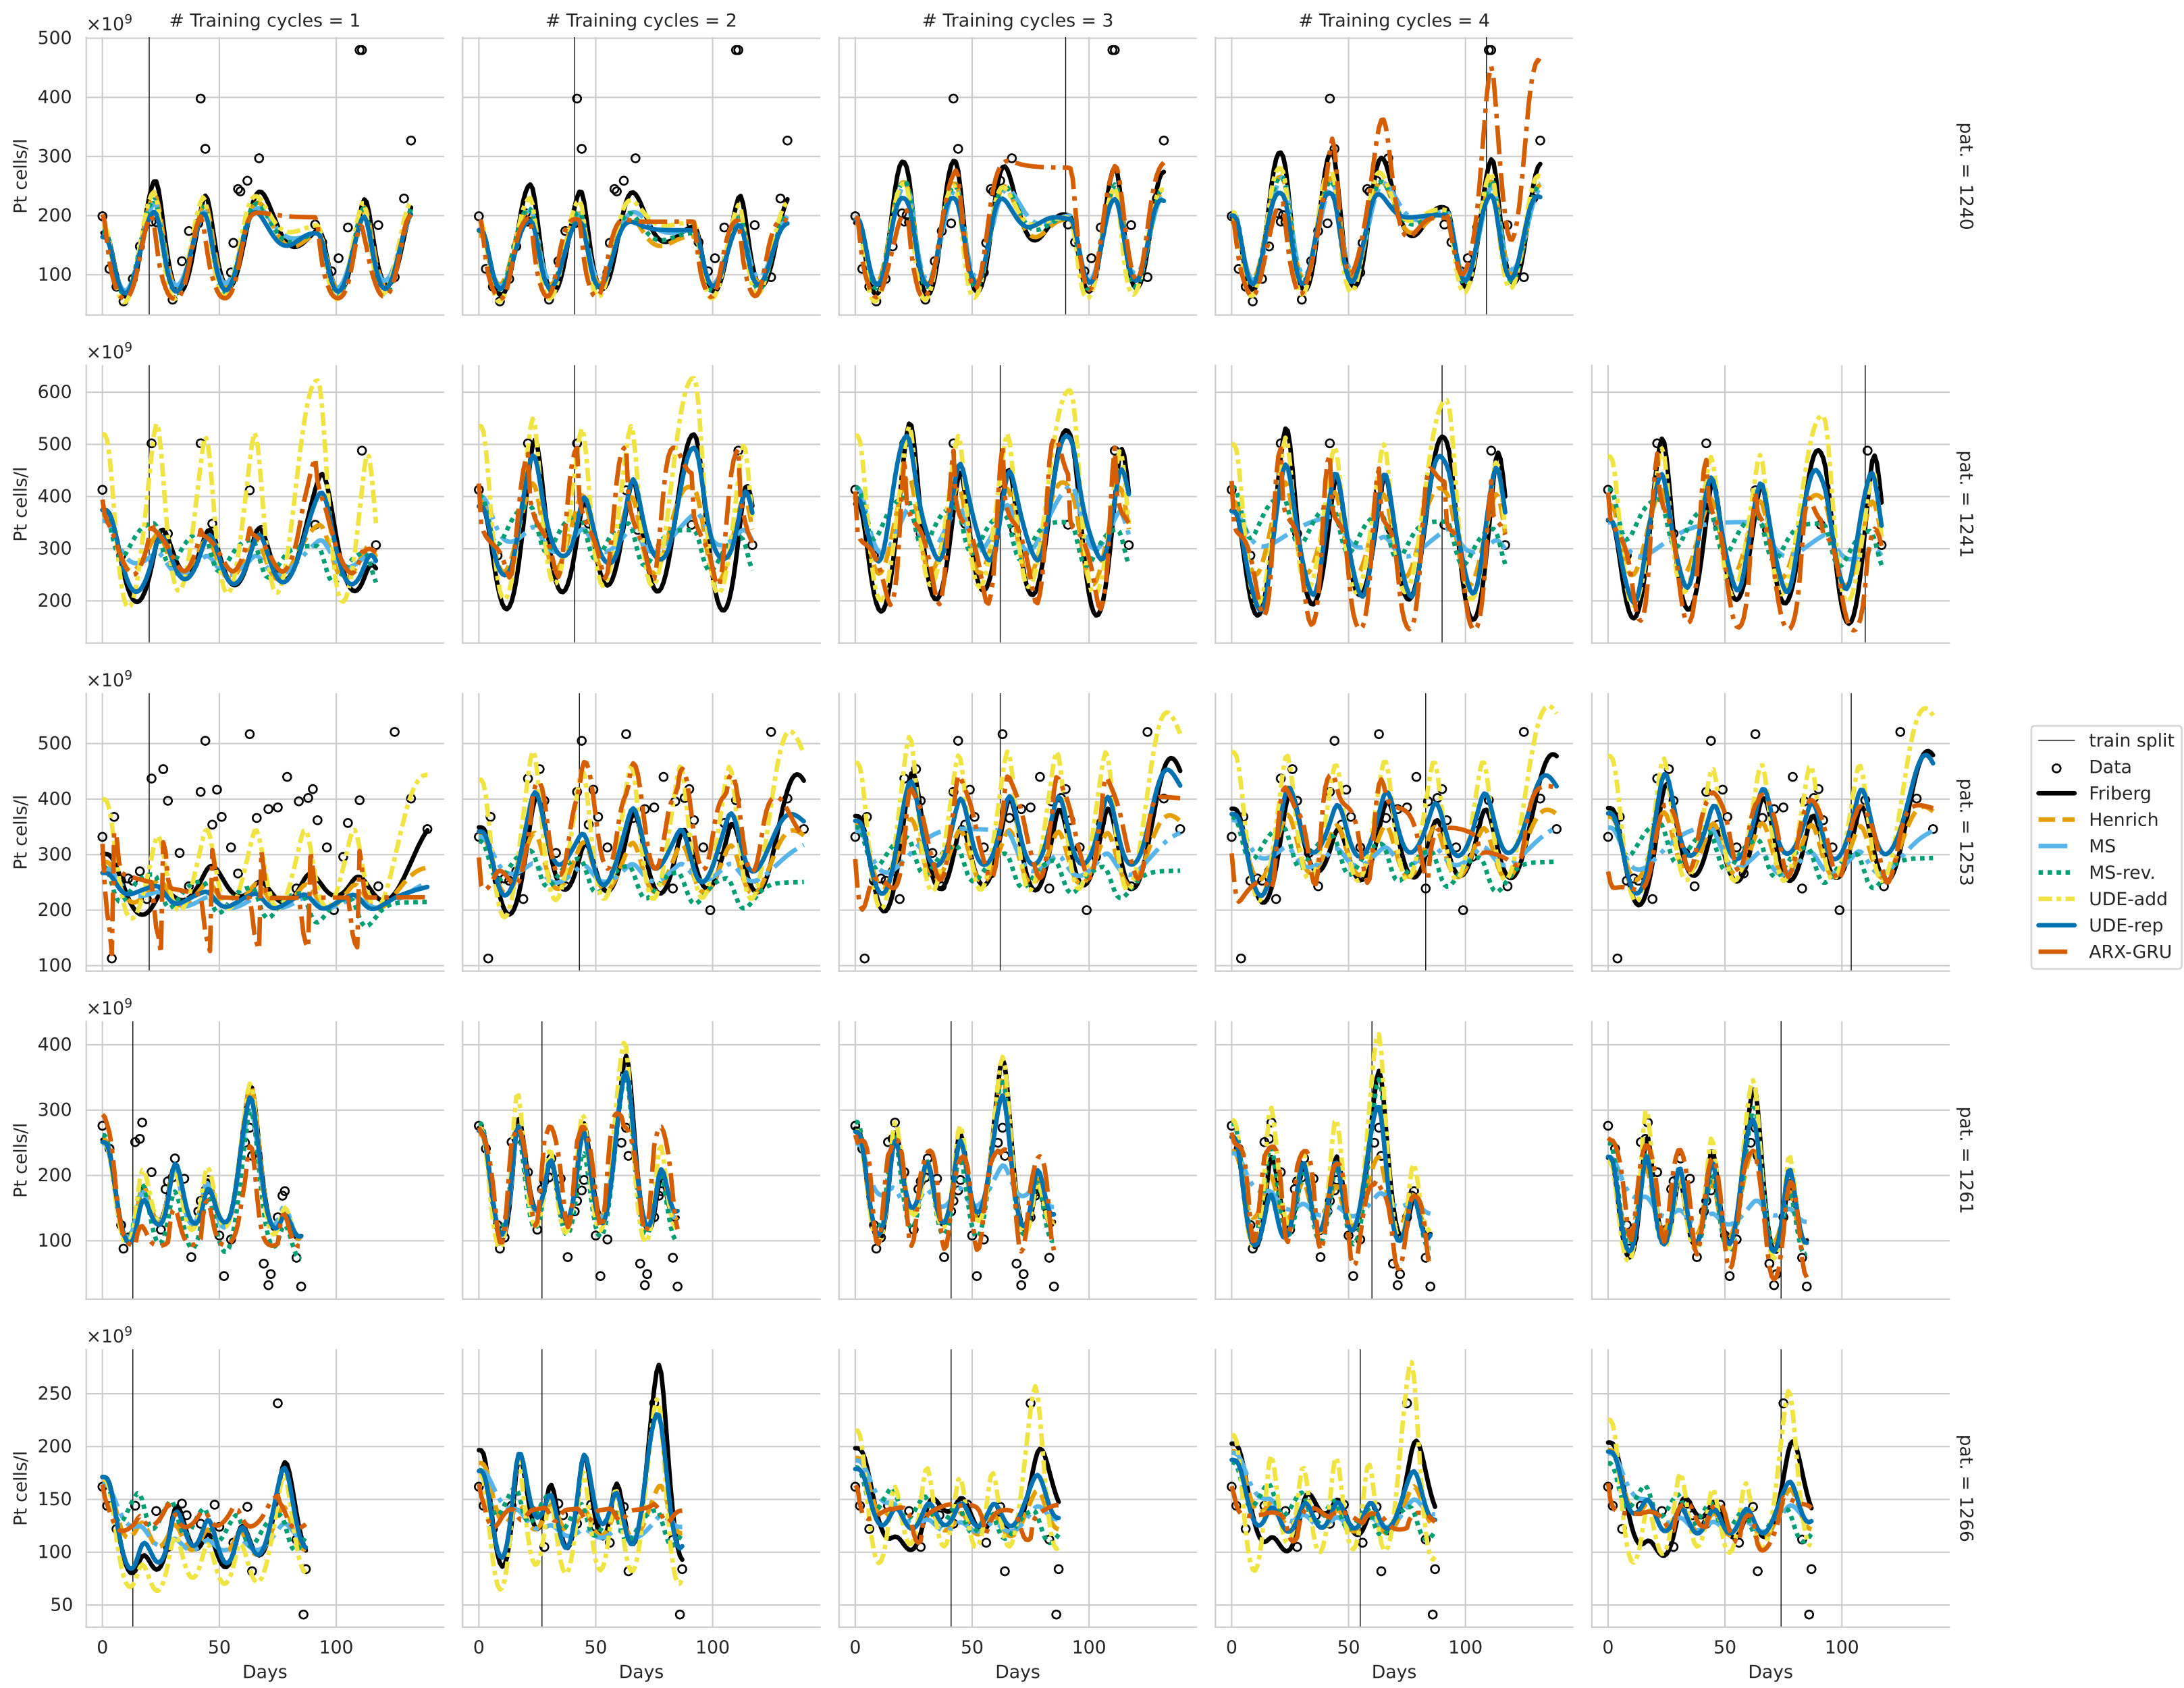

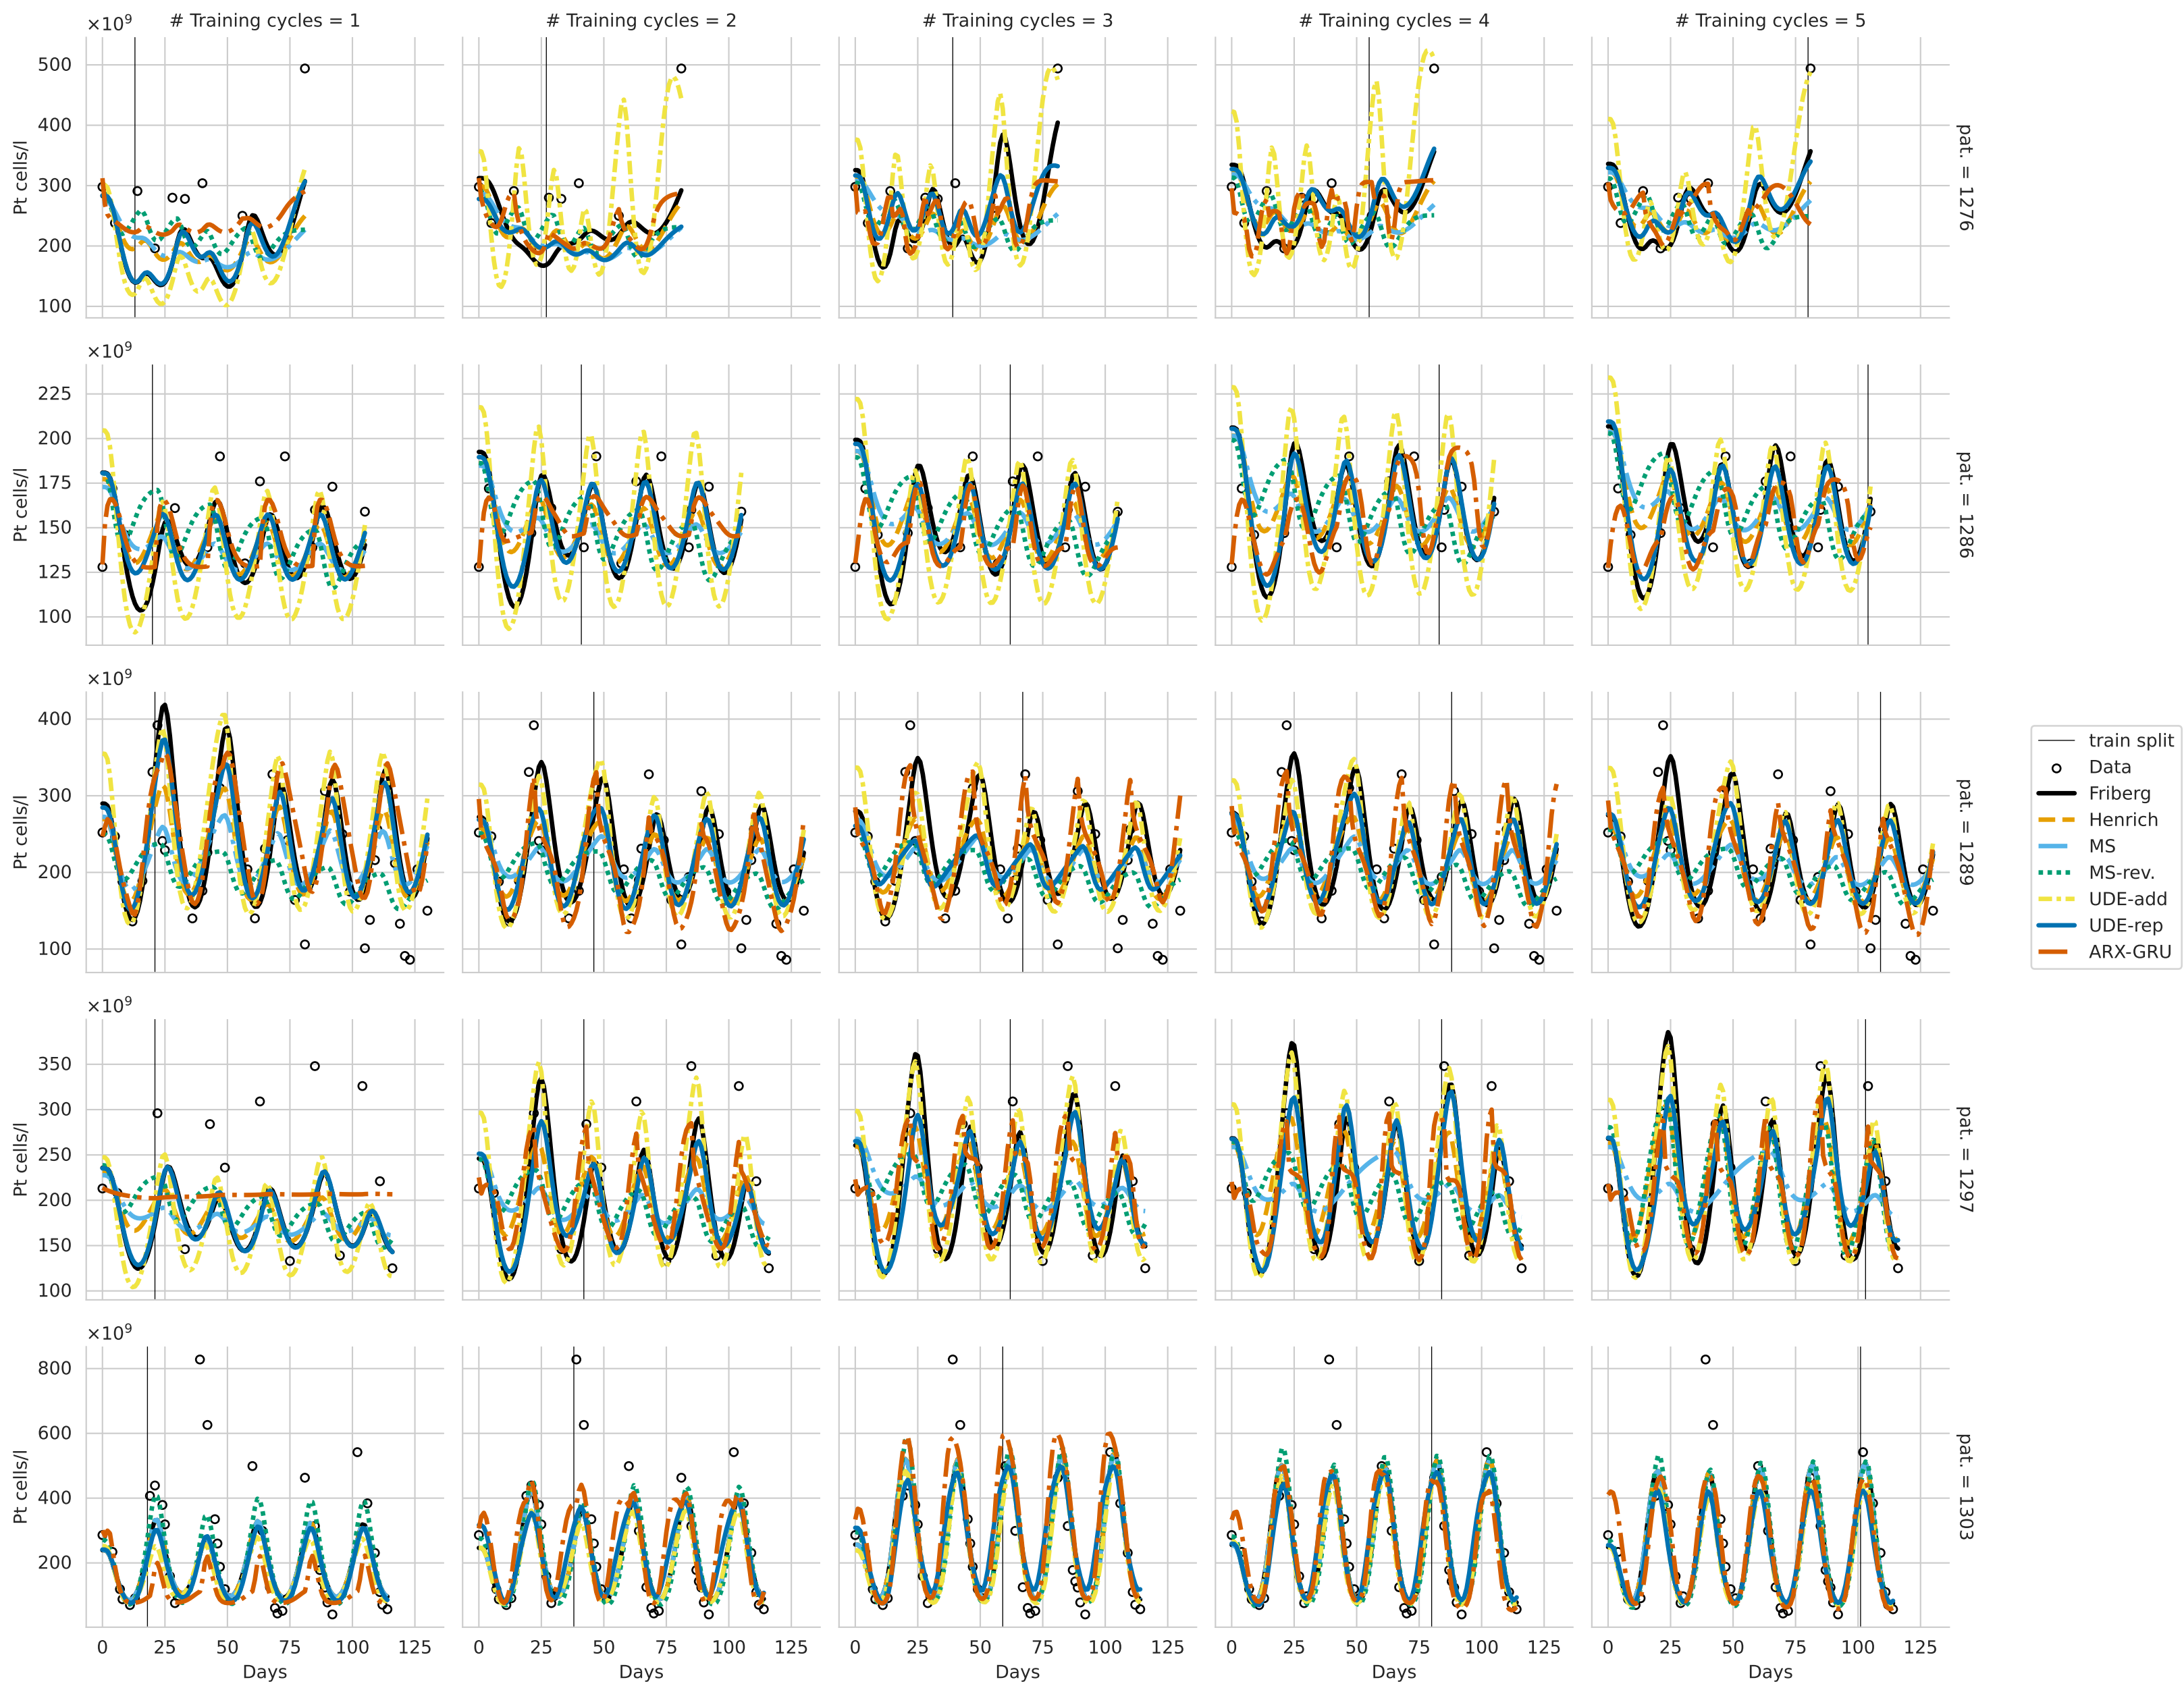



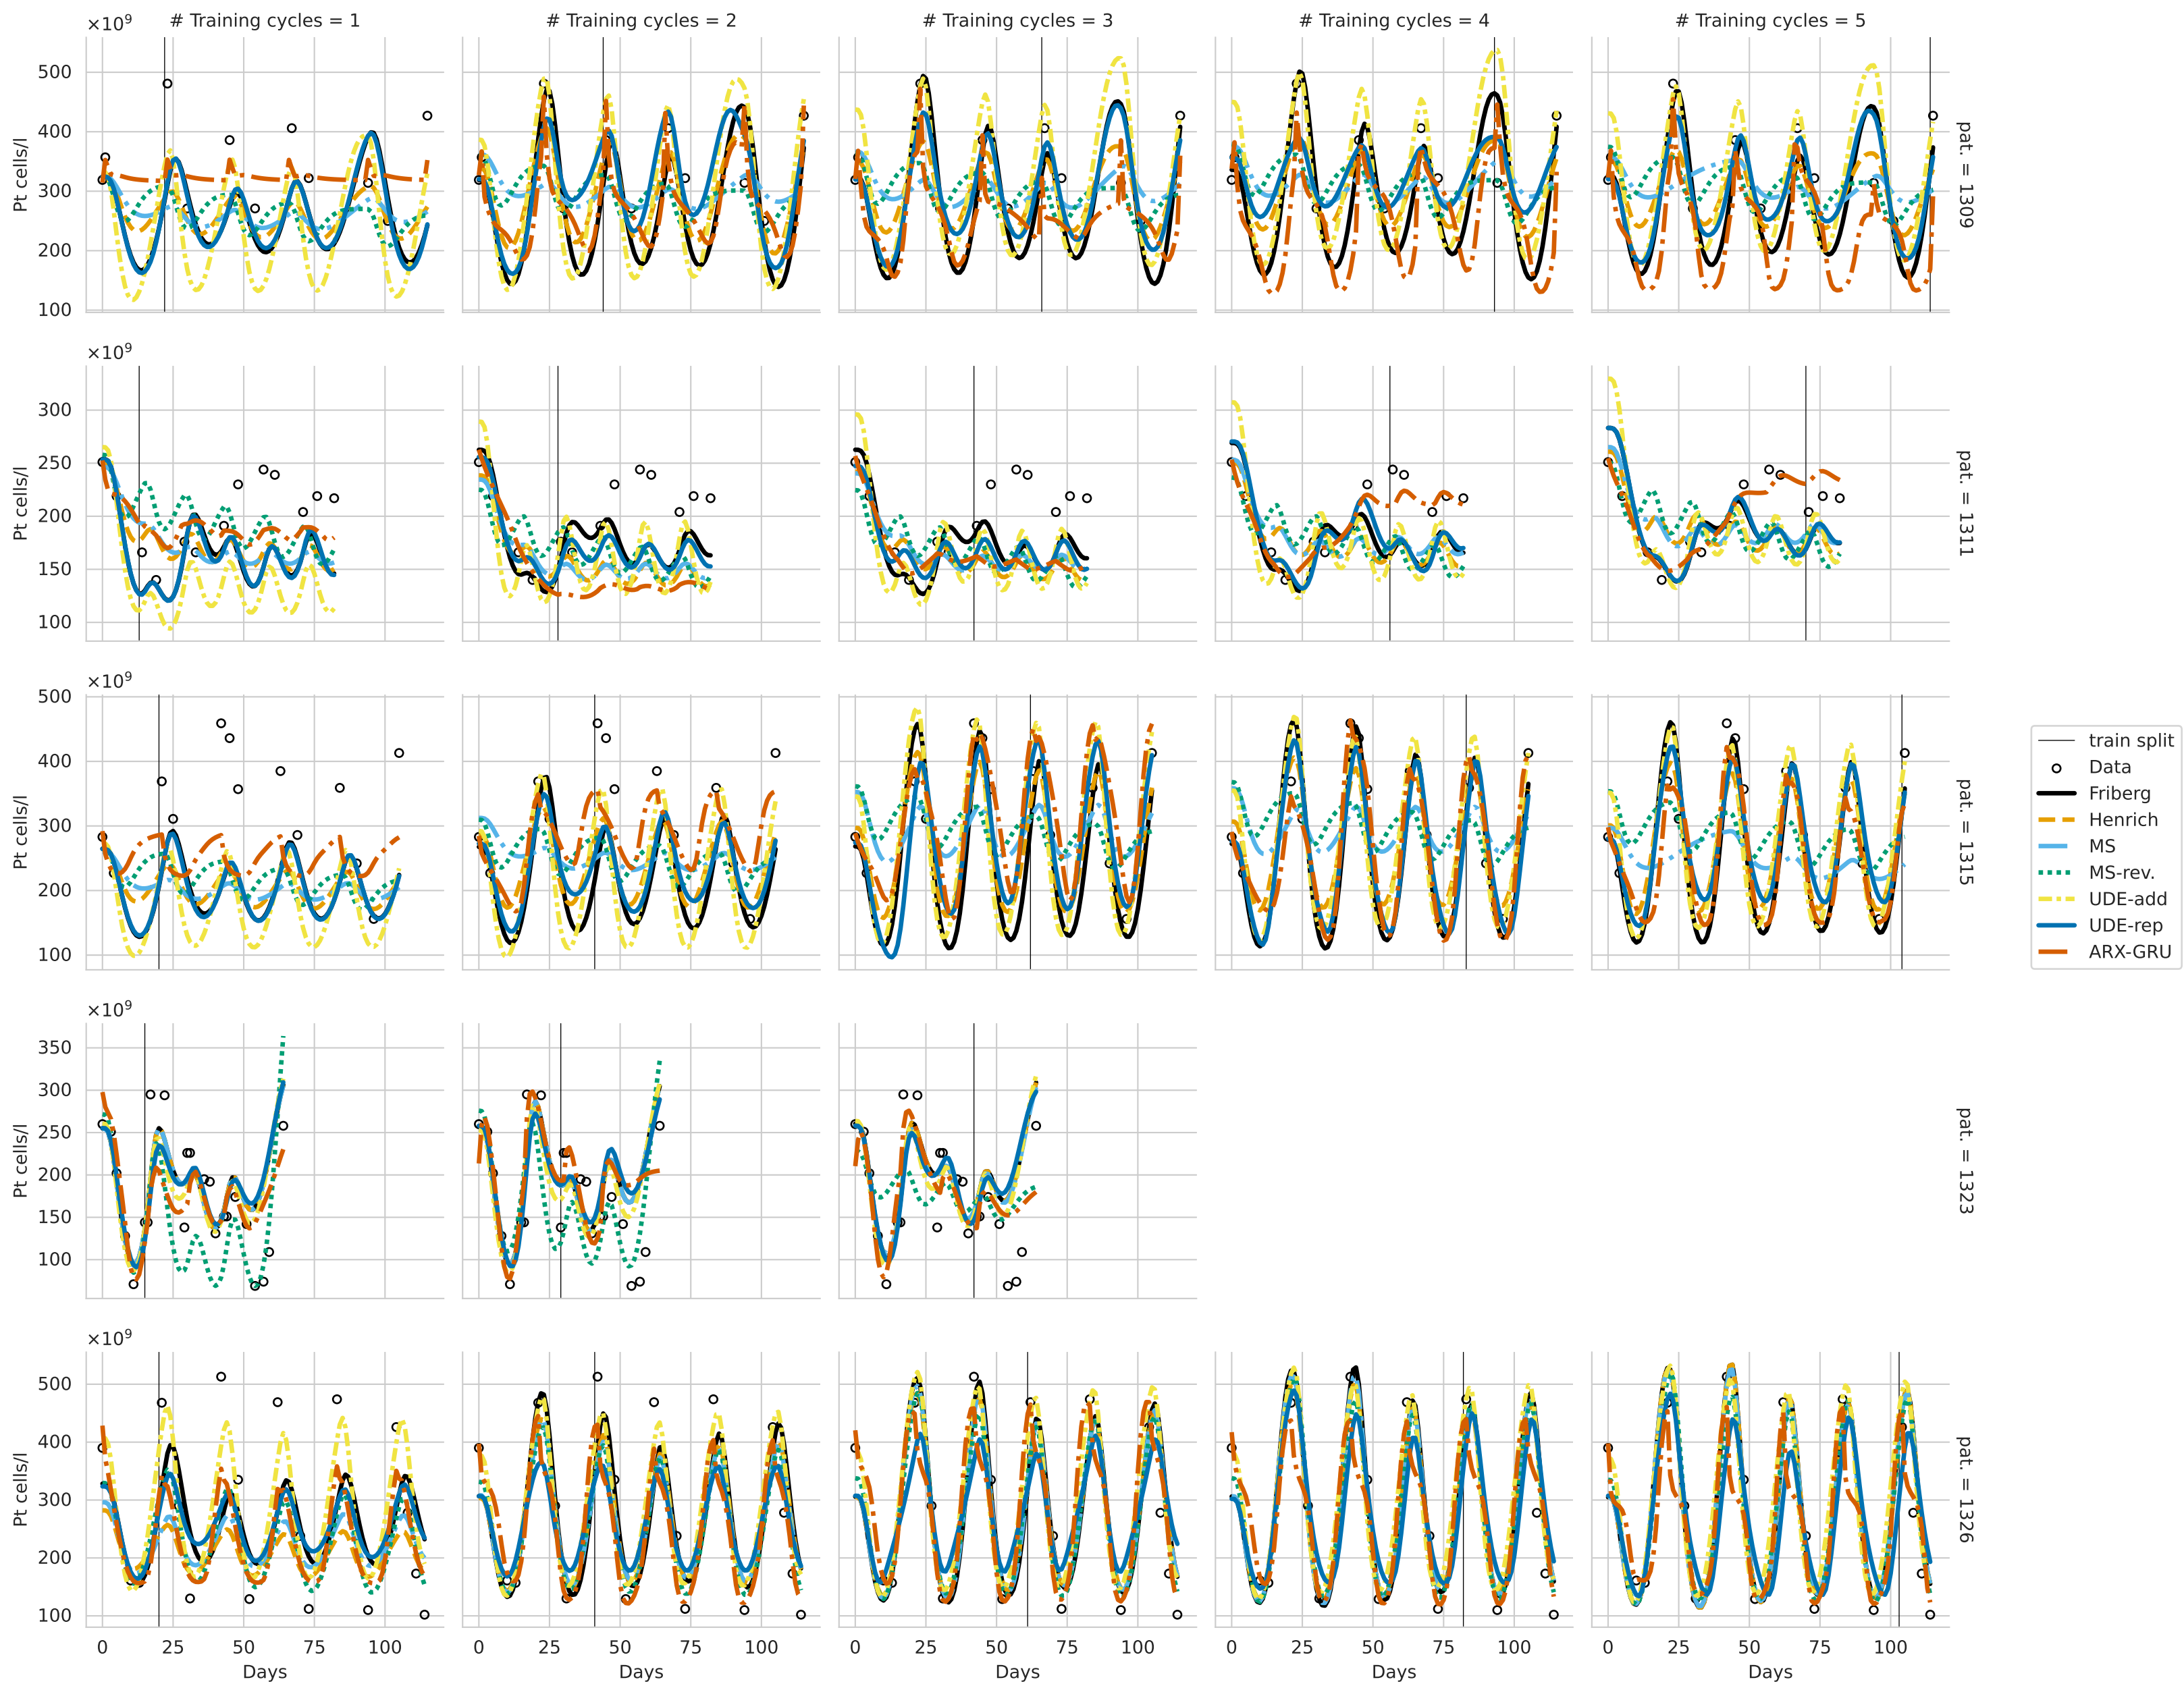

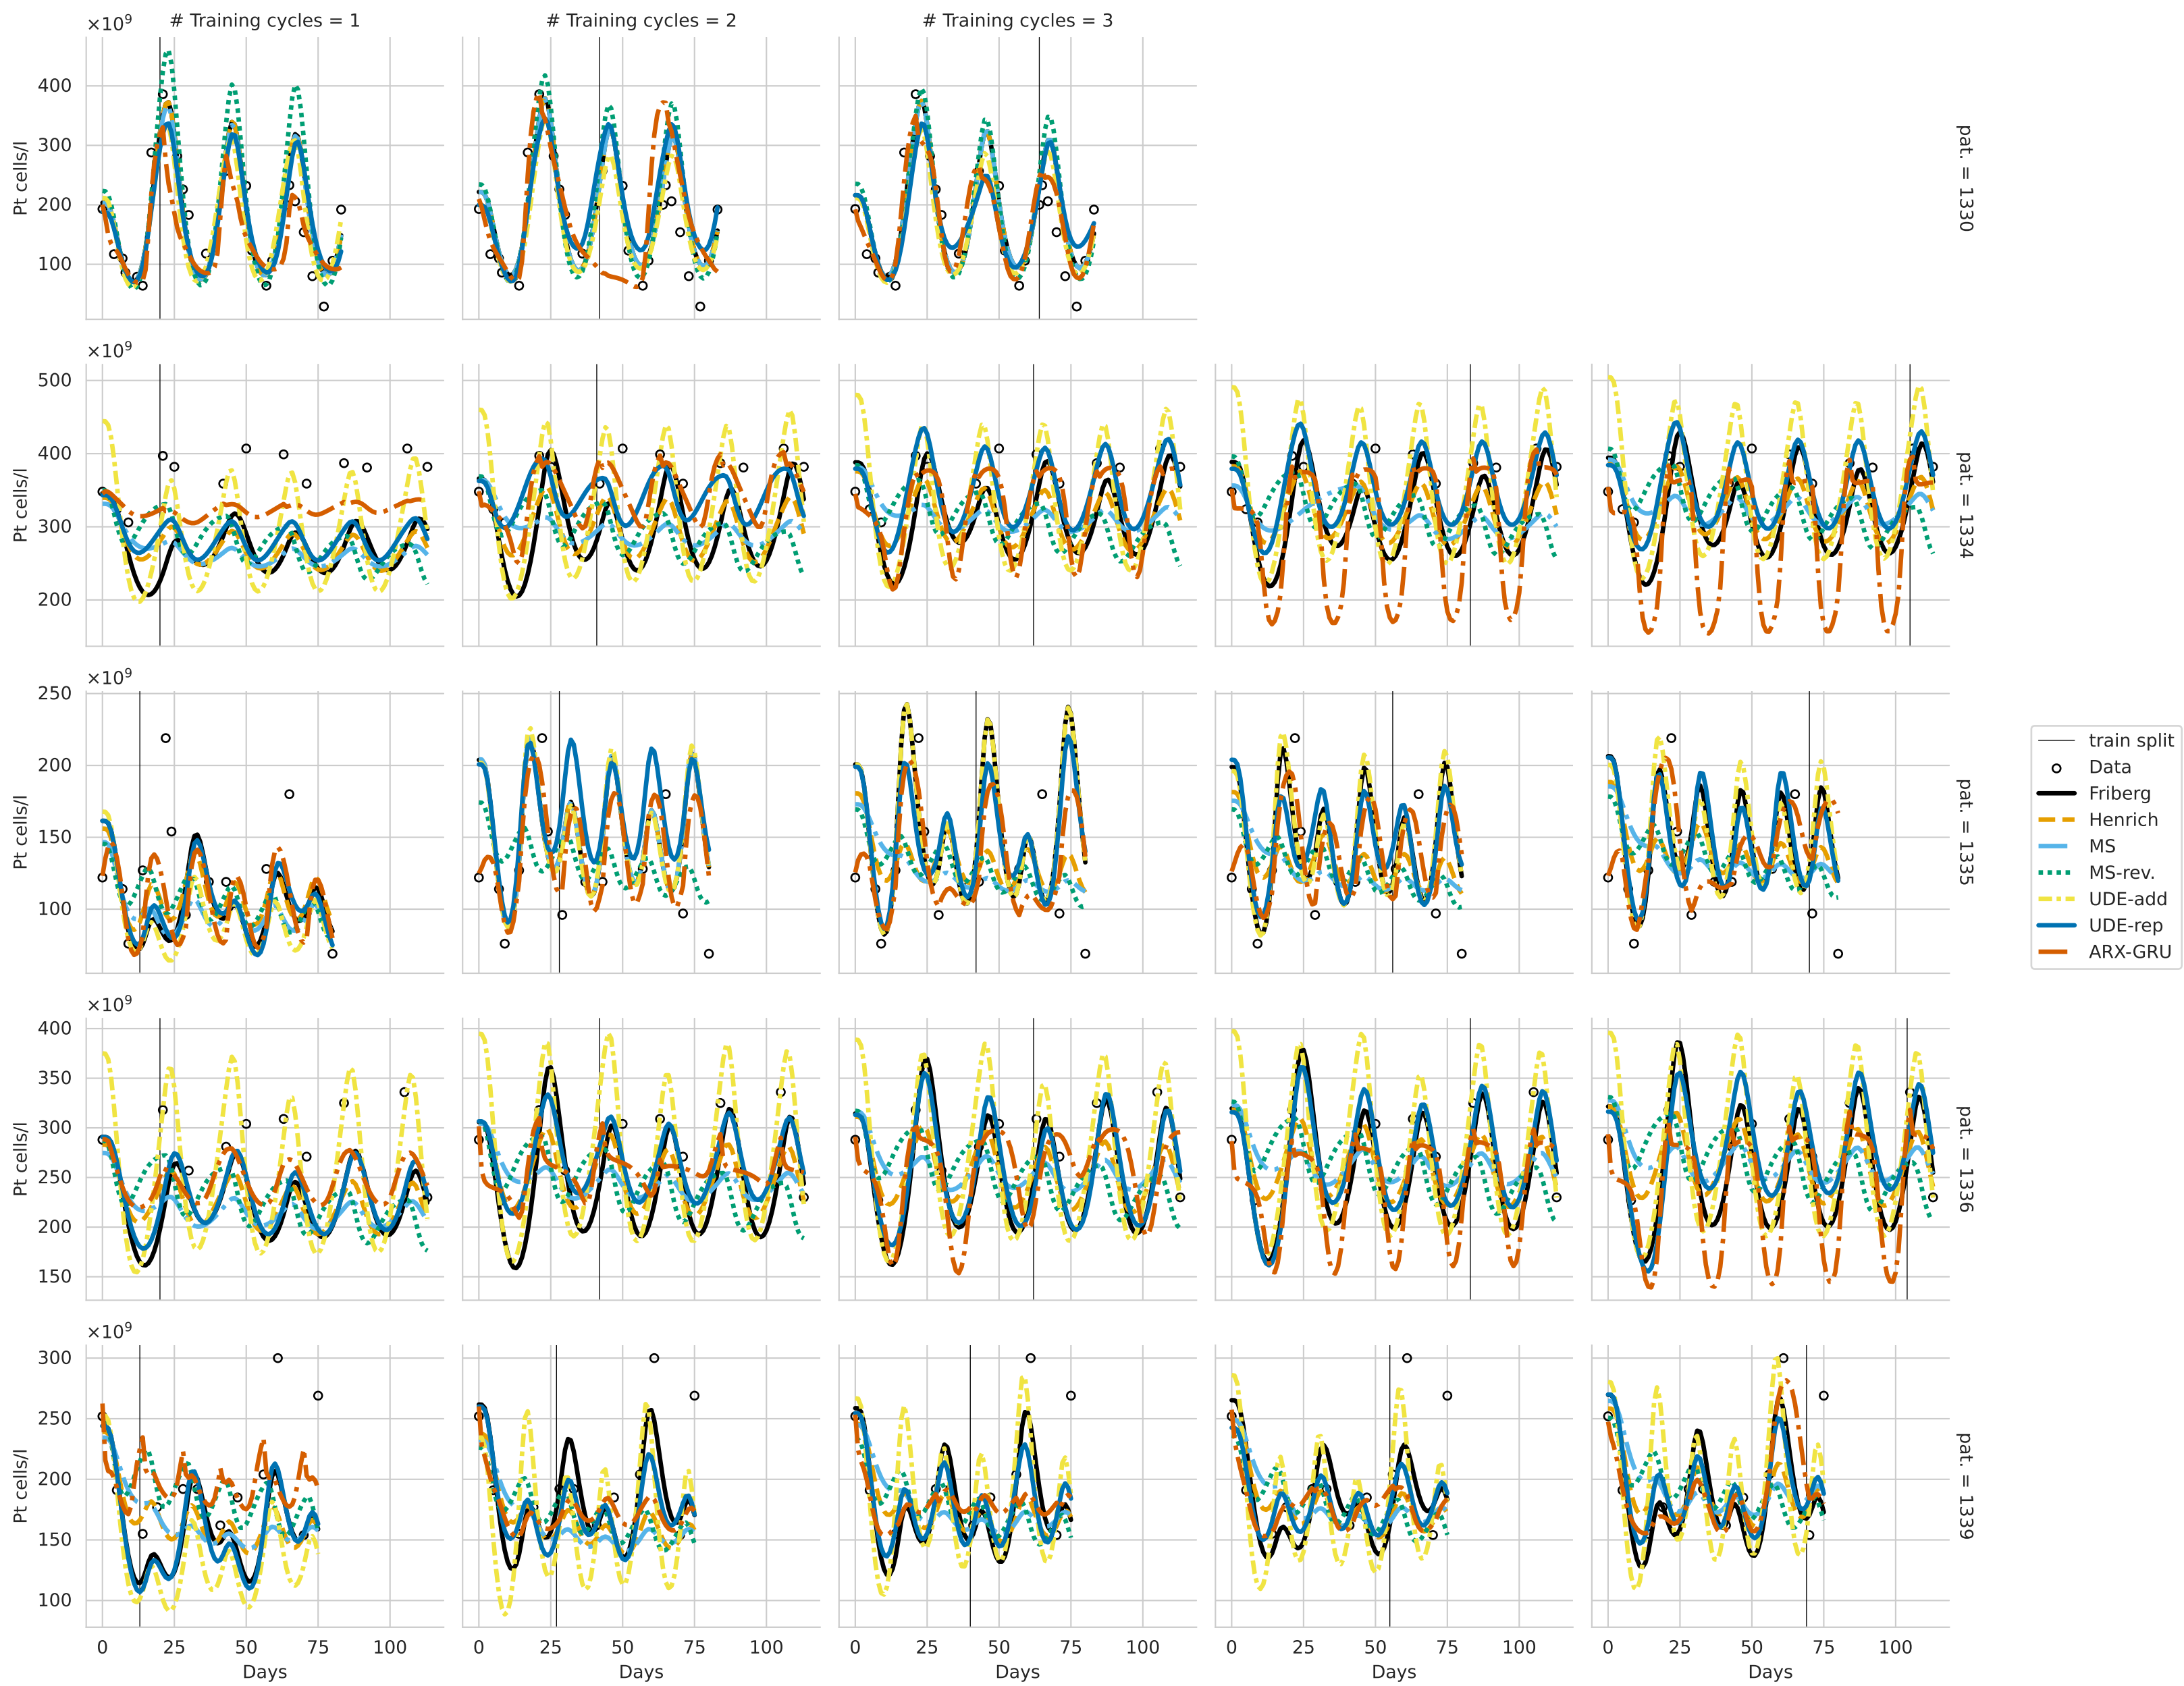



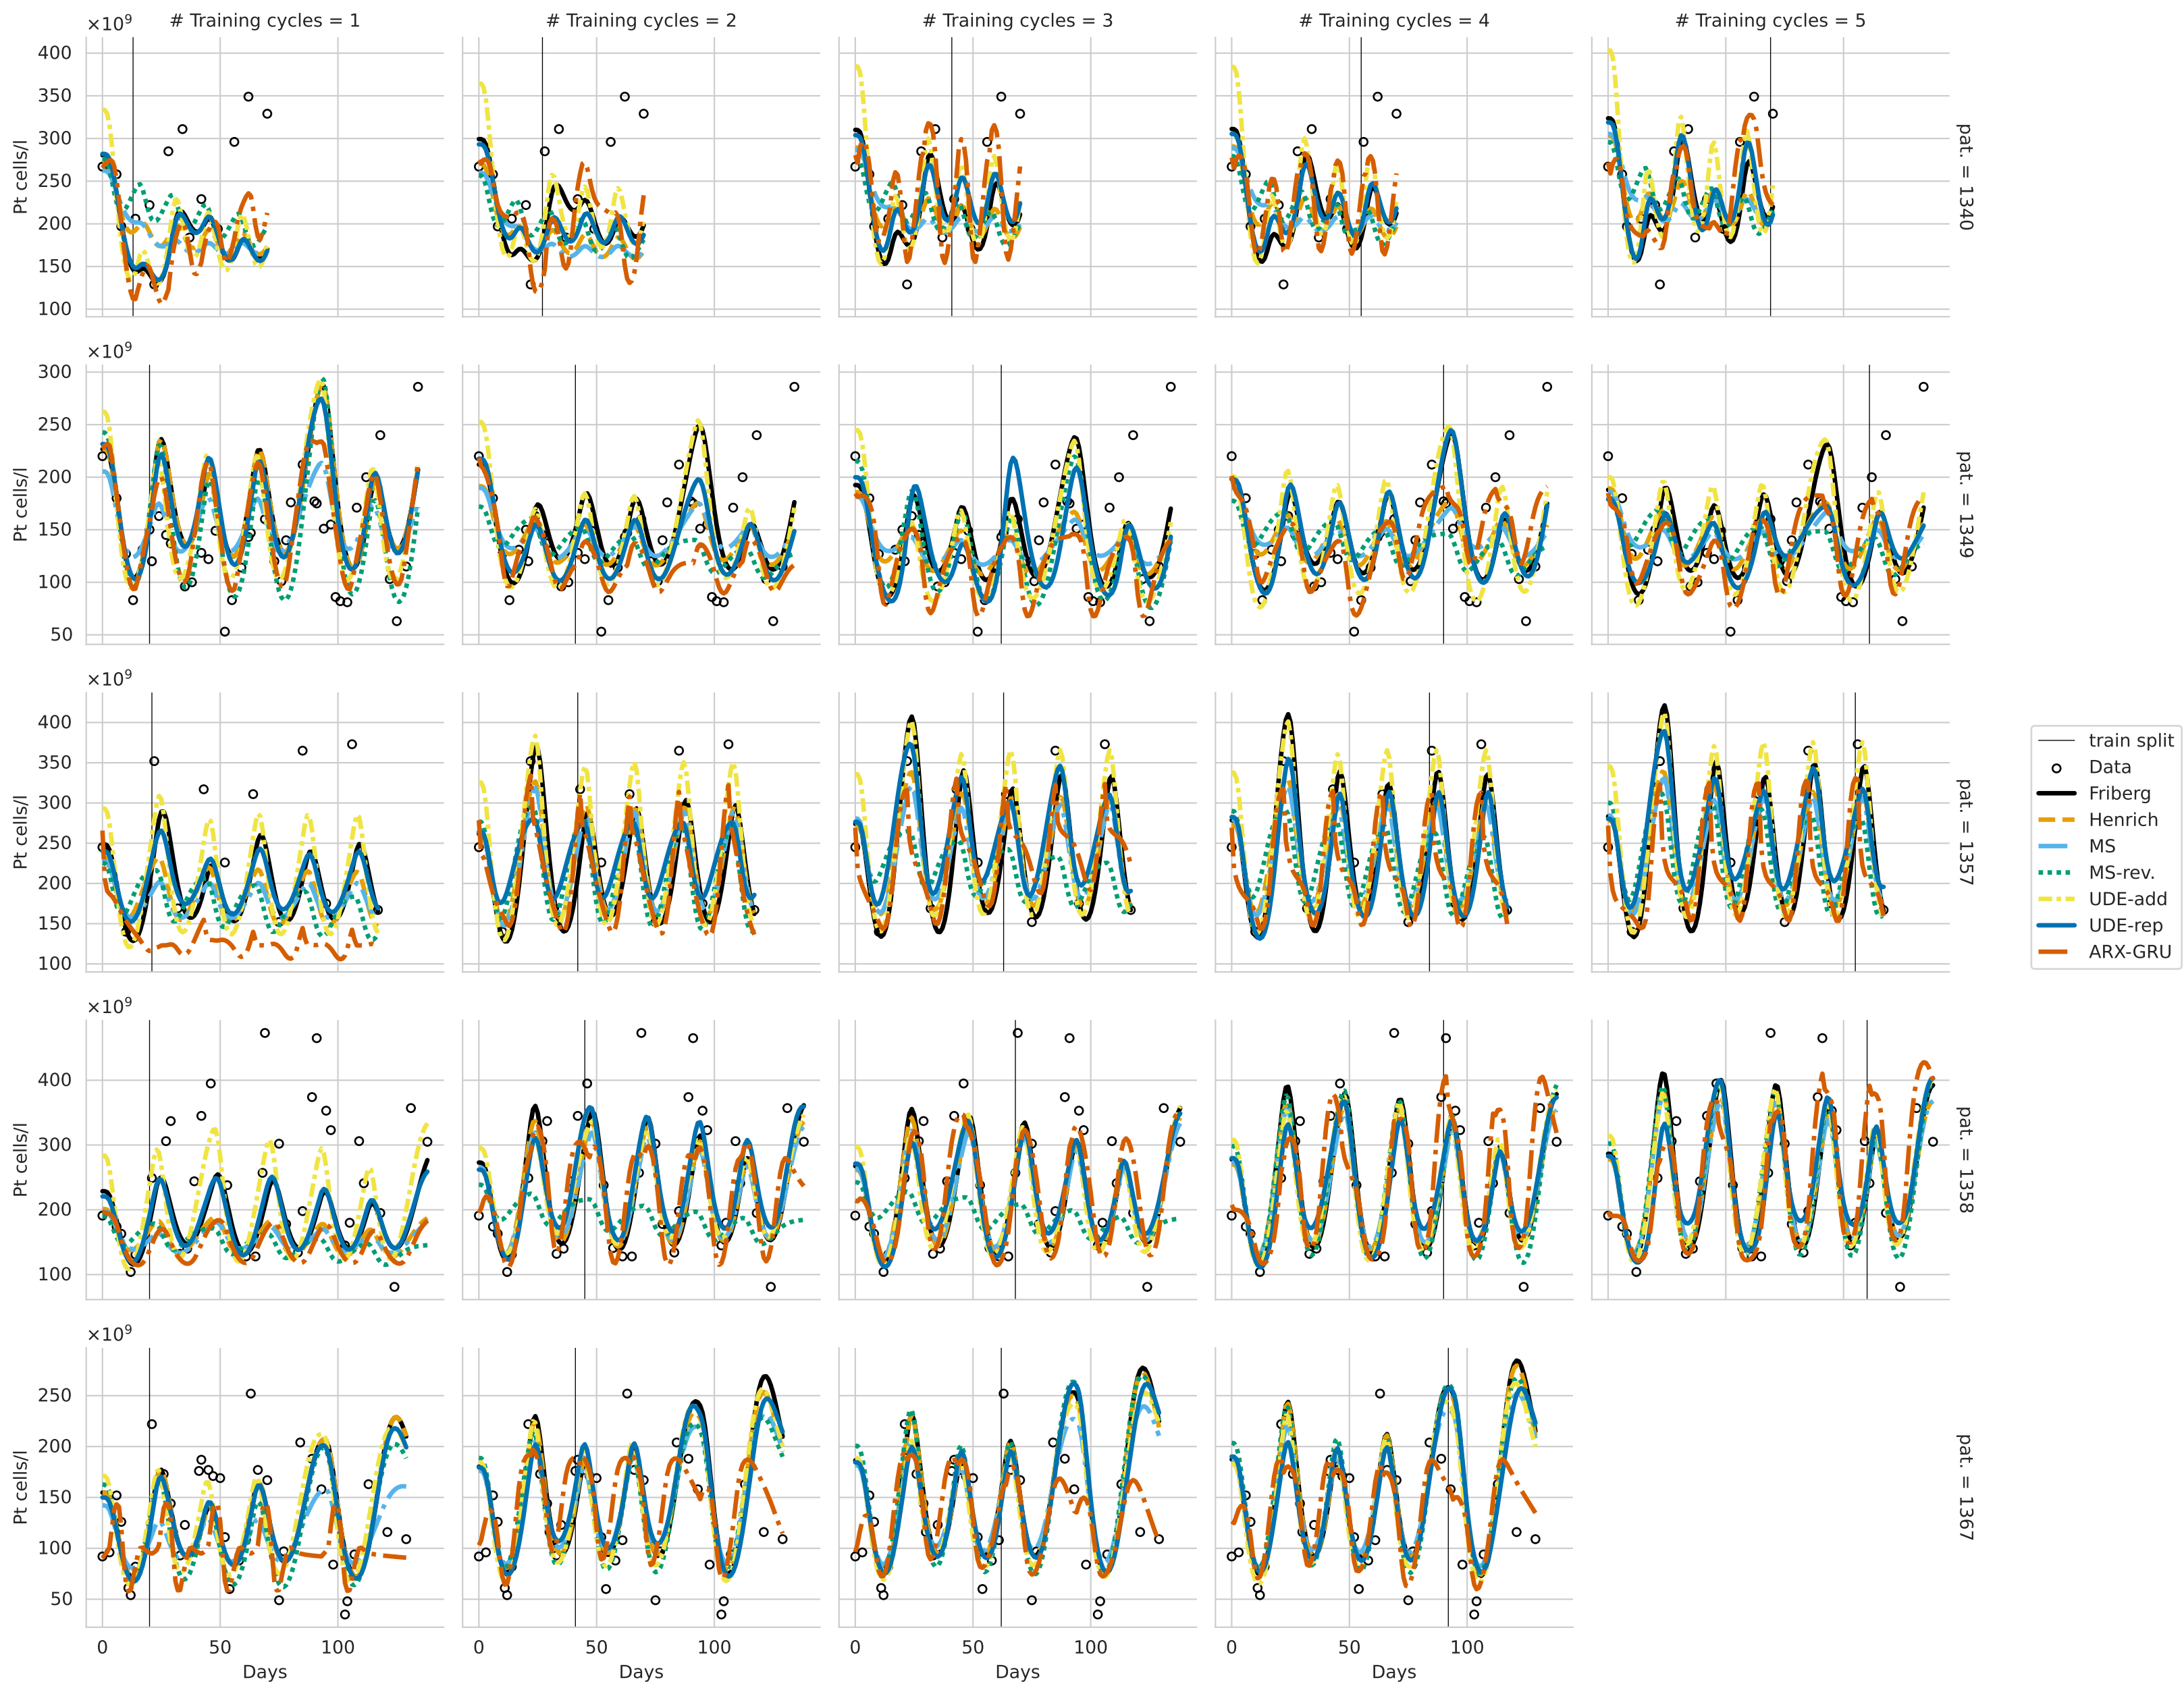

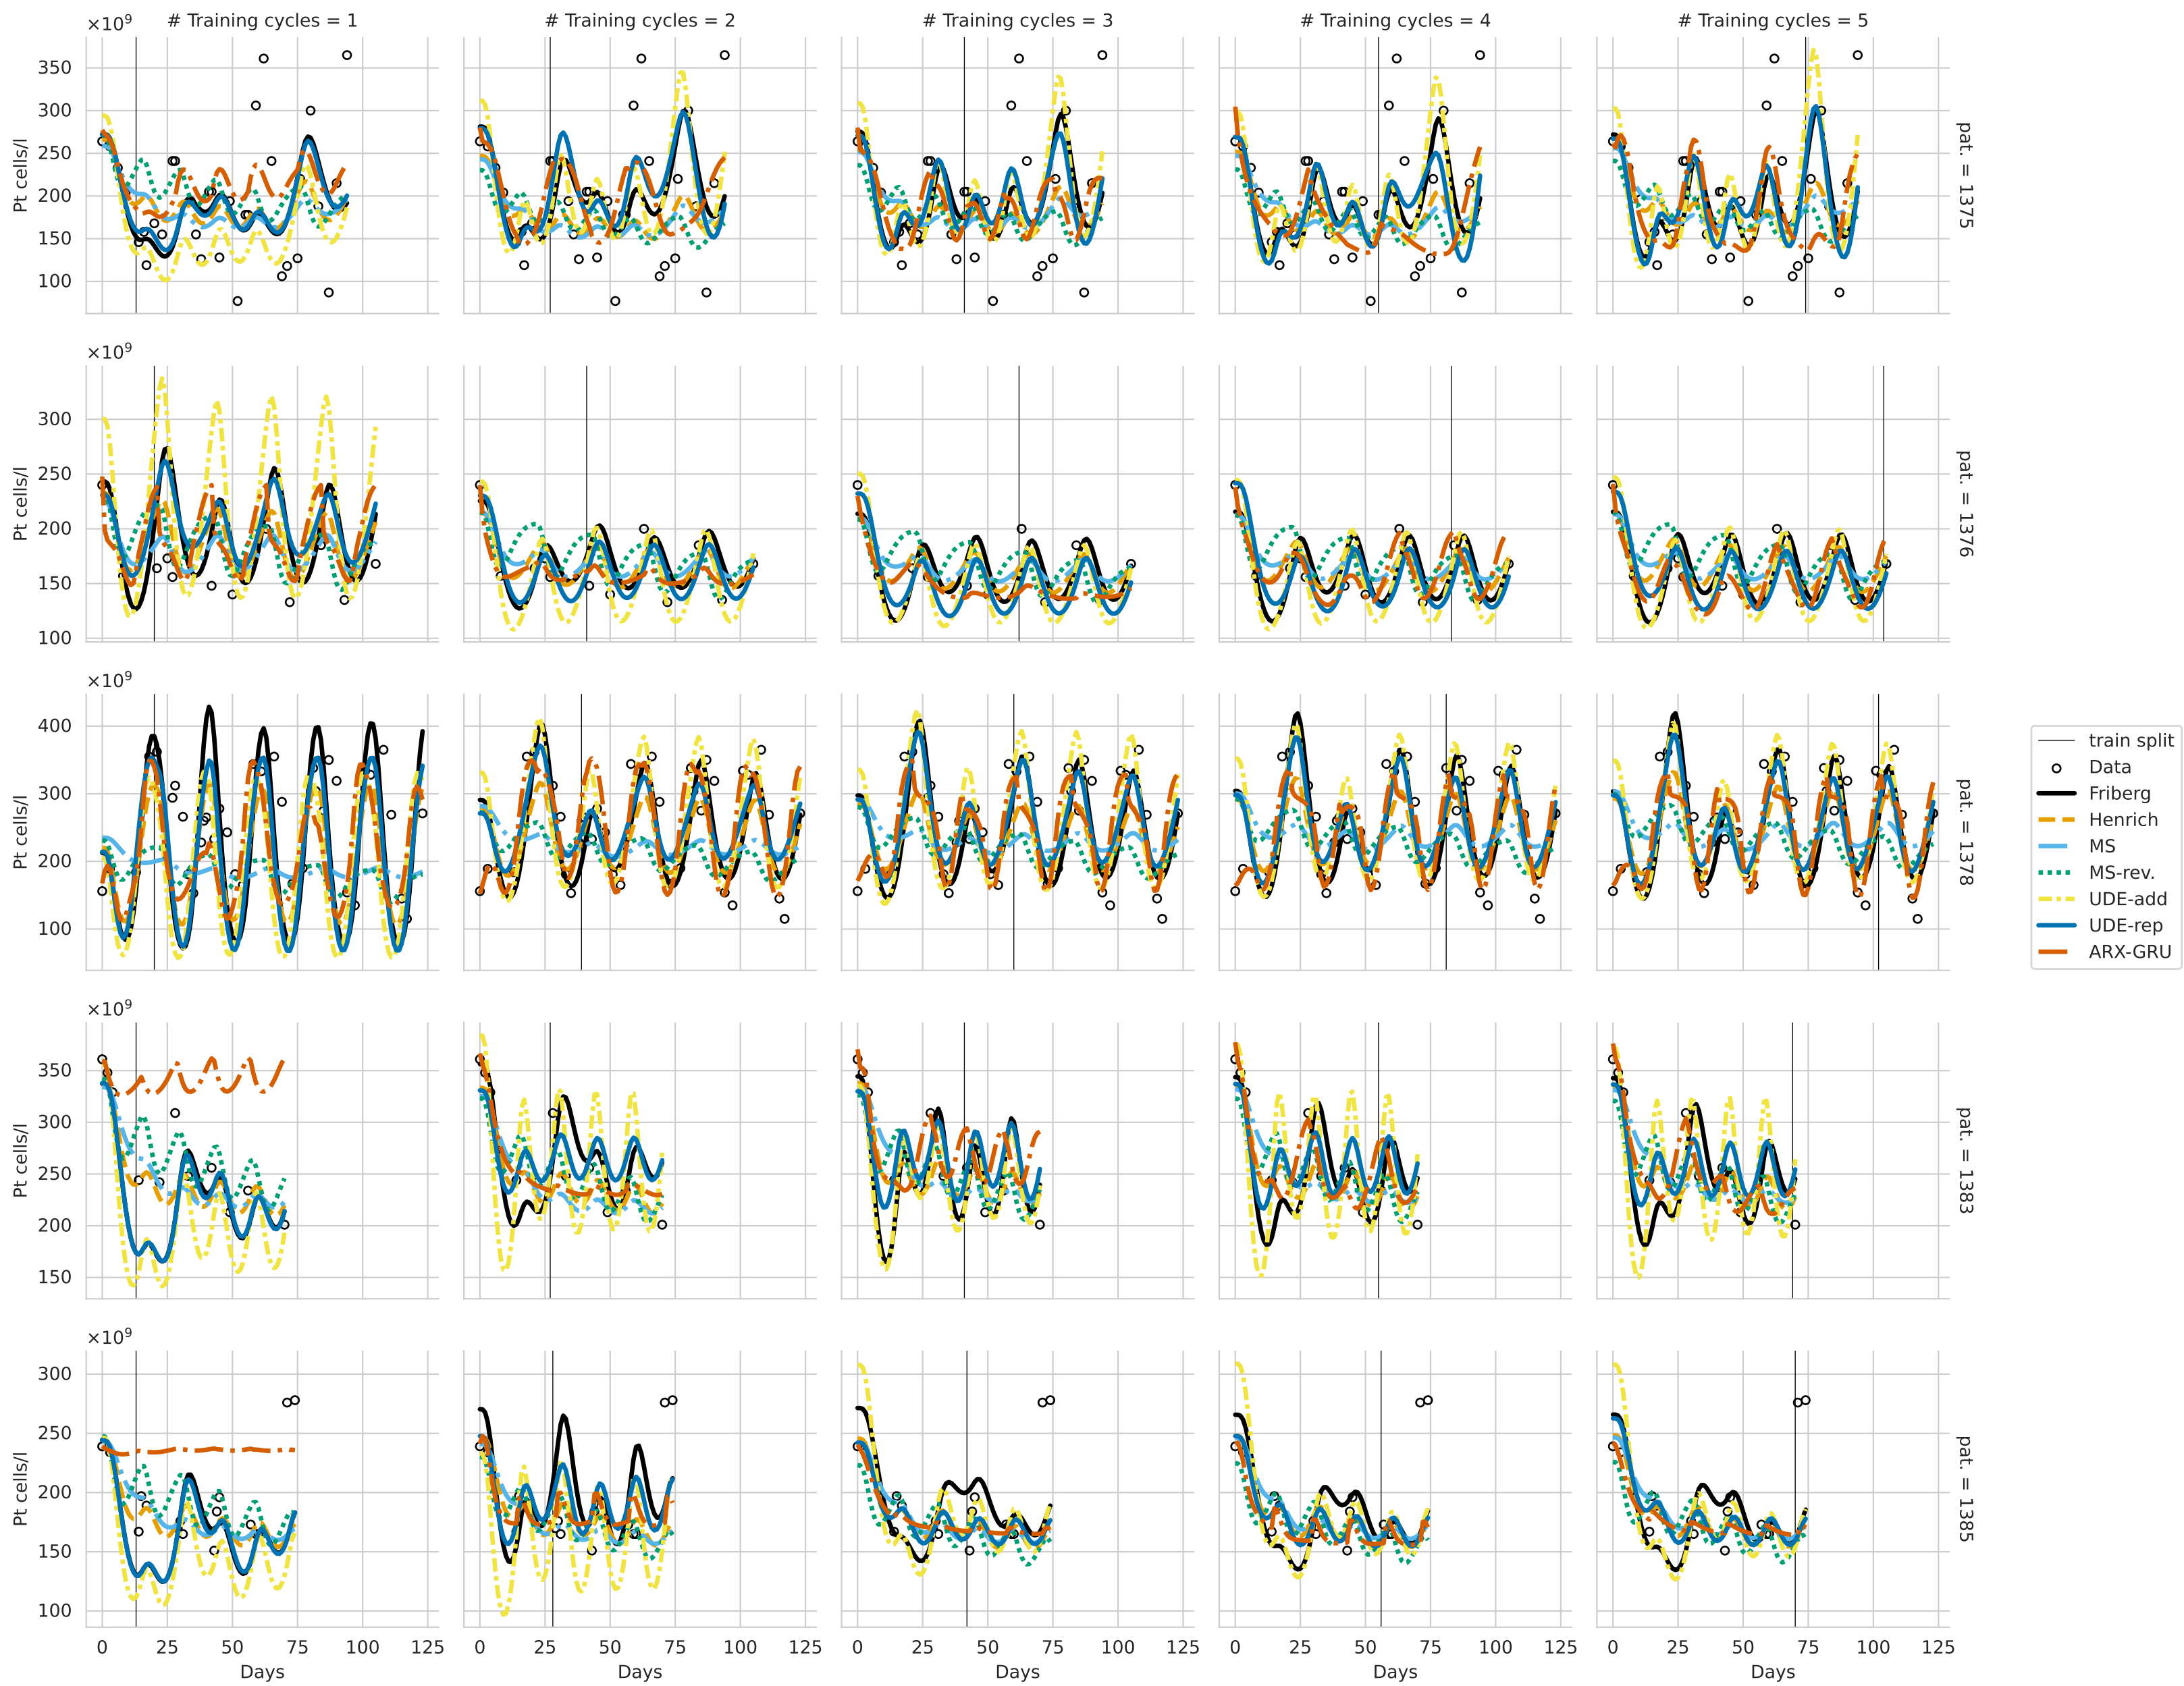



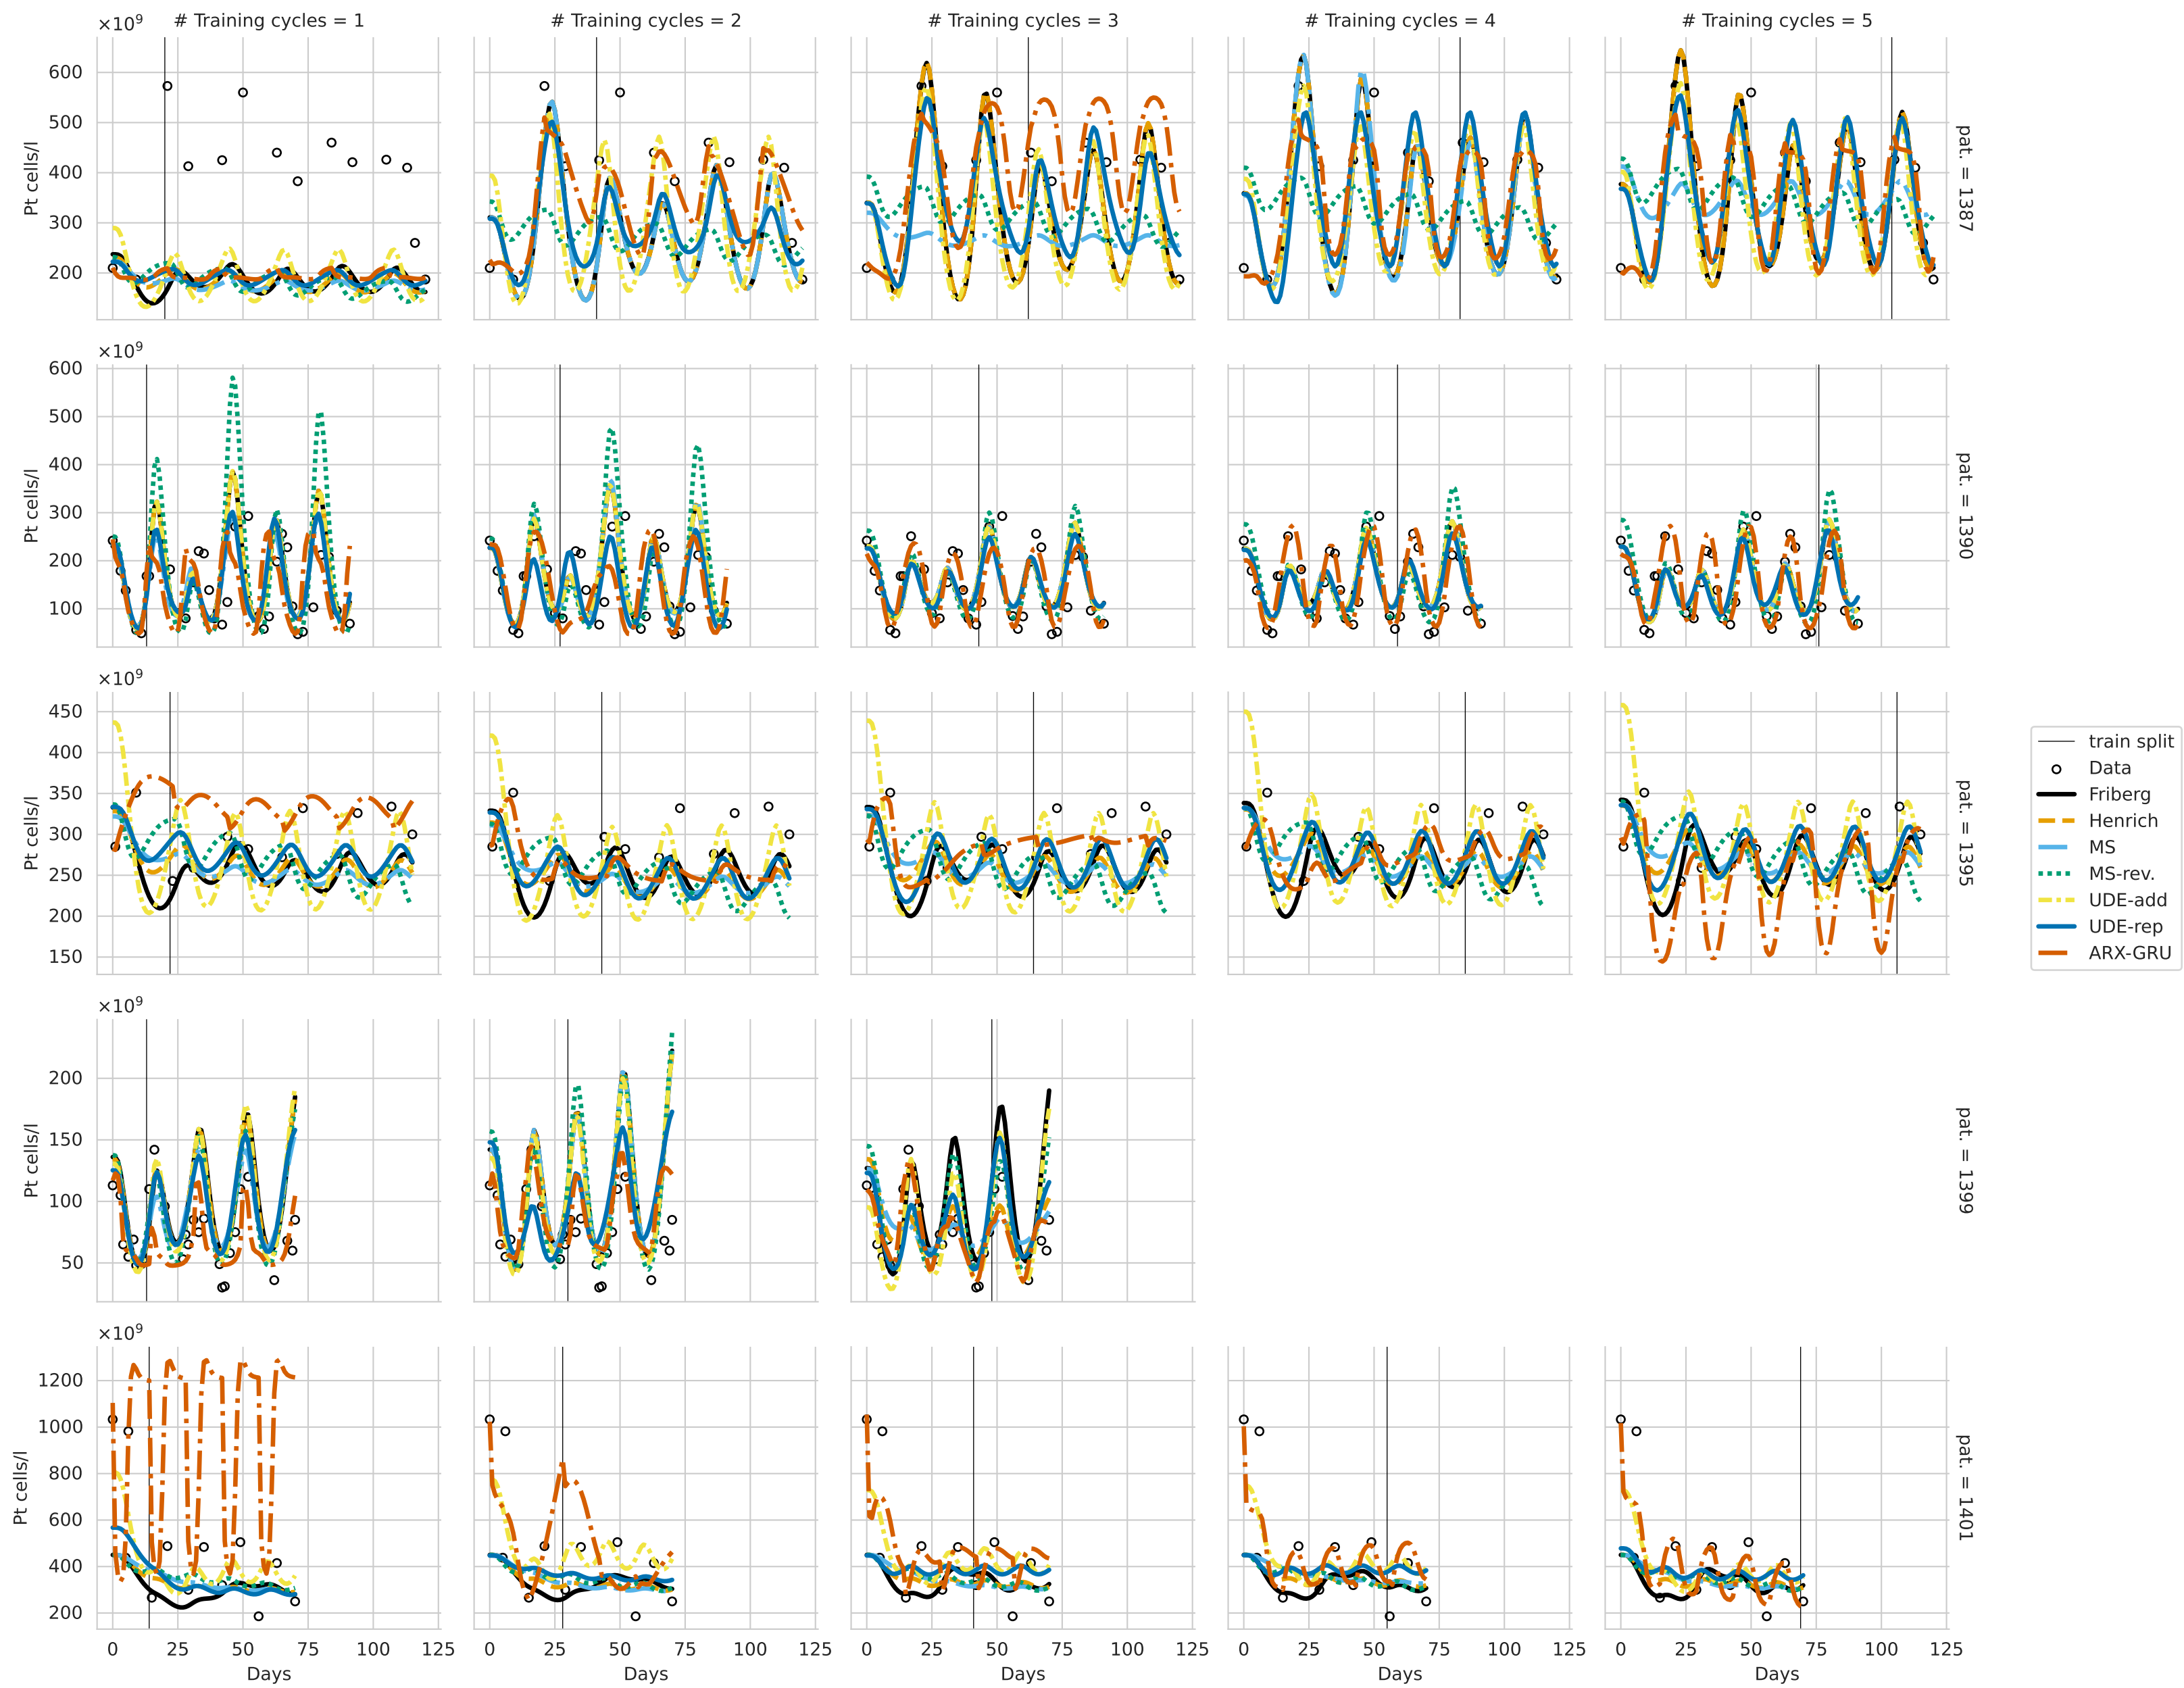

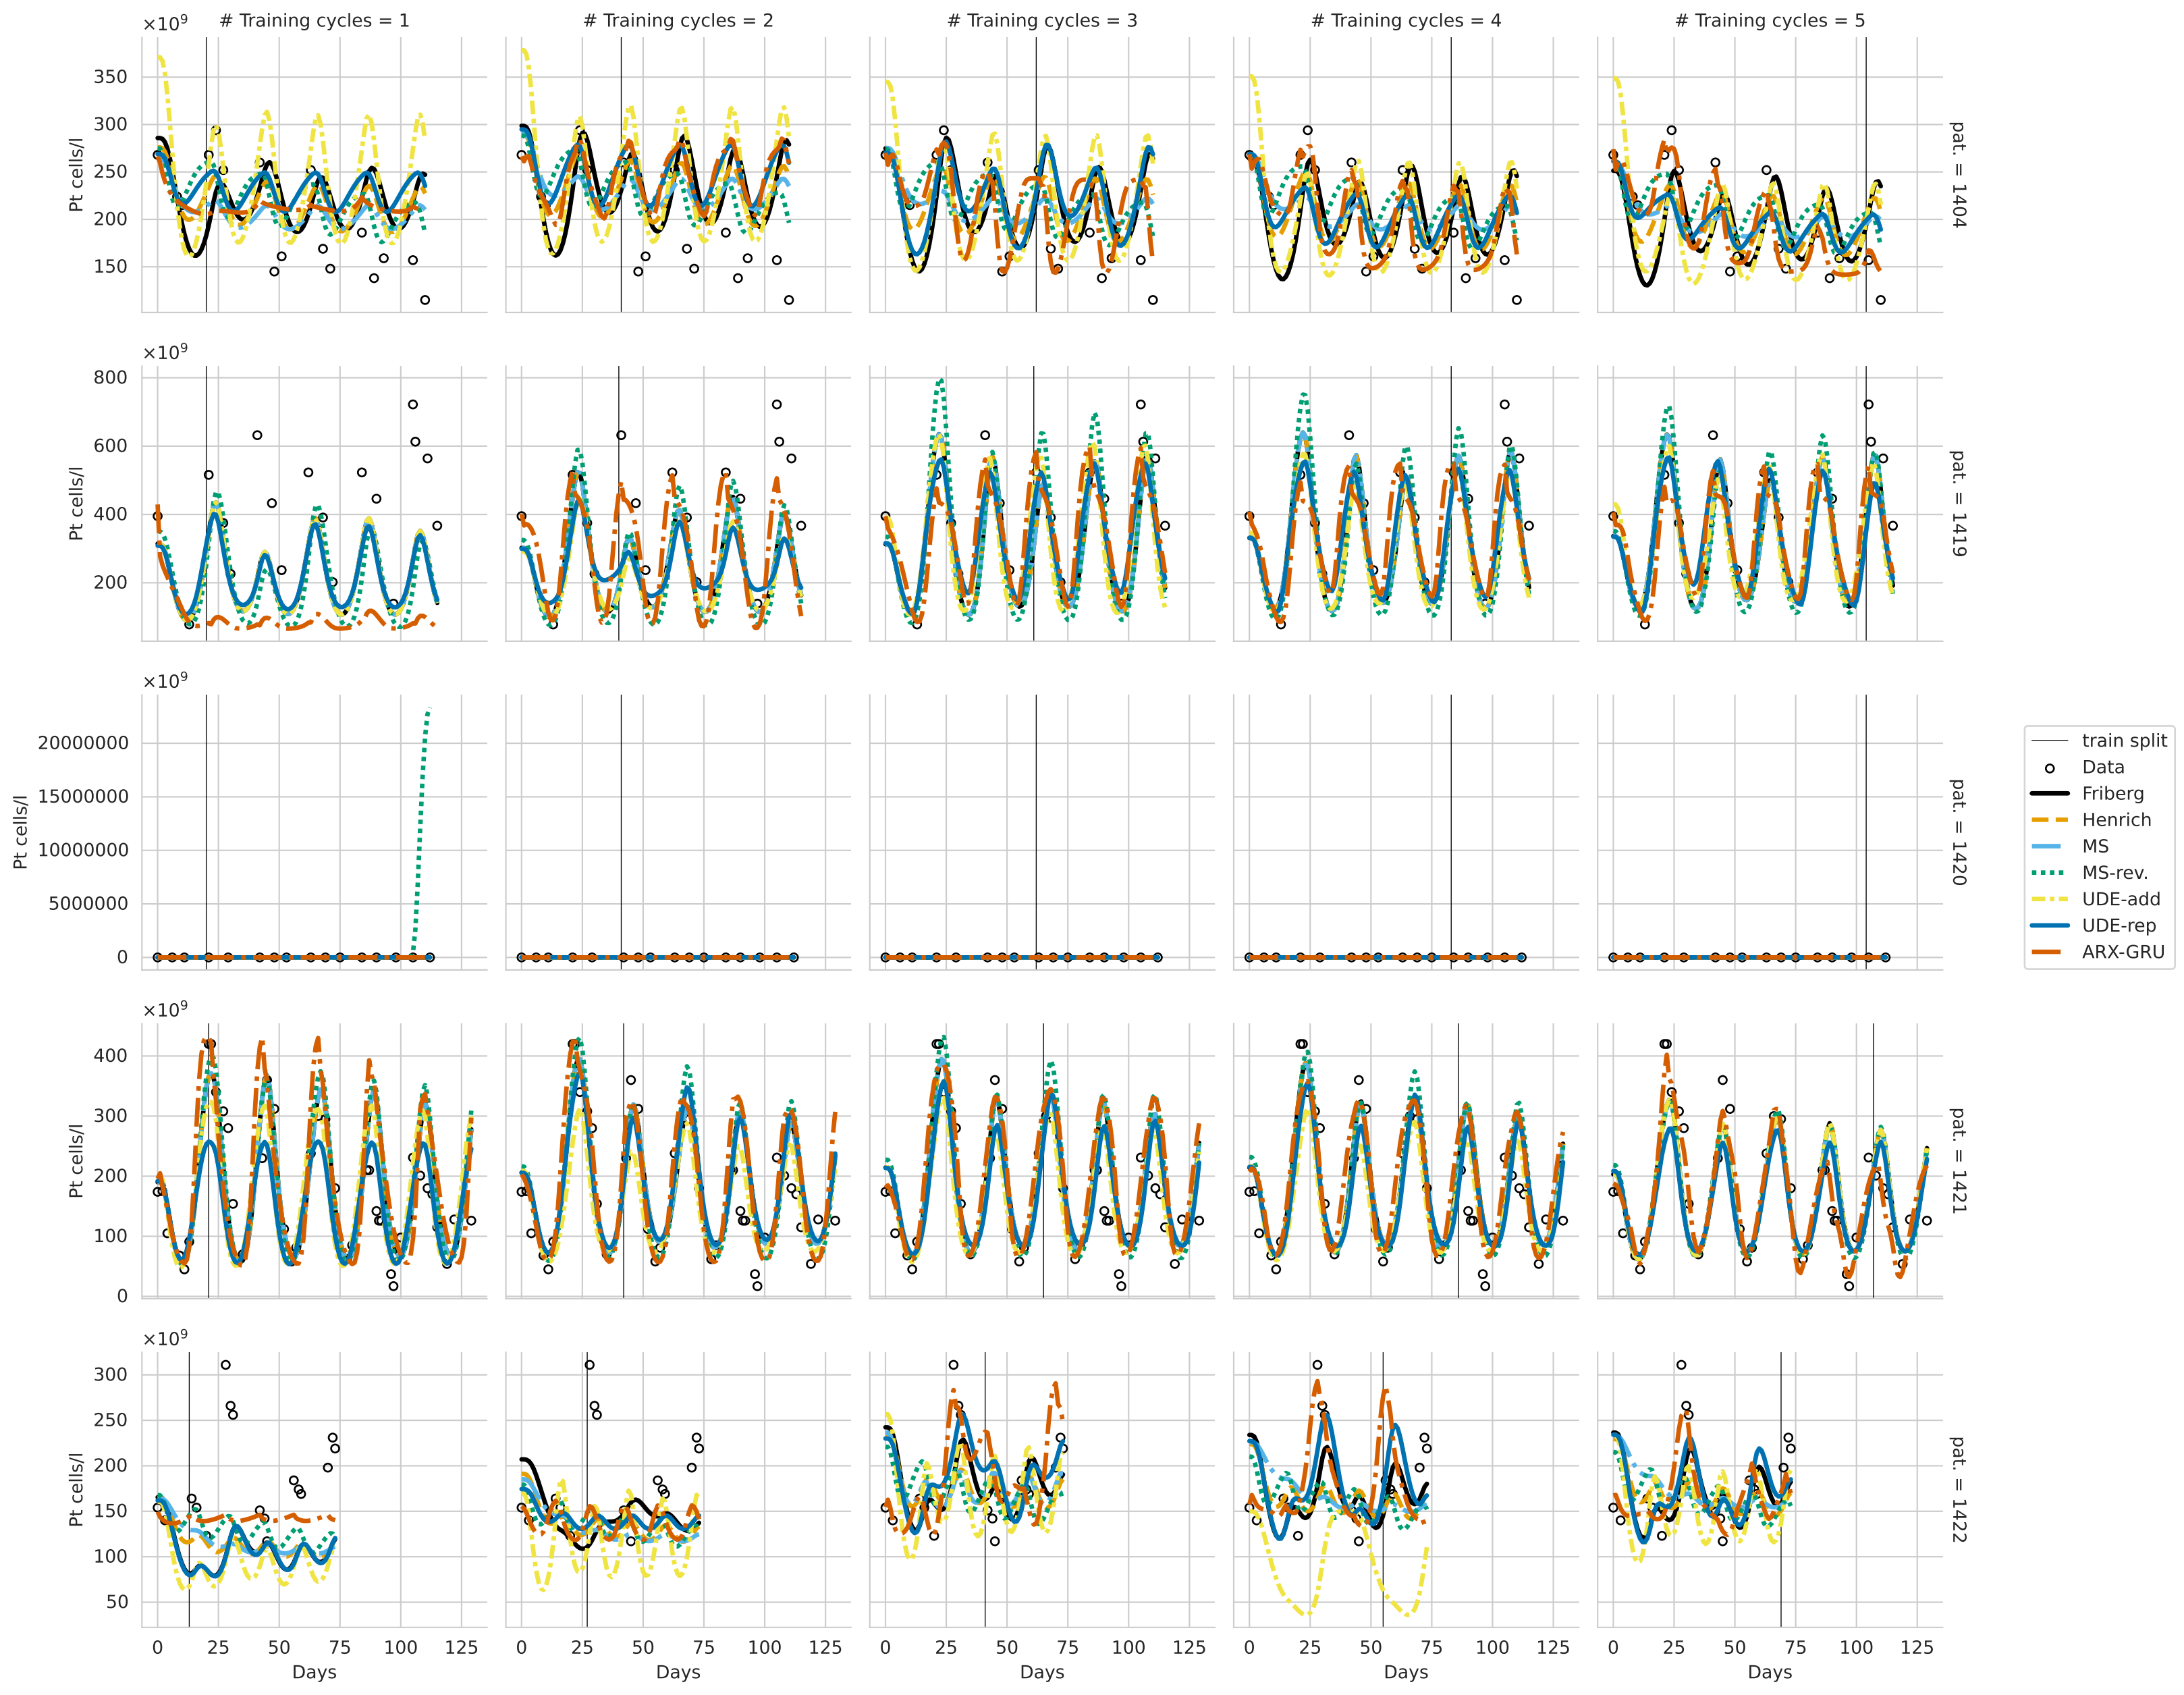



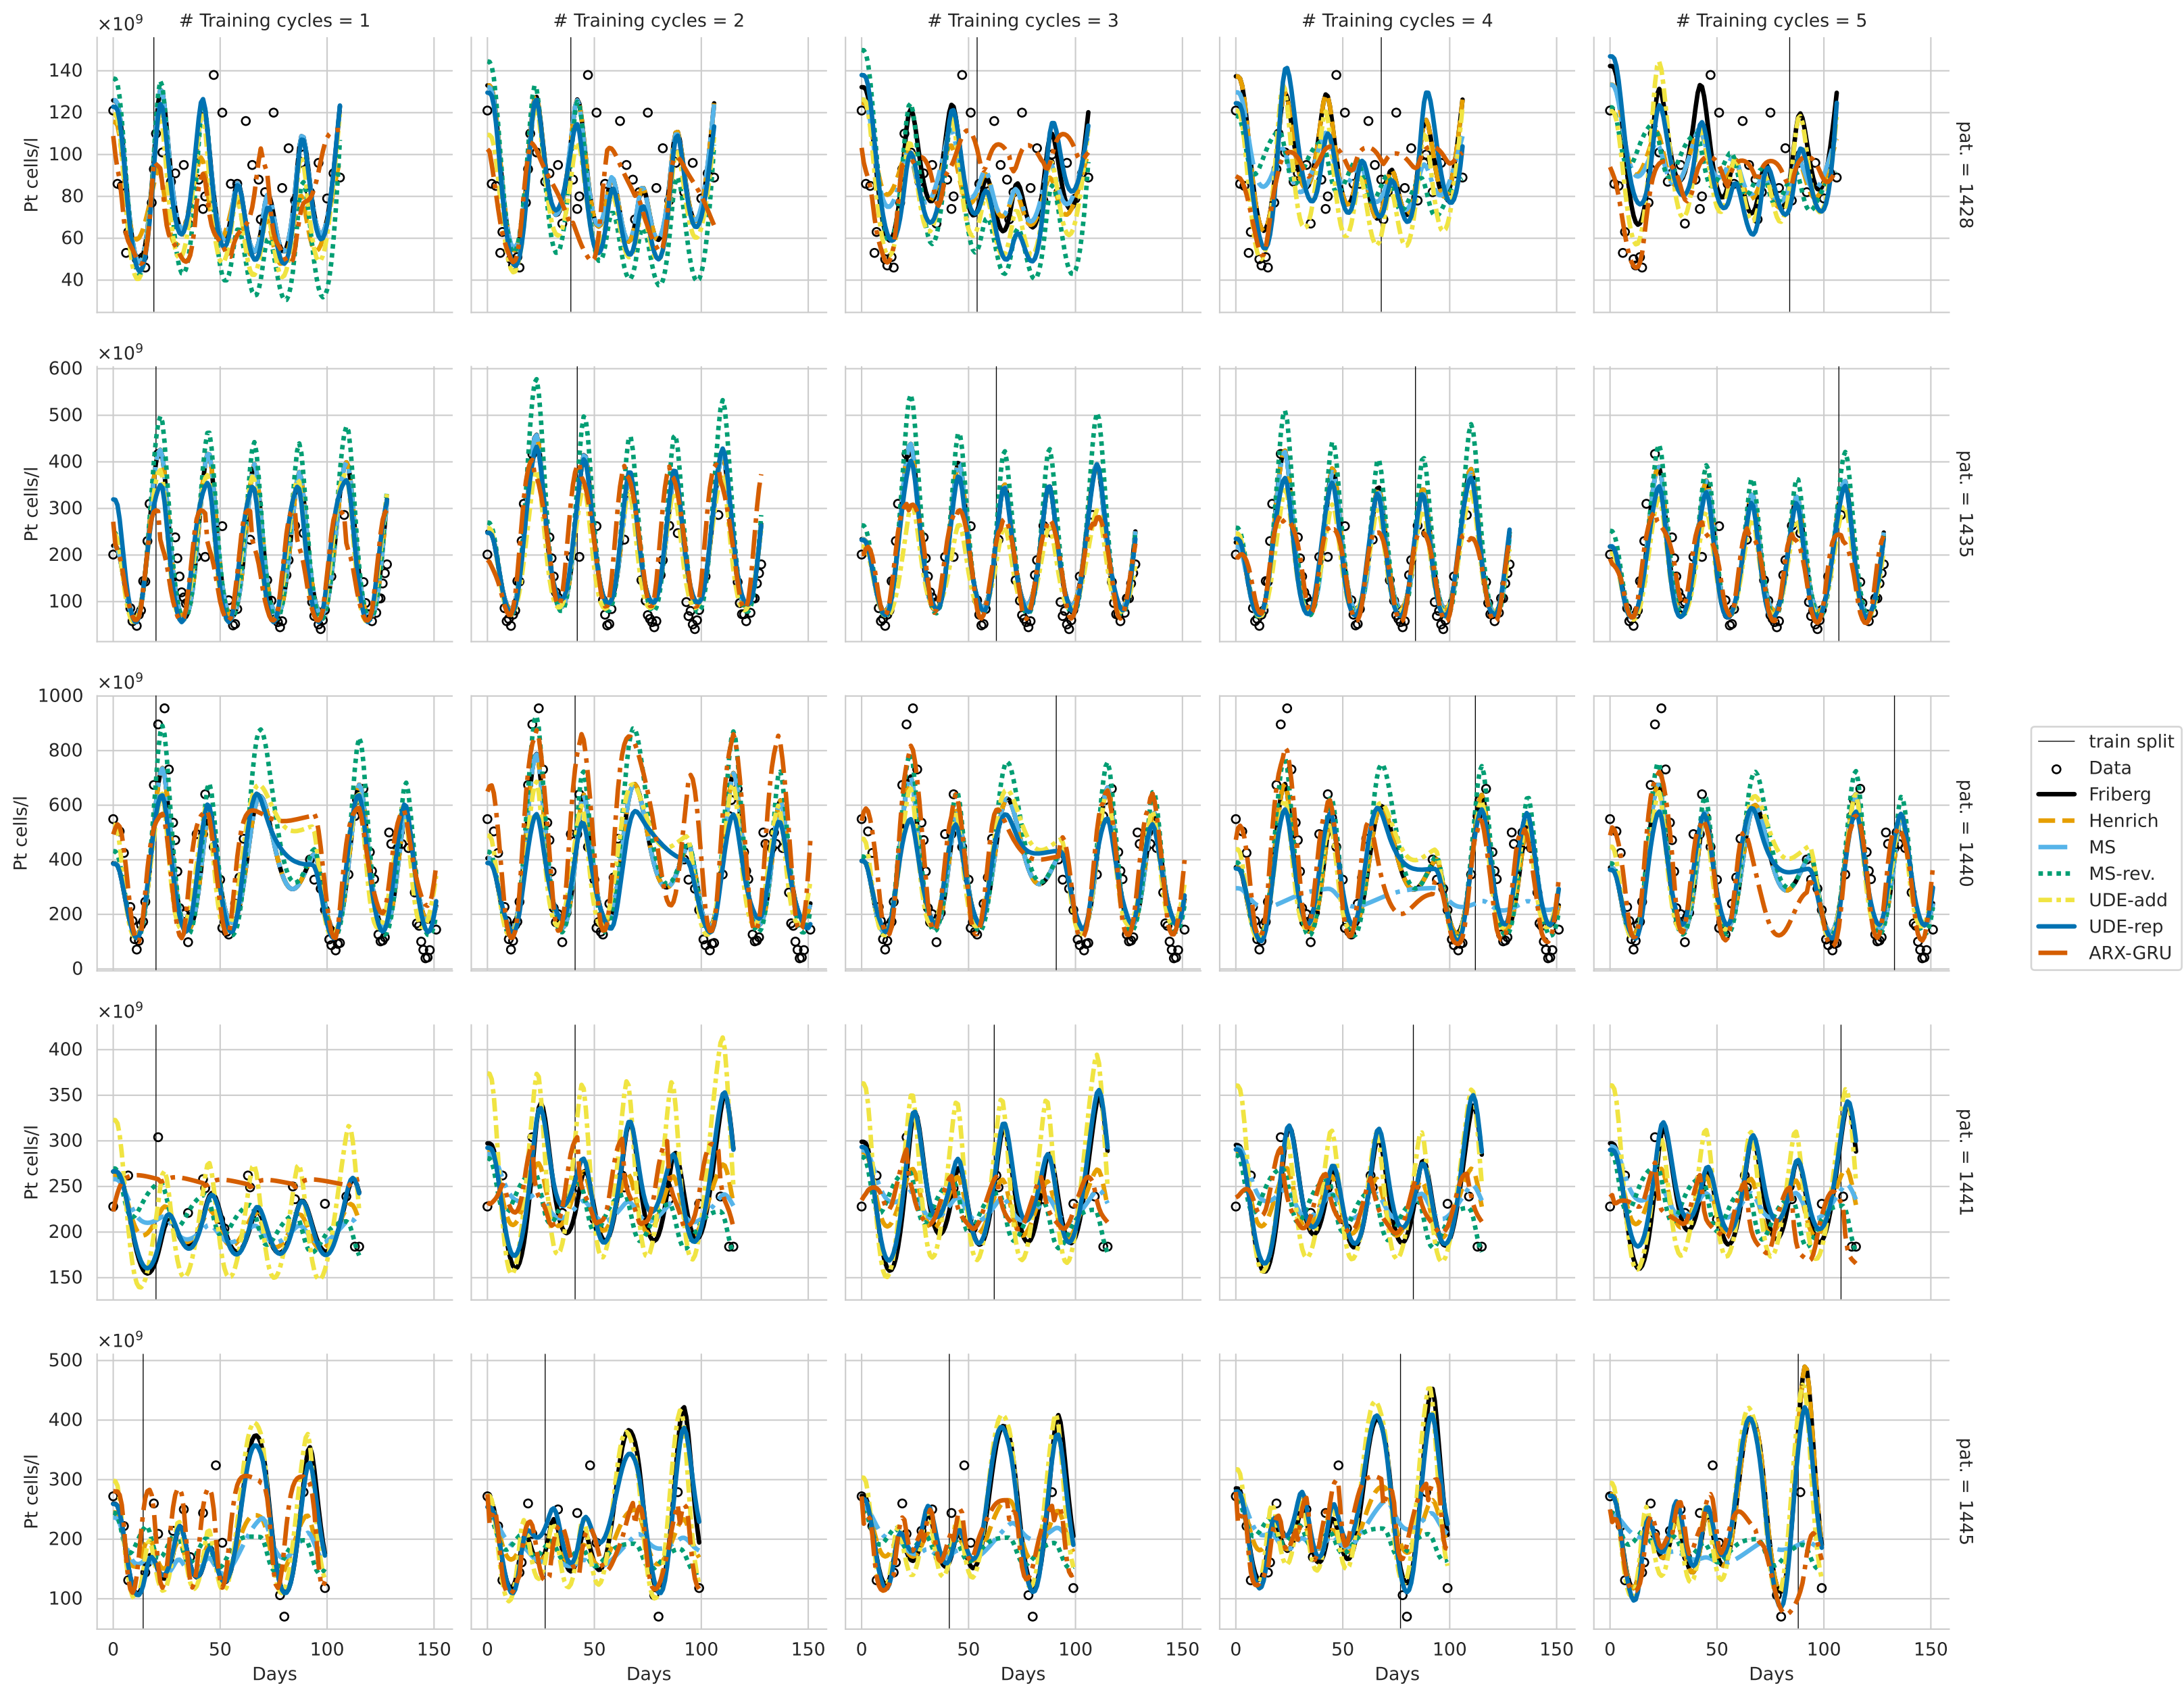

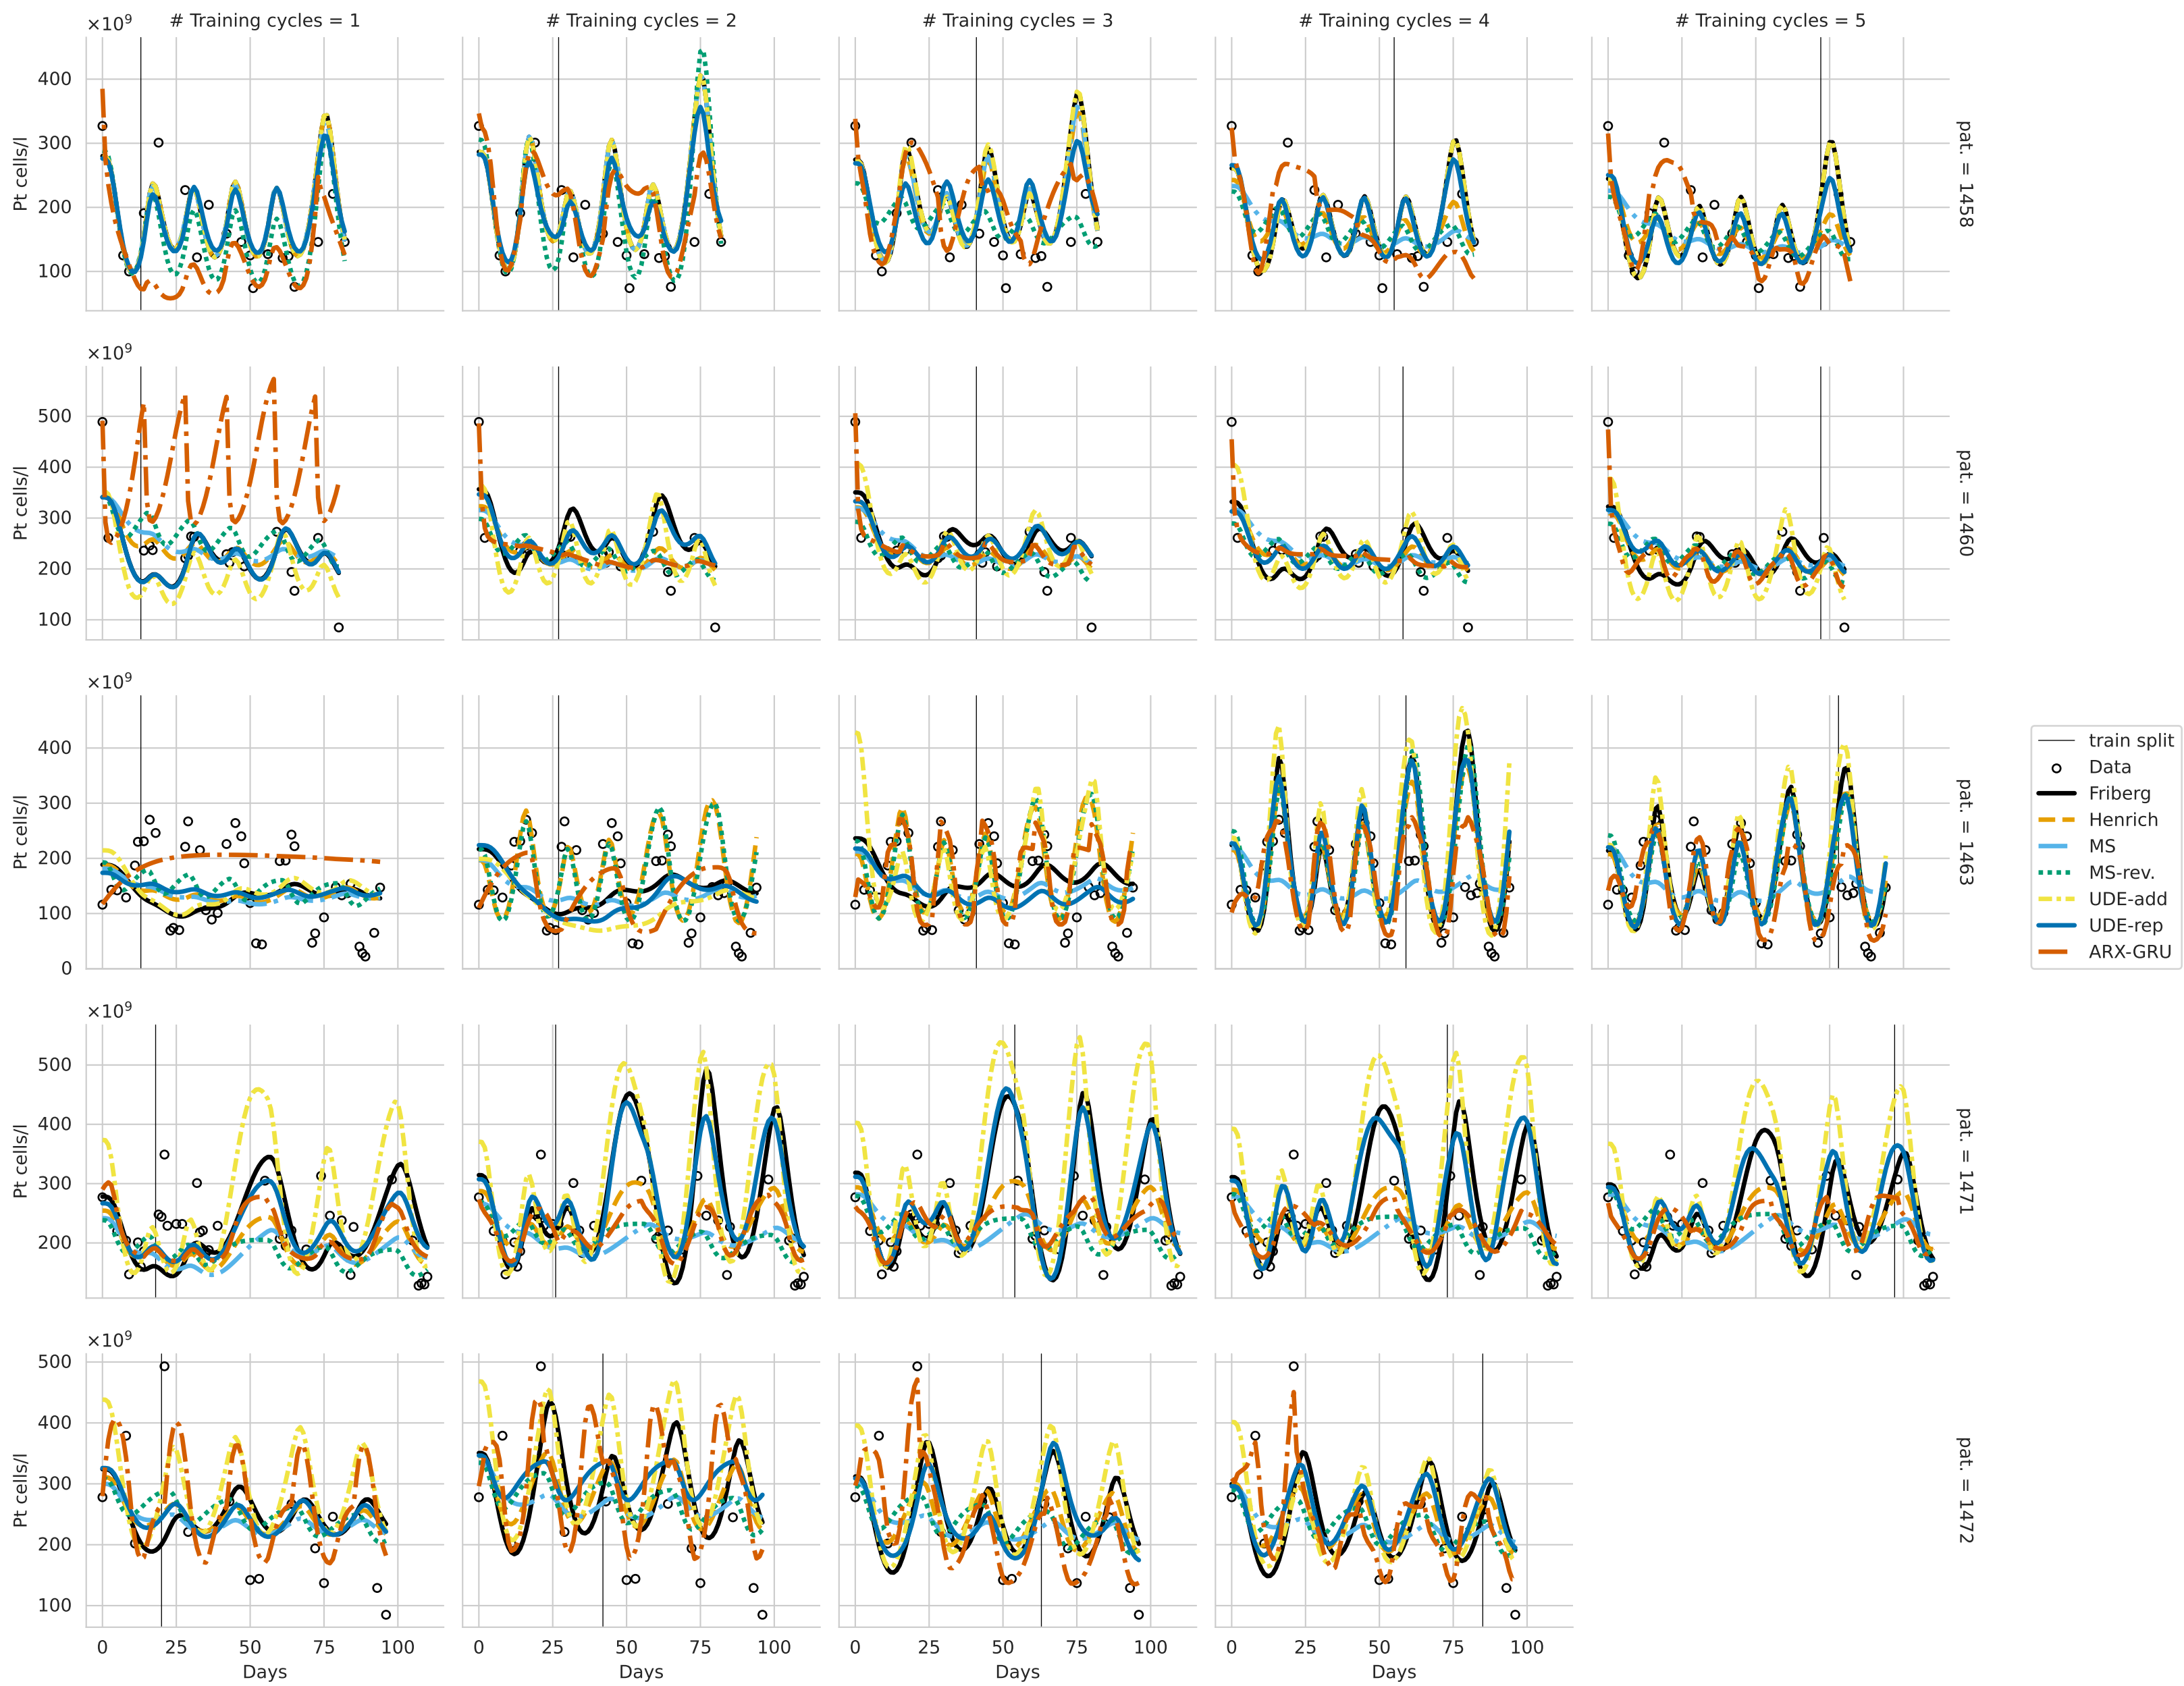



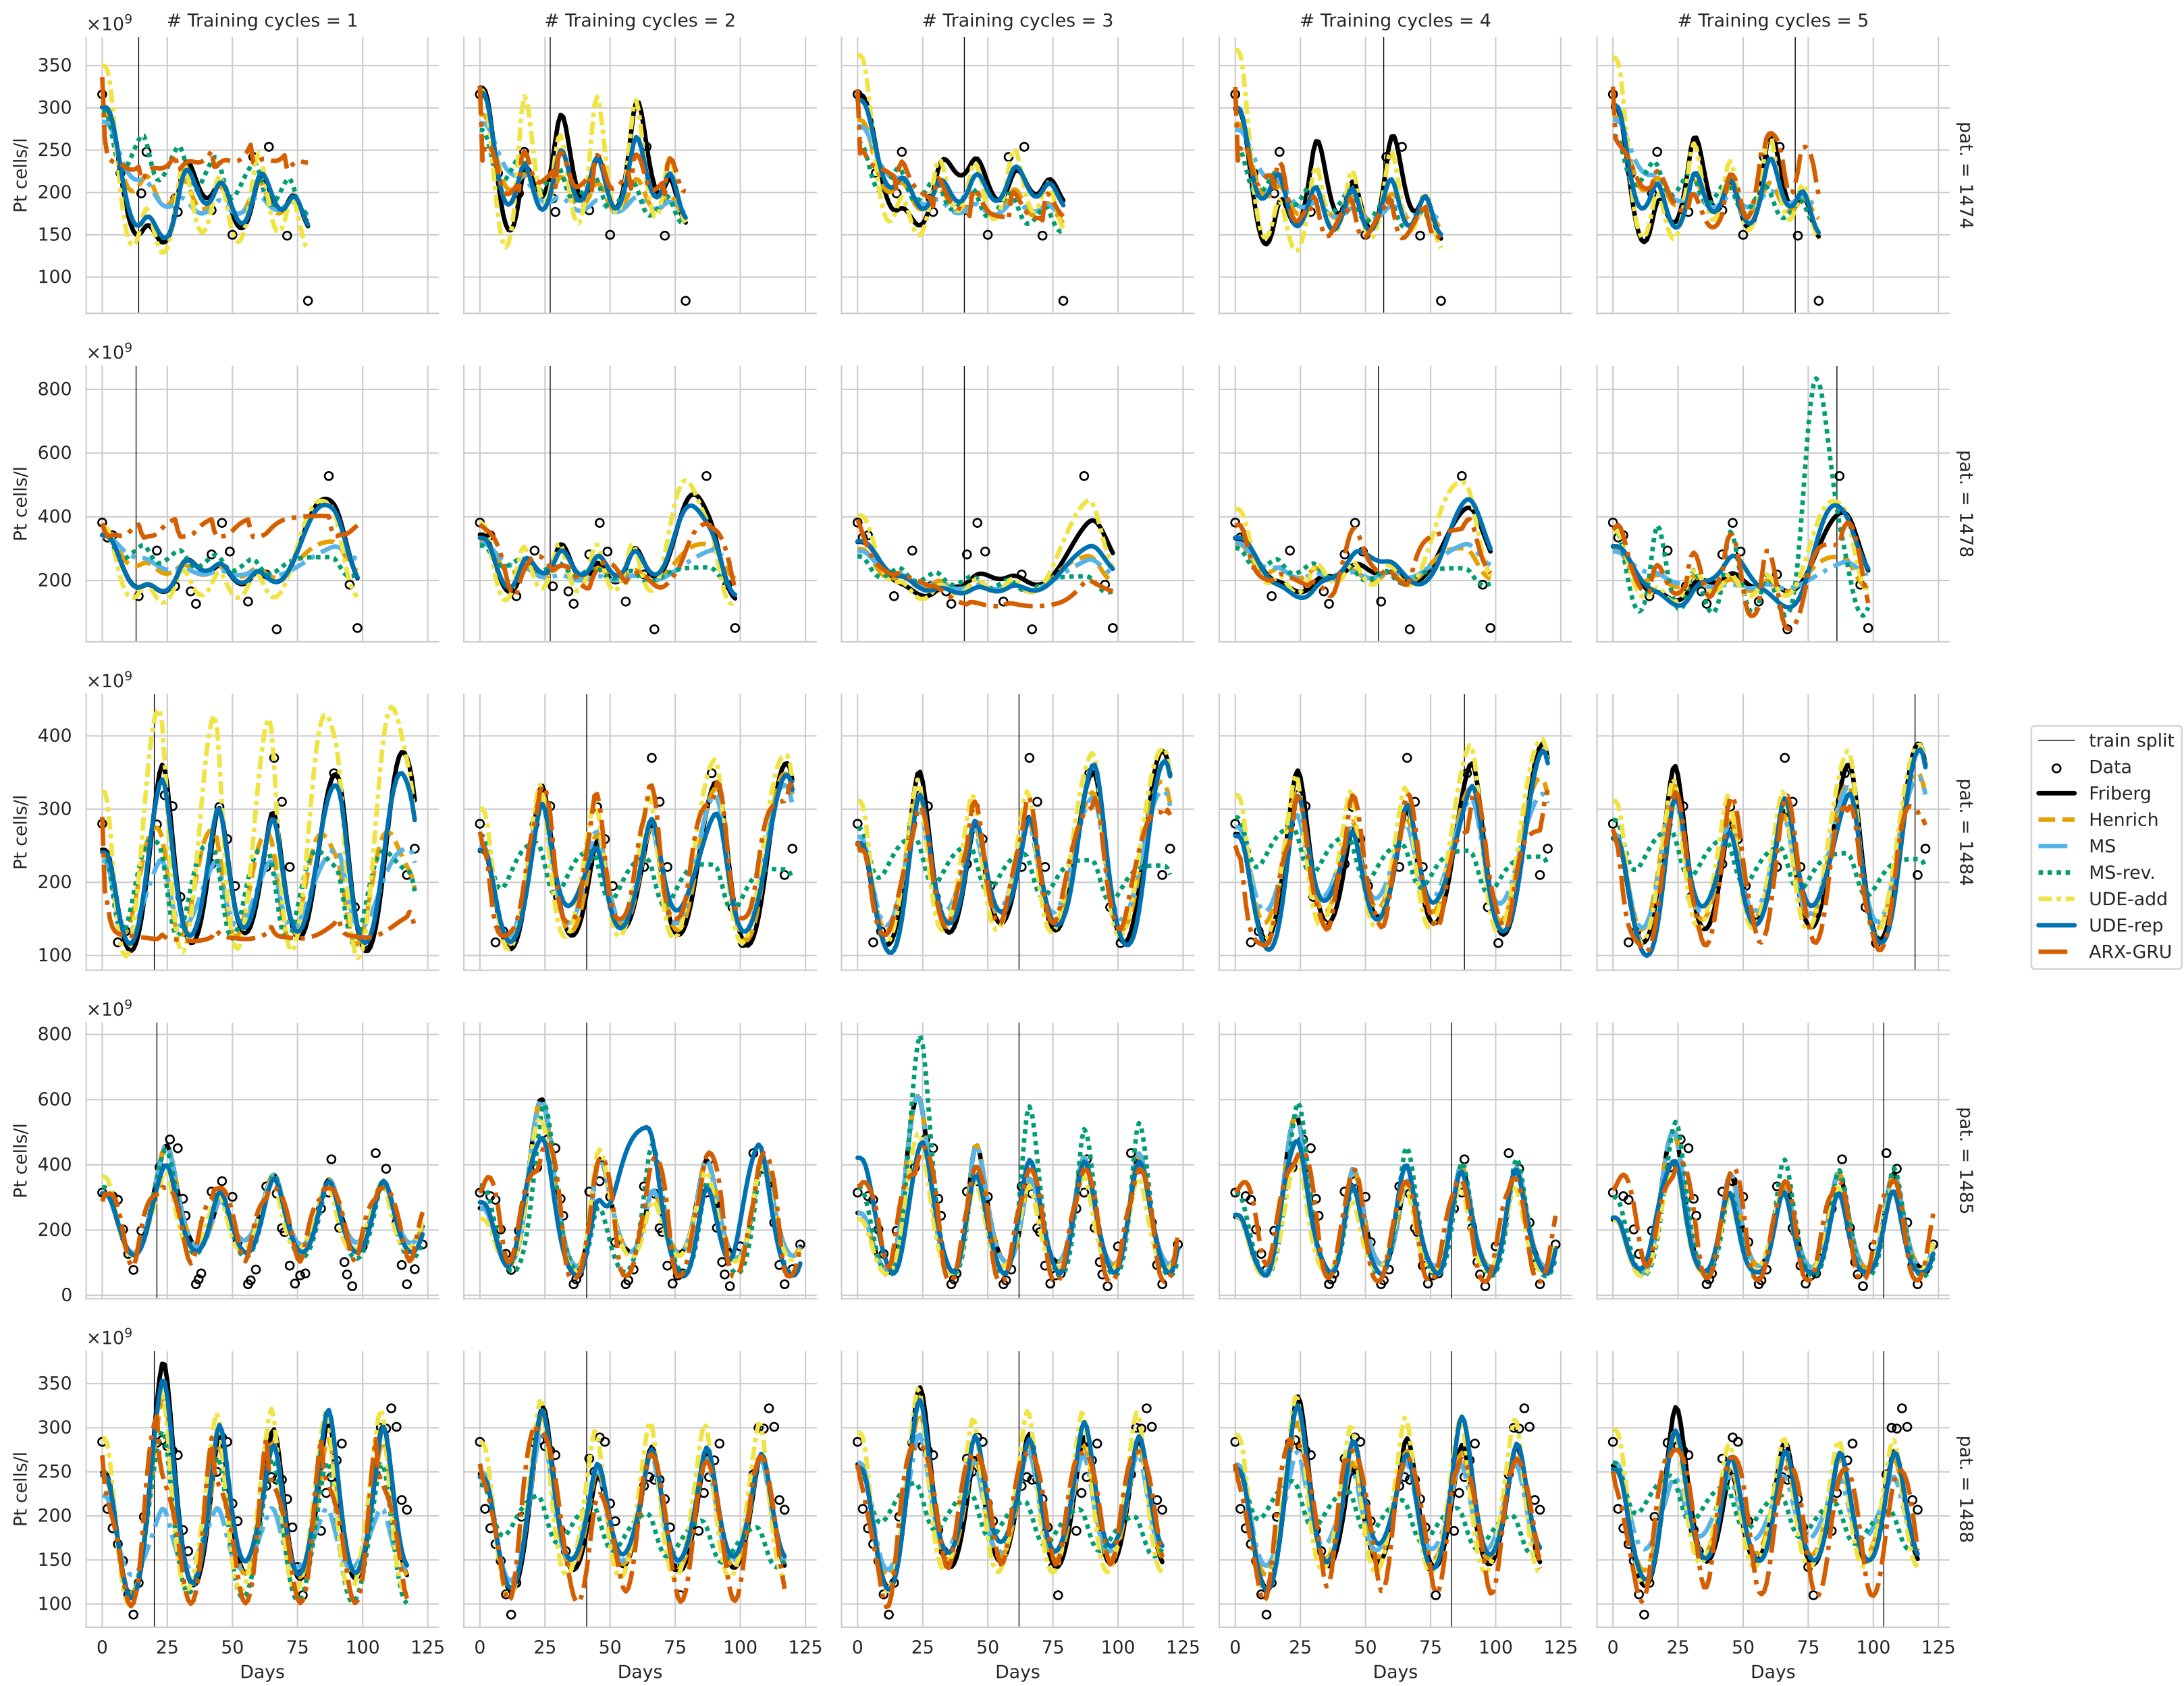

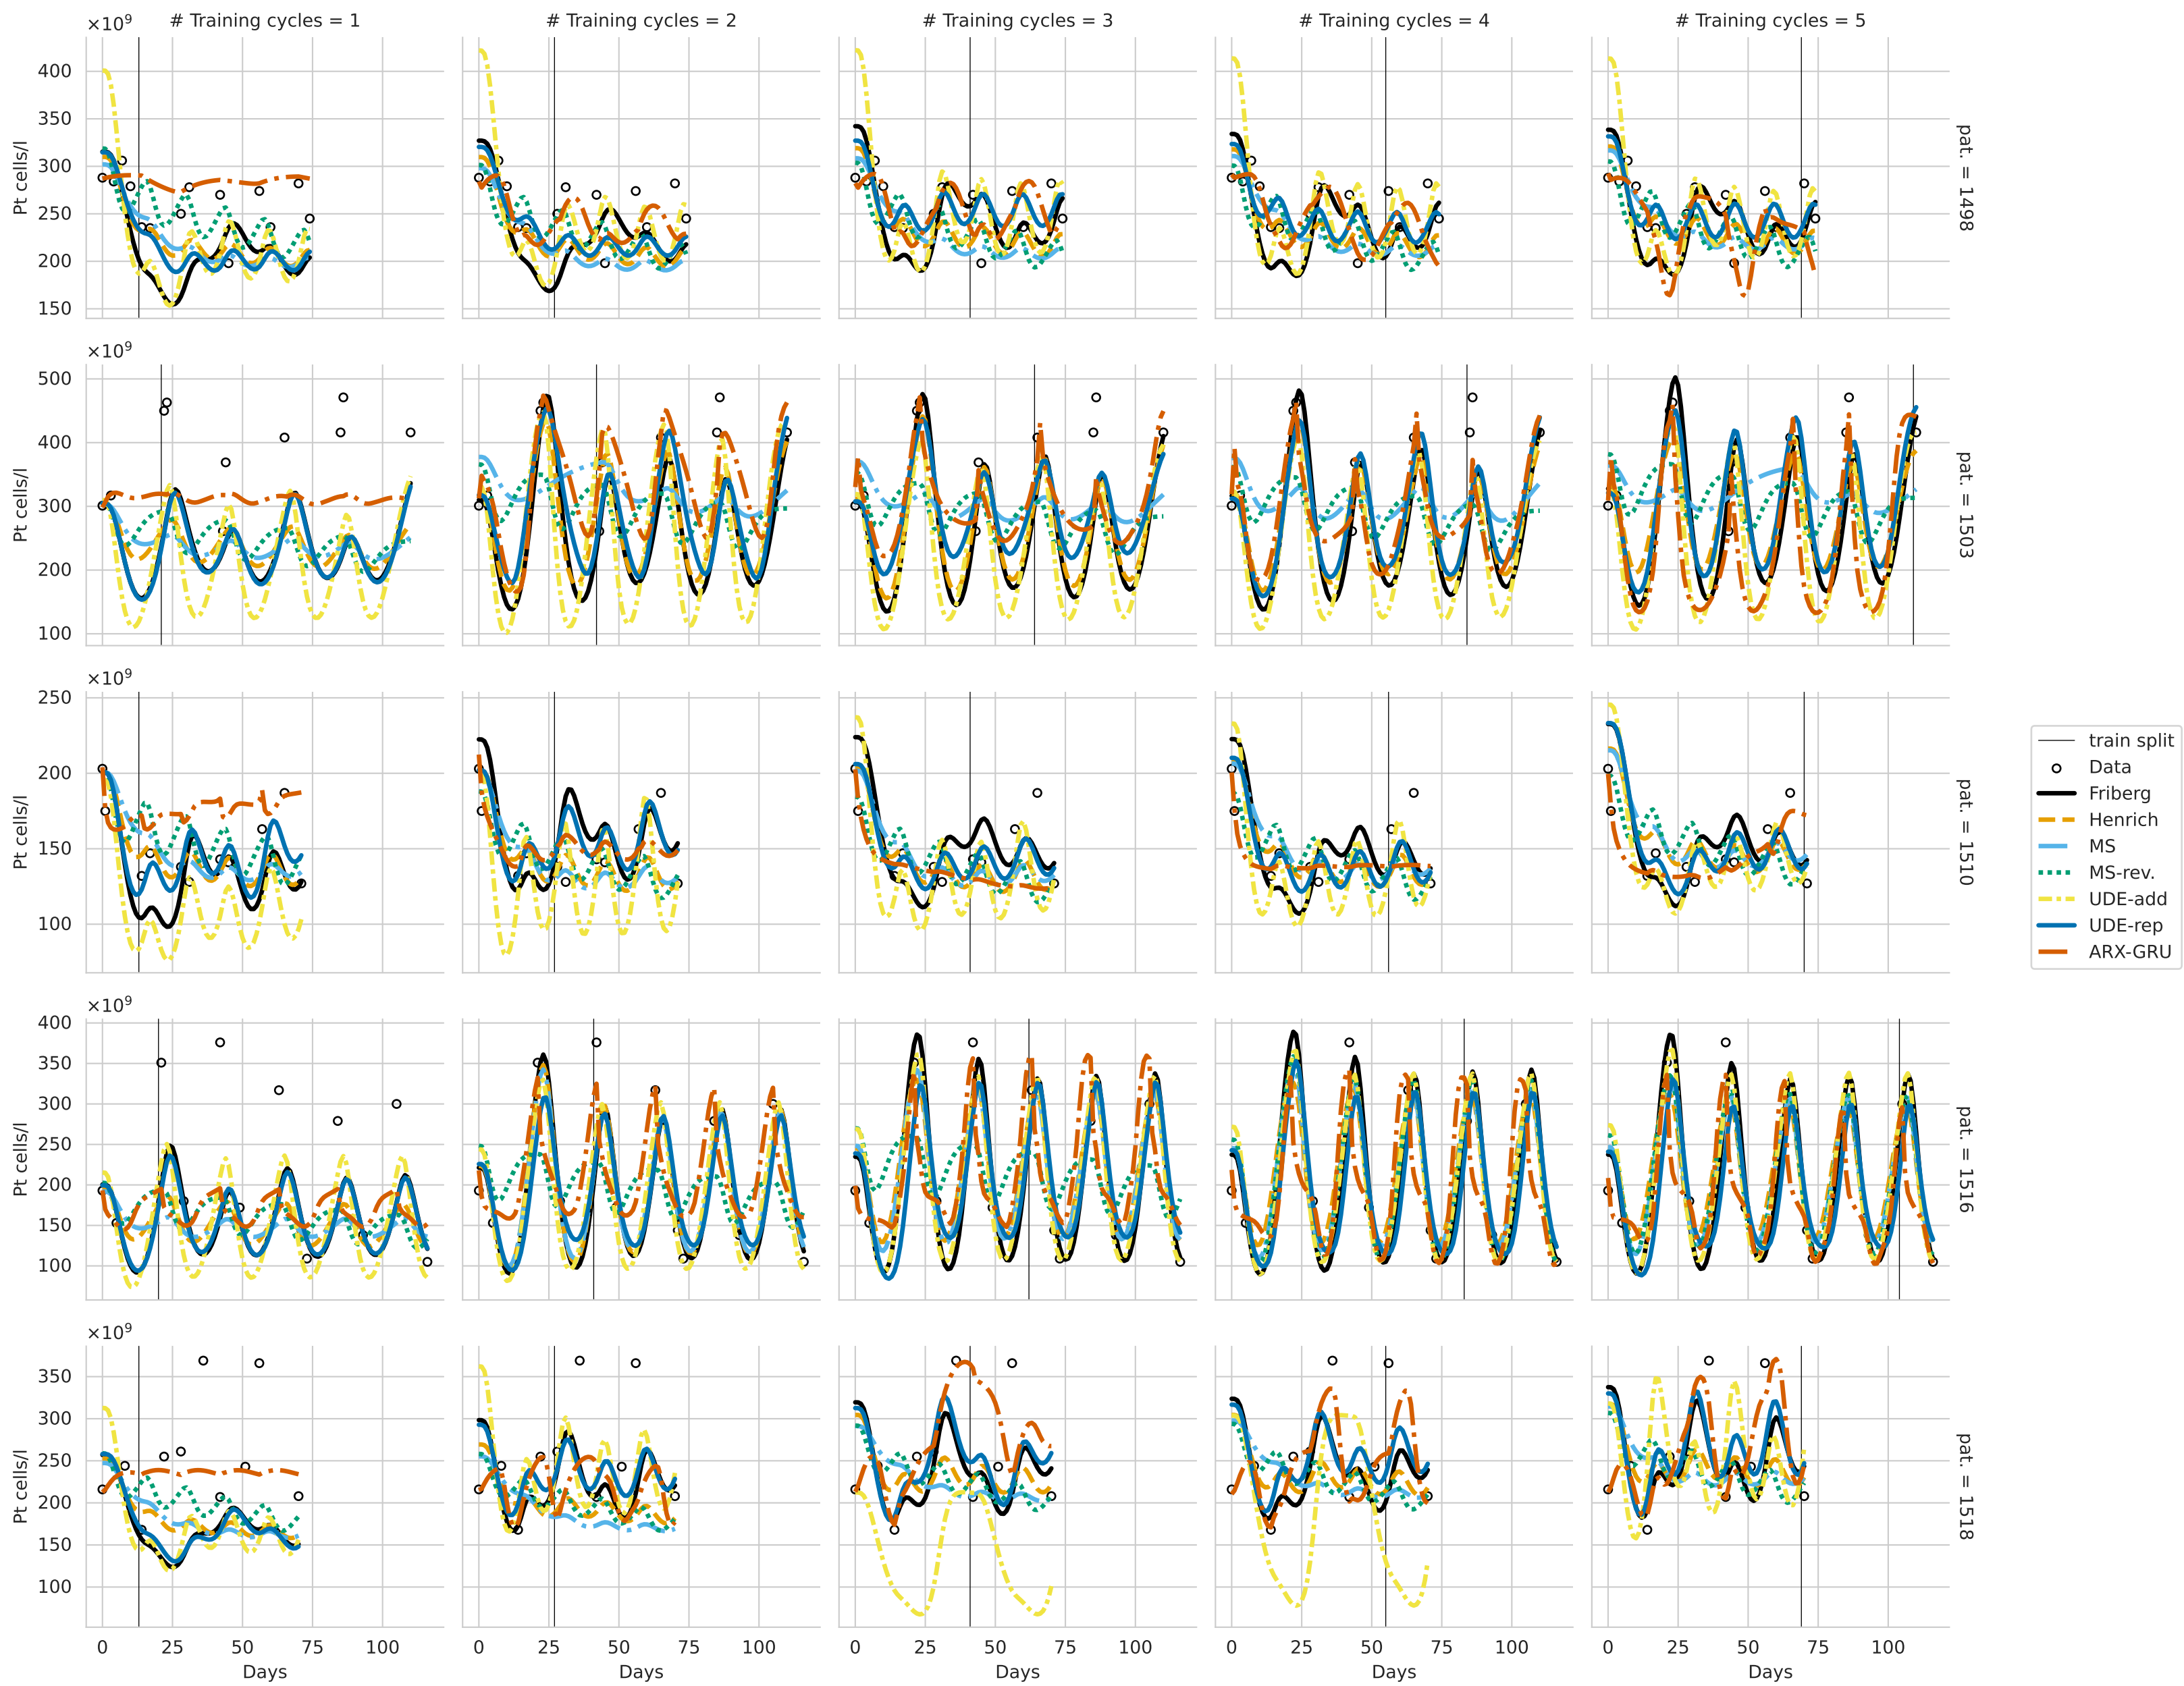



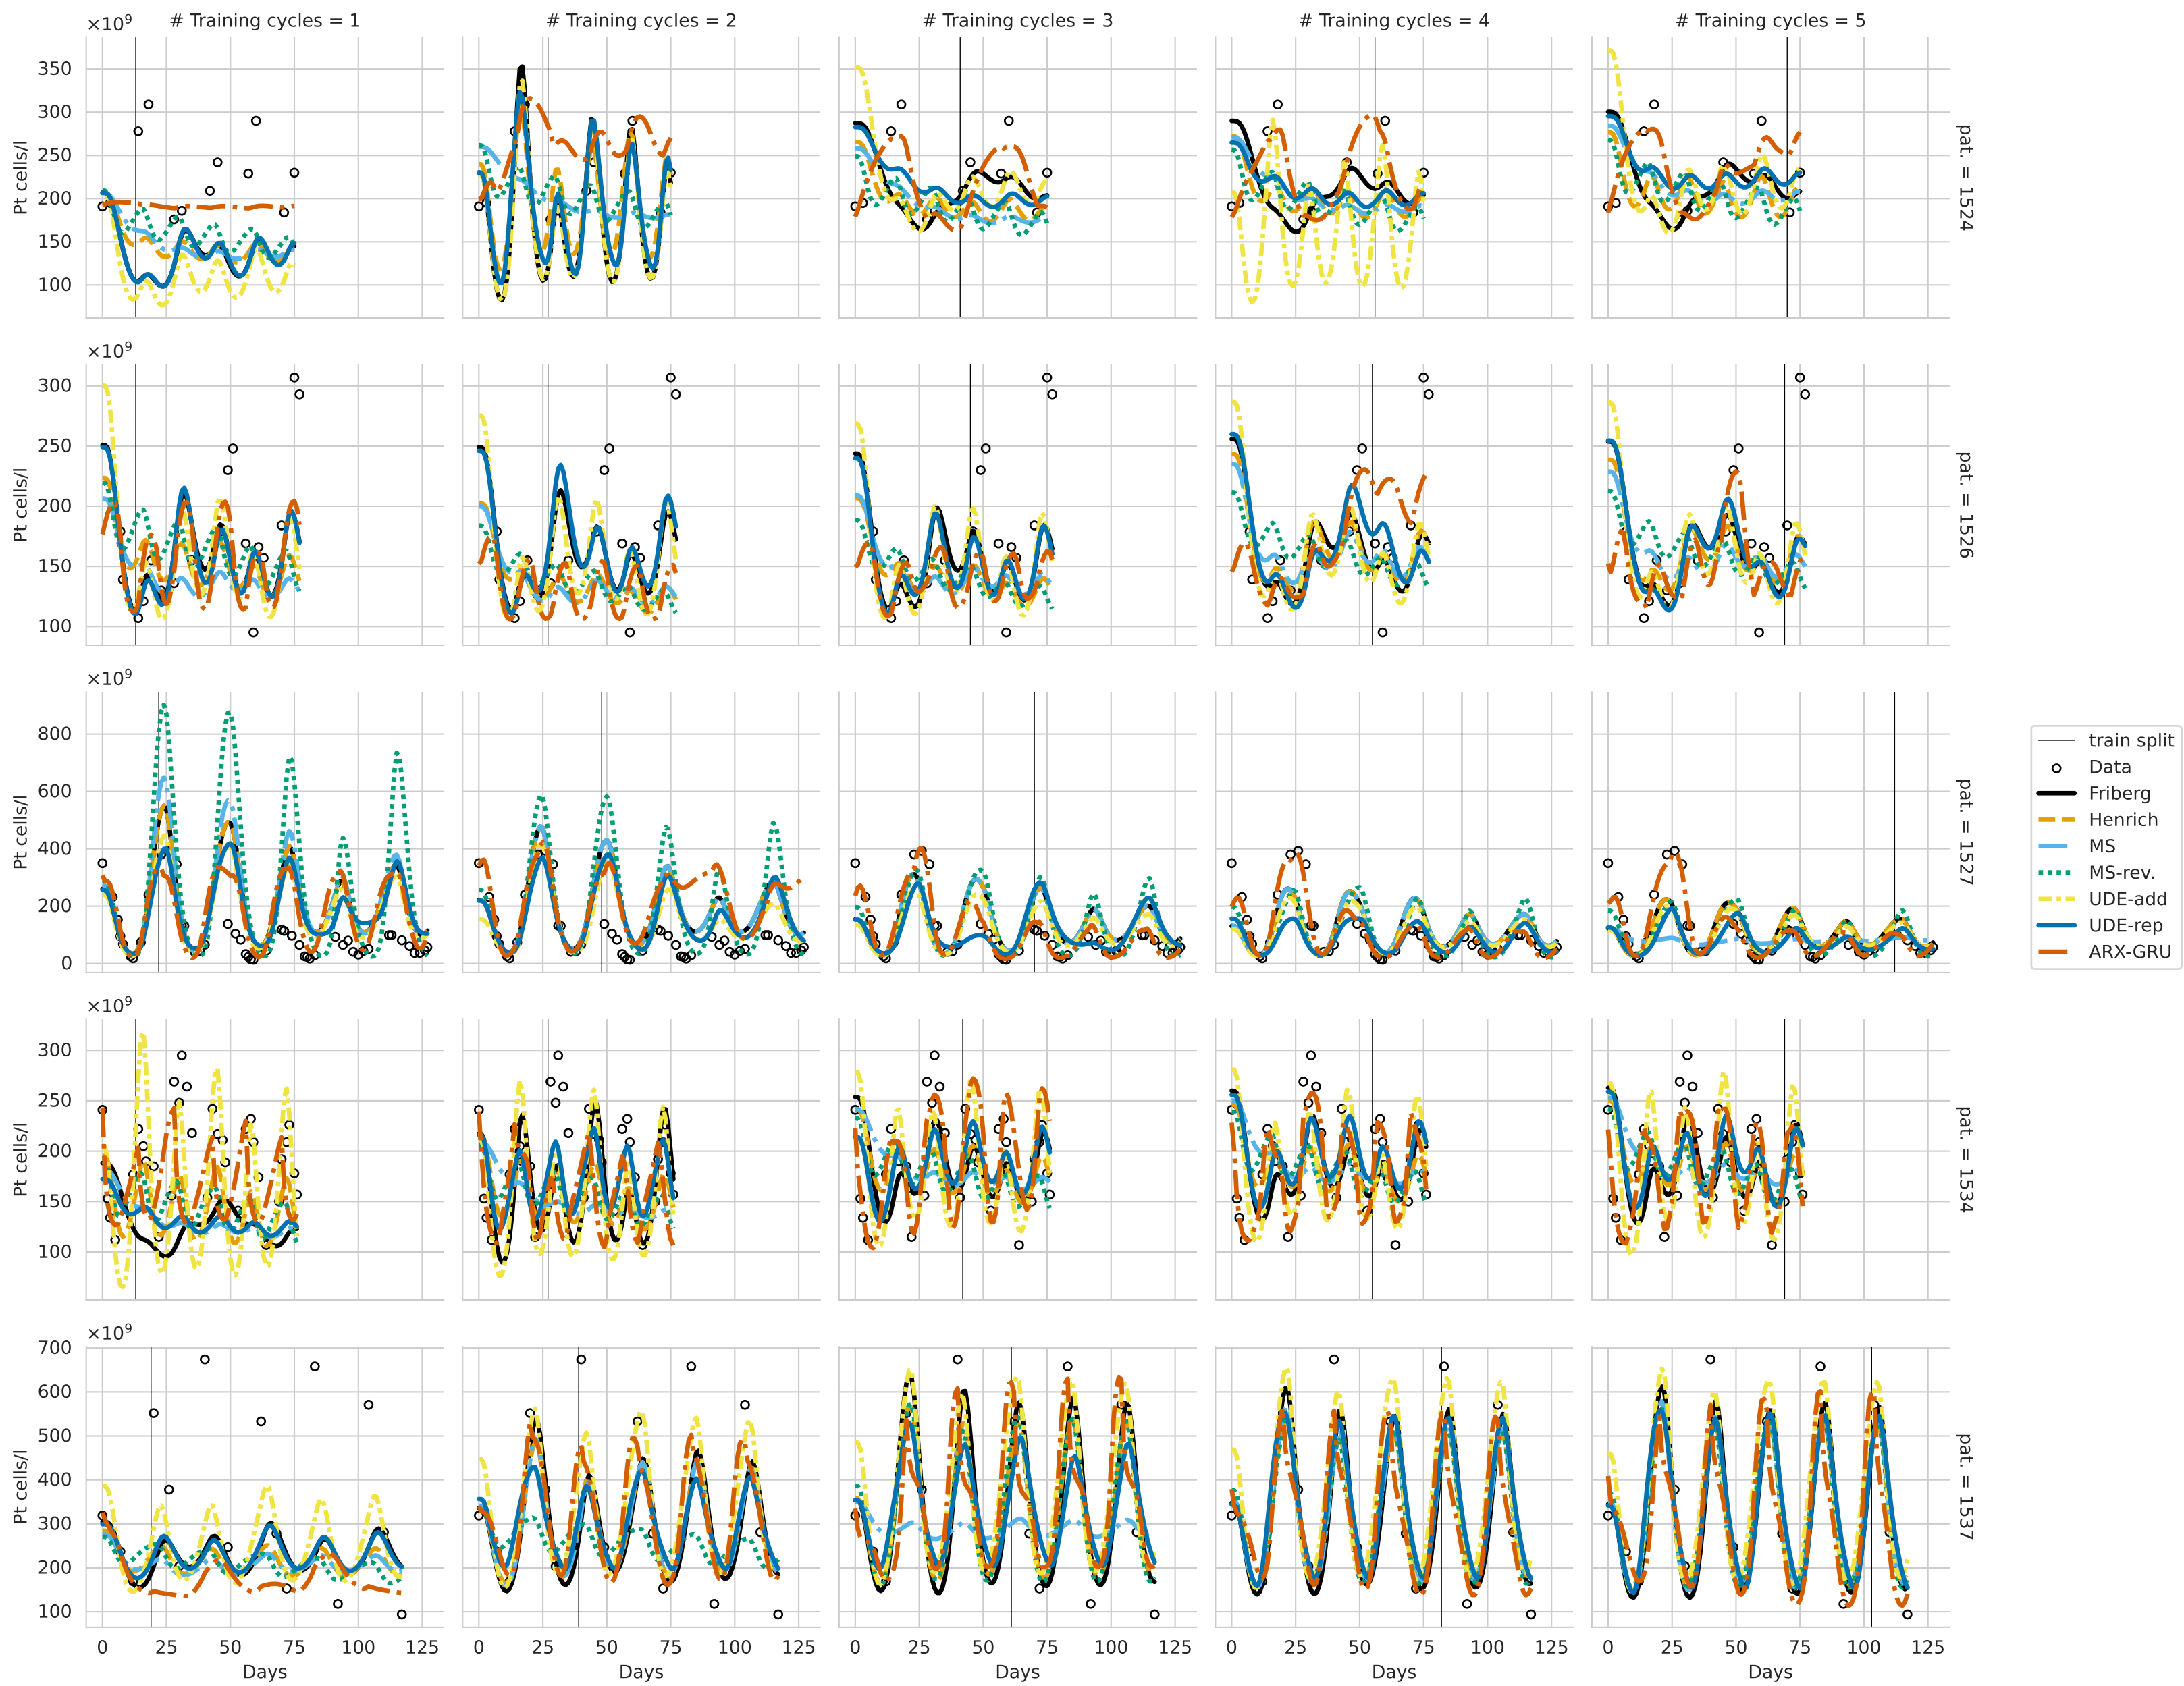

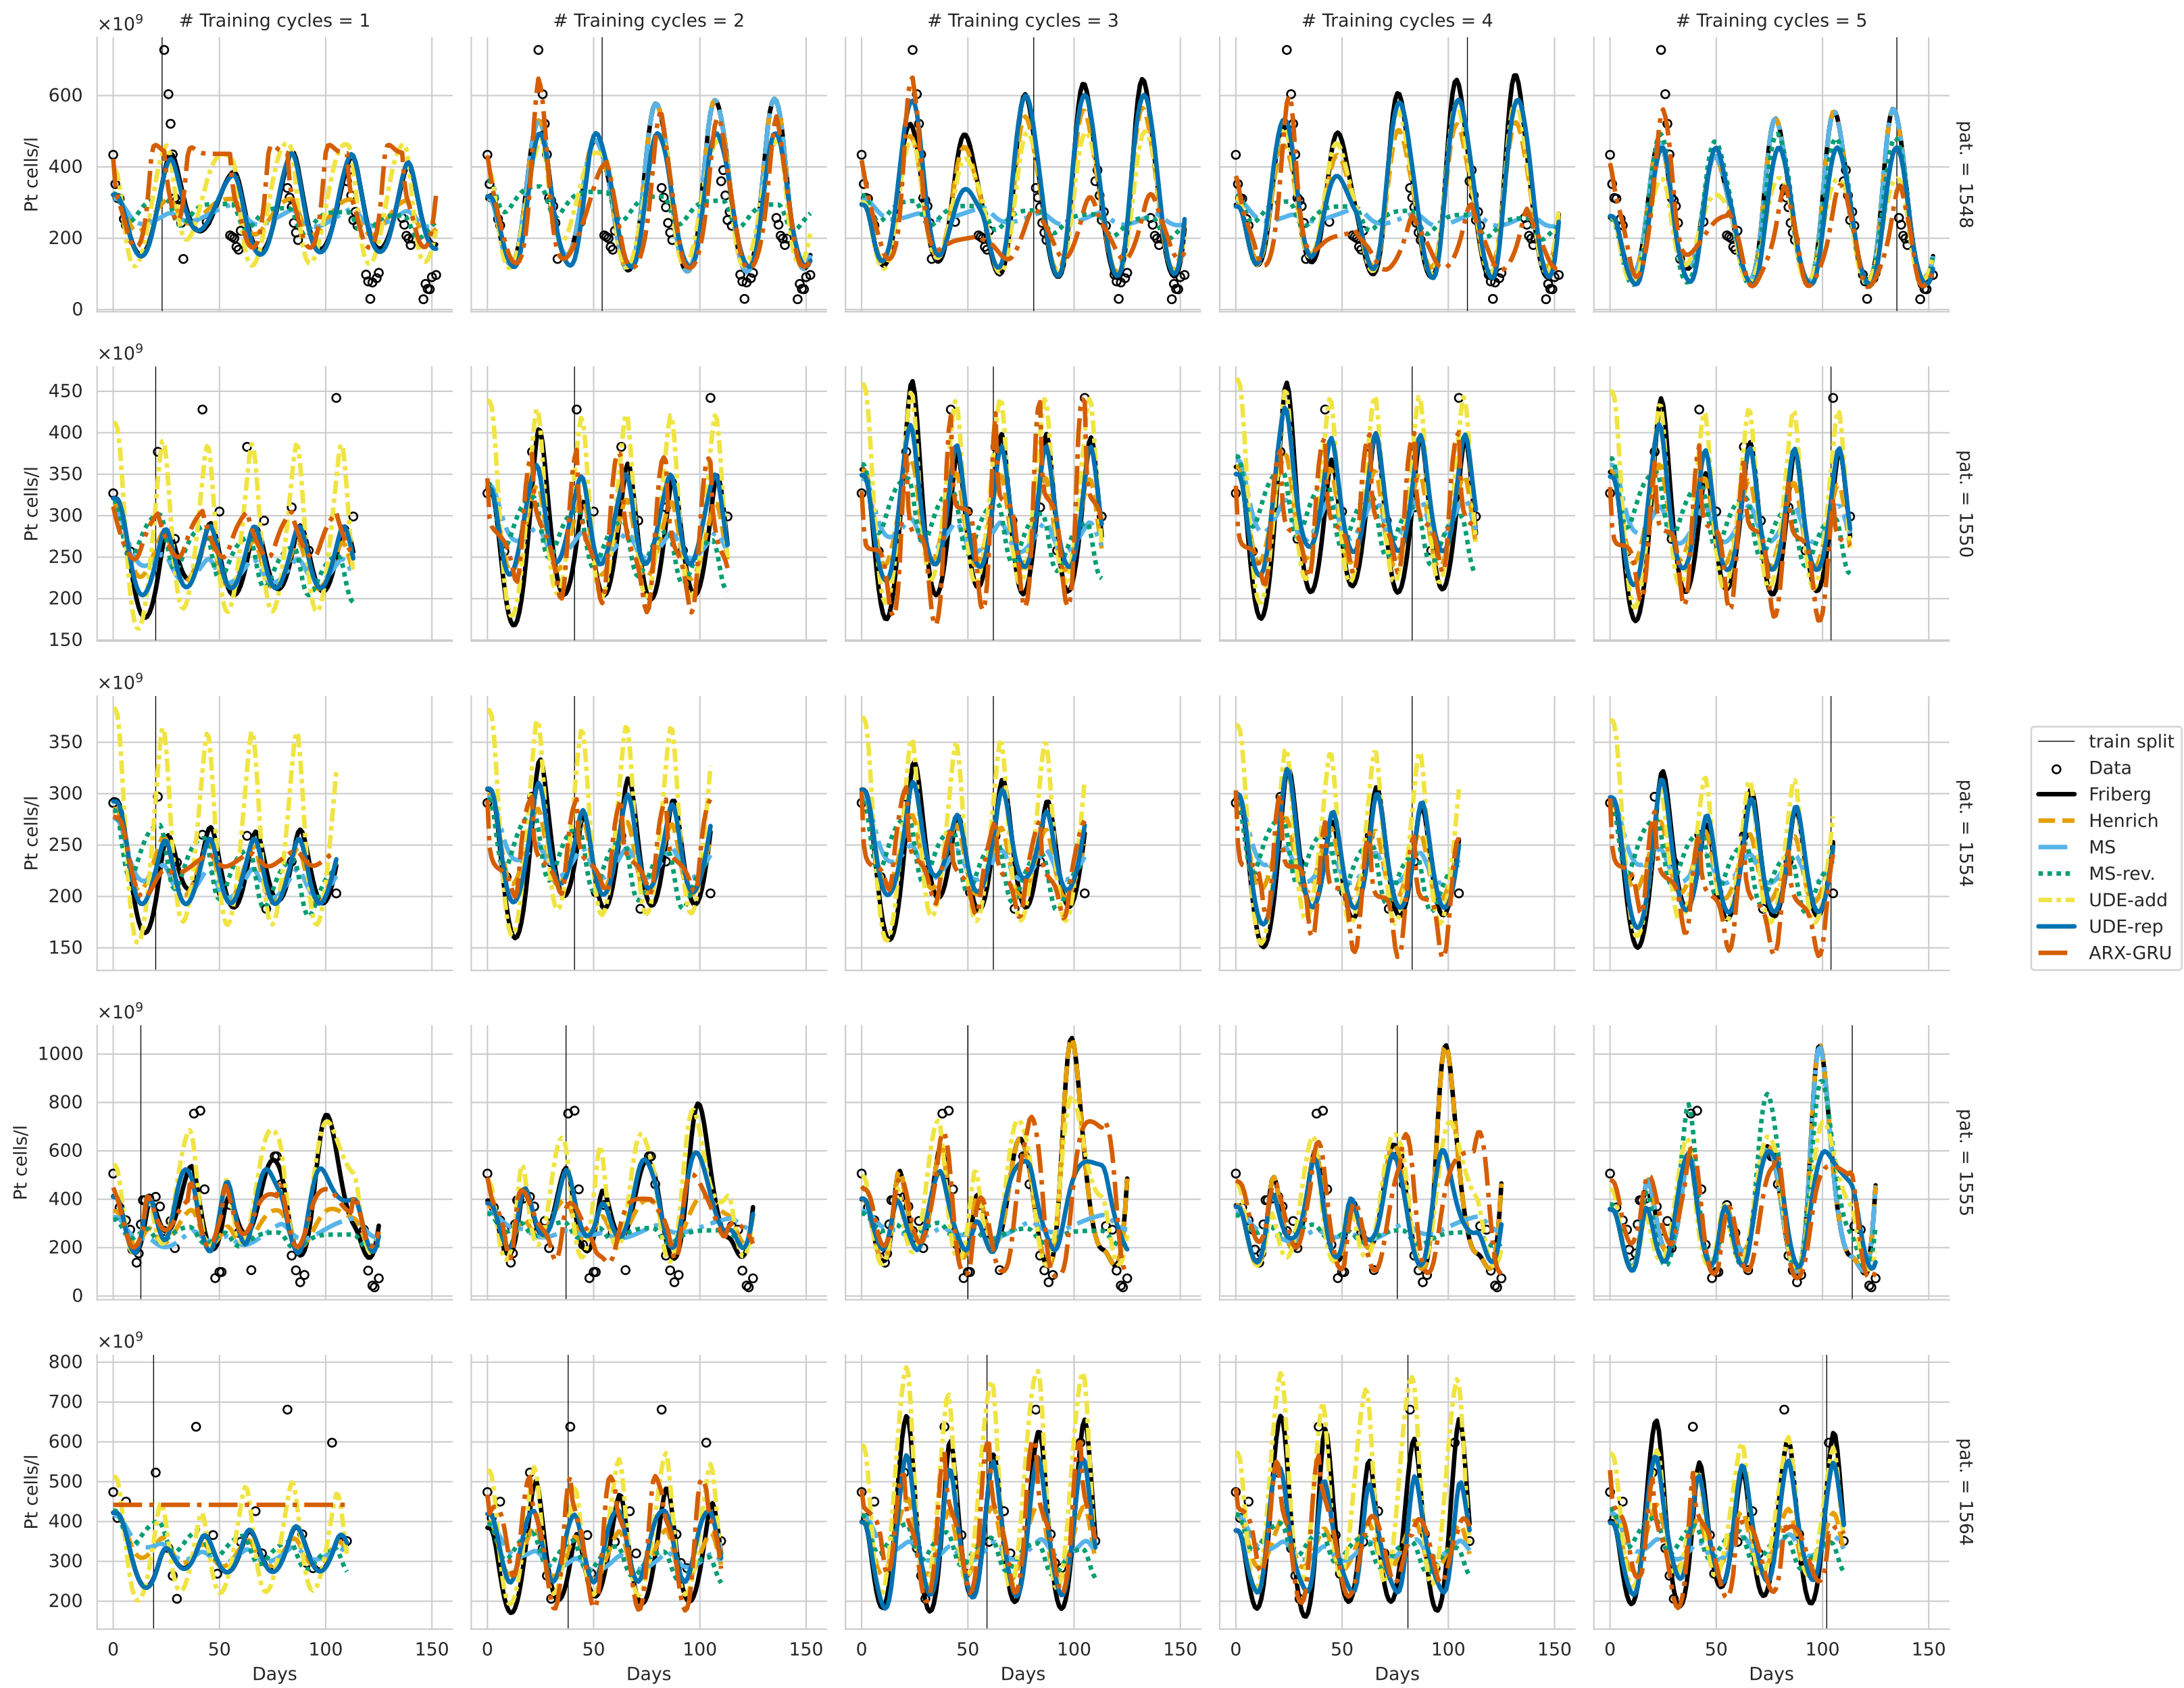



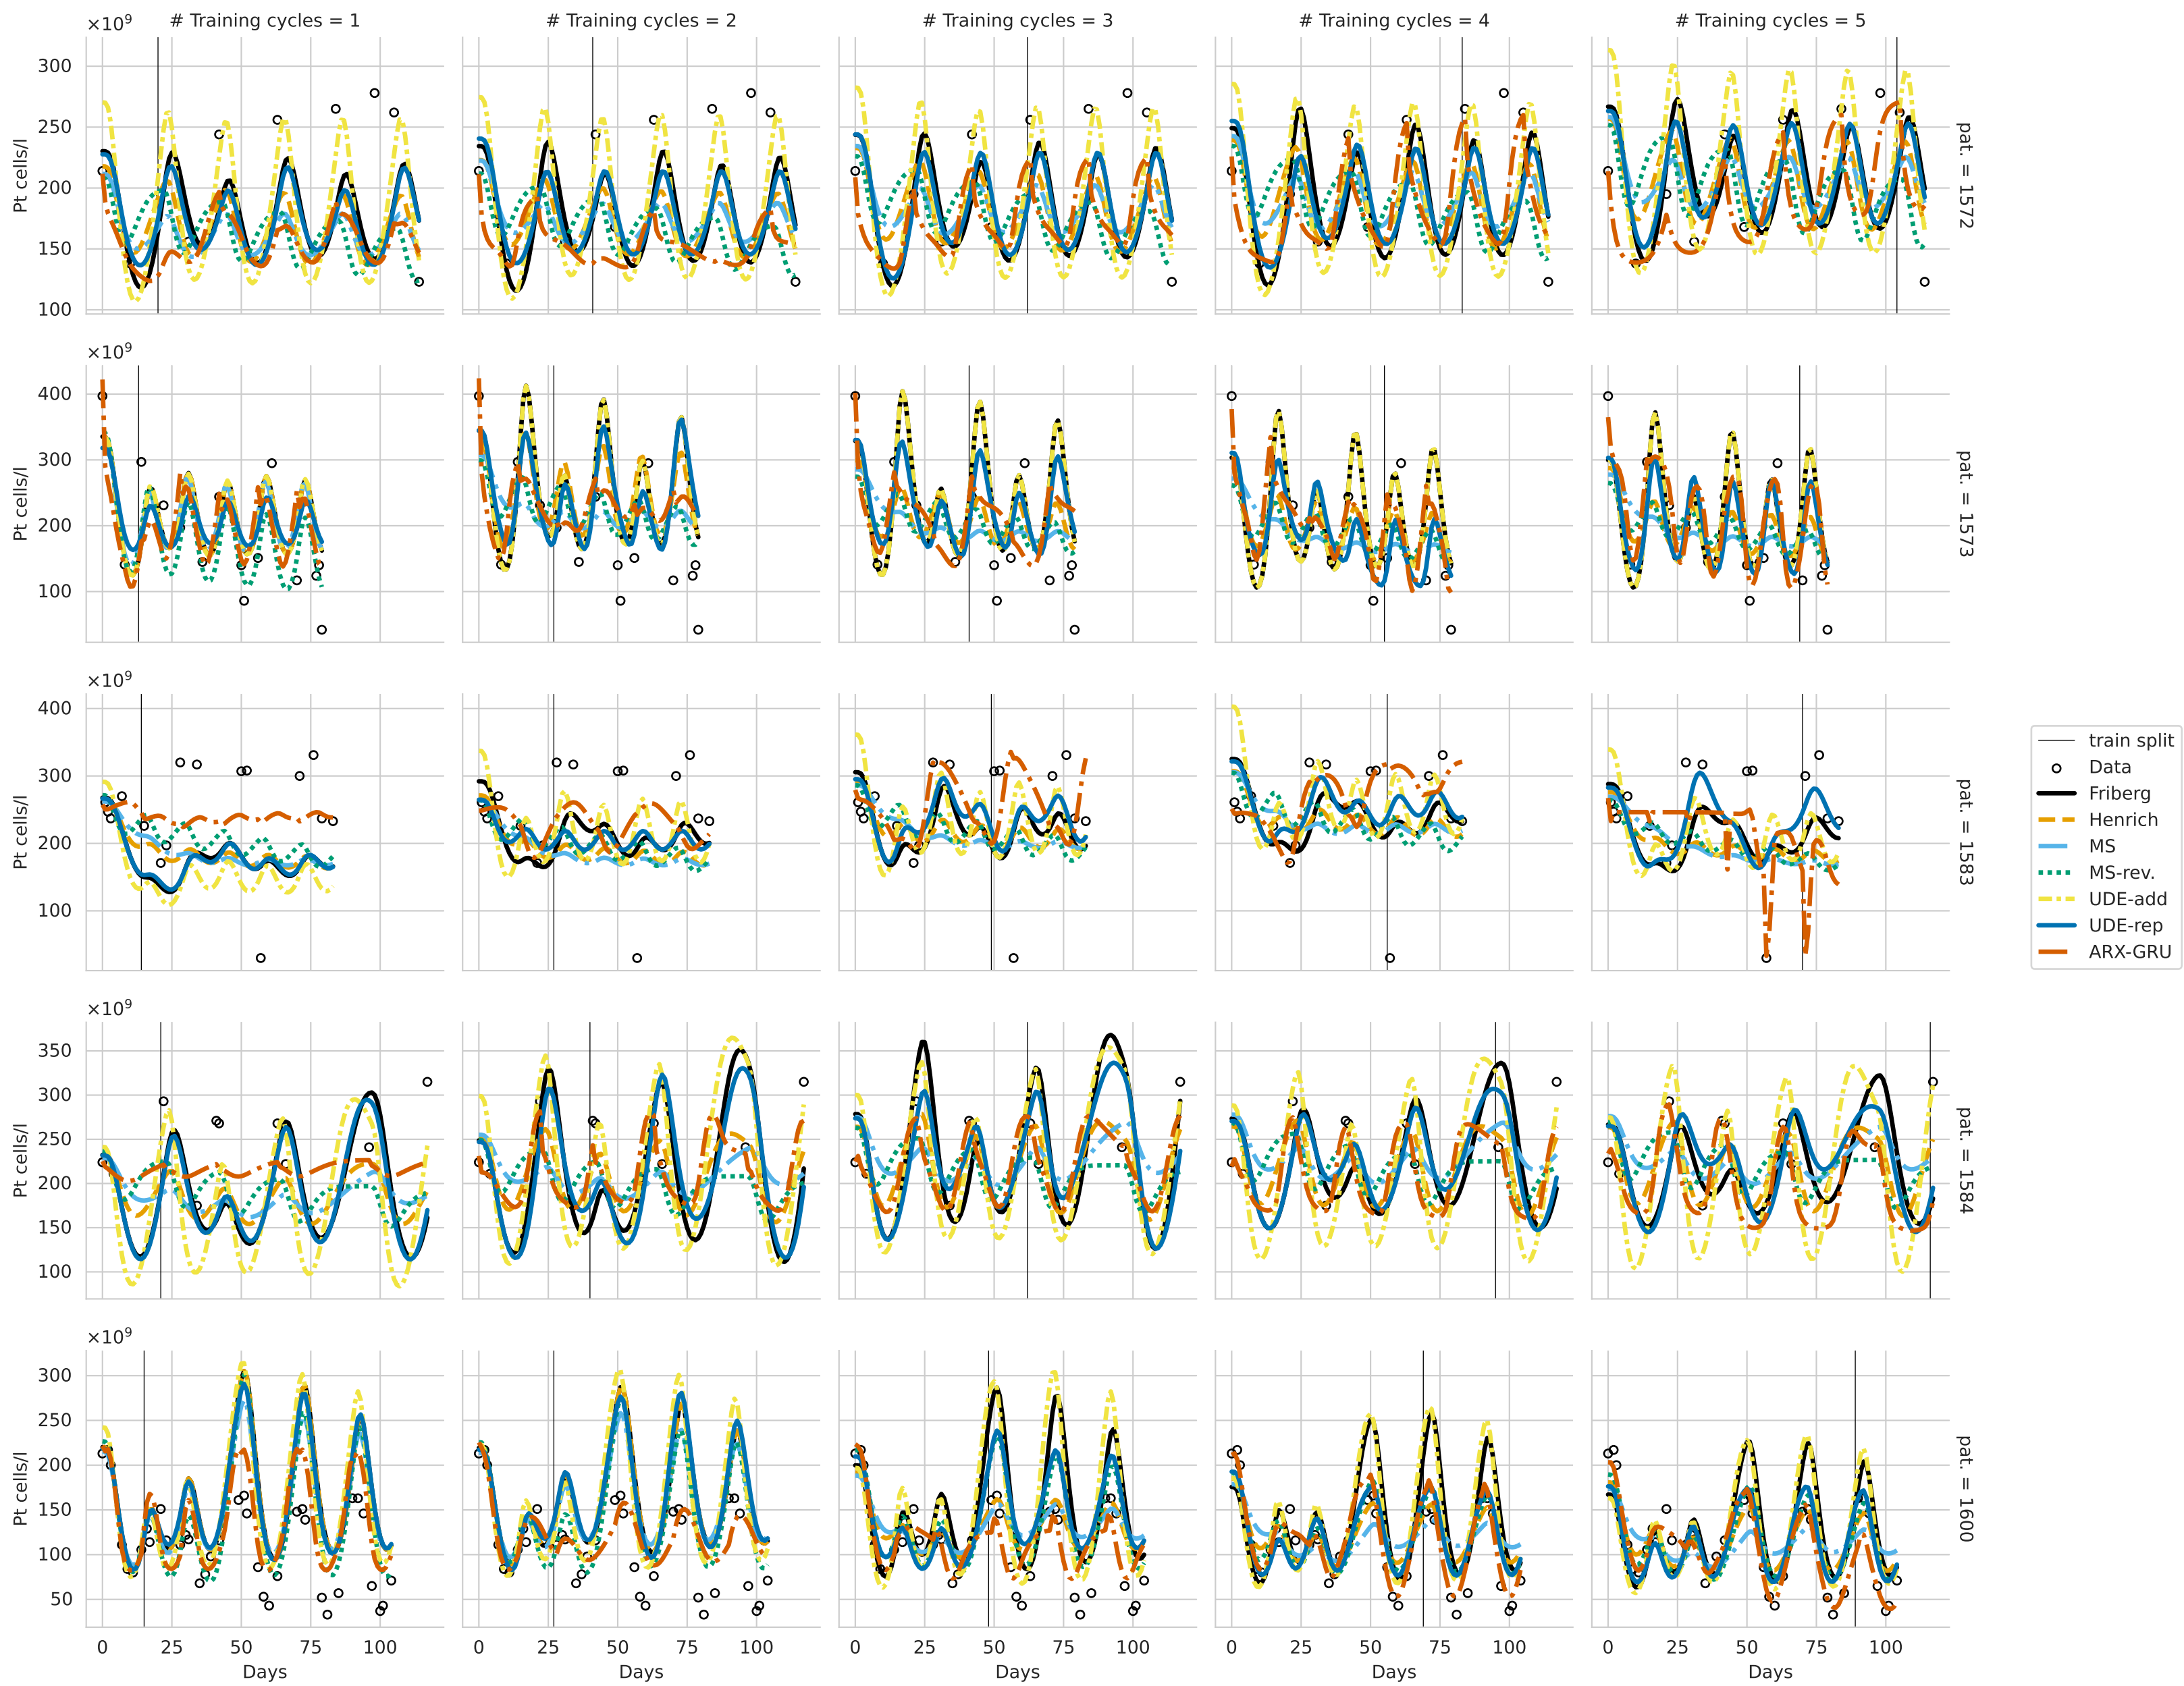

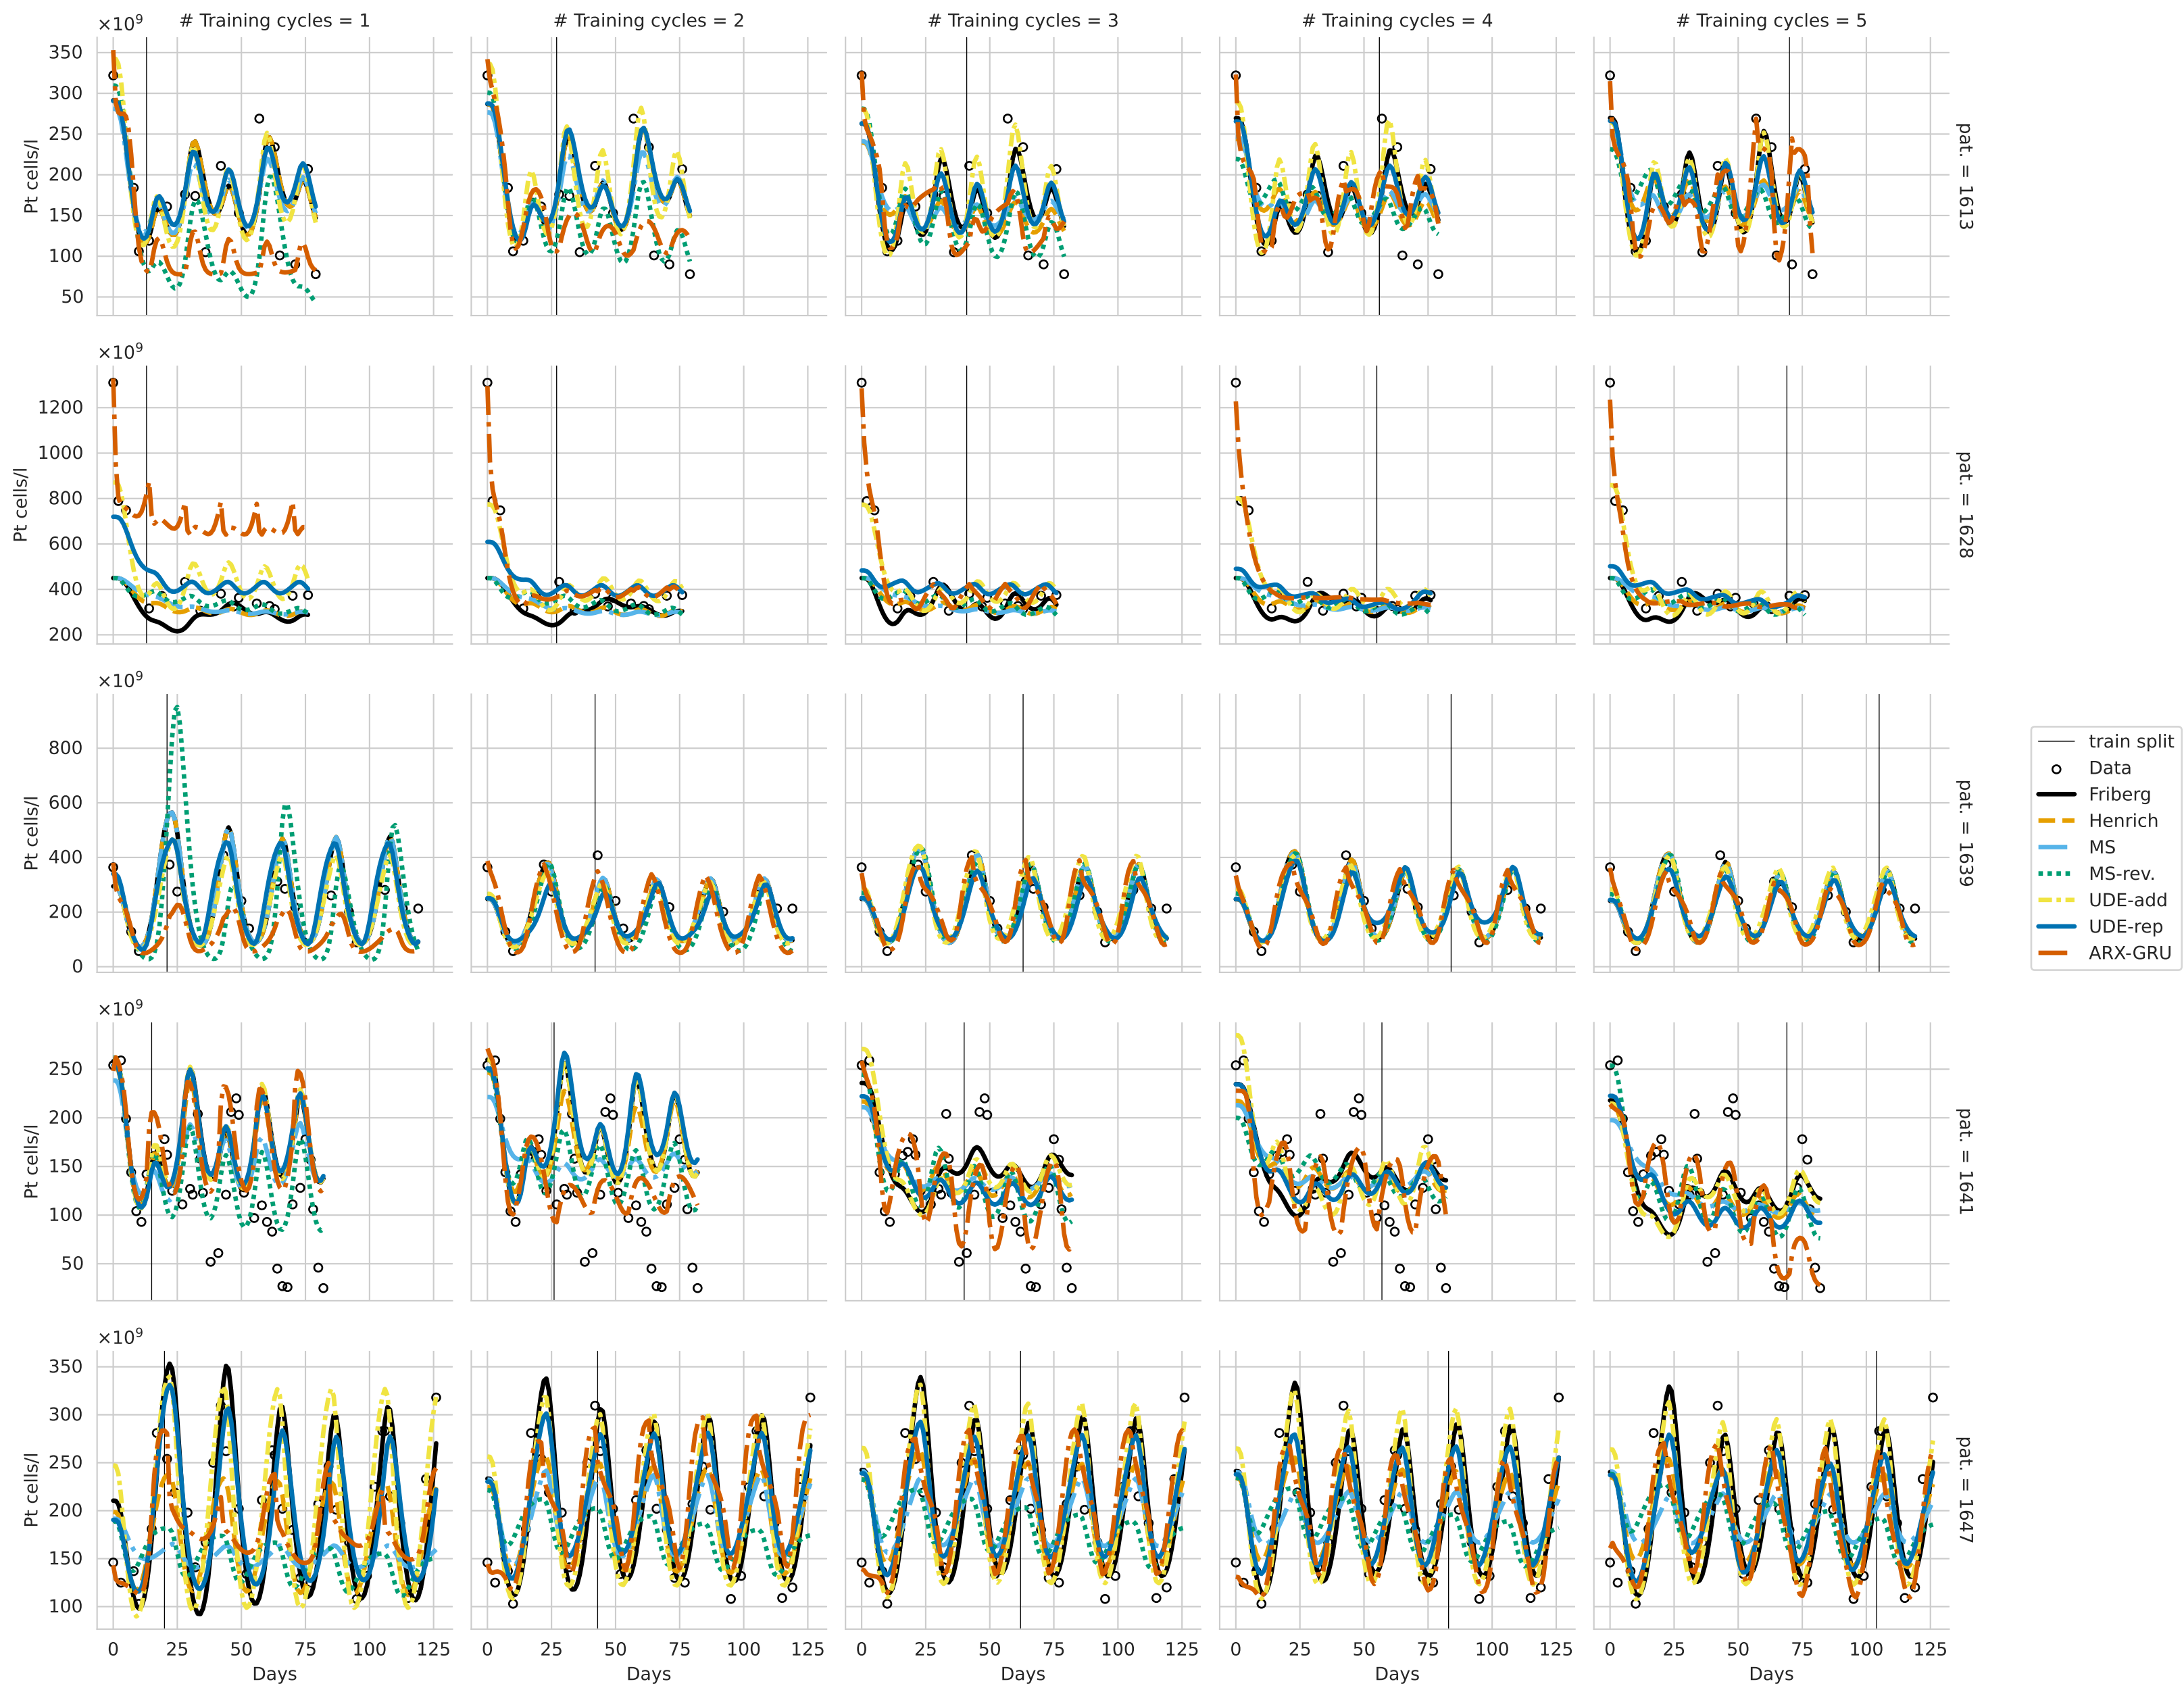



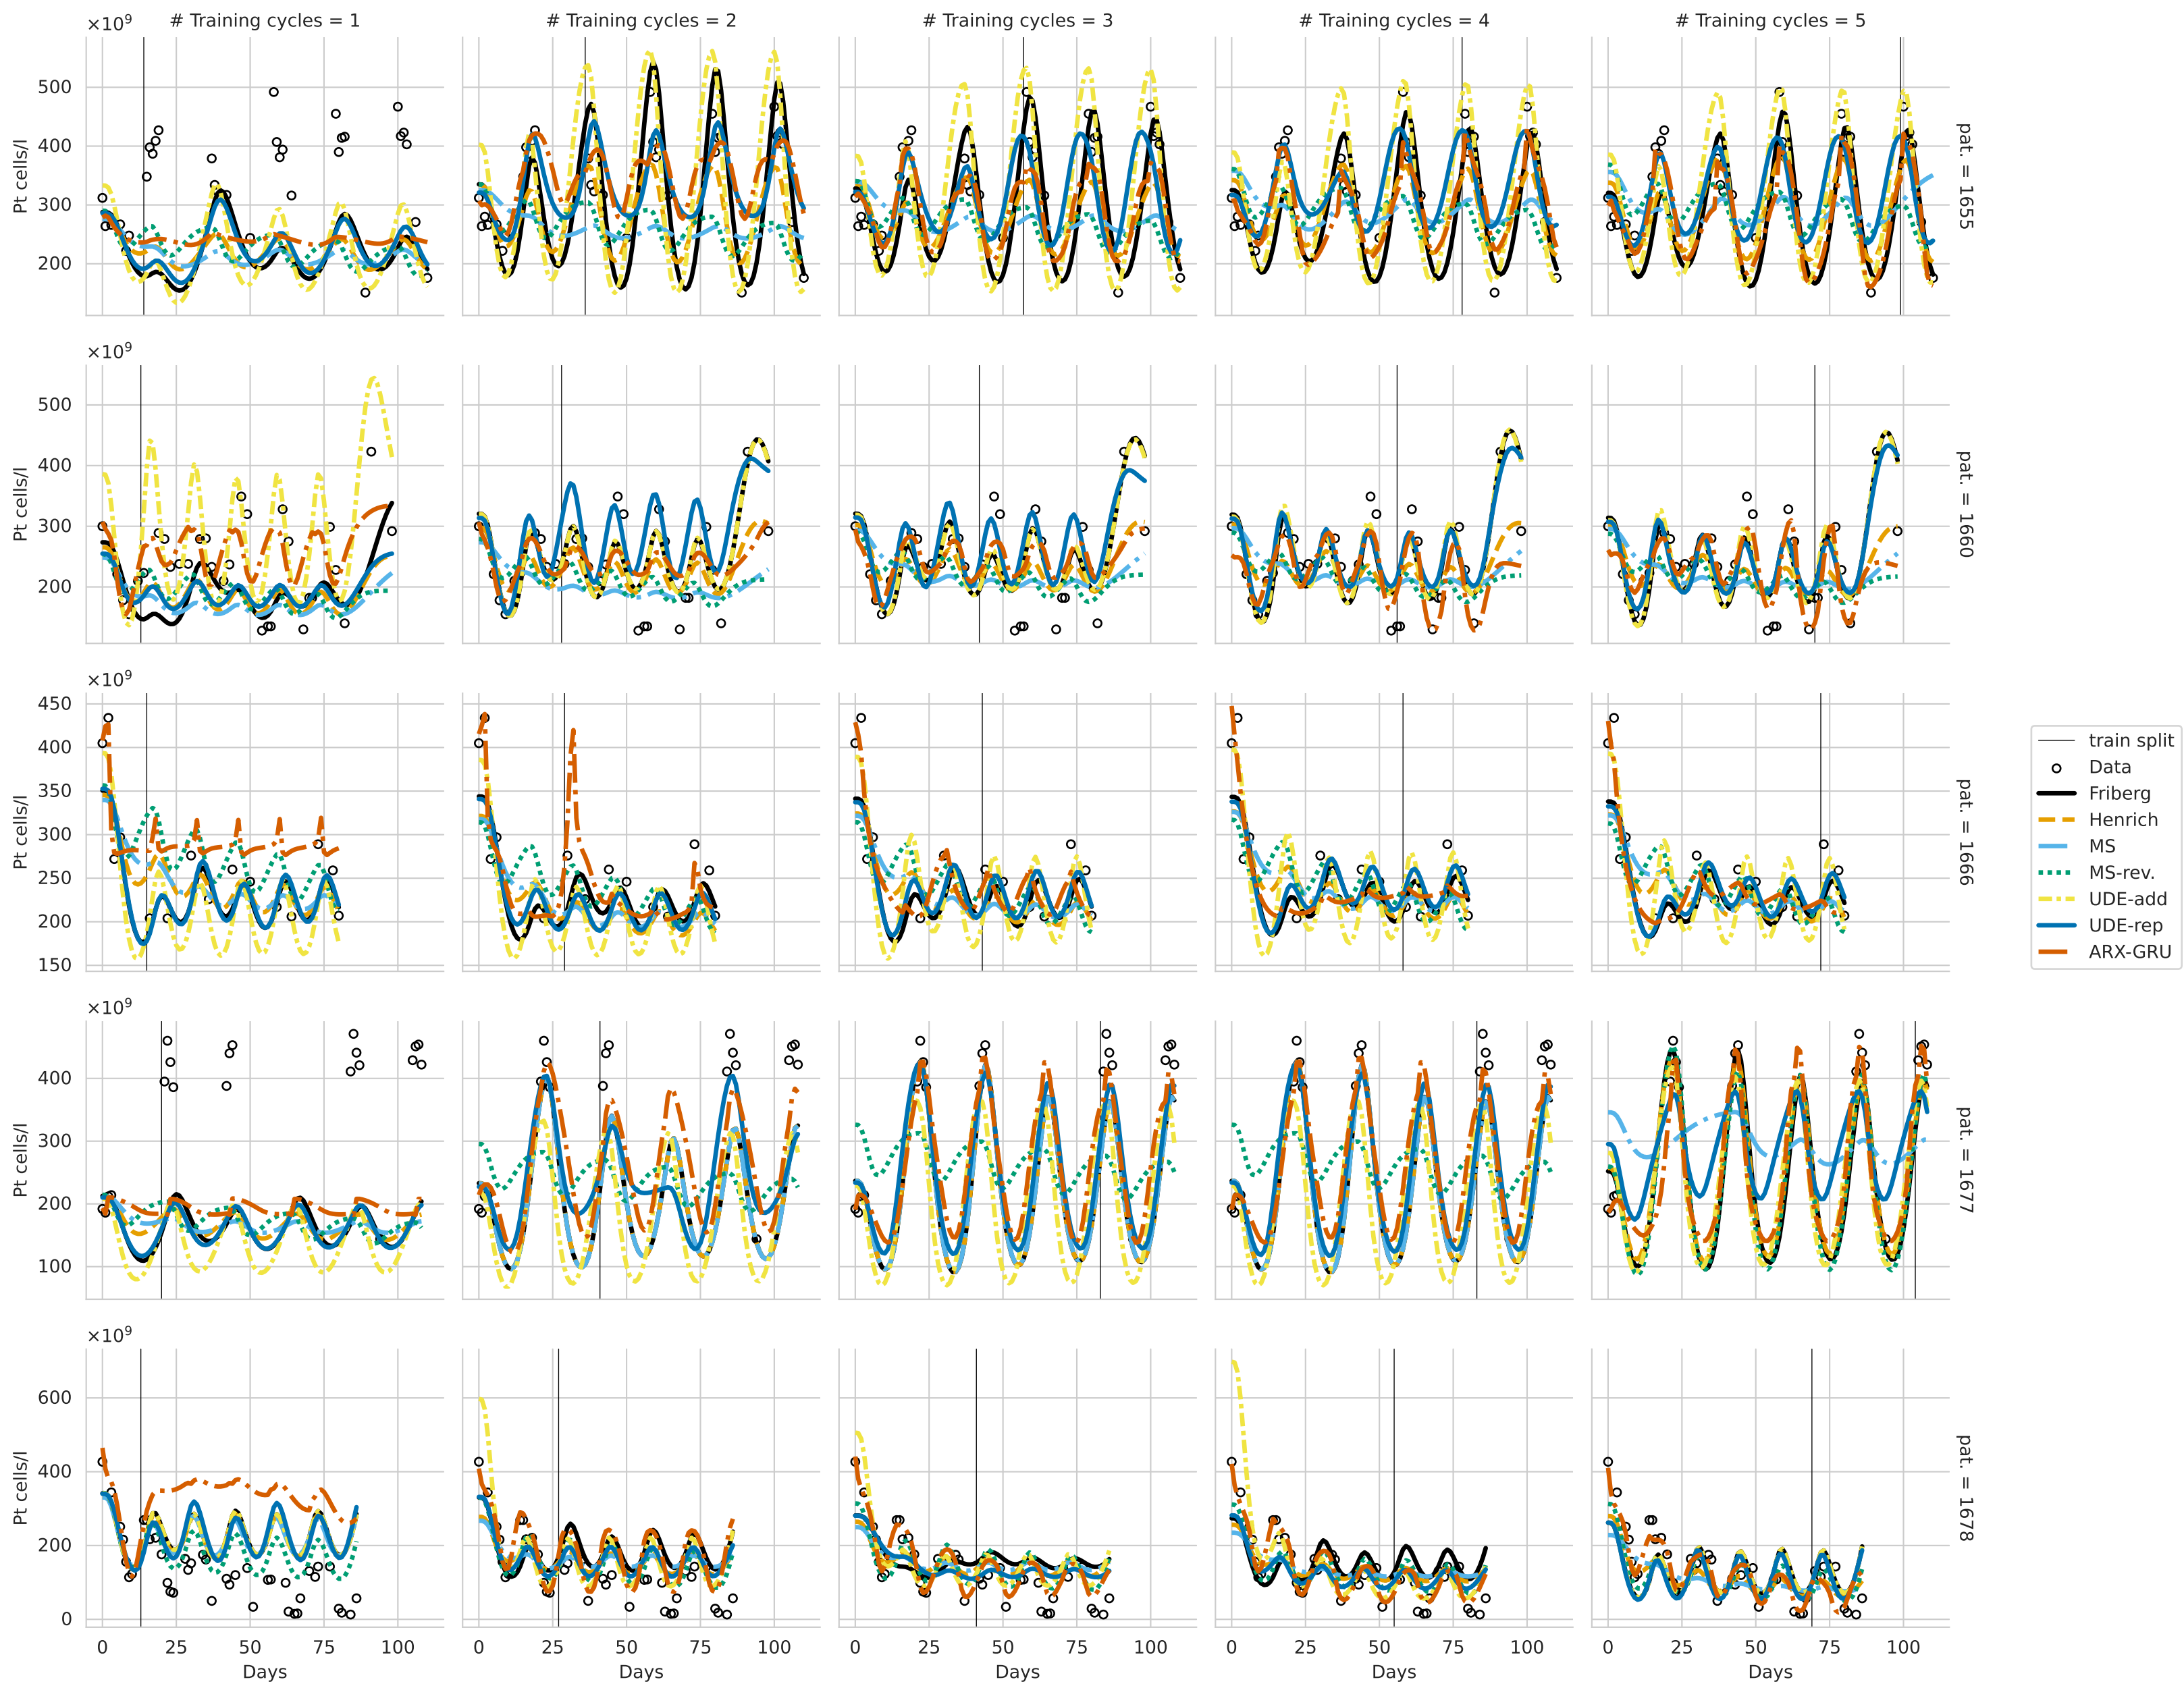

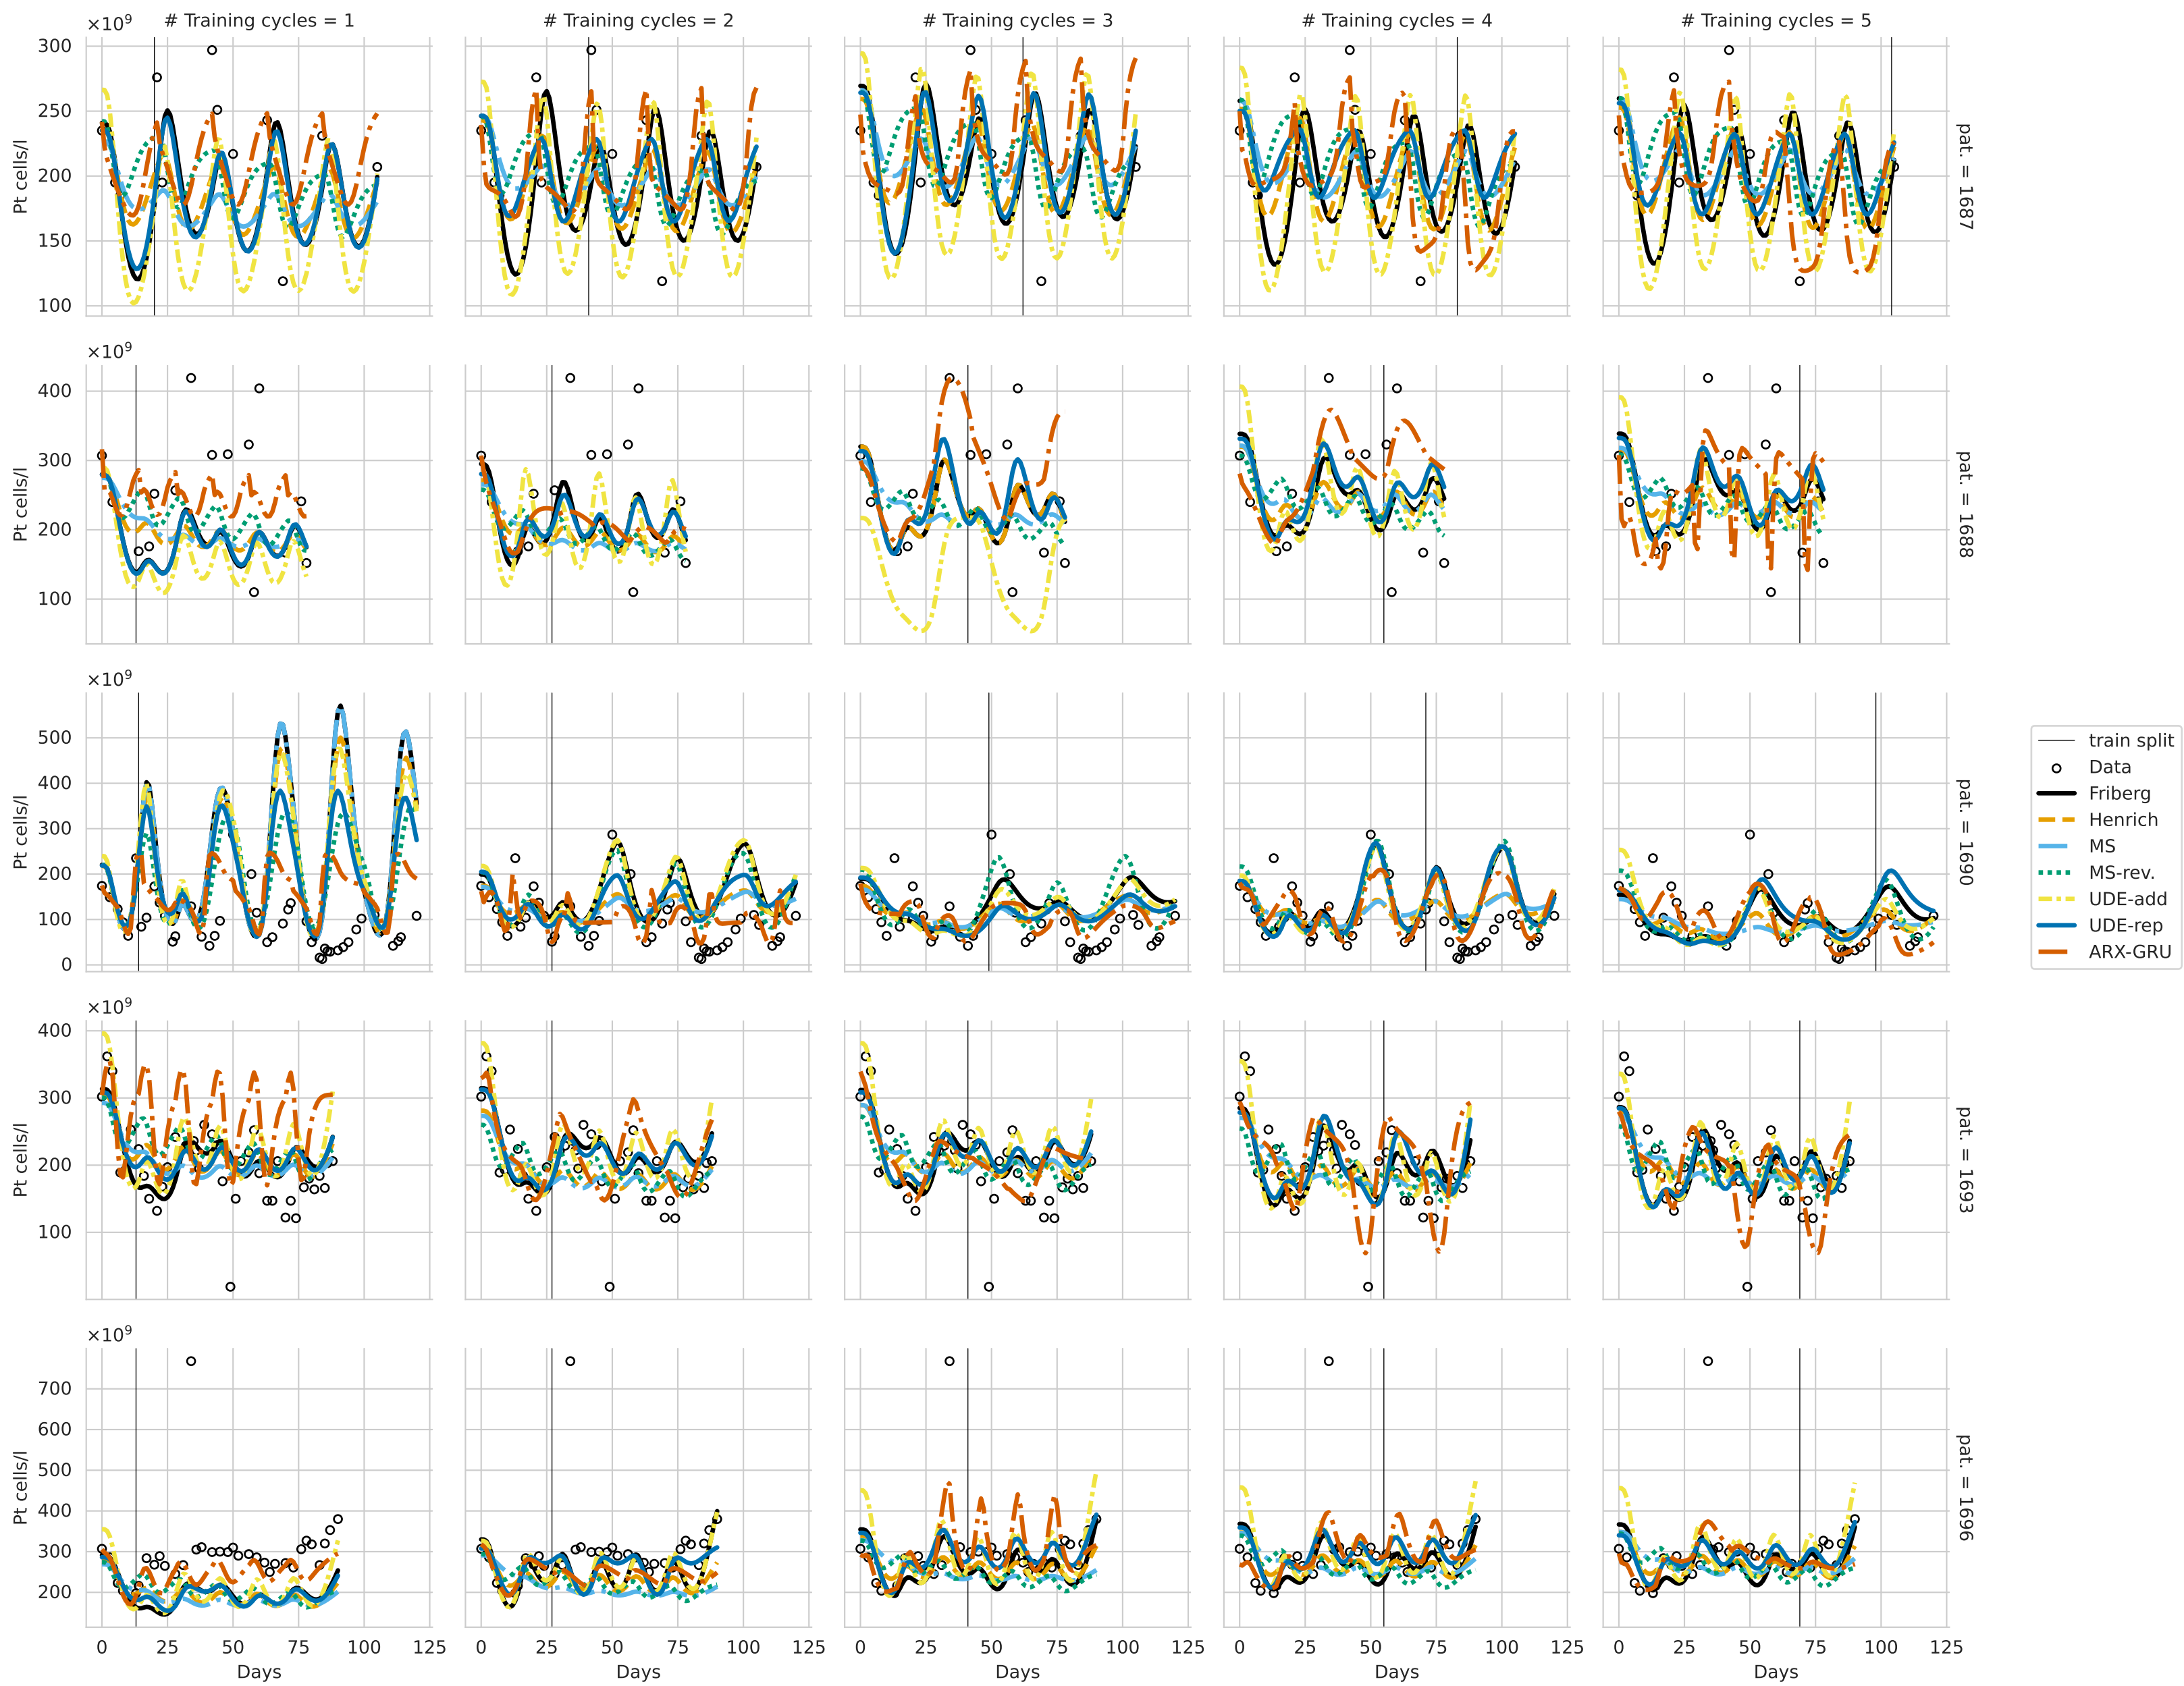

Supplement: Supplementary file 3 [file supplement_2.pdf]
